# Supplementary material for: Relativistic and Electron Correlation Effects in Static Dipole Polarizabilities for Main-Group Elements
Source: arXiv:2408.10513 source file (2024-09-14)
Supplement: Supplementary file 1 [file si.pdf]

# Supporting Information for “Relativistic and Electron Correlation Effects in Static Dipole Polarizabilities for Main-Group Elements”

YingXing Cheng\*

*Institute of Applied Analysis and Numerical Simulation Numerical Mathematics for High Performance Computing, University of Stuttgart, Pfaffenwaldring 57, 70569, Stuttgart, Germany*

E-mail: [yingxing.cheng@mathematik.uni-stuttgart.de](mailto:yingxing.cheng@mathematik.uni-stuttgart.de)

## Contents

|                                             |           |
|---------------------------------------------|-----------|
| <b>S1 Data obtained by fitting Eq. (S1)</b> | <b>6</b>  |
| S1.1 Group 1 elements . . . . .             | 6         |
| S1.2 Group 2 elements . . . . .             | 10        |
| S1.3 Group 13 elements . . . . .            | 14        |
| S1.4 Group 14 elements . . . . .            | 21        |
| S1.5 Group 15 elements . . . . .            | 27        |
| S1.6 Group 16 elements . . . . .            | 30        |
| S1.7 Group 17 elements . . . . .            | 36        |
| S1.8 Group 18 elements . . . . .            | 43        |
| <b>S2 Data obtained by fitting Eq. (S3)</b> | <b>47</b> |
| S2.1 Group 1 elements . . . . .             | 47        |

|                                                           |            |
|-----------------------------------------------------------|------------|
| S2.2 Group 2 elements . . . . .                           | 51         |
| S2.3 Group 13 elements . . . . .                          | 55         |
| S2.4 Group 14 elements . . . . .                          | 62         |
| S2.5 Group 15 elements . . . . .                          | 68         |
| S2.6 Group 16 elements . . . . .                          | 71         |
| S2.7 Group 17 elements . . . . .                          | 77         |
| S2.8 Group 18 elements . . . . .                          | 84         |
| <b>S3 Summary of most accurate results using Eq. (S3)</b> | <b>88</b>  |
| <b>S4 Comparison with literature</b>                      | <b>90</b>  |
| S4.1 Group 1 elements . . . . .                           | 90         |
| S4.2 Group 2 elements . . . . .                           | 95         |
| S4.3 Group 13 elements . . . . .                          | 101        |
| S4.4 Group 14 elements . . . . .                          | 107        |
| S4.5 Group 15 elements . . . . .                          | 111        |
| S4.6 Group 16 elements . . . . .                          | 115        |
| S4.7 Group 17 elements . . . . .                          | 117        |
| S4.8 Group 18 elements . . . . .                          | 120        |
| <b>S5 Uncertainty estimation</b>                          | <b>125</b> |
| S5.1 Group 1 elements . . . . .                           | 125        |
| S5.2 Group 2 elements . . . . .                           | 127        |
| S5.3 Group 13 elements . . . . .                          | 129        |
| S5.4 Group 14 elements . . . . .                          | 131        |
| S5.5 Group 15 elements . . . . .                          | 131        |
| S5.6 Group 16 elements . . . . .                          | 132        |
| S5.7 Group 17 elements . . . . .                          | 132        |
| S5.8 Group 18 elements . . . . .                          | 134        |



Static dipole polarizabilities were computed using the finite-field method.<sup>1</sup> The energy of an atom in an external electric field of strength  $F_z$  along the  $z$ -axis is given by:

$$E(F_z) \approx E_0 - \frac{1}{2}\alpha F_z^2 - \frac{1}{4!}\gamma F_z^4, \quad (\text{S1})$$

where  $E_0$  is the field-free energy,  $\alpha$  is the dipole polarizability, and  $\gamma$  is the dipole hyperpolarizability. Least-squares fitting was used to extract  $\alpha$  and  $\gamma$  from computed energies at different field strengths. In cases where  $\gamma$  resulted in unphysical values, only  $\alpha$  was retained using:

$$E(F_z) \approx E_0 - \frac{1}{2}\alpha F_z^2. \quad (\text{S2})$$

The least-squares procedure is used instead of numerical differentiation for reasons discussed in Ref. 2. In practice, this procedure could lead to an unreasonable  $\gamma$ , including extremely positive or negative values. In these cases, an expansion only including  $\alpha$  is also used:

$$E(F_z) \approx E_0 - \frac{1}{2}\alpha F_z^2. \quad (\text{S3})$$

The results obtained from Eq. (S1), denoted as  $\alpha(2)$ , should always be used instead of the values obtained from Eq. (S3), denoted as  $\alpha(1)$ , except in cases where all the following conditions are satisfied:

1. The relative difference between  $\alpha(1)$  and  $\alpha(2)$ , denoted as  $\tau$ , is greater than 0.6%, i.e.,

$$\tau = \frac{|\alpha(2) - \alpha(1)|}{\alpha(2)} \times 100\% > 0.6\%. \quad (\text{S4})$$

2. An invalid  $\gamma$  is obtained from Eq. (S1). For simplicity, in this work, an invalid  $\gamma$  is defined as when at least one of the following conditions is satisfied:

(a) For CCSD(T) methods,

$$\gamma_{\text{CCSD(T)}} < 0, \quad \gamma_{\text{CCSD}} < 0, \quad \epsilon = \frac{\max(\gamma_{\text{CCSD(T)}}, \gamma_{\text{CCSD}})}{\min(\gamma_{\text{CCSD(T)}}, \gamma_{\text{CCSD}})} > 10, \quad (\text{S5})$$

where  $\gamma_{\text{CCSD(T)}}$  and  $\gamma_{\text{CCSD}}$  are the  $\gamma$  values obtained by the CCSD(T) and CCSD methods, respectively. Here,  $\max(a, b)$  represents the maximum value between  $a$  and  $b$ , and  $\min(a, b)$  represents the minimum value between  $a$  and  $b$ .  $\epsilon$  represents the ratio of the maximum to the minimum of these  $\gamma$  values, indicating a significant difference between the  $\gamma$  values from the two methods when  $\epsilon > 10$ .

(b) For MRCISD methods:

$$\gamma_{\text{MRCISD}} < 0, \quad (\text{S6})$$

where  $\gamma_{\text{MRCISD}}$  refers to the  $\gamma$  value obtained by the MRCISD method.

In this work, a calculation is uniquely identified by a combination of computational method, basis set, and correlation level, represented by a string such as “2C-SR-CC@s-aug-ANO-RCC@ (core 3) [vir 279]”. The different components of this identifier are connected by the delimiter “@”. The first element refers to the computational method, which can be one of several values such as “NR-CC”, “SR-CC”, “DC-CC”, or “DC-CI”. The prefix “2C” or “4C” indicates whether the two-component or four-component relativistic Hamiltonian is used, respectively. The second element denotes the basis set used in the calculation. The last element represents the correlation level, which affects the accuracy of the correlated calculations. In this study, the correlation level is determined by the number of active electrons and virtual orbitals, denoted as “(core n) [vir m]”, where “n” represents the sum of outer-core and valence electrons, and “m” denotes the number of virtual orbitals. In the context of coupled-cluster methods, various correlated methods can be employed, such as DHF, MP2, CCSD, and CCSD(T). All

these methods share the same identifier format. The percentage error  $\delta_m$  is defined as

$$\delta_m = \frac{\alpha_m - \alpha_{\text{CCSD(T)}}}{\alpha_{\text{CCSD(T)}}} \times 100\% \quad (\text{S7})$$

where  $m$  can be DHF, MP2, or CCSD. For open-shell atoms, the difference in dipole polarizability, denoted as  $\Delta\alpha$ , between  $M_L = 0$  and  $M_L = \pm 1$  states is also presented.

The electric field information used to calculate dipole polarizability is provided in the “**calc-info.csv**” file, where “**Atom**”, “**CalcType**”, “**State**”, and “**Field**” correspond to the type of atom, the identifier, the state of the atom, and the electric field applied in atomic units (a.u.). The atomic state includes the ground state (“**gs**”), and for p-block atoms,  $M_L = 0$  and  $M_L = \pm 1$  states are denoted by “**m10**” and “**m11**”, respectively. The “**sym\_X\_root\_N**” represents the “**N**” number of states (roots) in symmetry “**X**” to optimize. For more details, see Ref. 3.

## S1 Data obtained by fitting Eq. (S1)

In the following tables, the results with highlighted identifiers are used to obtain the most accurate results in this work, as shown in the main text. The identifiers with “**NR-CC**”, “**SR-CC**”, “**DC-CC**”, and “**DC-CI**” are highlighted in teal, blue, red, and green, respectively. Additional test results are also included for reliable estimates and basis set choices.

### S1.1 Group 1 elements

Table S1: The results of dipole polarizability for Group 1 elements.

| <b>Z</b> | <b>Atom</b> | <b>State</b>   | $\alpha_D$ (a.u.) | $\delta$ (%) | <b>Method</b> | <b>Comments</b>                                 |
|----------|-------------|----------------|-------------------|--------------|---------------|-------------------------------------------------|
| 3        | Li          | $^2S, M_L = 0$ | 170.13            | 3.52         | DHF           | <b>2C-NR-CC@s-aug-ANO-RCC@(core 3)[vir 229]</b> |
|          |             |                | 164.96            | 0.37         | MP2           |                                                 |
|          |             |                | 164.45            | 0.06         | CCSD          |                                                 |
|          |             |                | 164.34            | —            | CCSD(T)       |                                                 |
|          |             | $^2S, M_L = 0$ | 170.08            | 3.52         | DHF           | 2C-SR-CC@ANO-RCC@(core 3)[vir 179]              |

(continued)

Table S1. continued.

| Z  | Atom | State          | $\alpha_D$ (a.u.) | $\delta$ | Method  | Comments                                  |
|----|------|----------------|-------------------|----------|---------|-------------------------------------------|
|    |      |                | 165.04            | 0.45     | MP2     |                                           |
|    |      |                | 164.40            | 0.06     | CCSD    |                                           |
|    |      |                | 164.30            | --       | CCSD(T) |                                           |
|    |      |                | 170.07            | 3.52     | DHF     | 2C-SR-CC@d-aug-ANO-RCC@(core 3)[vir 279]  |
|    |      | $^2S, M_L = 0$ | $164.72 \pm 0.01$ | 0.27     | MP2     |                                           |
|    |      |                | 164.39            | 0.06     | CCSD    |                                           |
|    |      |                | 164.28            | --       | CCSD(T) |                                           |
|    |      |                | 170.07            | 3.52     | DHF     | 2C-SR-CC@s-aug-ANO-RCC@(core 3)[vir 229]  |
|    |      | $^2S, M_L = 0$ | 164.90            | 0.37     | MP2     |                                           |
|    |      |                | 164.39            | 0.06     | CCSD    |                                           |
|    |      |                | 164.29            | --       | CCSD(T) |                                           |
|    |      |                | 170.06            | 3.50     | DHF     | 4C-DC-CC@s-aug-ANO-RCC@(core 3)[vir 229]  |
|    |      | $^2S_{1/2}$    | $167.33 \pm 1.11$ | 1.84     | MP2     |                                           |
|    |      |                | 164.38            | 0.05     | CCSD    |                                           |
|    |      |                | $164.31 \pm 0.01$ | --       | CCSD(T) |                                           |
|    |      |                | 190.49            | 16.16    | DHF     | 2C-NR-CC@s-aug-ANO-RCC@(core 11)[vir 287] |
| 11 | Na   | $^2S, M_L = 0$ | 164.31            | 0.20     | MP2     |                                           |
|    |      |                | 165.41            | 0.87     | CCSD    |                                           |
|    |      |                | 163.98            | --       | CCSD(T) |                                           |
|    |      |                | 189.42            | 16.21    | DHF     | 2C-SR-CC@ANO-RCC@(core 11)[vir 237]       |
|    |      | $^2S, M_L = 0$ | 163.29            | 0.18     | MP2     |                                           |
|    |      |                | 164.42            | 0.87     | CCSD    |                                           |
|    |      |                | 163.00            | --       | CCSD(T) |                                           |
|    |      |                | 189.42            | 16.23    | DHF     | 2C-SR-CC@d-aug-ANO-RCC@(core 11)[vir 337] |
|    |      | $^2S, M_L = 0$ | $162.79 \pm 0.07$ | -0.11    | MP2     |                                           |
|    |      |                | 164.40            | 0.88     | CCSD    |                                           |
|    |      |                | 162.97            | --       | CCSD(T) |                                           |
|    |      |                | 189.42            | 16.22    | DHF     | 2C-SR-CC@s-aug-ANO-RCC@(core 11)[vir 287] |
|    |      | $^2S, M_L = 0$ | 163.30            | 0.19     | MP2     |                                           |
|    |      |                | 164.41            | 0.87     | CCSD    |                                           |
|    |      |                | 162.99            | --       | CCSD(T) |                                           |
|    |      |                | 189.38            | 15.99    | DHF     | 4C-DC-CC@s-aug-ANO-RCC@(core 11)[vir 287] |
|    |      | $^2S_{1/2}$    | $172.73 \pm 2.94$ | 5.80     | MP2     |                                           |
|    |      |                | 164.38            | 0.68     | CCSD    |                                           |
|    |      |                | $163.27 \pm 0.09$ | --       | CCSD(T) |                                           |
| 19 | K    | $^2S, M_L = 0$ | $417.92 \pm 0.02$ | 41.40    | DHF     | 2C-NR-CC@s-aug-ANO-RCC@(core 19)[vir 311] |
|    |      |                | $267.15 \pm 0.05$ | -9.61    | MP2     |                                           |
|    |      |                | $308.79 \pm 0.01$ | 4.48     | CCSD    |                                           |

(continued)

Table S1. continued.

| Z  | Atom | State          | $\alpha_D$ (a.u.) | $\delta$ | Method  | Comments                                  |
|----|------|----------------|-------------------|----------|---------|-------------------------------------------|
|    |      | $^2S, M_L = 0$ | 295.56            | --       | CCSD(T) |                                           |
|    |      |                | $409.13 \pm 0.01$ | 43.69    | DHF     | 2C-SR-CC@ANO-RCC@(core 19)[vir 261]       |
|    |      |                | $256.44 \pm 0.02$ | -9.94    | MP2     |                                           |
|    |      |                | 298.05            | 4.67     | CCSD    |                                           |
|    |      |                | 284.74            | --       | CCSD(T) |                                           |
|    |      | $^2S, M_L = 0$ | 410.46            | 41.08    | DHF     | 2C-SR-CC@d-aug-ANO-RCC@(core 19)[vir 361] |
|    |      |                | 262.41            | -9.80    | MP2     |                                           |
|    |      |                | 303.82            | 4.43     | CCSD    |                                           |
|    |      |                | 290.93            | --       | CCSD(T) |                                           |
|    |      | $^2S, M_L = 0$ | $410.38 \pm 0.02$ | 41.53    | DHF     | 2C-SR-CC@s-aug-ANO-RCC@(core 19)[vir 311] |
|    |      |                | $261.80 \pm 0.05$ | -9.71    | MP2     |                                           |
|    |      |                | $302.95 \pm 0.01$ | 4.48     | CCSD    |                                           |
|    |      |                | 289.96            | --       | CCSD(T) |                                           |
|    |      | $^2S_{1/2}$    | $410.22 \pm 0.02$ | 41.14    | DHF     | 4C-DC-CC@s-aug-ANO-RCC@(core 19)[vir 311] |
|    |      |                | $283.19 \pm 5.77$ | -2.56    | MP2     |                                           |
|    |      |                | 302.83            | 4.19     | CCSD    |                                           |
|    |      |                | $290.64 \pm 0.24$ | --       | CCSD(T) |                                           |
| 37 | Rb   | $^2S, M_L = 0$ | $525.10 \pm 0.04$ | 52.36    | DHF     | 2C-NR-CC@s-aug-ANO-RCC@(core 27)[vir 247] |
|    |      |                | $285.88 \pm 0.28$ | -17.05   | MP2     |                                           |
|    |      |                | $365.59 \pm 0.01$ | 6.08     | CCSD    |                                           |
|    |      |                | $344.65 \pm 0.01$ | --       | CCSD(T) |                                           |
|    |      | $^2S, M_L = 0$ | $485.99 \pm 0.02$ | 54.62    | DHF     | 2C-SR-CC@ANO-RCC@(core 27)[vir 197]       |
|    |      |                | $258.04 \pm 0.09$ | -17.90   | MP2     |                                           |
|    |      |                | 334.00            | 6.26     | CCSD    |                                           |
|    |      |                | 314.32            | --       | CCSD(T) |                                           |
|    |      | $^2S, M_L = 0$ | 486.26            | 52.01    | DHF     | 2C-SR-CC@d-aug-ANO-RCC@(core 27)[vir 297] |
|    |      |                | $264.62 \pm 0.45$ | -17.28   | MP2     |                                           |
|    |      |                | $338.92 \pm 0.01$ | 5.95     | CCSD    |                                           |
|    |      |                | $319.89 \pm 0.01$ | --       | CCSD(T) |                                           |
|    |      | $^2S, M_L = 0$ | $486.16 \pm 0.03$ | 52.24    | DHF     | 2C-SR-CC@s-aug-ANO-RCC@(core 27)[vir 247] |
|    |      |                | $264.06 \pm 0.21$ | -17.31   | MP2     |                                           |
|    |      |                | 338.45            | 5.98     | CCSD    |                                           |
|    |      |                | $319.34 \pm 0.01$ | --       | CCSD(T) |                                           |
|    |      | $^2S_{1/2}$    | $485.67 \pm 0.03$ | 51.73    | DHF     | 4C-DC-CC@s-aug-ANO-RCC@(core 27)[vir 247] |
|    |      |                | $291.38 \pm 7.1$  | -8.97    | MP2     |                                           |
|    |      |                | $338.13 \pm 0.01$ | 5.64     | CCSD    |                                           |
|    |      |                | $320.08 \pm 0.29$ | --       | CCSD(T) |                                           |
| 55 | Cs   | $^2S, M_L = 0$ | $808.80 \pm 0.02$ | 70.35    | DHF     | 2C-NR-CC@s-aug-ANO-RCC@(core 27)[vir 259] |

(continued)



Table S1. continued.

| Z  | Atom | State          | $\alpha_D$ (a.u.)  | $\delta$ | Method  | Comments                                         |
|----|------|----------------|--------------------|----------|---------|--------------------------------------------------|
|    |      |                | $323.81 \pm 0.83$  | -31.80   | MP2     |                                                  |
|    |      |                | $520.21 \pm 0.01$  | 9.57     | CCSD    |                                                  |
|    |      |                | $474.79 \pm 0.05$  | --       | CCSD(T) |                                                  |
|    |      | $^2S, M_L = 0$ | $670.54 \pm 0.02$  | 68.73    | DHF     | <b>2C-SR-CC@s-aug-ANO-RCC@(core 27)[vir 259]</b> |
|    |      |                | $270.10 \pm 0.56$  | -32.03   | MP2     |                                                  |
|    |      |                | $433.09 \pm 0.01$  | 8.98     | CCSD    |                                                  |
|    |      |                | $397.40 \pm 0.02$  | --       | CCSD(T) |                                                  |
|    |      | $^2S_{1/2}$    | $668.83 \pm 0.04$  | 67.98    | DHF     | 4C-DC-CC@d-aug-ANO-RCC@(core 27)[vir 309]        |
|    |      |                | $302.59 \pm 8.75$  | -24.00   | MP2     |                                                  |
|    |      |                | $432.13 \pm 0.02$  | 8.53     | CCSD    |                                                  |
|    |      |                | $398.16 \pm 0.4$   | --       | CCSD(T) |                                                  |
|    |      | $^2S_{1/2}$    | $668.83 \pm 0.01$  | 67.41    | DHF     | 4C-DC-CC@faegri@(core 27)[vir 299]               |
|    |      |                | $303.03 \pm 13.36$ | -24.15   | MP2     |                                                  |
|    |      |                | 436.01             | 9.13     | CCSD    |                                                  |
|    |      |                | $399.52 \pm 0.62$  | --       | CCSD(T) |                                                  |
|    |      | $^2S_{1/2}$    | $668.93 \pm 0.02$  | 67.97    | DHF     | <b>4C-DC-CC@s-aug-ANO-RCC@(core 27)[vir 259]</b> |
|    |      |                | $307.07 \pm 9.76$  | -22.89   | MP2     |                                                  |
|    |      |                | $432.12 \pm 0.01$  | 8.51     | CCSD    |                                                  |
|    |      |                | $398.24 \pm 0.41$  | --       | CCSD(T) |                                                  |
| 87 | Fr   | $^2S, M_L = 0$ | $968.32 \pm 0.03$  | 78.78    | DHF     | <b>2C-NR-CC@s-aug-ANO-RCC@(core 41)[vir 217]</b> |
|    |      |                | $314.41 \pm 1.13$  | -41.95   | MP2     |                                                  |
|    |      |                | 604.83             | 11.67    | CCSD    |                                                  |
|    |      |                | $541.62 \pm 0.04$  | --       | CCSD(T) |                                                  |
|    |      | $^2S, M_L = 0$ | 539.80             | 69.37    | DHF     | 2C-SR-CC@ANO-RCC@(core 41)[vir 185]              |
|    |      |                | $192.73 \pm 0.53$  | -39.53   | MP2     |                                                  |
|    |      |                | 347.22             | 8.94     | CCSD    |                                                  |
|    |      |                | $318.72 \pm 0.02$  | --       | CCSD(T) |                                                  |
|    |      | $^2S, M_L = 0$ | $539.73 \pm 0.02$  | 69.08    | DHF     | 2C-SR-CC@d-aug-ANO-RCC@(core 41)[vir 249]        |
|    |      |                | $191.06 \pm 0.88$  | -40.15   | MP2     |                                                  |
|    |      |                | $347.73 \pm 0.01$  | 8.93     | CCSD    |                                                  |
|    |      |                | $319.21 \pm 0.03$  | --       | CCSD(T) |                                                  |
|    |      | $^2S, M_L = 0$ | 539.78             | 69.02    | DHF     | <b>2C-SR-CC@s-aug-ANO-RCC@(core 41)[vir 217]</b> |
|    |      |                | $194.23 \pm 0.28$  | -39.18   | MP2     |                                                  |
|    |      |                | 347.75             | 8.89     | CCSD    |                                                  |
|    |      |                | $319.36 \pm 0.01$  | --       | CCSD(T) |                                                  |
|    |      | $^2S_{1/2}$    | 530.15             | 67.03    | DHF     | <b>4C-DC-CC@s-aug-ANO-RCC@(core 41)[vir 217]</b> |
|    |      |                | $228.54 \pm 12.66$ | -28.00   | MP2     |                                                  |
|    |      |                | 343.52             | 8.23     | CCSD    |                                                  |

(continued)

Table S1. continued.

| Z | Atom | State | $\alpha_D$ (a.u.) | $\delta$ | Method  | Comments |
|---|------|-------|-------------------|----------|---------|----------|
|   |      |       | $317.40 \pm 0.57$ | --       | CCSD(T) |          |

## S1.2 Group 2 elements

Table S2: The results of dipole polarizability for Group 2 elements.

| Z  | Atom | State          | $\alpha_D$ (a.u.) | $\delta$ (%) | Method  | Comments                                                     |
|----|------|----------------|-------------------|--------------|---------|--------------------------------------------------------------|
| 4  | Be   | $^1S, M_L = 0$ | 45.62             | 20.67        | DHF     | <a href="#">2C-NR-CC@d-aug-dyall.cv4z@(core 4)[vir 266]</a>  |
|    |      |                | 42.10             | 11.36        | MP2     |                                                              |
|    |      |                | 37.96             | 0.42         | CCSD    |                                                              |
|    |      |                | 37.80             | --           | CCSD(T) |                                                              |
|    |      | $^1S, M_L = 0$ | 45.59             | 20.66        | DHF     | <a href="#">2C-SR-CC@d-aug-dyall.cv4z@(core 4)[vir 266]</a>  |
|    |      |                | 42.08             | 11.36        | MP2     |                                                              |
|    |      |                | 37.94             | 0.42         | CCSD    |                                                              |
|    |      |                | 37.79             | --           | CCSD(T) |                                                              |
|    |      | $^1S, M_L = 0$ | 45.59             | 23.45        | DHF     | 2C-SR-CC@dyall.cv4z@(core 4)[vir 166]                        |
|    |      |                | 41.47             | 12.31        | MP2     |                                                              |
|    |      |                | 37.11             | 0.48         | CCSD    |                                                              |
|    |      |                | 36.93             | --           | CCSD(T) |                                                              |
|    |      | $^1S, M_L = 0$ | 45.59             | 20.67        | DHF     | 2C-SR-CC@s-aug-dyall.cv4z@(core 4)[vir 216]                  |
|    |      |                | 42.07             | 11.34        | MP2     |                                                              |
|    |      |                | 37.94             | 0.42         | CCSD    |                                                              |
|    |      |                | 37.78             | --           | CCSD(T) |                                                              |
|    |      | $^1S_0$        | 45.59             | 20.66        | DHF     | <a href="#">4C-DC-CC@d-aug-dyall.cv4z@(core 4)[vir 266]</a>  |
|    |      |                | 42.07             | 11.36        | MP2     |                                                              |
|    |      |                | 37.94             | 0.42         | CCSD    |                                                              |
|    |      |                | 37.78             | --           | CCSD(T) |                                                              |
|    |      | $^1S_0$        | 45.59             | 23.06        | DHF     | 4C-DC-CC@dyall.cv4z@(core 4)[vir 132]                        |
|    |      |                | 41.64             | 12.40        | MP2     |                                                              |
|    |      |                | 37.18             | 0.36         | CCSD    |                                                              |
|    |      |                | 37.04             | --           | CCSD(T) |                                                              |
| 12 | Mg   | $^1S, M_L = 0$ | 81.59             | 14.05        | DHF     | <a href="#">2C-NR-CC@d-aug-dyall.cv4z@(core 10)[vir 314]</a> |
|    |      |                | 71.92             | 0.53         | MP2     |                                                              |
|    |      |                | 72.18             | 0.89         | CCSD    |                                                              |
|    |      |                | 71.54             | --           | CCSD(T) |                                                              |

(continued)

Table S2. continued.

| Z  | Atom | State          | $\alpha_D$ (a.u.) | $\delta$ | Method  | Comments                                                     |
|----|------|----------------|-------------------|----------|---------|--------------------------------------------------------------|
|    |      | $^1S, M_L = 0$ | 81.17             | 14.00    | DHF     | <a href="#">2C-SR-CC@d-aug-dyall.cv4z@(core 10)[vir 314]</a> |
|    |      |                | 71.55             | 0.49     | MP2     |                                                              |
|    |      |                | 71.83             | 0.88     | CCSD    |                                                              |
|    |      |                | 71.20             | --       | CCSD(T) |                                                              |
|    |      | $^1S, M_L = 0$ | 81.16             | 14.90    | DHF     | 2C-SR-CC@dyall.cv4z@(core 10)[vir 214]                       |
|    |      |                | 70.69             | 0.07     | MP2     |                                                              |
|    |      |                | 71.29             | 0.93     | CCSD    |                                                              |
|    |      |                | 70.64             | --       | CCSD(T) |                                                              |
|    |      | $^1S, M_L = 0$ | 81.17             | 14.00    | DHF     | 2C-SR-CC@s-aug-dyall.cv4z@(core 10)[vir 264]                 |
|    |      |                | 71.54             | 0.48     | MP2     |                                                              |
|    |      |                | 71.83             | 0.88     | CCSD    |                                                              |
|    |      |                | 71.20             | --       | CCSD(T) |                                                              |
|    |      | $^1S_0$        | 81.15             | 14.00    | DHF     | <a href="#">4C-DC-CC@d-aug-dyall.cv4z@(core 10)[vir 314]</a> |
|    |      |                | 71.54             | 0.49     | MP2     |                                                              |
|    |      |                | 71.82             | 0.88     | CCSD    |                                                              |
|    |      |                | 71.19             | --       | CCSD(T) |                                                              |
|    |      | $^1S_0$        | 81.15             | 14.64    | DHF     | 4C-DC-CC@dyall.cv4z@(core 10)[vir 182]                       |
|    |      |                | 70.88             | 0.13     | MP2     |                                                              |
|    |      |                | 71.33             | 0.76     | CCSD    |                                                              |
|    |      |                | 70.79             | --       | CCSD(T) |                                                              |
| 20 | Ca   | $^1S, M_L = 0$ | 185.43            | 15.97    | DHF     | <a href="#">2C-NR-CC@d-aug-dyall.cv4z@(core 20)[vir 510]</a> |
|    |      |                | 143.48            | -10.27   | MP2     |                                                              |
|    |      |                | 162.83            | 1.83     | CCSD    |                                                              |
|    |      |                | 159.90            | --       | CCSD(T) |                                                              |
|    |      | $^1S, M_L = 0$ | 182.83            | 16.00    | DHF     | <a href="#">2C-SR-CC@d-aug-dyall.cv4z@(core 20)[vir 510]</a> |
|    |      |                | 141.50            | -10.22   | MP2     |                                                              |
|    |      |                | 160.53            | 1.85     | CCSD    |                                                              |
|    |      |                | 157.61            | --       | CCSD(T) |                                                              |
|    |      | $^1S, M_L = 0$ | 182.84            | 17.07    | DHF     | 2C-SR-CC@dyall.cv4z@(core 20)[vir 410]                       |
|    |      |                | 139.08            | -10.95   | MP2     |                                                              |
|    |      |                | 159.25            | 1.96     | CCSD    |                                                              |
|    |      |                | 156.19            | --       | CCSD(T) |                                                              |
|    |      | $^1S, M_L = 0$ | 182.84            | 16.01    | DHF     | 2C-SR-CC@s-aug-dyall.cv4z@(core 20)[vir 460]                 |
|    |      |                | 141.49            | -10.23   | MP2     |                                                              |
|    |      |                | 160.53            | 1.85     | CCSD    |                                                              |
|    |      |                | 157.61            | --       | CCSD(T) |                                                              |
|    |      | $^1S_0$        | 182.79            | 16.02    | DHF     | 2C-DC-CC@s-aug-dyall.cv4z@(core 20)[vir 296]                 |
|    |      |                | 141.44            | -10.23   | MP2     |                                                              |

(continued)

Table S2. continued.

| Z  | Atom | State          | $\alpha_D$ (a.u.) | $\delta$ | Method  | Comments                                            |
|----|------|----------------|-------------------|----------|---------|-----------------------------------------------------|
| 38 | Sr   | $^1S_0$        | 160.39            | 1.80     | CCSD    | <b>4C-DC-CC@d-aug-dyall.cv4z@(core 20)[vir 346]</b> |
|    |      |                | 157.55            | --       | CCSD(T) |                                                     |
|    |      |                | 182.78            | 16.01    | DHF     |                                                     |
|    |      |                | 141.46            | -10.22   | MP2     |                                                     |
|    |      |                | 160.39            | 1.80     | CCSD    |                                                     |
|    |      |                | 157.55            | --       | CCSD(T) |                                                     |
|    |      | $^1S_0$        | 182.79            | 16.95    | DHF     | 4C-DC-CC@dyall.cv4z@(core 20)[vir 228]              |
|    |      |                | 139.43            | -10.80   | MP2     |                                                     |
|    |      |                | 159.19            | 1.85     | CCSD    |                                                     |
|    |      |                | 156.30            | --       | CCSD(T) |                                                     |
|    |      | $^1S, M_L = 0$ | 245.98 $\pm$ 0.01 | 17.34    | DHF     | <b>2C-NR-CC@s-aug-dyall.cv4z@(core 28)[vir 346]</b> |
|    |      |                | 179.52            | -14.37   | MP2     |                                                     |
|    |      |                | 214.36 $\pm$ 0.01 | 2.26     | CCSD    |                                                     |
|    |      |                | 209.64 $\pm$ 0.01 | --       | CCSD(T) |                                                     |
|    |      | $^1S, M_L = 0$ | 232.70 $\pm$ 0.01 | 17.66    | DHF     | 2C-SR-CC@d-aug-dyall.cv4z@(core 28)[vir 418]        |
|    |      |                | 170.18            | -13.96   | MP2     |                                                     |
|    |      |                | 202.44            | 2.36     | CCSD    |                                                     |
|    |      |                | 197.78            | --       | CCSD(T) |                                                     |
|    |      | $^1S, M_L = 0$ | 232.74            | 17.87    | DHF     | 2C-SR-CC@dyall.cv4z@(core 28)[vir 274]              |
|    |      |                | 167.29            | -15.28   | MP2     |                                                     |
|    |      |                | 202.09            | 2.35     | CCSD    |                                                     |
|    |      |                | 197.45            | --       | CCSD(T) |                                                     |
|    |      | $^1S, M_L = 0$ | 232.71 $\pm$ 0.01 | 17.63    | DHF     | <b>2C-SR-CC@s-aug-dyall.cv4z@(core 28)[vir 346]</b> |
|    |      |                | 170.23            | -13.95   | MP2     |                                                     |
|    |      |                | 202.44            | 2.34     | CCSD    |                                                     |
|    |      |                | 197.82            | --       | CCSD(T) |                                                     |
|    |      | $^1S_0$        | 232.55 $\pm$ 0.01 | 17.64    | DHF     | <b>2C-DC-CC@s-aug-dyall.cv4z@(core 28)[vir 346]</b> |
|    |      |                | 170.12            | -13.94   | MP2     |                                                     |
|    |      |                | 202.29 $\pm$ 0.01 | 2.34     | CCSD    |                                                     |
|    |      |                | 197.67 $\pm$ 0.01 | --       | CCSD(T) |                                                     |
|    |      | $^1S_0$        | 232.59            | 17.32    | DHF     | 4C-DC-CC@dyall.cv4z@(core 20)[vir 214]              |
|    |      |                | 169.11            | -14.70   | MP2     |                                                     |
|    |      |                | 202.68            | 2.24     | CCSD    |                                                     |
|    |      |                | 198.24            | --       | CCSD(T) |                                                     |
| 56 | Ba   | $^1S, M_L = 0$ | 368.03 $\pm$ 0.01 | 16.25    | DHF     | <b>2C-NR-CC@s-aug-dyall.cv4z@(core 28)[vir 398]</b> |
|    |      |                | 243.98 $\pm$ 0.01 | -22.93   | MP2     |                                                     |
|    |      |                | 323.68 $\pm$ 0.01 | 2.24     | CCSD    |                                                     |
|    |      |                | 316.58 $\pm$ 0.01 | --       | CCSD(T) |                                                     |

(continued)

Table S2. continued.

| Z  | Atom | State          | $\alpha_D$ (a.u.) | $\delta$ | Method  | Comments                                     |
|----|------|----------------|-------------------|----------|---------|----------------------------------------------|
|    |      | $^1S, M_L = 0$ | $324.30 \pm 0.02$ | 18.59    | DHF     | 2C-SR-CC@d-aug-dyall.cv4z@(core 28)[vir 470] |
|    |      |                | $216.09 \pm 0.01$ | -20.98   | MP2     |                                              |
|    |      |                | $281.69 \pm 0.01$ | 3.01     | CCSD    |                                              |
|    |      |                | 273.46            | --       | CCSD(T) |                                              |
|    |      | $^1S, M_L = 0$ | 324.43            | 18.91    | DHF     | 2C-SR-CC@dyall.cv4z@(core 28)[vir 326]       |
|    |      |                | 212.86            | -21.98   | MP2     |                                              |
|    |      |                | 281.23            | 3.08     | CCSD    |                                              |
|    |      |                | 272.83            | --       | CCSD(T) |                                              |
|    |      | $^1S, M_L = 0$ | $324.36 \pm 0.01$ | 18.40    | DHF     | 2C-SR-CC@s-aug-dyall.cv4z@(core 28)[vir 398] |
|    |      |                | 216.82            | -20.86   | MP2     |                                              |
|    |      |                | 282.15            | 2.99     | CCSD    |                                              |
|    |      |                | 273.96            | --       | CCSD(T) |                                              |
|    |      | $^1S_0$        | $323.86 \pm 0.01$ | 18.41    | DHF     | 2C-DC-CC@s-aug-dyall.cv4z@(core 28)[vir 398] |
|    |      |                | 216.61            | -20.80   | MP2     |                                              |
|    |      |                | 281.69            | 2.99     | CCSD    |                                              |
|    |      |                | 273.51            | --       | CCSD(T) |                                              |
|    |      | $^1S_0$        | 323.97            | 18.25    | DHF     | 4C-DC-CC@dyall.cv4z@(core 20)[vir 252]       |
|    |      |                | 214.87            | -21.57   | MP2     |                                              |
|    |      |                | 282.08            | 2.96     | CCSD    |                                              |
|    |      |                | 273.97            | --       | CCSD(T) |                                              |
| 88 | Ra   | $^1S, M_L = 0$ | $441.41 \pm 0.01$ | 16.52    | DHF     | 2C-NR-CC@s-aug-dyall.cv4z@(core 42)[vir 378] |
|    |      |                | 277.90            | -26.64   | MP2     |                                              |
|    |      |                | $387.80 \pm 0.01$ | 2.37     | CCSD    |                                              |
|    |      |                | $378.82 \pm 0.01$ | --       | CCSD(T) |                                              |
|    |      | $^1S, M_L = 0$ | $299.65 \pm 0.02$ | 21.22    | DHF     | 2C-SR-CC@d-aug-dyall.cv4z@(core 42)[vir 450] |
|    |      |                | $196.10 \pm 0.01$ | -20.67   | MP2     |                                              |
|    |      |                | 256.51            | 3.77     | CCSD    |                                              |
|    |      |                | 247.20            | --       | CCSD(T) |                                              |
|    |      | $^1S, M_L = 0$ | 299.76            | 21.74    | DHF     | 2C-SR-CC@dyall.cv4z@(core 42)[vir 306]       |
|    |      |                | 191.90            | -22.06   | MP2     |                                              |
|    |      |                | 255.61            | 3.81     | CCSD    |                                              |
|    |      |                | 246.22            | --       | CCSD(T) |                                              |
|    |      | $^1S, M_L = 0$ | $299.71 \pm 0.01$ | 21.00    | DHF     | 2C-SR-CC@s-aug-dyall.cv4z@(core 42)[vir 378] |
|    |      |                | 196.94            | -20.49   | MP2     |                                              |
|    |      |                | $256.97 \pm 0.01$ | 3.75     | CCSD    |                                              |
|    |      |                | $247.69 \pm 0.01$ | --       | CCSD(T) |                                              |
|    |      | $^1S_0$        | $296.71 \pm 0.01$ | 20.77    | DHF     | 2C-DC-CC@s-aug-dyall.cv4z@(core 42)[vir 380] |
|    |      |                | 196.84            | -19.88   | MP2     |                                              |

(continued)

Table S2. continued.

| Z | Atom | State   | $\alpha_D$ (a.u.) | $\delta$ | Method  | Comments                               |
|---|------|---------|-------------------|----------|---------|----------------------------------------|
|   |      |         | $254.70 \pm 0.01$ | 3.67     | CCSD    |                                        |
|   |      |         | $245.68 \pm 0.01$ | --       | CCSD(T) |                                        |
|   |      | $^1S_0$ | 296.97            | 20.75    | DHF     | 4C-DC-CC@dyall.cv4z@(core 20)[vir 234] |
|   |      |         | 194.89            | -20.75   | MP2     |                                        |
|   |      |         | 254.71            | 3.57     | CCSD    |                                        |
|   |      |         | 245.94            | --       | CCSD(T) |                                        |

### S1.3 Group 13 elements

Table S3: The results of dipole polarizability for Group 13 elements.

| Z | Atom | State              | $\alpha_D$ (a.u.) | $\delta$ (%) | Method  | Comments                                      |
|---|------|--------------------|-------------------|--------------|---------|-----------------------------------------------|
| 5 | B    | $^2P, M_L = 0$     | $24.61 \pm 0.01$  | 1.55         | DHF     | <b>2C-NR-CC@dyall.acv4z@(core 5)[vir 251]</b> |
|   |      | $^2P, M_L = \pm 1$ | 19.46             | 5.17         |         |                                               |
|   |      | $^2P$              | 21.17             | 3.74         |         | $\Delta\alpha = -5.15$                        |
|   |      | $^2P, M_L = 0$     | $23.48 \pm 0.07$  | -3.12        | MP2     |                                               |
|   |      | $^2P, M_L = \pm 1$ | $19.43 \pm 0.01$  | 5.05         |         |                                               |
|   |      | $^2P$              | $20.78 \pm 0.04$  | 1.81         |         | $\Delta\alpha = -4.05$                        |
|   |      | $^2P, M_L = 0$     | $24.21 \pm 0.01$  | -0.11        | CCSD    |                                               |
|   |      | $^2P, M_L = \pm 1$ | 18.48             | -0.13        |         |                                               |
|   |      | $^2P$              | $20.39 \pm 0.01$  | -0.12        |         | $\Delta\alpha = -5.73$                        |
|   |      | $^2P, M_L = 0$     | $24.23 \pm 0.01$  | --           | CCSD(T) |                                               |
|   |      | $^2P, M_L = \pm 1$ | 18.50             | --           |         |                                               |
|   |      | $^2P$              | 20.41             | --           |         | $\Delta\alpha = -5.74$                        |
|   |      | $^2P, M_L = 0$     | $24.61 \pm 0.01$  | 1.51         | DHF     | <b>2C-SR-CC@dyall.acv4z@(core 5)[vir 251]</b> |
|   |      | $^2P, M_L = \pm 1$ | 19.44             | 5.23         |         |                                               |
|   |      | $^2P$              | 21.17             | 3.76         |         | $\Delta\alpha = -5.17$                        |
|   |      | $^2P, M_L = 0$     | $23.41 \pm 0.08$  | -3.46        | MP2     |                                               |
|   |      | $^2P, M_L = \pm 1$ | $19.40 \pm 0.01$  | 4.98         |         |                                               |
|   |      | $^2P$              | $20.73 \pm 0.05$  | 1.63         |         | $\Delta\alpha = -4.01$                        |
|   |      | $^2P, M_L = 0$     | $24.21 \pm 0.01$  | -0.13        | CCSD    |                                               |
|   |      | $^2P, M_L = \pm 1$ | 18.47             | -0.06        |         |                                               |
|   |      | $^2P$              | 20.38             | -0.09        |         | $\Delta\alpha = -5.75$                        |
|   |      | $^2P, M_L = 0$     | $24.25 \pm 0.01$  | --           | CCSD(T) |                                               |
|   |      | $^2P, M_L = \pm 1$ | 18.48             | --           |         |                                               |

(continued)

Table S3. continued.

| Z  | Atom | State                      | $\alpha_D$ (a.u.) | $\delta$ | Method  | Comments                                                |
|----|------|----------------------------|-------------------|----------|---------|---------------------------------------------------------|
|    |      | $^2P$                      | $20.40 \pm 0.01$  | --       |         | $\Delta\alpha = -5.77$                                  |
|    |      | $^2P_{1/2}$                | 20.35             |          | MRCISD  | <a href="#">4C-DC-CI@dyall.acv4z@(core 5)[vir 251]</a>  |
|    |      | $^2P_{3/2}, M_J = \pm 1/2$ | 22.31             |          |         |                                                         |
|    |      | $^2P_{3/2}, M_J = \pm 3/2$ | 18.46             |          |         |                                                         |
|    |      | $^2P_{3/2}$                | 20.38             |          |         | $\bar{\alpha}_{J=3/2} - \alpha_{J=1/2} = 0.03$          |
| 13 | Al   | $^2P, M_L = 0$             | $71.65 \pm 1.5$   | 4.47     | DHF     | <a href="#">2C-NR-CC@dyall.acv4z@(core 13)[vir 363]</a> |
|    |      | $^2P, M_L = \pm 1$         | $53.60 \pm 0.06$  | 9.49     |         |                                                         |
|    |      | $^2P$                      | $59.62 \pm 0.87$  | 7.42     |         | $\Delta\alpha = -18.05$                                 |
|    |      | $^2P, M_L = 0$             | $69.92 \pm 0.34$  | 1.95     | MP2     |                                                         |
|    |      | $^2P, M_L = \pm 1$         | $51.09 \pm 0.07$  | 4.35     |         |                                                         |
|    |      | $^2P$                      | $57.37 \pm 0.2$   | 3.36     |         | $\Delta\alpha = -18.84$                                 |
|    |      | $^2P, M_L = 0$             | $68.33 \pm 0.89$  | -0.37    | CCSD    |                                                         |
|    |      | $^2P, M_L = \pm 1$         | $49.06 \pm 0.01$  | 0.21     |         |                                                         |
|    |      | $^2P$                      | $55.48 \pm 0.51$  | -0.03    |         | $\Delta\alpha = -19.28$                                 |
|    |      | $^2P, M_L = 0$             | $68.59 \pm 0.81$  | --       | CCSD(T) |                                                         |
|    |      | $^2P, M_L = \pm 1$         | $48.95 \pm 0.01$  | --       |         |                                                         |
|    |      | $^2P$                      | $55.50 \pm 0.47$  | --       |         | $\Delta\alpha = -19.63$                                 |
|    |      | $^2P, M_L = 0$             | $71.84 \pm 1.52$  | 3.71     | DHF     | <a href="#">2C-SR-CC@dyall.acv4z@(core 11)[vir 223]</a> |
|    |      | $^2P, M_L = \pm 1$         | $53.50 \pm 0.06$  | 8.91     |         |                                                         |
|    |      | $^2P$                      | $59.62 \pm 0.88$  | 6.76     |         | $\Delta\alpha = -18.34$                                 |
|    |      | $^2P, M_L = 0$             | $70.77 \pm 0.38$  | 2.16     | MP2     |                                                         |
|    |      | $^2P, M_L = \pm 1$         | $51.34 \pm 0.07$  | 4.52     |         |                                                         |
|    |      | $^2P$                      | $57.82 \pm 0.23$  | 3.54     |         | $\Delta\alpha = -19.42$                                 |
|    |      | $^2P, M_L = 0$             | $69.01 \pm 0.92$  | -0.38    | CCSD    |                                                         |
|    |      | $^2P, M_L = \pm 1$         | $49.18 \pm 0.01$  | 0.12     |         |                                                         |
|    |      | $^2P$                      | $55.79 \pm 0.53$  | -0.09    |         | $\Delta\alpha = -19.82$                                 |
|    |      | $^2P, M_L = 0$             | $69.27 \pm 0.84$  | --       | CCSD(T) |                                                         |
|    |      | $^2P, M_L = \pm 1$         | $49.12 \pm 0.01$  | --       |         |                                                         |
|    |      | $^2P$                      | $55.84 \pm 0.48$  | --       |         | $\Delta\alpha = -20.15$                                 |
|    |      | $^2P, M_L = 0$             | $71.97 \pm 1.38$  | 4.49     | DHF     | <a href="#">2C-SR-CC@dyall.acv4z@(core 13)[vir 363]</a> |
|    |      | $^2P, M_L = \pm 1$         | $53.50 \pm 0.06$  | 9.47     |         |                                                         |
|    |      | $^2P$                      | $59.66 \pm 0.8$   | 7.41     |         | $\Delta\alpha = -18.47$                                 |
|    |      | $^2P, M_L = 0$             | $70.38 \pm 0.32$  | 2.18     | MP2     |                                                         |
|    |      | $^2P, M_L = \pm 1$         | $50.97 \pm 0.09$  | 4.29     |         |                                                         |
|    |      | $^2P$                      | $57.44 \pm 0.2$   | 3.42     |         | $\Delta\alpha = -19.41$                                 |
|    |      | $^2P, M_L = 0$             | $68.62 \pm 0.82$  | -0.38    | CCSD    |                                                         |
|    |      | $^2P, M_L = \pm 1$         | $48.96 \pm 0.01$  | 0.18     |         |                                                         |
|    |      | $^2P$                      | $55.51 \pm 0.48$  | -0.05    |         | $\Delta\alpha = -19.65$                                 |

(continued)

Table S3. continued.

| Z | Atom | State                      | $\alpha_D$ (a.u.)  | $\delta$ | Method  | Comments                                       |
|---|------|----------------------------|--------------------|----------|---------|------------------------------------------------|
|   |      | $^2P, M_L = 0$             | $68.88 \pm 0.75$   | --       | CCSD(T) |                                                |
|   |      | $^2P, M_L = \pm 1$         | $48.87 \pm 0.01$   | --       |         |                                                |
|   |      | $^2P$                      | $55.54 \pm 0.43$   | --       |         | $\Delta\alpha = -20.01$                        |
|   |      | $^2P_{1/2}$                | $62.59 \pm 0.02$   | 8.83     | DHF     | 4C-DC-CC@dyall.acv4z@(core 11)[vir 223]        |
|   |      |                            | $135.51 \pm 32.81$ | 135.64   | MP2     |                                                |
|   |      |                            | 64.03              | 11.34    | CCSD    |                                                |
|   |      |                            | $57.51 \pm 1.75$   | --       | CCSD(T) |                                                |
|   |      | $^2P_{1/2}$                | $64.36 \pm 0.29$   | 23.97    | DHF     | 4C-DC-CC@dyall.acv4z@(core 13)[vir 363]        |
|   |      |                            | $67.80 \pm 12.11$  | 30.59    | MP2     |                                                |
|   |      |                            | $64.09 \pm 0.09$   | 23.44    | CCSD    |                                                |
|   |      |                            | $51.92 \pm 0.54$   | --       | CCSD(T) |                                                |
|   |      | $^2P_{1/2}$                | $57.61 \pm 0.02$   |          | MRCISD  | 4C-DC-CI@dyall.acv4z@(core 13)[vir 223]        |
|   |      | $^2P_{3/2}, M_J = \pm 1/2$ | $66.81 \pm 0.01$   |          |         |                                                |
|   |      | $^2P_{3/2}, M_J = \pm 3/2$ | 49.33              |          |         |                                                |
|   |      | $^2P_{3/2}$                | $58.07 \pm 0.01$   |          |         | $\bar{\alpha}_{J=3/2} - \alpha_{J=1/2} = 0.46$ |
|   |      | $^2P, M_L = 0$             | 81.29              | 10.22    | DHF     | 2C-NR-CC@dyall.acv4z@(core 31)[vir 481]        |
|   |      | $^2P, M_L = \pm 1$         | 47.87              | 13.27    |         |                                                |
|   |      | $^2P$                      | 59.01              | 11.85    |         | $\Delta\alpha = -33.41$                        |
|   |      | $^2P, M_L = 0$             | $62.61 \pm 0.13$   | -15.10   | MP2     |                                                |
|   |      | $^2P, M_L = \pm 1$         | $43.72 \pm 0.4$    | 3.45     |         |                                                |
|   |      | $^2P$                      | $50.02 \pm 0.33$   | -5.19    |         | $\Delta\alpha = -18.89$                        |
|   |      | $^2P, M_L = 0$             | $73.95 \pm 0.01$   | 0.27     | CCSD    |                                                |
|   |      | $^2P, M_L = \pm 1$         | 42.70              | 1.03     |         |                                                |
|   |      | $^2P$                      | $53.12 \pm 0.01$   | 0.67     |         | $\Delta\alpha = -31.25$                        |
|   |      | $^2P, M_L = 0$             | $73.75 \pm 0.09$   | --       | CCSD(T) |                                                |
|   |      | $^2P, M_L = \pm 1$         | 42.26              | --       |         |                                                |
|   |      | $^2P$                      | $52.76 \pm 0.05$   | --       |         | $\Delta\alpha = -31.49$                        |
|   |      | $^2P, M_L = 0$             | 82.78              | 11.92    | DHF     | 2C-SR-CC@dyall.acv4z@(core 13)[vir 203]        |
|   |      | $^2P, M_L = \pm 1$         | 46.72              | 13.89    |         |                                                |
|   |      | $^2P$                      | 58.74              | 12.96    |         | $\Delta\alpha = -36.06$                        |
|   |      | $^2P, M_L = 0$             | $62.09 \pm 1.95$   | -16.06   | MP2     |                                                |
|   |      | $^2P, M_L = \pm 1$         | $42.33 \pm 0.12$   | 3.19     |         |                                                |
|   |      | $^2P$                      | $48.92 \pm 1.13$   | -5.94    |         | $\Delta\alpha = -19.75$                        |
|   |      | $^2P, M_L = 0$             | 74.03              | 0.09     | CCSD    |                                                |
|   |      | $^2P, M_L = \pm 1$         | 41.53              | 1.23     |         |                                                |
|   |      | $^2P$                      | 52.36              | 0.69     |         | $\Delta\alpha = -32.50$                        |
|   |      | $^2P, M_L = 0$             | $73.96 \pm 0.02$   | --       | CCSD(T) |                                                |
|   |      | $^2P, M_L = \pm 1$         | $41.03 \pm 0.1$    | --       |         |                                                |

(continued)



Table S3. continued.

| Z  | Atom | State                      | $\alpha_D$ (a.u.) | $\delta$ | Method  | Comments                                                |
|----|------|----------------------------|-------------------|----------|---------|---------------------------------------------------------|
|    |      | $^2P$                      | $52.00 \pm 0.09$  | --       |         | $\Delta\alpha = -32.94$                                 |
|    |      | $^2P, M_L = 0$             | 82.78             | 10.49    | DHF     | <a href="#">2C-SR-CC@dyall.acv4z@(core 31)[vir 481]</a> |
|    |      | $^2P, M_L = \pm 1$         | 46.72             | 13.98    |         |                                                         |
|    |      | $^2P$                      | 58.74             | 12.31    |         |                                                         |
|    |      | $^2P, M_L = 0$             | $63.55 \pm 0.69$  | -15.18   | MP2     | $\Delta\alpha = -36.06$                                 |
|    |      | $^2P, M_L = \pm 1$         | $40.24 \pm 1.68$  | -1.84    |         |                                                         |
|    |      | $^2P$                      | $48.01 \pm 1.43$  | -8.21    |         | $\Delta\alpha = -23.32$                                 |
|    |      | $^2P, M_L = 0$             | $75.10 \pm 0.01$  | 0.24     | CCSD    |                                                         |
|    |      | $^2P, M_L = \pm 1$         | 41.64             | 1.58     |         |                                                         |
|    |      | $^2P$                      | $52.80 \pm 0.01$  | 0.94     |         | $\Delta\alpha = -33.46$                                 |
|    |      | $^2P, M_L = 0$             | $74.93 \pm 0.06$  | --       | CCSD(T) |                                                         |
|    |      | $^2P, M_L = \pm 1$         | $40.99 \pm 0.15$  | --       |         |                                                         |
|    |      | $^2P$                      | $52.30 \pm 0.13$  | --       |         | $\Delta\alpha = -33.93$                                 |
|    |      | $^2P_{1/2}$                | $57.03 \pm 0.01$  | 11.65    | DHF     | <a href="#">4C-DC-CC@dyall.acv4z@(core 13)[vir 203]</a> |
|    |      |                            | $52.64 \pm 5.18$  | 3.05     | MP2     |                                                         |
|    |      |                            | 52.18             | 2.15     | CCSD    |                                                         |
|    |      |                            | $51.08 \pm 0.32$  | --       | CCSD(T) |                                                         |
|    |      | $^2P_{1/2}$                | 50.66             |          | MRCISD  | <a href="#">4C-DC-CI@dyall.acv4z@(core 13)[vir 203]</a> |
|    |      | $^2P_{3/2}, M_J = \pm 1/2$ | 63.64             |          |         |                                                         |
|    |      | $^2P_{3/2}, M_J = \pm 3/2$ | 42.08             |          |         |                                                         |
|    |      | $^2P_{3/2}$                | 52.86             |          |         | $\bar{\alpha}_{J=3/2} - \alpha_{J=1/2} = 2.20$          |
| 49 | In   | $^2P, M_L = 0$             | 101.26            | 10.11    | DHF     | <a href="#">2C-NR-CC@dyall.acv4z@(core 49)[vir 553]</a> |
|    |      | $^2P, M_L = \pm 1$         | 67.12             | 15.93    |         |                                                         |
|    |      | $^2P$                      | 78.50             | 13.35    |         |                                                         |
|    |      | $^2P, M_L = 0$             | $77.00 \pm 3.7$   | -16.27   | MP2     | $\Delta\alpha = -34.15$                                 |
|    |      | $^2P, M_L = \pm 1$         | $60.30 \pm 0.21$  | 4.16     |         |                                                         |
|    |      | $^2P$                      | $65.87 \pm 2.14$  | -4.89    |         | $\Delta\alpha = -16.70$                                 |
|    |      | $^2P, M_L = 0$             | 92.49             | 0.57     | CCSD    |                                                         |
|    |      | $^2P, M_L = \pm 1$         | 58.49             | 1.03     |         |                                                         |
|    |      | $^2P$                      | 69.82             | 0.82     |         | $\Delta\alpha = -34.00$                                 |
|    |      | $^2P, M_L = 0$             | $91.97 \pm 0.07$  | --       | CCSD(T) |                                                         |
|    |      | $^2P, M_L = \pm 1$         | $57.90 \pm 0.02$  | --       |         |                                                         |
|    |      | $^2P$                      | $69.25 \pm 0.05$  | --       |         | $\Delta\alpha = -34.07$                                 |
|    |      | $^2P, M_L = 0$             | 104.13            | 10.90    | DHF     | <a href="#">2C-SR-CC@dyall.acv4z@(core 31)[vir 309]</a> |
|    |      | $^2P, M_L = \pm 1$         | 62.03             | 15.88    |         |                                                         |
|    |      | $^2P$                      | 76.06             | 13.55    |         |                                                         |
|    |      | $^2P, M_L = 0$             | $80.47 \pm 2.08$  | -14.30   | MP2     | $\Delta\alpha = -42.11$                                 |
|    |      | $^2P, M_L = \pm 1$         | $54.58 \pm 1.48$  | 1.96     |         |                                                         |

(continued)

Table S3. continued.

| Z  | Atom | State                      | $\alpha_D$ (a.u.) | $\delta$ | Method  | Comments                                       |
|----|------|----------------------------|-------------------|----------|---------|------------------------------------------------|
|    |      | $^2P$                      | $63.21 \pm 1.7$   | -5.64    | CCSD    | $\Delta\alpha = -25.90$                        |
|    |      | $^2P, M_L = 0$             | 94.69             | 0.84     |         |                                                |
|    |      | $^2P, M_L = \pm 1$         | 54.08             | 1.04     |         |                                                |
|    |      | $^2P$                      | 67.62             | 0.95     |         | $\Delta\alpha = -40.61$                        |
|    |      | $^2P, M_L = 0$             | $93.90 \pm 0.09$  | --       |         |                                                |
|    |      | $^2P, M_L = \pm 1$         | $53.53 \pm 0.06$  | --       |         |                                                |
|    |      | $^2P$                      | $66.98 \pm 0.07$  | --       | CCSD(T) | $\Delta\alpha = -40.38$                        |
|    |      | $^2P, M_L = 0$             | 104.13            | 10.57    |         | <b>2C-SR-CC@dyall.acv4z@(core 49)[vir 553]</b> |
|    |      | $^2P, M_L = \pm 1$         | 62.03             | 16.44    |         |                                                |
|    |      | $^2P$                      | 76.06             | 13.69    |         | $\Delta\alpha = -42.11$                        |
|    |      | $^2P, M_L = 0$             | $76.83 \pm 4.37$  | -18.42   |         | MP2                                            |
|    |      | $^2P, M_L = \pm 1$         | $59.31 \pm 1.47$  | 11.34    |         |                                                |
|    |      | $^2P$                      | $65.15 \pm 2.79$  | -2.62    |         | $\Delta\alpha = -17.52$                        |
|    |      | $^2P, M_L = 0$             | $94.79 \pm 0.01$  | 0.64     |         | CCSD                                           |
|    |      | $^2P, M_L = \pm 1$         | 54.11             | 1.59     |         |                                                |
|    |      | $^2P$                      | $67.67 \pm 0.01$  | 1.14     |         | $\Delta\alpha = -40.67$                        |
|    |      | $^2P, M_L = 0$             | $94.18 \pm 0.03$  | --       |         | CCSD(T)                                        |
|    |      | $^2P, M_L = \pm 1$         | $53.27 \pm 0.24$  | --       |         |                                                |
|    |      | $^2P$                      | $66.91 \pm 0.2$   | --       |         | $\Delta\alpha = -40.91$                        |
|    |      | $^2P_{1/2}$                | 70.05             | 13.12    | DHF     | <b>2C-DC-CC@dyall.acv4z@(core 31)[vir 309]</b> |
|    |      |                            | 55.88             | -9.76    | MP2     |                                                |
|    |      |                            | 60.17             | -2.83    | CCSD    |                                                |
|    |      |                            | 61.92             | --       | CCSD(T) |                                                |
|    |      | $^2P_{1/2}$                | 62.87             |          | MRCISD  | <b>4C-DC-CI@dyall.acv4z@(core 13)[vir 237]</b> |
|    |      | $^2P_{3/2}, M_J = \pm 1/2$ | 84.75             |          |         |                                                |
|    |      | $^2P_{3/2}, M_J = \pm 3/2$ | 56.36             |          |         |                                                |
|    |      | $^2P_{3/2}$                | 70.55             |          |         | $\bar{\alpha}_{J=3/2} - \alpha_{J=1/2} = 7.68$ |
| 81 | Tl   | $^2P, M_L = 0$             | $86.73 \pm 2.69$  | 1.72     | DHF     | <b>2C-NR-CC@dyall.acv4z@(core 45)[vir 309]</b> |
|    |      | $^2P, M_L = \pm 1$         | $75.12 \pm 0.07$  | 18.73    |         |                                                |
|    |      | $^2P$                      | $78.99 \pm 1.55$  | 11.88    | MP2     | $\Delta\alpha = -11.61$                        |
|    |      | $^2P, M_L = 0$             | $82.26 \pm 2.41$  | -3.53    |         |                                                |
|    |      | $^2P, M_L = \pm 1$         | $66.92 \pm 0.98$  | 5.76     |         |                                                |
|    |      | $^2P$                      | $72.03 \pm 1.6$   | 2.02     |         | $\Delta\alpha = -15.34$                        |
|    |      | $^2P, M_L = 0$             | $84.81 \pm 1.99$  | -0.54    | CCSD    |                                                |
|    |      | $^2P, M_L = \pm 1$         | $64.06 \pm 0.03$  | 1.25     |         |                                                |
|    |      | $^2P$                      | $70.98 \pm 1.15$  | 0.53     | CCSD(T) | $\Delta\alpha = -20.74$                        |
|    |      | $^2P, M_L = 0$             | $85.27 \pm 1.91$  | --       |         |                                                |
|    |      | $^2P, M_L = \pm 1$         | $63.27 \pm 0.01$  | --       |         |                                                |

(continued)

Table S3. continued.

| Z   | Atom | State                      | $\alpha_D$ (a.u.) | $\delta$ | Method  | Comments                                                |
|-----|------|----------------------------|-------------------|----------|---------|---------------------------------------------------------|
|     |      | $^2P$                      | $70.61 \pm 1.1$   | --       |         | $\Delta\alpha = -21.99$                                 |
|     |      | $^2P, M_L = 0$             | $103.65 \pm 1.5$  | 11.76    | DHF     | <a href="#">2C-SR-CC@dyall.acv4z@(core 35)[vir 309]</a> |
|     |      | $^2P, M_L = \pm 1$         | $58.08 \pm 0.1$   | 15.18    |         |                                                         |
|     |      | $^2P$                      | $73.27 \pm 0.87$  | 13.54    |         | $\Delta\alpha = -45.57$                                 |
|     |      | $^2P, M_L = 0$             | $71.19 \pm 4.41$  | -23.24   | MP2     |                                                         |
|     |      | $^2P, M_L = \pm 1$         | $62.26 \pm 1.28$  | 23.47    |         |                                                         |
|     |      | $^2P$                      | $65.24 \pm 2.75$  | 1.09     |         | $\Delta\alpha = -8.93$                                  |
|     |      | $^2P, M_L = 0$             | $93.35 \pm 1.64$  | 0.65     | CCSD    |                                                         |
|     |      | $^2P, M_L = \pm 1$         | $50.59 \pm 0.04$  | 0.33     |         |                                                         |
|     |      | $^2P$                      | $64.84 \pm 0.95$  | 0.48     |         | $\Delta\alpha = -42.76$                                 |
|     |      | $^2P, M_L = 0$             | $92.74 \pm 1.75$  | --       | CCSD(T) |                                                         |
|     |      | $^2P, M_L = \pm 1$         | $50.43 \pm 0.01$  | --       |         |                                                         |
|     |      | $^2P$                      | $64.53 \pm 1.01$  | --       |         | $\Delta\alpha = -42.32$                                 |
|     |      | $^2P, M_L = 0$             | $103.83 \pm 1.43$ | 12.04    | DHF     | <a href="#">2C-SR-CC@dyall.acv4z@(core 45)[vir 309]</a> |
|     |      | $^2P, M_L = \pm 1$         | $58.08 \pm 0.1$   | 15.68    |         |                                                         |
|     |      | $^2P$                      | $73.33 \pm 0.83$  | 13.93    |         | $\Delta\alpha = -45.74$                                 |
|     |      | $^2P, M_L = 0$             | $70.55 \pm 4.14$  | -23.87   | MP2     |                                                         |
|     |      | $^2P, M_L = \pm 1$         | $62.01 \pm 1.18$  | 23.49    |         |                                                         |
|     |      | $^2P$                      | $64.86 \pm 2.57$  | 0.76     |         | $\Delta\alpha = -8.54$                                  |
|     |      | $^2P, M_L = 0$             | $93.03 \pm 1.55$  | 0.38     | CCSD    |                                                         |
|     |      | $^2P, M_L = \pm 1$         | $50.47 \pm 0.03$  | 0.51     |         |                                                         |
|     |      | $^2P$                      | $64.65 \pm 0.9$   | 0.45     |         | $\Delta\alpha = -42.56$                                 |
|     |      | $^2P, M_L = 0$             | $92.67 \pm 1.63$  | --       | CCSD(T) |                                                         |
|     |      | $^2P, M_L = \pm 1$         | $50.21 \pm 0.02$  | --       |         |                                                         |
|     |      | $^2P$                      | $64.37 \pm 0.94$  | --       |         | $\Delta\alpha = -42.46$                                 |
|     |      | $^2P_{1/2}$                | 56.47             | 8.73     | DHF     | 4C-DC-CC@dyall.acv4z@(core 13)[vir 277]                 |
|     |      |                            | $52.81 \pm 2.8$   | 1.69     | MP2     |                                                         |
|     |      |                            | 51.93             | -0.01    | CCSD    |                                                         |
|     |      |                            | $51.94 \pm 0.2$   | --       | CCSD(T) |                                                         |
|     |      | $^2P_{1/2}$                | 56.46             | 10.15    | DHF     | <a href="#">4C-DC-CC@dyall.acv4z@(core 35)[vir 309]</a> |
|     |      |                            | $52.16 \pm 2.5$   | 1.75     | MP2     |                                                         |
|     |      |                            | 51.43             | 0.32     | CCSD    |                                                         |
|     |      |                            | $51.26 \pm 0.13$  | --       | CCSD(T) |                                                         |
|     |      | $^2P_{1/2}$                | 51.26             |          | MRCISD  | <a href="#">4C-DC-CI@dyall.acv4z@(core 13)[vir 277]</a> |
|     |      | $^2P_{3/2}, M_J = \pm 1/2$ | 106.41            |          |         |                                                         |
|     |      | $^2P_{3/2}, M_J = \pm 3/2$ | 57.01             |          |         |                                                         |
|     |      | $^2P_{3/2}$                | 81.71             |          |         |                                                         |
|     |      |                            |                   |          |         | $\bar{\alpha}_{J=3/2} - \alpha_{J=1/2} = 30.45$         |
| 113 | Nh   | $^2P, M_L = 0$             | $114.82 \pm 1.32$ | 9.15     | DHF     | <a href="#">2C-NR-CC@dyall.acv4z@(core 45)[vir 305]</a> |

(continued)

Table S3. continued.

| Z | Atom | State              | $\alpha_D$ (a.u.) | $\delta$ | Method  | Comments                                                      |
|---|------|--------------------|-------------------|----------|---------|---------------------------------------------------------------|
|   |      | $^2P, M_L = \pm 1$ | $96.98 \pm 0.06$  | 20.14    |         |                                                               |
|   |      | $^2P$              | $102.93 \pm 0.76$ | 15.80    |         | $\Delta\alpha = -17.84$                                       |
|   |      | $^2P, M_L = 0$     | $95.85 \pm 2.27$  | -8.88    | MP2     |                                                               |
|   |      | $^2P, M_L = \pm 1$ | $85.05 \pm 1.04$  | 5.36     |         |                                                               |
|   |      | $^2P$              | $88.65 \pm 1.56$  | -0.26    |         | $\Delta\alpha = -10.80$                                       |
|   |      | $^2P, M_L = 0$     | $105.63 \pm 1.21$ | 0.42     | CCSD    |                                                               |
|   |      | $^2P, M_L = \pm 1$ | $81.99 \pm 0.02$  | 1.57     |         |                                                               |
|   |      | $^2P$              | $89.87 \pm 0.7$   | 1.12     |         | $\Delta\alpha = -23.64$                                       |
|   |      | $^2P, M_L = 0$     | $105.19 \pm 1.21$ | --       | CCSD(T) |                                                               |
|   |      | $^2P, M_L = \pm 1$ | $80.72 \pm 0.01$  | --       |         |                                                               |
|   |      | $^2P$              | $88.88 \pm 0.7$   | --       |         | $\Delta\alpha = -24.47$                                       |
|   |      | $^2P, M_L = 0$     | $184.16 \pm 0.01$ | 28.62    | DHF     | <a href="#">2C-SR-CC@dyall.acv4z@(core 35)[vir 305]</a>       |
|   |      | $^2P, M_L = \pm 1$ | 59.88             | 16.61    |         |                                                               |
|   |      | $^2P$              | 101.31            | 23.60    |         | $\Delta\alpha = -124.27$                                      |
|   |      | $^2P, M_L = 0$     | $100.60 \pm 2.47$ | -29.74   | MP2     |                                                               |
|   |      | $^2P, M_L = \pm 1$ | $62.35 \pm 2.18$  | 21.41    |         |                                                               |
|   |      | $^2P$              | $75.10 \pm 2.28$  | -8.38    |         | $\Delta\alpha = -38.24$                                       |
|   |      | $^2P, M_L = 0$     | $146.58 \pm 0.01$ | 2.37     | CCSD    |                                                               |
|   |      | $^2P, M_L = \pm 1$ | 52.16             | 1.56     |         |                                                               |
|   |      | $^2P$              | 83.63             | 2.03     |         | $\Delta\alpha = -94.42$                                       |
|   |      | $^2P, M_L = 0$     | $143.18 \pm 0.19$ | --       | CCSD(T) |                                                               |
|   |      | $^2P, M_L = \pm 1$ | $51.36 \pm 0.02$  | --       |         |                                                               |
|   |      | $^2P$              | $81.96 \pm 0.11$  | --       |         | $\Delta\alpha = -91.82$                                       |
|   |      | $^2P, M_L = 0$     | $184.16 \pm 0.01$ | 29.01    | DHF     | <a href="#">2C-SR-CC@dyall.acv4z@(core 45)[vir 305]</a>       |
|   |      | $^2P, M_L = \pm 1$ | 59.89             | 17.29    |         |                                                               |
|   |      | $^2P$              | 101.31            | 24.12    |         | $\Delta\alpha = -124.27$                                      |
|   |      | $^2P, M_L = 0$     | $99.39 \pm 2.34$  | -30.37   | MP2     |                                                               |
|   |      | $^2P, M_L = \pm 1$ | $59.88 \pm 0.89$  | 17.27    |         |                                                               |
|   |      | $^2P$              | $73.05 \pm 1.53$  | -10.51   |         | $\Delta\alpha = -39.51$                                       |
|   |      | $^2P, M_L = 0$     | $145.77 \pm 0.01$ | 2.12     | CCSD    |                                                               |
|   |      | $^2P, M_L = \pm 1$ | $52.03 \pm 0.01$  | 1.89     |         |                                                               |
|   |      | $^2P$              | $83.27 \pm 0.01$  | 2.02     |         | $\Delta\alpha = -93.74$                                       |
|   |      | $^2P, M_L = 0$     | $142.75 \pm 0.17$ | --       | CCSD(T) |                                                               |
|   |      | $^2P, M_L = \pm 1$ | $51.06 \pm 0.05$  | --       |         |                                                               |
|   |      | $^2P$              | $81.62 \pm 0.11$  | --       |         | $\Delta\alpha = -91.69$                                       |
|   |      | $^2P_{1/2}$        | 32.46             | -0.32    | DHF     | <a href="#">2C-DC-CC@d-aug-dyall.acv4z@(core 51)[vir 449]</a> |
|   |      |                    | 32.19             | -1.15    | MP2     |                                                               |
|   |      |                    | $32.57 \pm 0.02$  | --       | CCSD    |                                                               |

(continued)

Table S3. continued.

| Z | Atom | State                      | $\alpha_D$ (a.u.) | $\delta$ | Method  | Comments                                         |
|---|------|----------------------------|-------------------|----------|---------|--------------------------------------------------|
|   |      | $^2P_{1/2}$                | 32.43             | -1.11    | DHF     | 2C-DC-CC@dyall.acv4z@(core 49)[vir 305]          |
|   |      |                            | 32.18             | -1.88    | MP2     |                                                  |
|   |      |                            | 32.59             | -0.61    | CCSD    |                                                  |
|   |      |                            | 32.79             | --       | CCSD(T) |                                                  |
|   |      | $^2P_{1/2}$                | 32.58             | -1.60    | DHF     | 4C-DC-CC@dyall.acv4z@(core 13)[vir 271]          |
|   |      |                            | $40.46 \pm 4.66$  | 22.22    | MP2     |                                                  |
|   |      |                            | 32.67             | -1.33    | CCSD    |                                                  |
|   |      |                            | $33.11 \pm 0.15$  | --       | CCSD(T) |                                                  |
|   |      | $^2P_{1/2}$                | 32.58             | -0.95    | DHF     | 4C-DC-CC@dyall.acv4z@(core 35)[vir 305]          |
|   |      |                            | $40.48 \pm 4.89$  | 23.07    | MP2     |                                                  |
|   |      |                            | 32.38             | -1.55    | CCSD    |                                                  |
|   |      |                            | $32.89 \pm 0.18$  | --       | CCSD(T) |                                                  |
|   |      | $^2P_{1/2}$                | 28.21             |          | MRCISD  | 4C-DC-CI@dyall.acv4z@(core 13)[vir 271]          |
|   |      | $^2P_{3/2}, M_J = \pm 1/2$ | $188.76 \pm 0.01$ |          |         |                                                  |
|   |      | $^2P_{3/2}, M_J = \pm 3/2$ | 71.21             |          |         |                                                  |
|   |      | $^2P_{3/2}$                | $129.98 \pm 0.01$ |          |         | $\bar{\alpha}_{J=3/2} - \alpha_{J=1/2} = 101.77$ |

## S1.4 Group 14 elements

Table S4: The results of dipole polarizability for Group 14 elements.

| Z | Atom | State              | $\alpha_D$ (a.u.) | $\delta$ (%) | Method  | Comments                               |
|---|------|--------------------|-------------------|--------------|---------|----------------------------------------|
| 6 | C    | $^3P, M_L = 0$     | 9.97              | -3.03        | DHF     | 2C-NR-CC@dyall.acv4z@(core 6)[vir 250] |
|   |      | $^3P, M_L = \pm 1$ | 12.02             | -2.74        |         |                                        |
|   |      | $^3P$              | 11.34             | -2.83        |         |                                        |
|   |      | $^3P, M_L = 0$     | $10.34 \pm 0.03$  | 0.62         | MP2     | $\Delta\alpha = 2.05$                  |
|   |      | $^3P, M_L = \pm 1$ | $11.76 \pm 0.09$  | -4.86        |         |                                        |
|   |      | $^3P$              | $11.29 \pm 0.08$  | -3.25        |         | $\Delta\alpha = 1.41$                  |
|   |      | $^3P, M_L = 0$     | 10.23             | -0.51        | CCSD    |                                        |
|   |      | $^3P, M_L = \pm 1$ | 12.30             | -0.45        |         |                                        |
|   |      | $^3P$              | 11.61             | -0.47        |         | $\Delta\alpha = 2.08$                  |
|   |      | $^3P, M_L = 0$     | 10.28             | --           | CCSD(T) |                                        |
|   |      | $^3P, M_L = \pm 1$ | 12.36             | --           |         |                                        |
|   |      | $^3P$              | 11.66             | --           |         | $\Delta\alpha = 2.08$                  |
|   |      | $^3P, M_L = 0$     | 9.96              | -3.18        | DHF     | 2C-SR-CC@dyall.acv4z@(core 6)[vir 176] |

(continued)

Table S4. continued.

| Z                  | Atom             | State              | $\alpha_D$ (a.u.) | $\delta$           | Method           | Comments                                      |         |                                                |  |
|--------------------|------------------|--------------------|-------------------|--------------------|------------------|-----------------------------------------------|---------|------------------------------------------------|--|
|                    |                  | $^3P, M_L = \pm 1$ | 12.02             | -2.91              | MP2              | $\Delta\alpha = 2.06$                         |         |                                                |  |
|                    |                  | $^3P$              | 11.33             | -2.99              |                  |                                               |         |                                                |  |
|                    |                  | $^3P, M_L = 0$     | $10.39 \pm 0.02$  | 0.99               |                  |                                               |         |                                                |  |
|                    |                  | $^3P, M_L = \pm 1$ | $12.00 \pm 0.05$  | -3.06              | CCSD             | $\Delta\alpha = 1.61$                         |         |                                                |  |
|                    |                  | $^3P$              | $11.46 \pm 0.04$  | -1.87              |                  |                                               |         |                                                |  |
|                    |                  | $^3P, M_L = 0$     | 10.23             | -0.52              |                  |                                               |         |                                                |  |
|                    |                  | $^3P, M_L = \pm 1$ | 12.31             | -0.50              | CCSD(T)          | $\Delta\alpha = 2.08$                         |         |                                                |  |
|                    |                  | $^3P$              | 11.62             | -0.50              |                  |                                               |         |                                                |  |
|                    |                  | $^3P, M_L = 0$     | 10.29             | --                 |                  |                                               |         |                                                |  |
|                    |                  | $^3P, M_L = \pm 1$ | 12.38             | --                 |                  | $\Delta\alpha = 2.09$                         |         |                                                |  |
|                    |                  | $^3P$              | 11.68             | --                 |                  |                                               |         |                                                |  |
|                    |                  | $^3P, M_L = 0$     | 9.96              | -3.15              | DHF              | <b>2C-SR-CC@dyall.acv4z@(core 6)[vir 250]</b> |         |                                                |  |
|                    |                  | $^3P, M_L = \pm 1$ | 12.02             | -2.79              |                  |                                               |         |                                                |  |
|                    |                  | $^3P$              | 11.33             | -2.89              |                  |                                               |         |                                                |  |
|                    |                  | $^3P, M_L = 0$     | $10.72 \pm 0.06$  | 4.25               | MP2              | $\Delta\alpha = 1.10$                         |         |                                                |  |
|                    |                  | $^3P, M_L = \pm 1$ | $11.82 \pm 0.08$  | -4.34              |                  |                                               |         |                                                |  |
|                    |                  | $^3P$              | $11.46 \pm 0.08$  | -1.82              |                  |                                               |         |                                                |  |
|                    |                  | $^3P, M_L = 0$     | 10.22             | -0.63              | CCSD             | $\Delta\alpha = 2.08$                         |         |                                                |  |
|                    |                  | $^3P, M_L = \pm 1$ | 12.30             | -0.48              |                  |                                               |         |                                                |  |
|                    |                  | $^3P$              | 11.61             | -0.53              |                  |                                               |         |                                                |  |
|                    |                  | $^3P, M_L = 0$     | 10.28             | --                 | CCSD(T)          | $\Delta\alpha = 2.08$                         |         |                                                |  |
|                    |                  | $^3P, M_L = \pm 1$ | 12.36             | --                 |                  |                                               |         |                                                |  |
|                    |                  | $^3P$              | 11.67             | --                 |                  |                                               |         |                                                |  |
|                    |                  |                    |                   | $^3P_0$            | 11.75            | 0.24                                          | DHF     | <b>4C-DC-CC@dyall.acv4z@(core 6)[vir 250]</b>  |  |
|                    |                  |                    |                   |                    | 12.04            | 2.67                                          | MP2     |                                                |  |
|                    |                  |                    |                   |                    | 11.62            | -0.87                                         | CCSD    |                                                |  |
|                    |                  |                    |                   |                    | 11.73            | --                                            | CCSD(T) |                                                |  |
|                    |                  | 14                 | Si                | $^3P, M_L = 0$     | 32.89            | 4.16                                          | DHF     | <b>2C-NR-CC@dyall.acv4z@(core 14)[vir 362]</b> |  |
|                    |                  |                    |                   | $^3P, M_L = \pm 1$ | $41.16 \pm 0.02$ | 3.38                                          |         |                                                |  |
|                    |                  |                    |                   | $^3P$              | $38.40 \pm 0.01$ | 3.60                                          |         |                                                |  |
|                    |                  |                    |                   | $^3P, M_L = 0$     | $33.20 \pm 0.01$ | 5.15                                          | MP2     | $\Delta\alpha = 8.27$                          |  |
|                    |                  |                    |                   | $^3P, M_L = \pm 1$ | $39.22 \pm 0.1$  | -1.48                                         |         |                                                |  |
| $^3P$              | $37.21 \pm 0.08$ |                    |                   | 0.40               |                  |                                               |         |                                                |  |
| $^3P, M_L = 0$     | 31.49            |                    |                   | -0.25              | CCSD             | $\Delta\alpha = 6.02$                         |         |                                                |  |
| $^3P, M_L = \pm 1$ | $39.77 \pm 0.02$ |                    |                   | -0.10              |                  |                                               |         |                                                |  |
| $^3P$              | $37.01 \pm 0.01$ |                    |                   | -0.14              |                  |                                               |         |                                                |  |
| $^3P, M_L = 0$     | 31.57            |                    |                   | --                 | CCSD(T)          | $\Delta\alpha = 8.28$                         |         |                                                |  |
| $^3P, M_L = \pm 1$ | $39.81 \pm 0.01$ |                    |                   | --                 |                  |                                               |         |                                                |  |

(continued)

Table S4. continued.

| Z  | Atom | State              | $\alpha_D$ (a.u.) | $\delta$ | Method  | Comments                                                |
|----|------|--------------------|-------------------|----------|---------|---------------------------------------------------------|
|    |      | $^3P$              | $37.07 \pm 0.01$  | --       |         | $\Delta\alpha = 8.24$                                   |
|    |      | $^3P, M_L = 0$     | 32.82             | 4.13     | DHF     | <a href="#">2C-SR-CC@dyall.acv4z@(core 14)[vir 362]</a> |
|    |      | $^3P, M_L = \pm 1$ | $41.23 \pm 0.02$  | 3.33     |         |                                                         |
|    |      | $^3P$              | $38.42 \pm 0.01$  | 3.55     |         | $\Delta\alpha = 8.41$                                   |
|    |      | $^3P, M_L = 0$     | $33.35 \pm 0.06$  | 5.83     | MP2     |                                                         |
|    |      | $^3P, M_L = \pm 1$ | $39.43 \pm 0.1$   | -1.17    |         |                                                         |
|    |      | $^3P$              | $37.41 \pm 0.09$  | 0.81     |         | $\Delta\alpha = 6.08$                                   |
|    |      | $^3P, M_L = 0$     | 31.43             | -0.28    | CCSD    |                                                         |
|    |      | $^3P, M_L = \pm 1$ | $39.85 \pm 0.01$  | -0.12    |         |                                                         |
|    |      | $^3P$              | $37.04 \pm 0.01$  | -0.16    |         | $\Delta\alpha = 8.42$                                   |
|    |      | $^3P, M_L = 0$     | 31.52             | --       | CCSD(T) |                                                         |
|    |      | $^3P, M_L = \pm 1$ | $39.90 \pm 0.01$  | --       |         |                                                         |
|    |      | $^3P$              | $37.10 \pm 0.01$  | --       |         | $\Delta\alpha = 8.38$                                   |
|    |      | $^3P_0$            | 41.70             | 12.69    | DHF     | <a href="#">2C-DC-CC@dyall.acv4z@(core 14)[vir 362]</a> |
|    |      |                    | 40.38             | 9.13     | MP2     |                                                         |
|    |      |                    | 37.56             | 1.51     | CCSD    |                                                         |
|    |      |                    | $37.00 \pm 0.01$  | --       | CCSD(T) |                                                         |
| 32 | Ge   | $^3P, M_L = 0$     | 34.44             | 5.30     | DHF     | <a href="#">2C-NR-CC@dyall.acv4z@(core 32)[vir 480]</a> |
|    |      | $^3P, M_L = \pm 1$ | 44.97             | 4.13     |         |                                                         |
|    |      | $^3P$              | 41.46             | 4.45     |         | $\Delta\alpha = 10.53$                                  |
|    |      | $^3P, M_L = 0$     | $41.04 \pm 4.25$  | 25.46    | MP2     |                                                         |
|    |      | $^3P, M_L = \pm 1$ | $35.70 \pm 4.14$  | -17.33   |         |                                                         |
|    |      | $^3P$              | $37.48 \pm 4.17$  | -5.58    |         | $\Delta\alpha = -5.34$                                  |
|    |      | $^3P, M_L = 0$     | 32.51             | -0.61    | CCSD    |                                                         |
|    |      | $^3P, M_L = \pm 1$ | 43.41             | 0.51     |         |                                                         |
|    |      | $^3P$              | 39.78             | 0.20     |         | $\Delta\alpha = 10.90$                                  |
|    |      | $^3P, M_L = 0$     | $32.71 \pm 0.15$  | --       | CCSD(T) |                                                         |
|    |      | $^3P, M_L = \pm 1$ | $43.19 \pm 0.16$  | --       |         |                                                         |
|    |      | $^3P$              | $39.70 \pm 0.16$  | --       |         | $\Delta\alpha = 10.48$                                  |
|    |      | $^3P, M_L = 0$     | 33.70             | 6.17     | DHF     | <a href="#">2C-SR-CC@dyall.acv4z@(core 22)[vir 246]</a> |
|    |      | $^3P, M_L = \pm 1$ | 45.04             | 3.13     |         |                                                         |
|    |      | $^3P$              | 41.26             | 3.94     |         | $\Delta\alpha = 11.34$                                  |
|    |      | $^3P, M_L = 0$     | $31.94 \pm 1.08$  | 0.63     | MP2     |                                                         |
|    |      | $^3P, M_L = \pm 1$ | $43.41 \pm 0.67$  | -0.62    |         |                                                         |
|    |      | $^3P$              | $39.59 \pm 0.83$  | -0.28    |         | $\Delta\alpha = 11.46$                                  |
|    |      | $^3P, M_L = 0$     | 31.83             | 0.28     | CCSD    |                                                         |
|    |      | $^3P, M_L = \pm 1$ | 43.55             | -0.28    |         |                                                         |
|    |      | $^3P$              | 39.65             | -0.13    |         | $\Delta\alpha = 11.72$                                  |

(continued)

Table S4. continued.

| Z  | Atom | State              | $\alpha_D$ (a.u.) | $\delta$ | Method  | Comments                                       |
|----|------|--------------------|-------------------|----------|---------|------------------------------------------------|
| 50 | Sn   | $^3P, M_L = 0$     | $31.74 \pm 0.02$  | --       | CCSD(T) |                                                |
|    |      | $^3P, M_L = \pm 1$ | $43.68 \pm 0.03$  | --       |         |                                                |
|    |      | $^3P$              | $39.70 \pm 0.03$  | --       |         | $\Delta\alpha = 11.93$                         |
|    |      | $^3P, M_L = 0$     | 33.70             | 6.25     | DHF     | <b>2C-SR-CC@dyall.acv4z@(core 32)[vir 480]</b> |
|    |      | $^3P, M_L = \pm 1$ | 45.04             | 3.71     |         |                                                |
|    |      | $^3P$              | 41.26             | 4.39     |         | $\Delta\alpha = 11.34$                         |
|    |      | $^3P, M_L = 0$     | $33.76 \pm 0.02$  | 6.42     | MP2     |                                                |
|    |      | $^3P, M_L = \pm 1$ | $38.71 \pm 2.22$  | -10.86   |         |                                                |
|    |      | $^3P$              | $37.06 \pm 1.81$  | -6.24    |         | $\Delta\alpha = 4.96$                          |
|    |      | $^3P, M_L = 0$     | 31.80             | 0.27     | CCSD    |                                                |
|    |      | $^3P, M_L = \pm 1$ | 43.52             | 0.19     |         |                                                |
|    |      | $^3P$              | 39.61             | 0.21     |         | $\Delta\alpha = 11.71$                         |
|    |      | $^3P, M_L = 0$     | $31.72 \pm 0.03$  | --       | CCSD(T) |                                                |
|    |      | $^3P, M_L = \pm 1$ | $43.43 \pm 0.08$  | --       |         |                                                |
|    |      | $^3P$              | $39.53 \pm 0.07$  | --       |         | $\Delta\alpha = 11.71$                         |
|    |      | $^3P_0$            | 43.85             | 11.88    | DHF     | <b>2C-DC-CC@dyall.acv4z@(core 22)[vir 246]</b> |
|    |      |                    | 41.36             | 5.54     | MP2     |                                                |
|    |      |                    | $39.91 \pm 0.01$  | 1.85     | CCSD    |                                                |
|    |      |                    | $39.19 \pm 0.02$  | --       | CCSD(T) |                                                |
|    |      | $^3P, M_L = 0$     | 50.99             | 7.37     | DHF     | <b>2C-NR-CC@dyall.acv4z@(core 50)[vir 552]</b> |
|    |      | $^3P, M_L = \pm 1$ | 62.62             | 5.28     |         |                                                |
|    |      | $^3P$              | 58.74             | 5.87     |         | $\Delta\alpha = 11.63$                         |
|    |      | $^3P, M_L = 0$     | $59.65 \pm 6.65$  | 25.62    | MP2     |                                                |
|    |      | $^3P, M_L = \pm 1$ | $56.69 \pm 0.52$  | -4.69    |         |                                                |
|    |      | $^3P$              | $57.68 \pm 3.86$  | 3.96     |         | $\Delta\alpha = -2.96$                         |
|    |      | $^3P, M_L = 0$     | 47.25             | -0.49    | CCSD    |                                                |
|    |      | $^3P, M_L = \pm 1$ | 59.77             | 0.49     |         |                                                |
|    |      | $^3P$              | 55.60             | 0.21     |         | $\Delta\alpha = 12.52$                         |
|    |      | $^3P, M_L = 0$     | $47.49 \pm 0.22$  | --       | CCSD(T) |                                                |
|    |      | $^3P, M_L = \pm 1$ | $59.48 \pm 0.09$  | --       |         |                                                |
|    |      | $^3P$              | $55.48 \pm 0.15$  | --       |         | $\Delta\alpha = 12.00$                         |
|    |      | $^3P, M_L = 0$     | 47.70             | 8.09     | DHF     | <b>2C-SR-CC@dyall.acv4z@(core 32)[vir 302]</b> |
|    |      | $^3P, M_L = \pm 1$ | 62.03             | 4.45     |         |                                                |
|    |      | $^3P$              | 57.25             | 5.44     |         | $\Delta\alpha = 14.33$                         |
|    |      | $^3P, M_L = 0$     | $47.07 \pm 0.04$  | 6.67     | MP2     |                                                |
|    |      | $^3P, M_L = \pm 1$ | $61.06 \pm 2.45$  | 2.82     |         |                                                |
|    |      | $^3P$              | $56.40 \pm 2.0$   | 3.86     |         | $\Delta\alpha = 13.99$                         |
|    |      | $^3P, M_L = 0$     | 44.26             | 0.30     | CCSD    |                                                |

(continued)



Table S4. continued.

| Z                  | Atom             | State              | $\alpha_D$ (a.u.) | $\delta$       | Method                 | Comments                                       |                                                |
|--------------------|------------------|--------------------|-------------------|----------------|------------------------|------------------------------------------------|------------------------------------------------|
|                    |                  | $^3P, M_L = \pm 1$ | 59.49             | 0.17           | CCSD(T)                | $\Delta\alpha = 15.23$                         |                                                |
|                    |                  | $^3P$              | 54.41             | 0.21           |                        |                                                |                                                |
|                    |                  | $^3P, M_L = 0$     | $44.13 \pm 0.06$  | --             |                        |                                                |                                                |
|                    |                  | $^3P, M_L = \pm 1$ | $59.39 \pm 0.01$  | --             |                        |                                                |                                                |
|                    |                  | $^3P$              | $54.30 \pm 0.04$  | --             |                        |                                                | $\Delta\alpha = 15.26$                         |
|                    |                  | $^3P, M_L = 0$     | 47.70             | 7.70           | DHF                    | <b>2C-SR-CC@dyall.acv4z@(core 50)[vir 552]</b> |                                                |
|                    |                  | $^3P, M_L = \pm 1$ | 62.03             | 4.92           | MP2                    | $\Delta\alpha = 14.33$                         |                                                |
|                    |                  | $^3P$              | 57.25             | 5.68           |                        |                                                |                                                |
|                    |                  | $^3P, M_L = 0$     | $49.91 \pm 1.82$  | 12.69          |                        |                                                |                                                |
|                    |                  | $^3P, M_L = \pm 1$ | $50.69 \pm 4.07$  | -14.27         |                        |                                                |                                                |
|                    |                  | $^3P$              | $50.43 \pm 3.48$  | -6.92          |                        |                                                | $\Delta\alpha = 0.78$                          |
|                    |                  | $^3P, M_L = 0$     | 44.25             | -0.09          | CCSD                   | $\Delta\alpha = 15.23$                         |                                                |
|                    |                  | $^3P, M_L = \pm 1$ | 59.48             | 0.60           |                        |                                                |                                                |
|                    |                  | $^3P$              | 54.40             | 0.41           |                        |                                                |                                                |
|                    |                  | $^3P, M_L = 0$     | $44.29 \pm 0.04$  | --             | CCSD(T)                |                                                |                                                |
|                    |                  | $^3P, M_L = \pm 1$ | $59.12 \pm 0.16$  | --             | $\Delta\alpha = 14.83$ |                                                |                                                |
|                    |                  | $^3P$              | $54.18 \pm 0.13$  | --             |                        |                                                |                                                |
|                    |                  | $^3P_0$            | 57.33             | 10.33          |                        | DHF                                            | <b>2C-DC-CC@dyall.acv4z@(core 32)[vir 302]</b> |
|                    |                  |                    | 53.12             | 2.24           |                        | MP2                                            |                                                |
|                    |                  |                    | 52.62             | 1.27           |                        | CCSD                                           |                                                |
|                    |                  |                    | 51.96             | --             | CCSD(T)                |                                                |                                                |
|                    |                  | 82                 | Pb                | $^3P, M_L = 0$ | 58.41                  | 9.25                                           | DHF                                            |
| $^3P, M_L = \pm 1$ | $70.01 \pm 0.15$ |                    |                   | 5.17           | MP2                    | $\Delta\alpha = 11.59$                         |                                                |
| $^3P$              | $66.14 \pm 0.13$ |                    |                   | 6.34           |                        |                                                |                                                |
| $^3P, M_L = 0$     | $54.90 \pm 0.15$ |                    |                   | 2.68           |                        |                                                |                                                |
| $^3P, M_L = \pm 1$ | $64.05 \pm 0.06$ |                    |                   | -3.77          |                        |                                                |                                                |
| $^3P$              | $61.00 \pm 0.1$  |                    |                   | -1.92          |                        |                                                | $\Delta\alpha = 9.15$                          |
| $^3P, M_L = 0$     | 53.71            |                    |                   | 0.46           | CCSD                   | $\Delta\alpha = 12.99$                         |                                                |
| $^3P, M_L = \pm 1$ | $66.70 \pm 0.12$ |                    |                   | 0.21           | CCSD(T)                |                                                |                                                |
| $^3P$              | $62.37 \pm 0.1$  |                    |                   | 0.28           |                        |                                                |                                                |
| $^3P, M_L = 0$     | $53.47 \pm 0.01$ |                    |                   | --             |                        |                                                |                                                |
| $^3P, M_L = \pm 1$ | $66.56 \pm 0.11$ |                    |                   | --             |                        |                                                |                                                |
| $^3P$              | $62.20 \pm 0.09$ |                    |                   | --             | $\Delta\alpha = 13.10$ |                                                |                                                |
| $^3P, M_L = 0$     | 47.45            |                    |                   | 8.24           | DHF                    | <b>2C-SR-CC@dyall.acv4z@(core 46)[vir 308]</b> |                                                |
| $^3P, M_L = \pm 1$ | $68.58 \pm 0.19$ |                    |                   | 4.21           | MP2                    | $\Delta\alpha = 21.12$                         |                                                |
| $^3P$              | $61.54 \pm 0.16$ |                    |                   | 5.21           |                        |                                                |                                                |
| $^3P, M_L = 0$     | $47.10 \pm 0.1$  |                    |                   | 7.43           |                        |                                                |                                                |
| $^3P, M_L = \pm 1$ | $62.75 \pm 0.06$ |                    |                   | -4.65          |                        |                                                |                                                |
|                    |                  |                    |                   |                |                        |                                                |                                                |

(continued)

Table S4. continued.

| Z   | Atom | State              | $\alpha_D$ (a.u.) | $\delta$ | Method                        | Comments                                       |
|-----|------|--------------------|-------------------|----------|-------------------------------|------------------------------------------------|
| 114 | Fl   | $^3P$              | $57.53 \pm 0.08$  | -1.63    | CCSD                          | $\Delta\alpha = 15.65$                         |
|     |      | $^3P, M_L = 0$     | $43.90 \pm 0.01$  | 0.13     |                               |                                                |
|     |      | $^3P, M_L = \pm 1$ | $65.81 \pm 0.13$  | -0.00    |                               |                                                |
|     |      | $^3P$              | $58.51 \pm 0.11$  | 0.03     |                               | $\Delta\alpha = 21.91$                         |
|     |      | $^3P, M_L = 0$     | $43.84 \pm 0.01$  | --       |                               |                                                |
|     |      | $^3P, M_L = \pm 1$ | $65.81 \pm 0.12$  | --       |                               |                                                |
|     |      | $^3P$              | $58.49 \pm 0.1$   | --       | DHF<br>MP2<br>CCSD<br>CCSD(T) | $\Delta\alpha = 21.97$                         |
|     |      | $^3P_0$            | 49.43             | 6.25     |                               | <b>2C-DC-CC@dyall.acv4z@(core 46)[vir 308]</b> |
|     |      |                    | 46.55             | 0.05     |                               |                                                |
|     |      |                    | 46.55             | 0.06     |                               |                                                |
|     |      |                    | 46.53             | --       |                               |                                                |
|     |      | $^3P, M_L = 0$     | $76.60 \pm 0.01$  | 10.65    | DHF                           | <b>2C-NR-CC@dyall.acv4z@(core 52)[vir 302]</b> |
|     |      | $^3P, M_L = \pm 1$ | $87.45 \pm 0.22$  | 6.31     |                               |                                                |
|     |      | $^3P$              | $83.83 \pm 0.18$  | 7.59     | MP2                           | $\Delta\alpha = 10.86$                         |
|     |      | $^3P, M_L = 0$     | $69.93 \pm 0.12$  | 1.03     |                               |                                                |
|     |      | $^3P, M_L = \pm 1$ | $77.81 \pm 0.11$  | -5.42    | CCSD                          |                                                |
|     |      | $^3P$              | $75.18 \pm 0.11$  | -3.51    |                               | $\Delta\alpha = 7.87$                          |
|     |      | $^3P, M_L = 0$     | 69.75             | 0.76     | CCSD(T)                       |                                                |
|     |      | $^3P, M_L = \pm 1$ | $82.64 \pm 0.16$  | 0.46     |                               |                                                |
|     |      | $^3P$              | $78.34 \pm 0.13$  | 0.55     | CCSD(T)                       | $\Delta\alpha = 12.90$                         |
|     |      | $^3P, M_L = 0$     | $69.22 \pm 0.01$  | --       |                               |                                                |
|     |      | $^3P, M_L = \pm 1$ | $82.27 \pm 0.16$  | --       | DHF                           |                                                |
|     |      | $^3P$              | $77.92 \pm 0.13$  | --       |                               | $\Delta\alpha = 13.04$                         |
|     |      | $^3P, M_L = 0$     | $50.51 \pm 0.02$  | 9.18     | DHF                           | 2C-SR-CC@dyall.acv4z@(core 46)[vir 302]        |
|     |      | $^3P, M_L = \pm 1$ | $94.26 \pm 0.26$  | 10.29    |                               |                                                |
|     |      | $^3P$              | $79.67 \pm 0.21$  | 10.05    | MP2                           | $\Delta\alpha = 43.75$                         |
|     |      | $^3P, M_L = 0$     | $53.40 \pm 0.04$  | 15.43    |                               |                                                |
|     |      | $^3P, M_L = \pm 1$ | $77.00 \pm 0.17$  | -9.90    | CCSD                          |                                                |
|     |      | $^3P$              | $69.13 \pm 0.14$  | -4.51    |                               | $\Delta\alpha = 23.60$                         |
|     |      | $^3P, M_L = 0$     | $46.47 \pm 0.01$  | 0.46     | CCSD(T)                       |                                                |
|     |      | $^3P, M_L = \pm 1$ | $85.93 \pm 0.17$  | 0.55     |                               |                                                |
|     |      | $^3P$              | $72.78 \pm 0.14$  | 0.53     | CCSD(T)                       | $\Delta\alpha = 39.46$                         |
|     |      | $^3P, M_L = 0$     | $46.26 \pm 0.01$  | --       |                               |                                                |
|     |      | $^3P, M_L = \pm 1$ | $85.46 \pm 0.17$  | --       | DHF                           |                                                |
|     |      | $^3P$              | $72.39 \pm 0.14$  | --       |                               | $\Delta\alpha = 39.20$                         |
|     |      | $^3P, M_L = 0$     | $50.51 \pm 0.02$  | 9.04     | DHF                           | <b>2C-SR-CC@dyall.acv4z@(core 52)[vir 302]</b> |
|     |      | $^3P, M_L = \pm 1$ | $94.23 \pm 0.28$  | 10.01    |                               |                                                |
|     |      | $^3P$              | $79.66 \pm 0.23$  | 9.81     |                               | $\Delta\alpha = 43.73$                         |

(continued)

Table S4. continued.

| Z | Atom | State              | $\alpha_D$ (a.u.) | $\delta$ | Method  | Comments                                       |
|---|------|--------------------|-------------------|----------|---------|------------------------------------------------|
|   |      | $^3P, M_L = 0$     | $53.52 \pm 0.04$  | 15.54    | MP2     |                                                |
|   |      | $^3P, M_L = \pm 1$ | $77.26 \pm 0.18$  | -9.81    |         |                                                |
|   |      | $^3P$              | $69.35 \pm 0.15$  | -4.41    |         | $\Delta\alpha = 23.74$                         |
|   |      | $^3P, M_L = 0$     | $46.56 \pm 0.01$  | 0.52     | CCSD    |                                                |
|   |      | $^3P, M_L = \pm 1$ | $86.11 \pm 0.19$  | 0.53     |         |                                                |
|   |      | $^3P$              | $72.93 \pm 0.15$  | 0.53     |         | $\Delta\alpha = 39.55$                         |
|   |      | $^3P, M_L = 0$     | $46.32 \pm 0.01$  | --       | CCSD(T) |                                                |
|   |      | $^3P, M_L = \pm 1$ | $85.66 \pm 0.18$  | --       |         |                                                |
|   |      | $^3P$              | $72.54 \pm 0.15$  | --       |         | $\Delta\alpha = 39.34$                         |
|   |      | $^3P_0$            | 29.88             | -2.88    | DHF     | <b>2C-DC-CC@dyall.acv4z@(core 50)[vir 302]</b> |
|   |      |                    | 31.39             | 2.03     | MP2     |                                                |
|   |      |                    | 30.39             | -1.24    | CCSD    |                                                |
|   |      |                    | 30.77             | --       | CCSD(T) |                                                |

## S1.5 Group 15 elements

Table S5: The results of dipole polarizability for Group 15 elements.

| Z | Atom | State                      | $\alpha_D$ (a.u.) | $\delta$ (%) | Method  | Comments                                      |
|---|------|----------------------------|-------------------|--------------|---------|-----------------------------------------------|
| 7 | N    | $^4S, M_L = 0$             | 6.79              | -6.27        | DHF     | <b>2C-NR-CC@dyall.acv4z@(core 7)[vir 249]</b> |
|   |      |                            | 7.11              | -1.91        | MP2     |                                               |
|   |      |                            | 7.19              | -0.80        | CCSD    |                                               |
|   |      |                            | 7.25              | --           | CCSD(T) |                                               |
|   |      | $^4S, M_L = 0$             | 6.79              | -6.70        | DHF     | <b>2C-SR-CC@dyall.acv4z@(core 7)[vir 159]</b> |
|   |      |                            | 7.14              | -1.92        | MP2     |                                               |
|   |      |                            | 7.22              | -0.78        | CCSD    |                                               |
|   |      |                            | 7.27              | --           | CCSD(T) |                                               |
|   |      | $^4S, M_L = 0$             | 6.79              | -6.28        | DHF     | <b>2C-SR-CC@dyall.acv4z@(core 7)[vir 249]</b> |
|   |      |                            | 7.10              | -1.90        | MP2     |                                               |
|   |      |                            | 7.18              | -0.80        | CCSD    |                                               |
|   |      |                            | 7.24              | --           | CCSD(T) |                                               |
|   |      | $^4S_{3/2}, M_J = \pm 1/2$ | 7.20              |              | MRCISD  | <b>4C-DC-CI@dyall.acv4z@(core 7)[vir 159]</b> |
|   |      | $^4S_{3/2}, M_J = \pm 3/2$ | 7.20              |              |         |                                               |
|   |      | $^4S_{3/2}$                | 7.20              |              |         |                                               |

(continued)

Table S5. continued.

| Z  | Atom | State                      | $\alpha_D$ (a.u.) | $\delta$ | Method  | Comments                                       |
|----|------|----------------------------|-------------------|----------|---------|------------------------------------------------|
| 15 | P    | $^4S, M_L = 0$             | 24.95             | 0.12     | DHF     | <b>2C-NR-CC@dyall.acv4z@(core 15)[vir 361]</b> |
|    |      |                            | 24.83             | -0.34    | MP2     |                                                |
|    |      |                            | 24.85             | -0.28    | CCSD    |                                                |
|    |      |                            | 24.92             | --       | CCSD(T) |                                                |
|    |      | $^4S, M_L = 0$             | 24.95             | -0.80    | DHF     | <b>2C-SR-CC@dyall.acv4z@(core 15)[vir 185]</b> |
|    |      |                            | 25.10             | -0.22    | MP2     |                                                |
|    |      |                            | 25.08             | -0.29    | CCSD    |                                                |
|    |      |                            | 25.16             | --       | CCSD(T) |                                                |
|    |      | $^4S, M_L = 0$             | 24.96             | 0.08     | DHF     | <b>2C-SR-CC@dyall.acv4z@(core 15)[vir 361]</b> |
|    |      |                            | 24.86             | -0.32    | MP2     |                                                |
|    |      |                            | 24.86             | -0.28    | CCSD    |                                                |
|    |      |                            | 24.93             | --       | CCSD(T) |                                                |
|    |      | $^4S_{3/2}, M_J = \pm 1/2$ | 24.83             |          | MRCISD  | <b>4C-DC-CI@dyall.acv4z@(core 15)[vir 185]</b> |
|    |      | $^4S_{3/2}, M_J = \pm 3/2$ | 24.83             |          |         |                                                |
|    |      | $^4S_{3/2}$                | 24.83             |          |         |                                                |
| 33 | As   | $^4S, M_L = 0$             | 30.00             | 0.55     | DHF     | <b>2C-NR-CC@dyall.acv4z@(core 33)[vir 479]</b> |
|    |      |                            | $29.86 \pm 0.21$  | 0.09     | MP2     |                                                |
|    |      |                            | 29.76             | -0.24    | CCSD    |                                                |
|    |      |                            | $29.83 \pm 0.01$  | --       | CCSD(T) |                                                |
|    |      | $^4S, M_L = 0$             | 29.82             | 0.68     | DHF     | <b>2C-SR-CC@dyall.acv4z@(core 15)[vir 185]</b> |
|    |      |                            | $29.70 \pm 0.21$  | 0.28     | MP2     |                                                |
|    |      |                            | 29.53             | -0.31    | CCSD    |                                                |
|    |      |                            | $29.62 \pm 0.01$  | --       | CCSD(T) |                                                |
|    |      | $^4S, M_L = 0$             | 29.82             | 0.41     | DHF     | <b>2C-SR-CC@dyall.acv4z@(core 33)[vir 479]</b> |
|    |      |                            | $29.74 \pm 0.21$  | 0.12     | MP2     |                                                |
|    |      |                            | 29.62             | -0.25    | CCSD    |                                                |
|    |      |                            | $29.70 \pm 0.01$  | --       | CCSD(T) |                                                |
|    |      | $^4S_{3/2}, M_J = \pm 1/2$ | 29.00             |          | MRCISD  | <b>4C-DC-CI@dyall.acv4z@(core 15)[vir 185]</b> |
|    |      | $^4S_{3/2}, M_J = \pm 3/2$ | 28.96             |          |         |                                                |
|    |      | $^4S_{3/2}$                | 28.98             |          |         |                                                |
| 51 | Sb   | $^4S, M_L = 0$             | 44.76             | 2.25     | DHF     | <b>2C-NR-CC@dyall.acv4z@(core 51)[vir 551]</b> |
|    |      |                            | $43.23 \pm 0.14$  | -1.26    | MP2     |                                                |
|    |      |                            | $43.79 \pm 0.01$  | 0.02     | CCSD    |                                                |
|    |      |                            | $43.78 \pm 0.01$  | --       | CCSD(T) |                                                |
|    |      | $^4S, M_L = 0$             | 43.68             | 1.44     | DHF     | <b>2C-SR-CC@dyall.acv4z@(core 15)[vir 227]</b> |
|    |      |                            | $42.79 \pm 0.14$  | -0.62    | MP2     |                                                |
|    |      |                            | 43.01             | -0.11    | CCSD    |                                                |
|    |      |                            | 43.05             | --       | CCSD(T) |                                                |

(continued)

Table S5. continued.

| Z   | Atom | State                      | $\alpha_D$ (a.u.) | $\delta$ | Method  | Comments                                                |
|-----|------|----------------------------|-------------------|----------|---------|---------------------------------------------------------|
|     |      | $^4S, M_L = 0$             | 43.68             | 1.66     | DHF     | <a href="#">2C-SR-CC@dyall.acv4z@(core 51)[vir 551]</a> |
|     |      |                            | $42.59 \pm 0.14$  | -0.88    | MP2     |                                                         |
|     |      |                            | $42.94 \pm 0.01$  | -0.06    | CCSD    |                                                         |
|     |      |                            | $42.96 \pm 0.01$  | --       | CCSD(T) |                                                         |
|     |      | $^4S_{3/2}, M_J = \pm 1/2$ | 42.22             |          | MRCISD  | <a href="#">4C-DC-CI@dyall.acv4z@(core 15)[vir 227]</a> |
|     |      | $^4S_{3/2}, M_J = \pm 3/2$ | 41.73             |          |         |                                                         |
|     |      | $^4S_{3/2}$                | 41.98             |          |         |                                                         |
|     |      |                            |                   |          |         |                                                         |
|     |      |                            |                   |          |         |                                                         |
|     |      |                            |                   |          |         |                                                         |
| 83  | Bi   | $^4S, M_L = 0$             | $52.60 \pm 0.01$  | 2.77     | DHF     | <a href="#">2C-NR-CC@dyall.acv4z@(core 47)[vir 307]</a> |
|     |      |                            | $50.14 \pm 0.01$  | -2.03    | MP2     |                                                         |
|     |      |                            | $51.21 \pm 0.01$  | 0.06     | CCSD    |                                                         |
|     |      |                            | $51.18 \pm 0.01$  | --       | CCSD(T) |                                                         |
|     |      | $^4S, M_L = 0$             | $49.35 \pm 0.01$  | 1.17     | DHF     | <a href="#">2C-SR-CC@dyall.acv4z@(core 15)[vir 265]</a> |
|     |      |                            | $48.19 \pm 0.01$  | -1.21    | MP2     |                                                         |
|     |      |                            | $48.71 \pm 0.01$  | -0.14    | CCSD    |                                                         |
|     |      |                            | $48.78 \pm 0.01$  | --       | CCSD(T) |                                                         |
|     |      | $^4S, M_L = 0$             | $49.35 \pm 0.01$  | 1.54     | DHF     | <a href="#">2C-SR-CC@dyall.acv4z@(core 47)[vir 307]</a> |
|     |      |                            | $47.81 \pm 0.01$  | -1.63    | MP2     |                                                         |
|     |      |                            | $48.54 \pm 0.01$  | -0.12    | CCSD    |                                                         |
|     |      |                            | $48.60 \pm 0.01$  | --       | CCSD(T) |                                                         |
|     |      | $^4S_{3/2}, M_J = \pm 1/2$ | 51.42             |          | MRCISD  | <a href="#">4C-DC-CI@dyall.acv4z@(core 15)[vir 265]</a> |
|     |      | $^4S_{3/2}, M_J = \pm 3/2$ | 41.71             |          |         |                                                         |
|     |      | $^4S_{3/2}$                | 46.57             |          |         |                                                         |
|     |      |                            |                   |          |         |                                                         |
|     |      |                            |                   |          |         |                                                         |
|     |      |                            |                   |          |         |                                                         |
|     |      |                            |                   |          |         |                                                         |
|     |      |                            |                   |          |         |                                                         |
|     |      |                            |                   |          |         |                                                         |
| 115 | Mc   | $^4S, M_L = 0$             | $66.00 \pm 0.03$  | 3.72     | DHF     | <a href="#">2C-NR-CC@dyall.acv4z@(core 47)[vir 303]</a> |
|     |      |                            | $61.58 \pm 0.02$  | -3.23    | MP2     |                                                         |
|     |      |                            | $63.82 \pm 0.03$  | 0.29     | CCSD    |                                                         |
|     |      |                            | $63.63 \pm 0.03$  | --       | CCSD(T) |                                                         |
|     |      | $^4S, M_L = 0$             | $63.43 \pm 0.05$  | 4.05     | DHF     | <a href="#">2C-SR-CC@dyall.acv4z@(core 15)[vir 265]</a> |
|     |      |                            | $57.69 \pm 0.21$  | -5.37    | MP2     |                                                         |
|     |      |                            | $61.12 \pm 0.03$  | 0.27     | CCSD    |                                                         |
|     |      |                            | $60.96 \pm 0.03$  | --       | CCSD(T) |                                                         |
|     |      | $^4S, M_L = 0$             | $63.43 \pm 0.04$  | 4.59     | DHF     | <a href="#">2C-SR-CC@dyall.acv4z@(core 47)[vir 303]</a> |
|     |      |                            | $56.95 \pm 0.22$  | -6.10    | MP2     |                                                         |
|     |      |                            | $60.80 \pm 0.03$  | 0.25     | CCSD    |                                                         |
|     |      |                            | $60.65 \pm 0.03$  | --       | CCSD(T) |                                                         |
|     |      | $^4S_{3/2}, M_J = \pm 1/2$ | 97.20             |          | MRCISD  | <a href="#">4C-DC-CI@dyall.acv4z@(core 15)[vir 265]</a> |
|     |      | $^4S_{3/2}, M_J = \pm 3/2$ | 40.07             |          |         |                                                         |
|     |      | $^4S_{3/2}$                | 68.64             |          |         |                                                         |

## S1.6 Group 16 elements

Table S6: The results of dipole polarizability for Group 16 elements.

| Z | Atom | State              | $\alpha_D$ (a.u.) | $\delta$ (%) | Method  | Comments                                               |
|---|------|--------------------|-------------------|--------------|---------|--------------------------------------------------------|
| 8 | O    | $^3P, M_L = 0$     | 4.90              | -14.82       | DHF     | <a href="#">2C-NR-CC@dyall.acv4z@(core 8)[vir 248]</a> |
|   |      | $^3P, M_L = \pm 1$ | 4.44              | -8.65        |         |                                                        |
|   |      | $^3P$              | 4.59              | -10.94       |         |                                                        |
|   |      | $^3P, M_L = 0$     | $5.10 \pm 0.06$   | -11.29       | MP2     | $\Delta\alpha = -0.46$                                 |
|   |      | $^3P, M_L = \pm 1$ | 4.79              | -1.49        |         |                                                        |
|   |      | $^3P$              | $4.89 \pm 0.04$   | -5.13        |         | $\Delta\alpha = -0.31$                                 |
|   |      | $^3P, M_L = 0$     | 5.63              | -2.01        | CCSD    |                                                        |
|   |      | $^3P, M_L = \pm 1$ | 4.80              | -1.28        |         |                                                        |
|   |      | $^3P$              | 5.08              | -1.55        |         | $\Delta\alpha = -0.83$                                 |
|   |      | $^3P, M_L = 0$     | 5.75              | --           | CCSD(T) |                                                        |
|   |      | $^3P, M_L = \pm 1$ | 4.86              | --           |         |                                                        |
|   |      | $^3P$              | 5.16              | --           |         | $\Delta\alpha = -0.89$                                 |
|   |      | $^3P, M_L = 0$     | 4.90              | -14.91       | DHF     | <a href="#">2C-SR-CC@dyall.acv4z@(core 8)[vir 186]</a> |
|   |      | $^3P, M_L = \pm 1$ | 4.44              | -8.63        |         |                                                        |
|   |      | $^3P$              | 4.59              | -10.97       |         |                                                        |
|   |      | $^3P, M_L = 0$     | $5.45 \pm 0.02$   | -5.35        | MP2     | $\Delta\alpha = -0.47$                                 |
|   |      | $^3P, M_L = \pm 1$ | $4.73 \pm 0.01$   | -2.68        |         |                                                        |
|   |      | $^3P$              | $4.97 \pm 0.01$   | -3.67        |         | $\Delta\alpha = -0.73$                                 |
|   |      | $^3P, M_L = 0$     | 5.64              | -2.13        | CCSD    |                                                        |
|   |      | $^3P, M_L = \pm 1$ | 4.80              | -1.22        |         |                                                        |
|   |      | $^3P$              | 5.08              | -1.56        |         | $\Delta\alpha = -0.84$                                 |
|   |      | $^3P, M_L = 0$     | 5.76              | --           | CCSD(T) |                                                        |
|   |      | $^3P, M_L = \pm 1$ | 4.86              | --           |         |                                                        |
|   |      | $^3P$              | 5.16              | --           |         | $\Delta\alpha = -0.91$                                 |
|   |      | $^3P, M_L = 0$     | 4.90              | -14.91       | DHF     | <a href="#">2C-SR-CC@dyall.acv4z@(core 8)[vir 248]</a> |
|   |      | $^3P, M_L = \pm 1$ | 4.44              | -8.53        |         |                                                        |
|   |      | $^3P$              | 4.59              | -10.91       |         |                                                        |
|   |      | $^3P, M_L = 0$     | $5.20 \pm 0.04$   | -9.81        | MP2     | $\Delta\alpha = -0.47$                                 |
|   |      | $^3P, M_L = \pm 1$ | $4.48 \pm 0.07$   | -7.69        |         |                                                        |
|   |      | $^3P$              | $4.72 \pm 0.06$   | -8.48        |         | $\Delta\alpha = -0.72$                                 |
|   |      | $^3P, M_L = 0$     | 5.64              | -2.09        | CCSD    |                                                        |
|   |      | $^3P, M_L = \pm 1$ | 4.80              | -1.13        |         |                                                        |
|   |      | $^3P$              | 5.08              | -1.49        |         | $\Delta\alpha = -0.84$                                 |

(continued)

Table S6. continued.

| Z | Atom | State                | $\alpha_D$ (a.u.) | $\delta$ | Method  | Comments                                                |
|---|------|----------------------|-------------------|----------|---------|---------------------------------------------------------|
|   |      | $^3P, M_L = 0$       | 5.76              | --       | CCSD(T) |                                                         |
|   |      | $^3P, M_L = \pm 1$   | 4.85              | --       |         |                                                         |
|   |      | $^3P$                | 5.15              | --       |         | $\Delta\alpha = -0.91$                                  |
|   |      | $^3P_2, M_J = 0$     | 5.41              |          | MRCISD  | <a href="#">4C-DC-CI@dyall.acv4z@(core 8)[vir 116]</a>  |
|   |      | $^3P_2, M_J = \pm 1$ | 4.84              |          |         |                                                         |
|   |      | $^3P_2, M_J = \pm 2$ | 5.27              |          |         |                                                         |
|   |      | $^3P_2$              | 5.13              |          |         |                                                         |
|   |      | $^3P_2, M_J = 0$     | 5.24              |          | MRCISD  | 4C-DC-CI@dyall.acv4z@(core 8)[vir 186]                  |
|   |      | $^3P_2, M_J = \pm 1$ | 4.74              |          |         |                                                         |
|   |      | $^3P_2, M_J = \pm 2$ | 5.12              |          |         |                                                         |
|   |      | $^3P_2$              | 4.99              |          |         |                                                         |
|   | 16   | $^3P, M_L = 0$       | 20.97             | -2.55    | DHF     | <a href="#">2C-NR-CC@dyall.acv4z@(core 16)[vir 360]</a> |
|   |      | $^3P, M_L = \pm 1$   | 17.89             | -0.53    |         |                                                         |
|   |      | $^3P$                | 18.92             | -1.29    |         | $\Delta\alpha = -3.08$                                  |
|   |      | $^3P, M_L = 0$       | $11.19 \pm 1.69$  | -48.00   | MP2     |                                                         |
|   |      | $^3P, M_L = \pm 1$   | $11.80 \pm 1.13$  | -34.40   |         |                                                         |
|   |      | $^3P$                | $11.60 \pm 1.34$  | -39.49   |         | $\Delta\alpha = 0.61$                                   |
|   |      | $^3P, M_L = 0$       | 21.55             | 0.14     | CCSD    |                                                         |
|   |      | $^3P, M_L = \pm 1$   | 18.02             | 0.17     |         |                                                         |
|   |      | $^3P$                | 19.20             | 0.16     |         | $\Delta\alpha = -3.53$                                  |
|   |      | $^3P, M_L = 0$       | $21.52 \pm 0.04$  | --       | CCSD(T) |                                                         |
|   |      | $^3P, M_L = \pm 1$   | $17.99 \pm 0.03$  | --       |         |                                                         |
|   |      | $^3P$                | $19.17 \pm 0.03$  | --       |         | $\Delta\alpha = -3.53$                                  |
|   |      | $^3P, M_L = 0$       | 21.04             | -3.48    | DHF     | <a href="#">2C-SR-CC@dyall.acv4z@(core 16)[vir 184]</a> |
|   |      | $^3P, M_L = \pm 1$   | 17.89             | -1.33    |         |                                                         |
|   |      | $^3P$                | 18.94             | -2.14    |         | $\Delta\alpha = -3.15$                                  |
|   |      | $^3P, M_L = 0$       | $11.99 \pm 1.08$  | -44.99   | MP2     |                                                         |
|   |      | $^3P, M_L = \pm 1$   | $12.47 \pm 0.7$   | -31.19   |         |                                                         |
|   |      | $^3P$                | $12.31 \pm 0.85$  | -36.37   |         | $\Delta\alpha = 0.48$                                   |
|   |      | $^3P, M_L = 0$       | 21.81             | 0.07     | CCSD    |                                                         |
|   |      | $^3P, M_L = \pm 1$   | 18.16             | 0.15     |         |                                                         |
|   |      | $^3P$                | 19.38             | 0.12     |         | $\Delta\alpha = -3.65$                                  |
|   |      | $^3P, M_L = 0$       | $21.80 \pm 0.02$  | --       | CCSD(T) |                                                         |
|   |      | $^3P, M_L = \pm 1$   | $18.13 \pm 0.02$  | --       |         |                                                         |
|   |      | $^3P$                | $19.35 \pm 0.02$  | --       |         | $\Delta\alpha = -3.67$                                  |
|   |      | $^3P, M_L = 0$       | 21.04             | -2.75    | DHF     | <a href="#">2C-SR-CC@dyall.acv4z@(core 16)[vir 360]</a> |
|   |      | $^3P, M_L = \pm 1$   | 17.89             | -0.64    |         |                                                         |
|   |      | $^3P$                | 18.94             | -1.43    |         | $\Delta\alpha = -3.15$                                  |

(continued)

Table S6. continued.

| Z                  | Atom             | State                | $\alpha_D$ (a.u.) | $\delta$           | Method  | Comments                                                |     |                                                         |
|--------------------|------------------|----------------------|-------------------|--------------------|---------|---------------------------------------------------------|-----|---------------------------------------------------------|
|                    |                  | $^3P, M_L = 0$       | $12.45 \pm 0.94$  | -42.46             | MP2     | $\Delta\alpha = -0.01$                                  |     |                                                         |
|                    |                  | $^3P, M_L = \pm 1$   | $12.44 \pm 0.67$  | -30.90             | CCSD    |                                                         |     |                                                         |
|                    |                  | $^3P$                | $12.44 \pm 0.77$  | -35.24             |         |                                                         |     |                                                         |
|                    |                  | $^3P, M_L = 0$       | 21.62             | -0.05              | CCSD    | $\Delta\alpha = -3.60$                                  |     |                                                         |
|                    |                  | $^3P, M_L = \pm 1$   | 18.02             | 0.09               | CCSD(T) |                                                         |     |                                                         |
|                    |                  | $^3P$                | 19.22             | 0.04               |         |                                                         |     |                                                         |
|                    |                  | $^3P, M_L = 0$       | $21.63 \pm 0.02$  | --                 |         | $\Delta\alpha = -3.63$                                  |     |                                                         |
|                    |                  | $^3P, M_L = \pm 1$   | $18.00 \pm 0.02$  | --                 |         |                                                         |     |                                                         |
|                    |                  | $^3P$                | $19.21 \pm 0.02$  | --                 |         |                                                         |     |                                                         |
|                    |                  | $^3P_2, M_J = 0$     | 20.21             |                    | MRCISD  | <a href="#">4C-DC-CI@dyall.acv4z@(core 16)[vir 184]</a> |     |                                                         |
|                    |                  | $^3P_2, M_J = \pm 1$ | 17.94             |                    |         |                                                         |     |                                                         |
|                    |                  | $^3P_2, M_J = \pm 2$ | 19.64             |                    |         |                                                         |     |                                                         |
|                    |                  | $^3P_2$              | 19.08             |                    |         |                                                         |     |                                                         |
|                    |                  | $^3P_2, M_J = 0$     | 19.89             |                    | MRCISD  | 4C-DC-CI@dyall.acv4z@(core 16)[vir 252]                 |     |                                                         |
|                    |                  | $^3P_2, M_J = \pm 1$ | 17.73             |                    |         |                                                         |     |                                                         |
|                    |                  | $^3P_2, M_J = \pm 2$ | 19.35             |                    |         |                                                         |     |                                                         |
|                    |                  | $^3P_2$              | 18.81             |                    |         |                                                         |     |                                                         |
|                    |                  | 34                   | Se                | $^3P, M_L = 0$     | 27.85   | -4.71                                                   | DHF | <a href="#">2C-NR-CC@dyall.acv4z@(core 34)[vir 478]</a> |
|                    |                  |                      |                   | $^3P, M_L = \pm 1$ | 23.65   | -0.66                                                   | MP2 |                                                         |
|                    |                  |                      |                   | $^3P$              | 25.05   | -2.20                                                   |     |                                                         |
| $^3P, M_L = 0$     | $9.35 \pm 8.62$  |                      |                   | -68.01             | MP2     | $\Delta\alpha = -4.20$                                  |     |                                                         |
| $^3P, M_L = \pm 1$ | $21.34 \pm 0.72$ |                      |                   | -10.38             | CCSD    |                                                         |     |                                                         |
| $^3P$              | $17.34 \pm 5.01$ |                      |                   | -32.30             |         |                                                         |     |                                                         |
| $^3P, M_L = 0$     | 28.32            |                      |                   | -3.11              | CCSD    | $\Delta\alpha = 11.99$                                  |     |                                                         |
| $^3P, M_L = \pm 1$ | 23.62            |                      |                   | -0.78              | CCSD(T) |                                                         |     |                                                         |
| $^3P$              | 25.19            |                      |                   | -1.67              |         |                                                         |     |                                                         |
| $^3P, M_L = 0$     | $29.23 \pm 0.46$ |                      |                   | --                 | CCSD(T) | $\Delta\alpha = -4.69$                                  |     |                                                         |
| $^3P, M_L = \pm 1$ | $23.81 \pm 0.07$ |                      |                   | --                 |         |                                                         |     |                                                         |
| $^3P$              | $25.62 \pm 0.27$ |                      |                   | --                 |         |                                                         |     |                                                         |
| $^3P, M_L = 0$     | 28.00            |                      |                   | -3.86              | DHF     | <a href="#">2C-SR-CC@dyall.acv4z@(core 16)[vir 184]</a> |     |                                                         |
| $^3P, M_L = \pm 1$ | 23.46            |                      |                   | -1.16              | MP2     |                                                         |     |                                                         |
| $^3P$              | 24.97            |                      |                   | -2.19              |         |                                                         |     |                                                         |
| $^3P, M_L = 0$     | $8.34 \pm 12.31$ |                      |                   | -71.36             | MP2     | $\Delta\alpha = -4.54$                                  |     |                                                         |
| $^3P, M_L = \pm 1$ | $22.97 \pm 0.28$ |                      |                   | -3.21              | CCSD    |                                                         |     |                                                         |
| $^3P$              | $18.10 \pm 7.11$ |                      |                   | -29.12             |         |                                                         |     |                                                         |
| $^3P, M_L = 0$     | 28.48            |                      |                   | -2.23              | CCSD    | $\Delta\alpha = 14.63$                                  |     |                                                         |
| $^3P, M_L = \pm 1$ | 23.45            |                      |                   | -1.22              |         |                                                         |     |                                                         |
| $^3P$              | 25.12            | -1.60                |                   |                    |         |                                                         |     |                                                         |
|                    |                  |                      |                   |                    |         | $\Delta\alpha = -5.03$                                  |     |                                                         |

(continued)



Table S6. continued.

| Z  | Atom | State                | $\alpha_D$ (a.u.) | $\delta$ | Method  | Comments                                                |
|----|------|----------------------|-------------------|----------|---------|---------------------------------------------------------|
|    |      | $^3P, M_L = 0$       | $29.13 \pm 0.22$  | --       | CCSD(T) |                                                         |
|    |      | $^3P, M_L = \pm 1$   | $23.74 \pm 0.09$  | --       |         |                                                         |
|    |      | $^3P$                | $25.53 \pm 0.15$  | --       |         | $\Delta\alpha = -5.39$                                  |
|    |      | $^3P, M_L = 0$       | 28.00             | -4.63    | DHF     | <a href="#">2C-SR-CC@dyall.acv4z@(core 34)[vir 478]</a> |
|    |      | $^3P, M_L = \pm 1$   | 23.46             | -0.90    |         |                                                         |
|    |      | $^3P$                | 24.98             | -2.33    |         | $\Delta\alpha = -4.54$                                  |
|    |      | $^3P, M_L = 0$       | $15.55 \pm 7.71$  | -47.03   | MP2     |                                                         |
|    |      | $^3P, M_L = \pm 1$   | $22.93 \pm 0.35$  | -3.13    |         |                                                         |
|    |      | $^3P$                | $20.47 \pm 4.46$  | -19.93   |         | $\Delta\alpha = 7.38$                                   |
|    |      | $^3P, M_L = 0$       | 28.52             | -2.86    | CCSD    |                                                         |
|    |      | $^3P, M_L = \pm 1$   | 23.46             | -0.89    |         |                                                         |
|    |      | $^3P$                | 25.15             | -1.64    |         | $\Delta\alpha = -5.06$                                  |
|    |      | $^3P, M_L = 0$       | $29.36 \pm 0.33$  | --       | CCSD(T) |                                                         |
|    |      | $^3P, M_L = \pm 1$   | $23.67 \pm 0.04$  | --       |         |                                                         |
|    |      | $^3P$                | $25.57 \pm 0.19$  | --       |         | $\Delta\alpha = -5.69$                                  |
|    |      | $^3P_2, M_J = 0$     | 25.87             |          | MRCISD  | <a href="#">4C-DC-CI@dyall.acv4z@(core 16)[vir 184]</a> |
|    |      | $^3P_2, M_J = \pm 1$ | 23.08             |          |         |                                                         |
|    |      | $^3P_2, M_J = \pm 2$ | 25.18             |          |         |                                                         |
|    |      | $^3P_2$              | 24.48             |          |         |                                                         |
| 52 | Te   | $^3P, M_L = 0$       | 41.88             | -2.11    | DHF     | <a href="#">2C-NR-CC@dyall.acv4z@(core 52)[vir 550]</a> |
|    |      | $^3P, M_L = \pm 1$   | 36.97             | 1.44     |         |                                                         |
|    |      | $^3P$                | 38.61             | 0.12     |         | $\Delta\alpha = -4.91$                                  |
|    |      | $^3P, M_L = 0$       | $28.66 \pm 7.63$  | -33.01   | MP2     |                                                         |
|    |      | $^3P, M_L = \pm 1$   | $29.10 \pm 4.58$  | -20.14   |         |                                                         |
|    |      | $^3P$                | $28.96 \pm 5.78$  | -24.90   |         | $\Delta\alpha = 0.44$                                   |
|    |      | $^3P, M_L = 0$       | 41.68             | -2.58    | CCSD    |                                                         |
|    |      | $^3P, M_L = \pm 1$   | 36.27             | -0.47    |         |                                                         |
|    |      | $^3P$                | 38.08             | -1.25    |         | $\Delta\alpha = -5.41$                                  |
|    |      | $^3P, M_L = 0$       | $42.79 \pm 0.49$  | --       | CCSD(T) |                                                         |
|    |      | $^3P, M_L = \pm 1$   | $36.44 \pm 0.01$  | --       |         |                                                         |
|    |      | $^3P$                | $38.56 \pm 0.28$  | --       |         | $\Delta\alpha = -6.34$                                  |
|    |      | $^3P, M_L = 0$       | 42.01             | -1.72    | DHF     | <a href="#">2C-SR-CC@dyall.acv4z@(core 16)[vir 216]</a> |
|    |      | $^3P, M_L = \pm 1$   | 35.96             | 1.21     |         |                                                         |
|    |      | $^3P$                | 37.98             | 0.11     |         | $\Delta\alpha = -6.05$                                  |
|    |      | $^3P, M_L = 0$       | $16.91 \pm 15.45$ | -60.43   | MP2     |                                                         |
|    |      | $^3P, M_L = \pm 1$   | $26.15 \pm 6.08$  | -26.40   |         |                                                         |
|    |      | $^3P$                | $23.07 \pm 10.21$ | -39.18   |         | $\Delta\alpha = 9.24$                                   |
|    |      | $^3P, M_L = 0$       | 42.13             | -1.44    | CCSD    |                                                         |

(continued)

Table S6. continued.

| Z  | Atom | State                | $\alpha_D$ (a.u.) | $\delta$ | Method  | Comments                                                |
|----|------|----------------------|-------------------|----------|---------|---------------------------------------------------------|
|    |      | $^3P, M_L = \pm 1$   | 35.55             | 0.05     |         |                                                         |
|    |      | $^3P$                | 37.74             | -0.51    |         | $\Delta\alpha = -6.58$                                  |
|    |      | $^3P, M_L = 0$       | $42.74 \pm 0.15$  | --       | CCSD(T) |                                                         |
|    |      | $^3P, M_L = \pm 1$   | $35.53 \pm 0.14$  | --       |         |                                                         |
|    |      | $^3P$                | $37.94 \pm 0.14$  | --       |         | $\Delta\alpha = -7.21$                                  |
|    |      | $^3P, M_L = 0$       | 42.01             | -1.33    | DHF     | <a href="#">2C-SR-CC@dyall.acv4z@(core 52)[vir 550]</a> |
|    |      | $^3P, M_L = \pm 1$   | 35.96             | 0.64     |         |                                                         |
|    |      | $^3P$                | 37.98             | -0.10    |         | $\Delta\alpha = -6.05$                                  |
|    |      | $^3P, M_L = 0$       | $14.64 \pm 16.69$ | -65.61   | MP2     |                                                         |
|    |      | $^3P, M_L = \pm 1$   | $37.70 \pm 1.28$  | 5.51     |         |                                                         |
|    |      | $^3P$                | $30.02 \pm 9.69$  | -21.04   |         | $\Delta\alpha = 23.06$                                  |
|    |      | $^3P, M_L = 0$       | 42.02             | -1.32    | CCSD    |                                                         |
|    |      | $^3P, M_L = \pm 1$   | 35.44             | -0.83    |         |                                                         |
|    |      | $^3P$                | 37.63             | -1.01    |         | $\Delta\alpha = -6.58$                                  |
|    |      | $^3P, M_L = 0$       | $42.58 \pm 0.12$  | --       | CCSD(T) |                                                         |
|    |      | $^3P, M_L = \pm 1$   | $35.73 \pm 0.06$  | --       |         |                                                         |
|    |      | $^3P$                | $38.01 \pm 0.09$  | --       |         | $\Delta\alpha = -6.84$                                  |
|    |      | $^3P_2, M_J = 0$     | 38.00             |          | MRCISD  | <a href="#">4C-DC-CI@dyall.acv4z@(core 16)[vir 216]</a> |
|    |      | $^3P_2, M_J = \pm 1$ | 35.16             |          |         |                                                         |
|    |      | $^3P_2, M_J = \pm 2$ | 37.29             |          |         |                                                         |
|    |      | $^3P_2$              | 36.58             |          |         |                                                         |
| 84 | Po   | $^3P, M_L = 0$       | $50.21 \pm 0.01$  | 0.58     | DHF     | <a href="#">2C-NR-CC@dyall.acv4z@(core 48)[vir 296]</a> |
|    |      | $^3P, M_L = \pm 1$   | $44.79 \pm 0.01$  | 2.31     |         |                                                         |
|    |      | $^3P$                | $46.60 \pm 0.01$  | 1.68     |         | $\Delta\alpha = -5.42$                                  |
|    |      | $^3P, M_L = 0$       | $31.26 \pm 10.96$ | -37.38   | MP2     |                                                         |
|    |      | $^3P, M_L = \pm 1$   | $39.37 \pm 2.73$  | -10.07   |         |                                                         |
|    |      | $^3P$                | $36.67 \pm 6.71$  | -19.99   |         | $\Delta\alpha = 8.11$                                   |
|    |      | $^3P, M_L = 0$       | $49.54 \pm 0.01$  | -0.78    | CCSD    |                                                         |
|    |      | $^3P, M_L = \pm 1$   | $43.65 \pm 0.01$  | -0.28    |         |                                                         |
|    |      | $^3P$                | $45.61 \pm 0.01$  | -0.46    |         | $\Delta\alpha = -5.88$                                  |
|    |      | $^3P, M_L = 0$       | $49.92 \pm 0.02$  | --       | CCSD(T) |                                                         |
|    |      | $^3P, M_L = \pm 1$   | $43.78 \pm 0.02$  | --       |         |                                                         |
|    |      | $^3P$                | $45.83 \pm 0.02$  | --       |         | $\Delta\alpha = -6.14$                                  |
|    |      | $^3P, M_L = 0$       | $50.27 \pm 0.01$  | -1.36    | DHF     | <a href="#">2C-SR-CC@dyall.acv4z@(core 16)[vir 262]</a> |
|    |      | $^3P, M_L = \pm 1$   | 41.40             | 0.40     |         |                                                         |
|    |      | $^3P$                | 44.35             | -0.27    |         | $\Delta\alpha = -8.87$                                  |
|    |      | $^3P, M_L = 0$       | $48.53 \pm 0.2$   | -4.77    | MP2     |                                                         |
|    |      | $^3P, M_L = \pm 1$   | $41.28 \pm 0.01$  | 0.12     |         |                                                         |

(continued)

Table S6. continued.

| Z   | Atom | State                | $\alpha_D$ (a.u.) | $\delta$ | Method  | Comments                                                |
|-----|------|----------------------|-------------------|----------|---------|---------------------------------------------------------|
|     |      | $^3P$                | $43.70 \pm 0.12$  | -1.75    | CCSD    | $\Delta\alpha = -7.24$                                  |
|     |      | $^3P, M_L = 0$       | $50.46 \pm 0.01$  | -0.98    |         |                                                         |
|     |      | $^3P, M_L = \pm 1$   | 40.96             | -0.65    |         |                                                         |
|     |      | $^3P$                | 44.13             | -0.78    | CCSD(T) | $\Delta\alpha = -9.50$                                  |
|     |      | $^3P, M_L = 0$       | $50.96 \pm 0.01$  | --       |         |                                                         |
|     |      | $^3P, M_L = \pm 1$   | 41.23             | --       |         |                                                         |
|     |      | $^3P$                | 44.48             | --       |         | $\Delta\alpha = -9.73$                                  |
|     |      | $^3P, M_L = 0$       | $50.27 \pm 0.01$  | -1.05    | DHF     | <a href="#">2C-SR-CC@dyall.acv4z@(core 48)[vir 296]</a> |
|     |      | $^3P, M_L = \pm 1$   | 41.40             | 0.78     |         |                                                         |
|     |      | $^3P$                | 44.36             | 0.08     | MP2     | $\Delta\alpha = -8.87$                                  |
|     |      | $^3P, M_L = 0$       | $47.99 \pm 0.21$  | -5.53    |         |                                                         |
|     |      | $^3P, M_L = \pm 1$   | $41.07 \pm 0.03$  | -0.03    |         |                                                         |
|     |      | $^3P$                | $43.38 \pm 0.13$  | -2.13    | CCSD    | $\Delta\alpha = -6.93$                                  |
|     |      | $^3P, M_L = 0$       | $50.28 \pm 0.01$  | -1.02    |         |                                                         |
|     |      | $^3P, M_L = \pm 1$   | 40.82             | -0.63    |         |                                                         |
|     |      | $^3P$                | 43.97             | -0.78    | CCSD(T) | $\Delta\alpha = -9.46$                                  |
|     |      | $^3P, M_L = 0$       | $50.80 \pm 0.01$  | --       |         |                                                         |
|     |      | $^3P, M_L = \pm 1$   | 41.08             | --       |         |                                                         |
|     |      | $^3P$                | 44.32             | --       |         | $\Delta\alpha = -9.72$                                  |
|     |      | $^3P_2, M_J = 0$     | 43.83             |          | MRCISD  | <a href="#">4C-DC-CI@dyall.acv4z@(core 16)[vir 262]</a> |
|     |      | $^3P_2, M_J = \pm 1$ | 42.61             |          |         |                                                         |
|     |      | $^3P_2, M_J = \pm 2$ | 43.52             |          |         |                                                         |
|     |      | $^3P_2$              | 43.22             |          |         |                                                         |
| 116 | Lv   | $^3P, M_L = 0$       | $64.05 \pm 0.01$  | 2.11     | DHF     | <a href="#">2C-NR-CC@dyall.acv4z@(core 48)[vir 294]</a> |
|     |      | $^3P, M_L = \pm 1$   | 58.64             | 3.39     |         |                                                         |
|     |      | $^3P$                | $60.44 \pm 0.01$  | 2.93     | MP2     | $\Delta\alpha = -5.41$                                  |
|     |      | $^3P, M_L = 0$       | $61.15 \pm 0.1$   | -2.51    |         |                                                         |
|     |      | $^3P, M_L = \pm 1$   | $56.07 \pm 0.03$  | -1.15    |         |                                                         |
|     |      | $^3P$                | $57.76 \pm 0.06$  | -1.63    | CCSD    | $\Delta\alpha = -5.08$                                  |
|     |      | $^3P, M_L = 0$       | $62.40 \pm 0.02$  | -0.52    |         |                                                         |
|     |      | $^3P, M_L = \pm 1$   | 56.62             | -0.17    |         |                                                         |
|     |      | $^3P$                | $58.55 \pm 0.01$  | -0.30    | CCSD(T) | $\Delta\alpha = -5.78$                                  |
|     |      | $^3P, M_L = 0$       | $62.72 \pm 0.02$  | --       |         |                                                         |
|     |      | $^3P, M_L = \pm 1$   | 56.72             | --       |         |                                                         |
|     |      | $^3P$                | $58.72 \pm 0.01$  | --       |         | $\Delta\alpha = -6.01$                                  |
|     |      | $^3P, M_L = 0$       | $67.24 \pm 0.01$  | -0.63    | DHF     | <a href="#">2C-SR-CC@dyall.acv4z@(core 16)[vir 262]</a> |
|     |      | $^3P, M_L = \pm 1$   | $52.88 \pm 0.01$  | 1.69     |         |                                                         |
|     |      | $^3P$                | $57.67 \pm 0.01$  | 0.77     |         | $\Delta\alpha = -14.36$                                 |

(continued)

Table S6. continued.

| Z | Atom | State                | $\alpha_D$ (a.u.) | $\delta$ | Method  | Comments                                                |
|---|------|----------------------|-------------------|----------|---------|---------------------------------------------------------|
|   |      | $^3P, M_L = 0$       | $64.21 \pm 0.22$  | -5.12    | MP2     |                                                         |
|   |      | $^3P, M_L = \pm 1$   | $51.15 \pm 0.05$  | -1.63    |         |                                                         |
|   |      | $^3P$                | $55.50 \pm 0.13$  | -3.00    |         | $\Delta\alpha = -13.05$                                 |
|   |      | $^3P, M_L = 0$       | $67.14 \pm 0.02$  | -0.77    | CCSD    |                                                         |
|   |      | $^3P, M_L = \pm 1$   | 51.78             | -0.43    |         |                                                         |
|   |      | $^3P$                | $56.90 \pm 0.01$  | -0.57    |         | $\Delta\alpha = -15.37$                                 |
|   |      | $^3P, M_L = 0$       | $67.67 \pm 0.02$  | --       | CCSD(T) |                                                         |
|   |      | $^3P, M_L = \pm 1$   | 52.00             | --       |         |                                                         |
|   |      | $^3P$                | $57.22 \pm 0.01$  | --       |         | $\Delta\alpha = -15.67$                                 |
|   |      | $^3P, M_L = 0$       | $67.24 \pm 0.01$  | -0.25    | DHF     | <a href="#">2C-SR-CC@dyall.acv4z@(core 48)[vir 294]</a> |
|   |      | $^3P, M_L = \pm 1$   | 52.88             | 2.09     |         |                                                         |
|   |      | $^3P$                | $57.67 \pm 0.01$  | 1.17     |         | $\Delta\alpha = -14.36$                                 |
|   |      | $^3P, M_L = 0$       | $63.29 \pm 0.2$   | -6.11    | MP2     |                                                         |
|   |      | $^3P, M_L = \pm 1$   | $51.07 \pm 0.03$  | -1.40    |         |                                                         |
|   |      | $^3P$                | $55.14 \pm 0.12$  | -3.26    |         | $\Delta\alpha = -12.22$                                 |
|   |      | $^3P, M_L = 0$       | $66.82 \pm 0.02$  | -0.88    | CCSD    |                                                         |
|   |      | $^3P, M_L = \pm 1$   | 51.57             | -0.43    |         |                                                         |
|   |      | $^3P$                | $56.66 \pm 0.01$  | -0.61    |         | $\Delta\alpha = -15.25$                                 |
|   |      | $^3P, M_L = 0$       | $67.41 \pm 0.01$  | --       | CCSD(T) |                                                         |
|   |      | $^3P, M_L = \pm 1$   | 51.80             | --       |         |                                                         |
|   |      | $^3P$                | $57.00 \pm 0.01$  | --       |         | $\Delta\alpha = -15.62$                                 |
|   |      | $^3P_2, M_J = 0$     | 68.41             |          | MRCISD  | <a href="#">4C-DC-CI@dyall.acv4z@(core 16)[vir 262]</a> |
|   |      | $^3P_2, M_J = \pm 1$ | 74.92             |          |         |                                                         |
|   |      | $^3P_2, M_J = \pm 2$ | 70.04             |          |         |                                                         |
|   |      | $^3P_2$              | 71.66             |          |         |                                                         |

## S1.7 Group 17 elements

Table S7: The results of dipole polarizability for Group 17 elements.

| Z | Atom | State              | $\alpha_D$ (a.u.) | $\delta$ (%) | Method | Comments                                               |
|---|------|--------------------|-------------------|--------------|--------|--------------------------------------------------------|
| 9 | F    | $^2P, M_L = 0$     | 3.02              | -9.49        | DHF    | <a href="#">2C-NR-CC@dyall.acv4z@(core 9)[vir 247]</a> |
|   |      | $^2P, M_L = \pm 1$ | 3.31              | -11.43       |        |                                                        |
|   |      | $^2P$              | 3.21              | -10.83       |        | $\Delta\alpha = 0.29$                                  |
|   |      | $^2P, M_L = 0$     | $3.32 \pm 0.01$   | -0.40        | MP2    |                                                        |

(continued)

Table S7. continued.

| Z | Atom | State                      | $\alpha_D$ (a.u.) | $\delta$ | Method  | Comments                                               |
|---|------|----------------------------|-------------------|----------|---------|--------------------------------------------------------|
|   |      | $^2P, M_L = \pm 1$         | $3.57 \pm 0.02$   | -4.35    |         |                                                        |
|   |      | $^2P$                      | $3.49 \pm 0.02$   | -3.13    |         | $\Delta\alpha = 0.25$                                  |
|   |      | $^2P, M_L = 0$             | 3.29              | -1.36    | CCSD    |                                                        |
|   |      | $^2P, M_L = \pm 1$         | 3.67              | -1.77    |         |                                                        |
|   |      | $^2P$                      | 3.54              | -1.64    |         | $\Delta\alpha = 0.38$                                  |
|   |      | $^2P, M_L = 0$             | 3.33              | --       | CCSD(T) |                                                        |
|   |      | $^2P, M_L = \pm 1$         | 3.73              | --       |         |                                                        |
|   |      | $^2P$                      | 3.60              | --       |         | $\Delta\alpha = 0.40$                                  |
|   |      | $^2P, M_L = 0$             | 3.02              | -9.62    | DHF     | <a href="#">2C-SR-CC@dyall.acv4z@(core 9)[vir 183]</a> |
|   |      | $^2P, M_L = \pm 1$         | 3.31              | -11.39   |         |                                                        |
|   |      | $^2P$                      | 3.21              | -10.85   |         | $\Delta\alpha = 0.30$                                  |
|   |      | $^2P, M_L = 0$             | $3.61 \pm 0.06$   | 8.26     | MP2     |                                                        |
|   |      | $^2P, M_L = \pm 1$         | $3.43 \pm 0.05$   | -8.15    |         |                                                        |
|   |      | $^2P$                      | $3.49 \pm 0.05$   | -3.09    |         | $\Delta\alpha = -0.18$                                 |
|   |      | $^2P, M_L = 0$             | 3.29              | -1.48    | CCSD    |                                                        |
|   |      | $^2P, M_L = \pm 1$         | 3.67              | -1.73    |         |                                                        |
|   |      | $^2P$                      | 3.55              | -1.65    |         | $\Delta\alpha = 0.38$                                  |
|   |      | $^2P, M_L = 0$             | 3.34              | --       | CCSD(T) |                                                        |
|   |      | $^2P, M_L = \pm 1$         | 3.74              | --       |         |                                                        |
|   |      | $^2P$                      | 3.60              | --       |         | $\Delta\alpha = 0.40$                                  |
|   |      | $^2P, M_L = 0$             | 3.02              | -9.61    | DHF     | <a href="#">2C-SR-CC@dyall.acv4z@(core 9)[vir 247]</a> |
|   |      | $^2P, M_L = \pm 1$         | 3.31              | -11.41   |         |                                                        |
|   |      | $^2P$                      | 3.21              | -10.85   |         | $\Delta\alpha = 0.30$                                  |
|   |      | $^2P, M_L = 0$             | $3.49 \pm 0.03$   | 4.58     | MP2     |                                                        |
|   |      | $^2P, M_L = \pm 1$         | $3.46 \pm 0.05$   | -7.34    |         |                                                        |
|   |      | $^2P$                      | $3.47 \pm 0.04$   | -3.66    |         | $\Delta\alpha = -0.03$                                 |
|   |      | $^2P, M_L = 0$             | 3.29              | -1.47    | CCSD    |                                                        |
|   |      | $^2P, M_L = \pm 1$         | 3.67              | -1.72    |         |                                                        |
|   |      | $^2P$                      | 3.55              | -1.65    |         | $\Delta\alpha = 0.39$                                  |
|   |      | $^2P, M_L = 0$             | 3.34              | --       | CCSD(T) |                                                        |
|   |      | $^2P, M_L = \pm 1$         | 3.74              | --       |         |                                                        |
|   |      | $^2P$                      | 3.61              | --       |         | $\Delta\alpha = 0.40$                                  |
|   |      | $^2P_{3/2}, M_J = \pm 1/2$ | 3.43              |          | MRCISD  | <a href="#">4C-DC-CI@dyall.acv4z@(core 9)[vir 115]</a> |
|   |      | $^2P_{3/2}, M_J = \pm 3/2$ | 3.70              |          |         |                                                        |
|   |      | $^2P_{3/2}$                | 3.57              |          |         |                                                        |
|   |      | $^2P_{1/2}$                | 3.57              |          |         | $\bar{\alpha}_{J=3/2} - \alpha_{J=1/2} = -0.00$        |
|   |      | $^2P_{3/2}, M_J = \pm 1/2$ | 3.37              |          | MRCISD  | <a href="#">4C-DC-CI@dyall.acv4z@(core 9)[vir 183]</a> |
|   |      | $^2P_{3/2}, M_J = \pm 3/2$ | 3.61              |          |         |                                                        |

(continued)

Table S7. continued.

| Z  | Atom | State              | $\alpha_D$ (a.u.) | $\delta$ | Method  | Comments                                                |
|----|------|--------------------|-------------------|----------|---------|---------------------------------------------------------|
| 17 | Cl   | $^2P_{3/2}$        | 3.49              |          |         |                                                         |
|    |      | $^2P_{1/2}$        | 3.49              |          |         | $\bar{\alpha}_{J=3/2} - \alpha_{J=1/2} = -0.00$         |
|    |      | $^2P, M_L = 0$     | 13.09             | -2.35    | DHF     | <a href="#">2C-NR-CC@dyall.acv4z@(core 17)[vir 359]</a> |
|    |      | $^2P, M_L = \pm 1$ | 14.69             | -2.73    |         |                                                         |
|    |      | $^2P$              | 14.16             | -2.61    |         | $\Delta\alpha = 1.60$                                   |
|    |      | $^2P, M_L = 0$     | $13.57 \pm 0.02$  | 1.24     | MP2     |                                                         |
|    |      | $^2P, M_L = \pm 1$ | $14.90 \pm 0.03$  | -1.39    |         |                                                         |
|    |      | $^2P$              | $14.45 \pm 0.03$  | -0.58    |         | $\Delta\alpha = 1.32$                                   |
|    |      | $^2P, M_L = 0$     | 13.29             | -0.89    | CCSD    |                                                         |
|    |      | $^2P, M_L = \pm 1$ | 14.96             | -0.93    |         |                                                         |
|    |      | $^2P$              | 14.41             | -0.92    |         | $\Delta\alpha = 1.68$                                   |
|    |      | $^2P, M_L = 0$     | 13.41             | --       | CCSD(T) |                                                         |
|    |      | $^2P, M_L = \pm 1$ | 15.11             | --       |         |                                                         |
|    |      | $^2P$              | 14.54             | --       |         | $\Delta\alpha = 1.70$                                   |
|    |      | $^2P, M_L = 0$     | 13.08             | -3.09    | DHF     | <a href="#">2C-SR-CC@dyall.acv4z@(core 17)[vir 169]</a> |
|    |      | $^2P, M_L = \pm 1$ | 14.72             | -3.56    |         |                                                         |
|    |      | $^2P$              | 14.18             | -3.41    |         | $\Delta\alpha = 1.64$                                   |
|    |      | $^2P, M_L = 0$     | $14.27 \pm 0.16$  | 5.68     | MP2     |                                                         |
|    |      | $^2P, M_L = \pm 1$ | $15.29 \pm 0.02$  | 0.13     |         |                                                         |
|    |      | $^2P$              | $14.95 \pm 0.09$  | 1.84     |         | $\Delta\alpha = 1.02$                                   |
|    |      | $^2P, M_L = 0$     | 13.37             | -0.92    | CCSD    |                                                         |
|    |      | $^2P, M_L = \pm 1$ | 15.12             | -0.97    |         |                                                         |
|    |      | $^2P$              | 14.54             | -0.95    |         | $\Delta\alpha = 1.75$                                   |
|    |      | $^2P, M_L = 0$     | $13.50 \pm 0.01$  | --       | CCSD(T) |                                                         |
|    |      | $^2P, M_L = \pm 1$ | 15.27             | --       |         |                                                         |
|    |      | $^2P$              | 14.68             | --       |         | $\Delta\alpha = 1.77$                                   |
|    |      | $^2P, M_L = 0$     | 13.08             | -2.57    | DHF     | <a href="#">2C-SR-CC@dyall.acv4z@(core 17)[vir 359]</a> |
|    |      | $^2P, M_L = \pm 1$ | 14.72             | -2.67    |         |                                                         |
|    |      | $^2P$              | 14.18             | -2.64    |         | $\Delta\alpha = 1.64$                                   |
|    |      | $^2P, M_L = 0$     | $14.88 \pm 0.33$  | 10.81    | MP2     |                                                         |
|    |      | $^2P, M_L = \pm 1$ | $14.04 \pm 0.23$  | -7.19    |         |                                                         |
|    |      | $^2P$              | $14.32 \pm 0.26$  | -1.66    |         | $\Delta\alpha = -0.84$                                  |
|    |      | $^2P, M_L = 0$     | 13.28             | -1.11    | CCSD    |                                                         |
|    |      | $^2P, M_L = \pm 1$ | 15.00             | -0.85    |         |                                                         |
|    |      | $^2P$              | 14.43             | -0.93    |         | $\Delta\alpha = 1.72$                                   |
|    |      | $^2P, M_L = 0$     | $13.43 \pm 0.01$  | --       | CCSD(T) |                                                         |
|    |      | $^2P, M_L = \pm 1$ | 15.13             | --       |         |                                                         |
|    |      | $^2P$              | $14.56 \pm 0.01$  | --       |         | $\Delta\alpha = 1.70$                                   |

(continued)

Table S7. continued.

| Z  | Atom | State                      | $\alpha_D$ (a.u.) | $\delta$ | Method  | Comments                                                |
|----|------|----------------------------|-------------------|----------|---------|---------------------------------------------------------|
| 35 | Br   | $^2P_{3/2}, M_J = \pm 1/2$ | 13.78             |          | MRCISD  | <a href="#">4C-DC-CI@dyall.acv4z@(core 17)[vir 169]</a> |
|    |      | $^2P_{3/2}, M_J = \pm 3/2$ | 14.94             |          |         |                                                         |
|    |      | $^2P_{3/2}$                | 14.36             |          |         |                                                         |
|    |      | $^2P_{1/2}$                | 14.40             |          |         | $\bar{\alpha}_{J=3/2} - \alpha_{J=1/2} = -0.04$         |
|    |      | $^2P_{3/2}, M_J = \pm 1/2$ | 13.64             |          | MRCISD  | <a href="#">4C-DC-CI@dyall.acv4z@(core 17)[vir 243]</a> |
|    |      | $^2P_{3/2}, M_J = \pm 3/2$ | 14.78             |          |         |                                                         |
|    |      | $^2P_{3/2}$                | 14.21             |          |         |                                                         |
|    |      | $^2P_{1/2}$                | 14.25             |          |         | $\bar{\alpha}_{J=3/2} - \alpha_{J=1/2} = -0.04$         |
|    |      | $^2P, M_L = 0$             | 18.76             | -3.28    | DHF     | <a href="#">2C-NR-CC@dyall.acv4z@(core 35)[vir 477]</a> |
|    |      | $^2P, M_L = \pm 1$         | 21.07             | -0.41    |         |                                                         |
|    |      | $^2P$                      | 20.30             | -1.31    |         | $\Delta\alpha = 2.30$                                   |
|    |      | $^2P, M_L = 0$             | $27.52 \pm 5.29$  | 41.85    | MP2     |                                                         |
|    |      | $^2P, M_L = \pm 1$         | $3.53 \pm 11.19$  | -83.30   |         |                                                         |
|    |      | $^2P$                      | $11.53 \pm 9.64$  | -43.96   |         | $\Delta\alpha = -23.99$                                 |
| 35 | Br   | $^2P, M_L = 0$             | 18.84             | -2.88    | CCSD    |                                                         |
|    |      | $^2P, M_L = \pm 1$         | 21.25             | 0.45     |         |                                                         |
|    |      | $^2P$                      | 20.45             | -0.60    |         | $\Delta\alpha = 2.41$                                   |
|    |      | $^2P, M_L = 0$             | $19.40 \pm 0.27$  | --       | CCSD(T) |                                                         |
|    |      | $^2P, M_L = \pm 1$         | $21.15 \pm 0.18$  | --       |         |                                                         |
|    |      | $^2P$                      | $20.57 \pm 0.22$  | --       |         | $\Delta\alpha = 1.75$                                   |
|    |      | $^2P, M_L = 0$             | 18.58             | -4.68    | DHF     | <a href="#">2C-SR-CC@dyall.acv4z@(core 17)[vir 183]</a> |
|    |      | $^2P, M_L = \pm 1$         | 21.09             | -0.89    |         |                                                         |
|    |      | $^2P$                      | 20.26             | -2.08    |         | $\Delta\alpha = 2.51$                                   |
|    |      | $^2P, M_L = 0$             | $42.67 \pm 15.0$  | 118.90   | MP2     |                                                         |
|    |      | $^2P, M_L = \pm 1$         | $8.02 \pm 8.37$   | -62.32   |         |                                                         |
|    |      | $^2P$                      | $19.57 \pm 11.03$ | -5.39    |         | $\Delta\alpha = -34.65$                                 |
|    |      | $^2P, M_L = 0$             | 18.68             | -4.16    | CCSD    |                                                         |
|    |      | $^2P, M_L = \pm 1$         | 21.28             | -0.03    |         |                                                         |
|    |      | $^2P$                      | 20.41             | -1.33    |         | $\Delta\alpha = 2.59$                                   |
|    |      | $^2P, M_L = 0$             | $19.49 \pm 0.44$  | --       | CCSD(T) |                                                         |
|    |      | $^2P, M_L = \pm 1$         | $21.28 \pm 0.12$  | --       |         |                                                         |
|    |      | $^2P$                      | $20.69 \pm 0.27$  | --       |         | $\Delta\alpha = 1.79$                                   |
|    |      | $^2P, M_L = 0$             | 18.58             | -5.18    | DHF     | <a href="#">2C-SR-CC@dyall.acv4z@(core 35)[vir 477]</a> |
|    |      | $^2P, M_L = \pm 1$         | 21.09             | -2.80    |         |                                                         |
|    |      | $^2P$                      | 20.26             | -3.54    |         | $\Delta\alpha = 2.51$                                   |
|    |      | $^2P, M_L = 0$             | $43.98 \pm 15.8$  | 124.42   | MP2     |                                                         |
|    |      | $^2P, M_L = \pm 1$         | $25.65 \pm 2.79$  | 18.20    |         |                                                         |
|    |      | $^2P$                      | $31.76 \pm 9.4$   | 51.25    |         | $\Delta\alpha = -18.33$                                 |

(continued)

Table S7. continued.

| Z  | Atom | State                      | $\alpha_D$ (a.u.)  | $\delta$ | Method  | Comments                                                |
|----|------|----------------------------|--------------------|----------|---------|---------------------------------------------------------|
| 53 | I    | $^2P, M_L = 0$             | 18.68              | -4.69    | CCSD    | $\Delta\alpha = 2.62$                                   |
|    |      | $^2P, M_L = \pm 1$         | 21.30              | -1.82    |         |                                                         |
|    |      | $^2P$                      | 20.43              | -2.71    |         |                                                         |
|    |      | $^2P, M_L = 0$             | $19.60 \pm 0.49$   | --       | CCSD(T) | $\Delta\alpha = 2.10$                                   |
|    |      | $^2P, M_L = \pm 1$         | $21.70 \pm 0.12$   | --       |         |                                                         |
|    |      | $^2P$                      | $21.00 \pm 0.3$    | --       |         |                                                         |
|    |      | $^2P_{3/2}, M_J = \pm 1/2$ | 19.16              |          | MRCISD  | <a href="#">4C-DC-CI@dyall.acv4z@(core 17)[vir 183]</a> |
|    |      | $^2P_{3/2}, M_J = \pm 3/2$ | 20.95              |          |         |                                                         |
|    |      | $^2P_{3/2}$                | 20.06              |          |         |                                                         |
|    |      | $^2P_{1/2}$                | 20.27              |          |         |                                                         |
|    |      |                            |                    |          |         | $\bar{\alpha}_{J=3/2} - \alpha_{J=1/2} = -0.22$         |
|    |      | $^2P, M_L = 0$             | 30.51              | -8.26    | DHF     | <a href="#">2C-NR-CC@dyall.acv4z@(core 53)[vir 549]</a> |
|    |      | $^2P, M_L = \pm 1$         | 33.28              | 0.34     |         |                                                         |
|    |      | $^2P$                      | 32.36              | -2.53    |         |                                                         |
|    |      | $^2P, M_L = 0$             | $126.35 \pm 53.93$ | 279.93   | MP2     | $\Delta\alpha = -100.86$                                |
|    |      | $^2P, M_L = \pm 1$         | $25.49 \pm 4.65$   | -23.14   |         |                                                         |
|    |      | $^2P$                      | $59.11 \pm 31.37$  | 78.06    |         |                                                         |
|    |      | $^2P, M_L = 0$             | 30.12              | -9.44    | CCSD    | $\Delta\alpha = 2.87$                                   |
|    |      | $^2P, M_L = \pm 1$         | 32.99              | -0.53    |         |                                                         |
|    |      | $^2P$                      | 32.03              | -3.51    |         |                                                         |
|    |      | $^2P, M_L = 0$             | $33.26 \pm 1.67$   | --       | CCSD(T) | $\Delta\alpha = -0.09$                                  |
|    |      | $^2P, M_L = \pm 1$         | $33.17 \pm 0.04$   | --       |         |                                                         |
|    |      | $^2P$                      | $33.20 \pm 0.96$   | --       |         |                                                         |
| 53 | I    | $^2P, M_L = 0$             | 29.61              | -0.56    | DHF     | <a href="#">2C-SR-CC@dyall.acv4z@(core 17)[vir 215]</a> |
|    |      | $^2P, M_L = \pm 1$         | 33.08              | -0.41    |         |                                                         |
|    |      | $^2P$                      | 31.92              | -0.46    |         |                                                         |
|    |      | $^2P, M_L = 0$             | $34.63 \pm 2.95$   | 16.28    | MP2     | $\Delta\alpha = -8.33$                                  |
|    |      | $^2P, M_L = \pm 1$         | $26.29 \pm 4.17$   | -20.84   |         |                                                         |
|    |      | $^2P$                      | $29.07 \pm 3.8$    | -9.35    |         |                                                         |
|    |      | $^2P, M_L = 0$             | 29.44              | -1.15    | CCSD    | $\Delta\alpha = 3.56$                                   |
|    |      | $^2P, M_L = \pm 1$         | 33.00              | -0.66    |         |                                                         |
|    |      | $^2P$                      | 31.81              | -0.81    |         |                                                         |
|    |      | $^2P, M_L = 0$             | $29.78 \pm 0.09$   | --       | CCSD(T) | $\Delta\alpha = 3.44$                                   |
|    |      | $^2P, M_L = \pm 1$         | $33.22 \pm 0.03$   | --       |         |                                                         |
|    |      | $^2P$                      | $32.07 \pm 0.06$   | --       |         |                                                         |
|    |      | $^2P, M_L = 0$             | 29.61              | -0.34    | DHF     | <a href="#">2C-SR-CC@dyall.acv4z@(core 53)[vir 549]</a> |
|    |      | $^2P, M_L = \pm 1$         | 33.08              | -0.44    |         |                                                         |
|    |      | $^2P$                      | 31.92              | -0.41    |         |                                                         |
|    |      | $^2P, M_L = 0$             | $37.81 \pm 4.98$   | 27.23    | MP2     |                                                         |

(continued)



Table S7. continued.

| Z                  | Atom             | State                      | $\alpha_D$ (a.u.) | $\delta$                                                | Method  | Comments                                                |
|--------------------|------------------|----------------------------|-------------------|---------------------------------------------------------|---------|---------------------------------------------------------|
| 85                 | At               | $^2P, M_L = \pm 1$         | $33.19 \pm 0.3$   | -0.11                                                   | CCSD    | $\Delta\alpha = -4.62$                                  |
|                    |                  | $^2P$                      | $34.73 \pm 2.88$  | 8.34                                                    |         |                                                         |
|                    |                  | $^2P, M_L = 0$             | 29.34             | -1.26                                                   |         |                                                         |
|                    |                  | $^2P, M_L = \pm 1$         | 32.93             | -0.89                                                   |         |                                                         |
|                    |                  | $^2P$                      | 31.73             | -1.01                                                   |         |                                                         |
|                    |                  | $^2P, M_L = 0$             | $29.72 \pm 0.11$  | --                                                      |         | $\Delta\alpha = 3.51$                                   |
|                    |                  | $^2P, M_L = \pm 1$         | $33.23 \pm 0.02$  | --                                                      |         |                                                         |
|                    |                  | $^2P$                      | $32.06 \pm 0.06$  | --                                                      |         |                                                         |
|                    |                  | $^2P_{3/2}, M_J = \pm 1/2$ | 29.92             |                                                         | MRCISD  | <a href="#">4C-DC-CI@dyall.acv4z@(core 17)[vir 215]</a> |
|                    |                  | $^2P_{3/2}, M_J = \pm 3/2$ | 32.63             |                                                         |         |                                                         |
|                    |                  | $^2P_{3/2}$                | 31.28             |                                                         |         |                                                         |
|                    |                  | $^2P_{1/2}$                | 32.01             |                                                         |         | $\bar{\alpha}_{J=3/2} - \alpha_{J=1/2} = -0.73$         |
|                    |                  | $^2P, M_L = 0$             | 37.85             | 1.42                                                    | DHF     | <a href="#">2C-NR-CC@dyall.acv4z@(core 49)[vir 295]</a> |
|                    |                  | $^2P, M_L = \pm 1$         | 40.94             | 0.86                                                    | MP2     | $\Delta\alpha = 3.09$                                   |
|                    |                  | $^2P$                      | 39.91             | 1.04                                                    |         |                                                         |
|                    |                  | $^2P, M_L = 0$             | $38.26 \pm 0.15$  | 2.51                                                    |         |                                                         |
|                    |                  | $^2P, M_L = \pm 1$         | $40.34 \pm 0.05$  | -0.64                                                   | CCSD    | $\Delta\alpha = 2.08$                                   |
|                    |                  | $^2P$                      | $39.64 \pm 0.1$   | 0.35                                                    |         |                                                         |
|                    |                  | $^2P, M_L = 0$             | 37.12             | -0.54                                                   |         |                                                         |
|                    |                  | $^2P, M_L = \pm 1$         | 40.31             | -0.70                                                   | CCSD(T) | $\Delta\alpha = 3.19$                                   |
|                    |                  | $^2P$                      | 39.25             | -0.65                                                   |         |                                                         |
|                    |                  | $^2P, M_L = 0$             | 37.32             | --                                                      |         |                                                         |
|                    |                  | $^2P, M_L = \pm 1$         | 40.59             | --                                                      |         | $\Delta\alpha = 3.27$                                   |
|                    |                  | $^2P$                      | 39.50             | --                                                      |         |                                                         |
| $^2P, M_L = 0$     | 34.70            | -0.34                      | DHF               | <a href="#">2C-SR-CC@dyall.acv4z@(core 17)[vir 261]</a> |         |                                                         |
| $^2P, M_L = \pm 1$ | 40.02            | -0.73                      | MP2               | $\Delta\alpha = 5.32$                                   |         |                                                         |
| $^2P$              | 38.25            | -0.61                      |                   |                                                         |         |                                                         |
| $^2P, M_L = 0$     | $35.42 \pm 0.03$ | 1.71                       |                   |                                                         |         |                                                         |
| $^2P, M_L = \pm 1$ | $39.69 \pm 0.03$ | -1.55                      | CCSD              | $\Delta\alpha = 4.27$                                   |         |                                                         |
| $^2P$              | $38.27 \pm 0.03$ | -0.57                      |                   |                                                         |         |                                                         |
| $^2P, M_L = 0$     | 34.56            | -0.76                      |                   |                                                         |         |                                                         |
| $^2P, M_L = \pm 1$ | 39.96            | -0.89                      | CCSD(T)           | $\Delta\alpha = 5.40$                                   |         |                                                         |
| $^2P$              | 38.16            | -0.85                      |                   |                                                         |         |                                                         |
| $^2P, M_L = 0$     | 34.82            | --                         |                   |                                                         |         |                                                         |
| $^2P, M_L = \pm 1$ | 40.32            | --                         |                   | $\Delta\alpha = 5.50$                                   |         |                                                         |
| $^2P$              | 38.48            | --                         |                   |                                                         |         |                                                         |
| $^2P, M_L = 0$     | 34.70            | -0.04                      |                   |                                                         | DHF     | <a href="#">2C-SR-CC@dyall.acv4z@(core 49)[vir 295]</a> |
| $^2P, M_L = \pm 1$ | 40.02            | -0.53                      |                   |                                                         |         |                                                         |

(continued)

Table S7. continued.

| Z   | Atom | State                      | $\alpha_D$ (a.u.) | $\delta$ | Method  | Comments                                                |
|-----|------|----------------------------|-------------------|----------|---------|---------------------------------------------------------|
|     |      | $^2P$                      | 38.25             | -0.38    | MP2     | $\Delta\alpha = 5.32$                                   |
|     |      | $^2P, M_L = 0$             | $35.57 \pm 0.07$  | 2.45     |         |                                                         |
|     |      | $^2P, M_L = \pm 1$         | $39.68 \pm 0.02$  | -1.38    |         |                                                         |
|     |      | $^2P$                      | $38.31 \pm 0.05$  | -0.22    | CCSD    | $\Delta\alpha = 4.11$                                   |
|     |      | $^2P, M_L = 0$             | 34.45             | -0.76    |         |                                                         |
|     |      | $^2P, M_L = \pm 1$         | 39.86             | -0.93    |         |                                                         |
|     |      | $^2P$                      | 38.06             | -0.88    | CCSD(T) | $\Delta\alpha = 5.41$                                   |
|     |      | $^2P, M_L = 0$             | 34.72             | --       |         |                                                         |
|     |      | $^2P, M_L = \pm 1$         | 40.23             | --       |         |                                                         |
|     |      | $^2P$                      | 38.39             | --       |         | $\Delta\alpha = 5.52$                                   |
|     |      | $^2P_{3/2}, M_J = \pm 1/2$ | 36.25             |          | MRCISD  | <a href="#">4C-DC-CI@dyall.acv4z@(core 17)[vir 261]</a> |
|     |      | $^2P_{3/2}, M_J = \pm 3/2$ | 41.59             |          |         |                                                         |
|     |      | $^2P_{3/2}$                | 38.92             |          |         |                                                         |
|     |      | $^2P_{1/2}$                | 40.79             |          |         | $\bar{\alpha}_{J=3/2} - \alpha_{J=1/2} = -1.87$         |
| 117 | Ts   | $^2P, M_L = 0$             | $53.67 \pm 0.02$  | 2.54     | DHF     | <a href="#">2C-NR-CC@dyall.acv4z@(core 49)[vir 293]</a> |
|     |      | $^2P, M_L = \pm 1$         | $50.56 \pm 0.02$  | 2.74     | MP2     |                                                         |
|     |      | $^2P$                      | $51.60 \pm 0.02$  | 2.67     |         | $\Delta\alpha = -3.10$                                  |
|     |      | $^2P, M_L = 0$             | $37.25 \pm 7.23$  | -28.83   | CCSD    |                                                         |
|     |      | $^2P, M_L = \pm 1$         | $48.83 \pm 0.54$  | -0.78    |         |                                                         |
|     |      | $^2P$                      | $44.97 \pm 4.2$   | -10.52   |         | $\Delta\alpha = 11.59$                                  |
|     |      | $^2P, M_L = 0$             | $52.38 \pm 0.02$  | 0.08     | CCSD(T) |                                                         |
|     |      | $^2P, M_L = \pm 1$         | $49.17 \pm 0.01$  | -0.10    |         |                                                         |
|     |      | $^2P$                      | $50.24 \pm 0.01$  | -0.04    |         | $\Delta\alpha = -3.21$                                  |
|     |      | $^2P, M_L = 0$             | $52.34 \pm 0.16$  | --       |         |                                                         |
|     |      | $^2P, M_L = \pm 1$         | $49.22 \pm 0.09$  | --       |         |                                                         |
|     |      | $^2P$                      | $50.26 \pm 0.12$  | --       |         | $\Delta\alpha = -3.12$                                  |
|     |      | $^2P, M_L = 0$             | 44.00             | 1.98     | DHF     | <a href="#">2C-SR-CC@dyall.acv4z@(core 17)[vir 247]</a> |
|     |      | $^2P, M_L = \pm 1$         | 53.31             | -0.37    | MP2     |                                                         |
|     |      | $^2P$                      | 50.21             | 0.30     |         | $\Delta\alpha = 9.31$                                   |
|     |      | $^2P, M_L = 0$             | $38.97 \pm 1.41$  | -9.68    | CCSD    |                                                         |
|     |      | $^2P, M_L = \pm 1$         | $56.70 \pm 2.14$  | 5.96     |         |                                                         |
|     |      | $^2P$                      | $50.79 \pm 1.93$  | 1.46     |         | $\Delta\alpha = 17.73$                                  |
|     |      | $^2P, M_L = 0$             | 43.87             | 1.68     | CCSD(T) |                                                         |
|     |      | $^2P, M_L = \pm 1$         | 52.99             | -0.98    |         |                                                         |
|     |      | $^2P$                      | 49.95             | -0.22    |         | $\Delta\alpha = 9.12$                                   |
|     |      | $^2P, M_L = 0$             | $43.15 \pm 0.6$   | --       |         |                                                         |
|     |      | $^2P, M_L = \pm 1$         | $53.51 \pm 0.04$  | --       |         |                                                         |
|     |      | $^2P$                      | $50.06 \pm 0.35$  | --       |         | $\Delta\alpha = 10.37$                                  |

(continued)

Table S7. continued.

| Z | Atom | State                      | $\alpha_D$ (a.u.) | $\delta$ | Method  | Comments                                                |
|---|------|----------------------------|-------------------|----------|---------|---------------------------------------------------------|
|   |      | $^2P, M_L = 0$             | 44.00             | 2.47     | DHF     | <a href="#">2C-SR-CC@dyall.acv4z@(core 49)[vir 293]</a> |
|   |      | $^2P, M_L = \pm 1$         | 53.31             | -0.15    |         |                                                         |
|   |      | $^2P$                      | 50.21             | 0.60     |         | $\Delta\alpha = 9.31$                                   |
|   |      | $^2P, M_L = 0$             | $38.02 \pm 2.09$  | -11.46   | MP2     |                                                         |
|   |      | $^2P, M_L = \pm 1$         | $58.99 \pm 3.85$  | 10.48    |         |                                                         |
|   |      | $^2P$                      | $52.00 \pm 3.37$  | 4.19     |         | $\Delta\alpha = 20.97$                                  |
|   |      | $^2P, M_L = 0$             | 43.69             | 1.75     | CCSD    |                                                         |
|   |      | $^2P, M_L = \pm 1$         | 52.77             | -1.16    |         |                                                         |
|   |      | $^2P$                      | 49.74             | -0.33    |         | $\Delta\alpha = 9.08$                                   |
|   |      | $^2P, M_L = 0$             | $42.94 \pm 0.6$   | --       | CCSD(T) |                                                         |
|   |      | $^2P, M_L = \pm 1$         | $53.39 \pm 0.09$  | --       |         |                                                         |
|   |      | $^2P$                      | $49.91 \pm 0.35$  | --       |         | $\Delta\alpha = 10.45$                                  |
|   |      | $^2P_{3/2}, M_J = \pm 1/2$ | 58.40             |          | MRCISD  | <a href="#">4C-DC-CI@dyall.acv4z@(core 17)[vir 247]</a> |
|   |      | $^2P_{3/2}, M_J = \pm 3/2$ | 71.89             |          |         |                                                         |
|   |      | $^2P_{3/2}$                | 65.15             |          |         |                                                         |
|   |      | $^2P_{1/2}$                | 227.28            |          |         | $\bar{\alpha}_{J=3/2} - \alpha_{J=1/2} = -162.14$       |

## S1.8 Group 18 elements

Table S8: The results of dipole polarizability for Group 18 elements.

| Z | Atom | State          | $\alpha_D$ (a.u.) | $\delta$ (%) | Method  | Comments                                               |
|---|------|----------------|-------------------|--------------|---------|--------------------------------------------------------|
| 2 | He   | $^1S, M_L = 0$ | 1.32              | -4.50        | DHF     | <a href="#">2C-NR-CC@dyall.acv4z@(core 2)[vir 104]</a> |
|   |      |                | 1.36              | -1.73        | MP2     |                                                        |
|   |      |                | 1.38              | 0.00         | CCSD    |                                                        |
|   |      |                | 1.38              | --           | CCSD(T) |                                                        |
|   |      | $^1S, M_L = 0$ | 1.32              | -4.50        | DHF     | <a href="#">2C-SR-CC@dyall.acv4z@(core 2)[vir 104]</a> |
|   |      |                | 1.36              | -1.73        | MP2     |                                                        |
|   |      |                | 1.38              | 0.00         | CCSD    |                                                        |
|   |      |                | 1.38              | --           | CCSD(T) |                                                        |
|   |      | $^1S_0$        | 1.32              | -4.50        | DHF     | <a href="#">4C-DC-CC@dyall.acv4z@(core 2)[vir 104]</a> |
|   |      |                | 1.36              | -1.73        | MP2     |                                                        |
|   |      |                | 1.38              | 0.00         | CCSD    |                                                        |
|   |      |                | 1.38              | --           | CCSD(T) |                                                        |

(continued)

Table S8. continued.

| Z  | Atom | State          | $\alpha_D$ (a.u.) | $\delta$ | Method  | Comments                                                |
|----|------|----------------|-------------------|----------|---------|---------------------------------------------------------|
| 10 | Ne   | $^1S, M_L = 0$ | 2.31              | -9.97    | DHF     | <a href="#">2C-NR-CC@dyall.acv4z@(core 10)[vir 246]</a> |
|    |      |                | 2.59              | 1.01     | MP2     |                                                         |
|    |      |                | 2.53              | -1.60    | CCSD    |                                                         |
|    |      |                | 2.57              | --       | CCSD(T) |                                                         |
|    |      | $^1S, M_L = 0$ | 2.32              | -10.00   | DHF     | <a href="#">2C-SR-CC@dyall.acv4z@(core 10)[vir 246]</a> |
|    |      |                | 2.60              | 1.02     | MP2     |                                                         |
|    |      |                | 2.53              | -1.60    | CCSD    |                                                         |
|    |      |                | 2.57              | --       | CCSD(T) |                                                         |
|    |      | $^1S_0$        | 2.32              | -9.99    | DHF     | 2C-DC-CC@dyall.acv4z@(core 10)[vir 246]                 |
|    |      |                | 2.60              | 1.02     | MP2     |                                                         |
|    |      |                | 2.53              | -1.60    | CCSD    |                                                         |
|    |      |                | 2.57              | --       | CCSD(T) |                                                         |
|    |      | $^1S_0$        | 2.32              | -9.99    | DHF     | <a href="#">4C-DC-CC@dyall.acv4z@(core 10)[vir 246]</a> |
|    |      |                | 2.60              | 1.02     | MP2     |                                                         |
|    |      |                | 2.53              | -1.60    | CCSD    |                                                         |
|    |      |                | 2.57              | --       | CCSD(T) |                                                         |
| 18 | Ar   | $^1S, M_L = 0$ | 10.71             | -2.68    | DHF     | <a href="#">2C-NR-CC@dyall.acv4z@(core 18)[vir 358]</a> |
|    |      |                | 11.04             | 0.28     | MP2     |                                                         |
|    |      |                | 10.91             | -0.87    | CCSD    |                                                         |
|    |      |                | 11.01             | --       | CCSD(T) |                                                         |
|    |      | $^1S, M_L = 0$ | 10.72             | -2.71    | DHF     | <a href="#">2C-SR-CC@dyall.acv4z@(core 18)[vir 358]</a> |
|    |      |                | 11.06             | 0.28     | MP2     |                                                         |
|    |      |                | 10.93             | -0.88    | CCSD    |                                                         |
|    |      |                | 11.02             | --       | CCSD(T) |                                                         |
|    |      | $^1S_0$        | 10.73             | -2.71    | DHF     | 2C-DC-CC@dyall.acv4z@(core 18)[vir 358]                 |
|    |      |                | 11.06             | 0.29     | MP2     |                                                         |
|    |      |                | 10.93             | -0.88    | CCSD    |                                                         |
|    |      |                | 11.03             | --       | CCSD(T) |                                                         |
|    |      | $^1S_0$        | 10.73             | -2.71    | DHF     | <a href="#">4C-DC-CC@dyall.acv4z@(core 18)[vir 358]</a> |
|    |      |                | 11.06             | 0.28     | MP2     |                                                         |
|    |      |                | 10.93             | -0.88    | CCSD    |                                                         |
|    |      |                | 11.02             | --       | CCSD(T) |                                                         |
| 36 | Kr   | $^1S, M_L = 0$ | 16.46             | -1.87    | DHF     | <a href="#">2C-NR-CC@dyall.acv4z@(core 36)[vir 476]</a> |
|    |      |                | 16.75             | -0.15    | MP2     |                                                         |
|    |      |                | 16.64             | -0.82    | CCSD    |                                                         |
|    |      |                | 16.78             | --       | CCSD(T) |                                                         |
|    |      | $^1S, M_L = 0$ | 16.44             | -1.93    | DHF     | 2C-SR-CC@d-aug-dyall.acv4z@(core 36)[vir 620]           |
|    |      |                | 16.74             | -0.14    | MP2     |                                                         |
|    |      |                |                   |          |         |                                                         |
|    |      |                |                   |          |         |                                                         |

(continued)

Table S8. continued.

| Z  | Atom | State          | $\alpha_D$ (a.u.) | $\delta$ | Method  | Comments                                                |
|----|------|----------------|-------------------|----------|---------|---------------------------------------------------------|
|    |      | $^1S, M_L = 0$ | 16.62             | -0.86    | CCSD    |                                                         |
|    |      |                | 16.76             | --       | CCSD(T) |                                                         |
|    |      |                | 16.43             | -2.04    | DHF     | <a href="#">2C-SR-CC@dyall.acv4z@(core 36)[vir 476]</a> |
|    |      |                | 16.74             | -0.15    | MP2     |                                                         |
|    |      |                | 16.63             | -0.84    | CCSD    |                                                         |
|    |      |                | 16.77             | --       | CCSD(T) |                                                         |
|    |      | $^1S_0$        | 16.46             | -2.03    | DHF     | <a href="#">2C-DC-CC@dyall.acv4z@(core 36)[vir 476]</a> |
|    |      |                | 16.77             | -0.15    | MP2     |                                                         |
|    |      |                | 16.66             | -0.84    | CCSD    |                                                         |
|    |      |                | 16.80             | --       | CCSD(T) |                                                         |
|    |      | $^1S_0$        | 16.45             | -2.15    | DHF     | 4C-DC-CC@dyall.acv4z@(core 26)[vir 232]                 |
|    |      |                | 16.79             | -0.15    | MP2     |                                                         |
|    |      |                | 16.68             | -0.83    | CCSD    |                                                         |
|    |      |                | 16.81             | --       | CCSD(T) |                                                         |
| 54 | Xe   | $^1S, M_L = 0$ | 27.09 $\pm$ 0.01  | -0.50    | DHF     | <a href="#">2C-NR-CC@dyall.acv4z@(core 26)[vir 286]</a> |
|    |      |                | 27.12 $\pm$ 0.01  | -0.38    | MP2     |                                                         |
|    |      |                | 27.04 $\pm$ 0.01  | -0.70    | CCSD    |                                                         |
|    |      |                | 27.23 $\pm$ 0.01  | --       | CCSD(T) |                                                         |
|    |      | $^1S, M_L = 0$ | 26.76             | -0.94    | DHF     | 2C-SR-CC@d-aug-dyall.acv4z@(core 26)[vir 430]           |
|    |      |                | 26.93             | -0.31    | MP2     |                                                         |
|    |      |                | 26.80             | -0.79    | CCSD    |                                                         |
|    |      |                | 27.01             | --       | CCSD(T) |                                                         |
|    |      | $^1S, M_L = 0$ | 26.76             | -0.95    | DHF     | 2C-SR-CC@d-aug-dyall.acv4z@(core 50)[vir 430]           |
|    |      |                | 26.92             | -0.34    | MP2     |                                                         |
|    |      |                | 26.80             | -0.79    | CCSD    |                                                         |
|    |      |                | 27.02             | --       | CCSD(T) |                                                         |
|    |      | $^1S, M_L = 0$ | 26.75             | -0.96    | DHF     | <a href="#">2C-SR-CC@dyall.acv4z@(core 26)[vir 286]</a> |
|    |      |                | 26.91             | -0.34    | MP2     |                                                         |
|    |      |                | 26.80             | -0.77    | CCSD    |                                                         |
|    |      |                | 27.01             | --       | CCSD(T) |                                                         |
|    |      | $^1S_0$        | 26.96             | -0.90    | DHF     | 2C-DC-CC@dyall.acv4z@(core 50)[vir 286]                 |
|    |      |                | 27.10             | -0.37    | MP2     |                                                         |
|    |      |                | 27.00             | -0.76    | CCSD    |                                                         |
|    |      |                | 27.21             | --       | CCSD(T) |                                                         |
|    |      | $^1S_0$        | 26.96             | -2.36    | DHF     | 2C-DC-CC@dyall.acv4z@(core 8)[vir 286]                  |
|    |      |                | 27.64             | 0.10     | MP2     |                                                         |
|    |      |                | 27.43             | -0.66    | CCSD    |                                                         |
|    |      |                | 27.61             | --       | CCSD(T) |                                                         |

(continued)

Table S8. continued.

| Z   | Atom | State          | $\alpha_D$ (a.u.) | $\delta$ | Method  | Comments                                       |
|-----|------|----------------|-------------------|----------|---------|------------------------------------------------|
| 86  | Rn   | $^1S_0$        | 26.95             | -0.91    | DHF     | <b>4C-DC-CC@dyall.acv4z@(core 50)[vir 286]</b> |
|     |      |                | 27.10             | -0.36    | MP2     |                                                |
|     |      |                | 27.00             | -0.76    | CCSD    |                                                |
|     |      |                | 27.20             | --       | CCSD(T) |                                                |
|     |      | $^1S, M_L = 0$ | $34.14 \pm 0.01$  | 0.16     | DHF     | <b>2C-NR-CC@dyall.acv4z@(core 50)[vir 294]</b> |
|     |      |                | $33.93 \pm 0.01$  | -0.46    | MP2     |                                                |
|     |      |                | $33.85 \pm 0.01$  | -0.69    | CCSD    |                                                |
|     |      |                | $34.08 \pm 0.01$  | --       | CCSD(T) |                                                |
|     |      | $^1S, M_L = 0$ | 32.78             | -1.15    | DHF     | 2C-SR-CC@d-aug-dyall.acv4z@(core 40)[vir 438]  |
|     |      |                | 33.11             | -0.15    | MP2     |                                                |
|     |      |                | 32.87             | -0.88    | CCSD    |                                                |
|     |      |                | 33.16             | --       | CCSD(T) |                                                |
|     |      | $^1S, M_L = 0$ | 32.77             | -1.14    | DHF     | 2C-SR-CC@dyall.acv4z@(core 40)[vir 294]        |
|     |      |                | 33.08             | -0.22    | MP2     |                                                |
|     |      |                | 32.87             | -0.86    | CCSD    |                                                |
|     |      |                | 33.15             | --       | CCSD(T) |                                                |
|     |      | $^1S, M_L = 0$ | 32.77             | -1.03    | DHF     | <b>2C-SR-CC@dyall.acv4z@(core 50)[vir 294]</b> |
|     |      |                | 33.02             | -0.28    | MP2     |                                                |
|     |      |                | 32.83             | -0.86    | CCSD    |                                                |
|     |      |                | 33.12             | --       | CCSD(T) |                                                |
|     |      | $^1S_0$        | 34.98             | -0.37    | DHF     | 2C-DC-CC@dyall.acv4z@(core 18)[vir 294]        |
|     |      |                | 34.99             | -0.35    | MP2     |                                                |
|     |      |                | 34.85             | -0.73    | CCSD    |                                                |
|     |      |                | 35.11             | --       | CCSD(T) |                                                |
|     |      | $^1S_0$        | 34.98             | -0.33    | DHF     | 2C-DC-CC@dyall.acv4z@(core 50)[vir 294]        |
|     |      |                | 34.94             | -0.44    | MP2     |                                                |
|     |      |                | 34.84             | -0.74    | CCSD    |                                                |
|     |      |                | 35.10             | --       | CCSD(T) |                                                |
|     |      | $^1S_0$        | 34.96             | -0.32    | DHF     | <b>4C-DC-CC@dyall.acv4z@(core 50)[vir 294]</b> |
|     |      |                | 34.90             | -0.48    | MP2     |                                                |
|     |      |                | 34.81             | -0.74    | CCSD    |                                                |
|     |      |                | 35.07             | --       | CCSD(T) |                                                |
| 118 | Og   | $^1S, M_L = 0$ | $45.60 \pm 0.02$  | 0.77     | DHF     | <b>2C-NR-CC@dyall.acv4z@(core 50)[vir 278]</b> |
|     |      |                | $45.01 \pm 0.02$  | -0.55    | MP2     |                                                |
|     |      |                | $44.97 \pm 0.02$  | -0.63    | CCSD    |                                                |
|     |      |                | $45.26 \pm 0.02$  | --       | CCSD(T) |                                                |
|     |      | $^1S, M_L = 0$ | 43.59             | -0.05    | DHF     | 2C-SR-CC@d-aug-dyall.acv4z@(core 50)[vir 422]  |
|     |      |                | 43.47             | -0.33    | MP2     |                                                |

(continued)

Table S8. continued.

| Z | Atom | State          | $\alpha_D$ (a.u.) | $\delta$ | Method  | Comments                                       |
|---|------|----------------|-------------------|----------|---------|------------------------------------------------|
|   |      |                | 43.28             | -0.75    | CCSD    |                                                |
|   |      |                | 43.61             | --       | CCSD(T) |                                                |
|   |      | $^1S, M_L = 0$ | 43.55             | -0.43    | DHF     | <b>2C-SR-CC@dyall.acv4z@(core 50)[vir 278]</b> |
|   |      |                | 43.52             | -0.49    | MP2     |                                                |
|   |      |                | 43.41             | -0.76    | CCSD    |                                                |
|   |      |                | 43.74             | --       | CCSD(T) |                                                |
|   |      | $^1S_0$        | 60.58             | 4.66     | DHF     | 2C-DC-CC@dyall.acv4z@(core 18)[vir 278]        |
|   |      |                | 56.21             | -2.90    | MP2     |                                                |
|   |      |                | 57.86             | -0.04    | CCSD    |                                                |
|   |      |                | 57.88             | --       | CCSD(T) |                                                |
|   |      | $^1S_0$        | 60.58             | 4.00     | DHF     | 2C-DC-CC@dyall.acv4z@(core 40)[vir 278]        |
|   |      |                | 55.90             | -4.03    | MP2     |                                                |
|   |      |                | 58.20             | -0.09    | CCSD    |                                                |
|   |      |                | 58.25             | --       | CCSD(T) |                                                |
|   |      | $^1S_0$        | 60.44             | 4.00     | DHF     | 2C-DC-Gaunt-CC@dyall.acv4z@(core 50)[vir 278]  |
|   |      |                | 55.68             | -4.19    | MP2     |                                                |
|   |      |                | 58.06             | -0.10    | CCSD    |                                                |
|   |      |                | 58.12             | --       | CCSD(T) |                                                |
|   |      | $^1S_0$        | 60.59             | 4.05     | DHF     | <b>4C-DC-CC@dyall.acv4z@(core 50)[vir 278]</b> |
|   |      |                | 55.78             | -4.22    | MP2     |                                                |
|   |      |                | 58.18             | -0.09    | CCSD    |                                                |
|   |      |                | 58.24             | --       | CCSD(T) |                                                |

## S2 Data obtained by fitting Eq. (S3)

In the following tables, the results with highlighted identifiers are used to obtain the most accurate results in this work, as shown in the main text. The identifiers with “NR-CC”, “SR-CC”, “DC-CC”, and “DC-CI” are highlighted in teal, blue, red, and green, respectively. Additional test results are also included for reliable estimates and basis set choices.

### S2.1 Group 1 elements

Table S9: The results of dipole polarizability for Group 1 elements.

| <b>Z</b> | <b>Atom</b> | <b>State</b>   | $\alpha_D$ (a.u.) | $\delta$ (%) | <b>Method</b> | <b>Comments</b>                                  |
|----------|-------------|----------------|-------------------|--------------|---------------|--------------------------------------------------|
| 3        | Li          | $^2S, M_L = 0$ | 170.12            | 3.51         | DHF           | <b>2C-NR-CC@s-aug-ANO-RCC@(core 3)[vir 229]</b>  |
|          |             |                | 165.01 $\pm$ 0.01 | 0.40         | MP2           |                                                  |
|          |             |                | 164.45            | 0.06         | CCSD          |                                                  |
|          |             |                | 164.35            | --           | CCSD(T)       |                                                  |
|          |             | $^2S, M_L = 0$ | 170.07            | 3.51         | DHF           | 2C-SR-CC@ANO-RCC@(core 3)[vir 179]               |
|          |             |                | 165.04            | 0.45         | MP2           |                                                  |
|          |             |                | 164.41            | 0.06         | CCSD          |                                                  |
|          |             |                | 164.30            | --           | CCSD(T)       |                                                  |
|          |             | $^2S, M_L = 0$ | 170.06            | 3.51         | DHF           | 2C-SR-CC@d-aug-ANO-RCC@(core 3)[vir 279]         |
|          |             |                | 164.88 $\pm$ 0.02 | 0.36         | MP2           |                                                  |
|          |             |                | 164.40            | 0.06         | CCSD          |                                                  |
|          |             |                | 164.29            | --           | CCSD(T)       |                                                  |
|          |             | $^2S, M_L = 0$ | 170.06            | 3.51         | DHF           | <b>2C-SR-CC@s-aug-ANO-RCC@(core 3)[vir 229]</b>  |
|          |             |                | 164.95 $\pm$ 0.01 | 0.40         | MP2           |                                                  |
|          |             |                | 164.40            | 0.06         | CCSD          |                                                  |
|          |             |                | 164.30            | --           | CCSD(T)       |                                                  |
|          |             | $^2S_{1/2}$    | 170.05            | 3.50         | DHF           | <b>4C-DC-CC@s-aug-ANO-RCC@(core 3)[vir 229]</b>  |
|          |             |                | 165.75 $\pm$ 0.34 | 0.89         | MP2           |                                                  |
|          |             |                | 164.39            | 0.06         | CCSD          |                                                  |
|          |             |                | 164.30            | --           | CCSD(T)       |                                                  |
| 11       | Na          | $^2S, M_L = 0$ | 190.77 $\pm$ 0.04 | 16.14        | DHF           | <b>2C-NR-CC@s-aug-ANO-RCC@(core 11)[vir 287]</b> |
|          |             |                | 164.51 $\pm$ 0.03 | 0.15         | MP2           |                                                  |
|          |             |                | 165.68 $\pm$ 0.04 | 0.87         | CCSD          |                                                  |
|          |             |                | 164.25 $\pm$ 0.04 | --           | CCSD(T)       |                                                  |
|          |             | $^2S, M_L = 0$ | 189.41            | 16.14        | DHF           | 2C-SR-CC@ANO-RCC@(core 11)[vir 237]              |
|          |             |                | 163.40 $\pm$ 0.01 | 0.19         | MP2           |                                                  |
|          |             |                | 164.50 $\pm$ 0.01 | 0.87         | CCSD          |                                                  |
|          |             |                | 163.08 $\pm$ 0.01 | --           | CCSD(T)       |                                                  |
|          |             | $^2S, M_L = 0$ | 189.71 $\pm$ 0.04 | 16.21        | DHF           | 2C-SR-CC@d-aug-ANO-RCC@(core 11)[vir 337]        |
|          |             |                | 163.32 $\pm$ 0.08 | 0.04         | MP2           |                                                  |
|          |             |                | 164.68 $\pm$ 0.04 | 0.88         | CCSD          |                                                  |
|          |             |                | 163.25 $\pm$ 0.04 | --           | CCSD(T)       |                                                  |
|          |             | $^2S, M_L = 0$ | 189.70 $\pm$ 0.04 | 16.20        | DHF           | <b>2C-SR-CC@s-aug-ANO-RCC@(core 11)[vir 287]</b> |
|          |             |                | 163.50 $\pm$ 0.03 | 0.15         | MP2           |                                                  |
|          |             |                | 164.68 $\pm$ 0.04 | 0.87         | CCSD          |                                                  |
|          |             |                | 163.26 $\pm$ 0.04 | --           | CCSD(T)       |                                                  |
|          |             | $^2S_{1/2}$    | 189.66 $\pm$ 0.04 | 16.11        | DHF           | <b>4C-DC-CC@s-aug-ANO-RCC@(core 11)[vir 287]</b> |

(continued)



Table S9. continued.

| Z  | Atom | State          | $\alpha_D$ (a.u.) | $\delta$ | Method  | Comments                                         |
|----|------|----------------|-------------------|----------|---------|--------------------------------------------------|
| 19 | K    | $^2S, M_L = 0$ | $167.17 \pm 1.06$ | 2.34     | MP2     | <b>2C-NR-CC@s-aug-ANO-RCC@(core 19)[vir 311]</b> |
|    |      |                | $164.65 \pm 0.04$ | 0.80     | CCSD    |                                                  |
|    |      |                | $163.35 \pm 0.02$ | --       | CCSD(T) |                                                  |
|    |      |                |                   |          |         |                                                  |
|    |      | $^2S, M_L = 0$ | $414.12 \pm 0.59$ | 40.53    | DHF     | 2C-SR-CC@ANO-RCC@(core 19)[vir 261]              |
|    |      |                | $268.66 \pm 0.23$ | -8.83    | MP2     |                                                  |
|    |      |                | $307.52 \pm 0.2$  | 4.35     | CCSD    |                                                  |
|    |      |                | $294.69 \pm 0.13$ | --       | CCSD(T) |                                                  |
|    |      | $^2S, M_L = 0$ | $404.41 \pm 0.65$ | 42.56    | DHF     | 2C-SR-CC@d-aug-ANO-RCC@(core 19)[vir 361]        |
|    |      |                | $258.24 \pm 0.25$ | -8.97    | MP2     |                                                  |
|    |      |                | $296.50 \pm 0.21$ | 4.52     | CCSD    |                                                  |
|    |      |                | $283.67 \pm 0.15$ | --       | CCSD(T) |                                                  |
|    |      | $^2S, M_L = 0$ | $410.09 \pm 0.07$ | 40.93    | DHF     | <b>2C-SR-CC@s-aug-ANO-RCC@(core 19)[vir 311]</b> |
|    |      |                | $263.16 \pm 0.14$ | -9.57    | MP2     |                                                  |
|    |      |                | 303.81            | 4.40     | CCSD    |                                                  |
|    |      |                | $291.00 \pm 0.01$ | --       | CCSD(T) |                                                  |
|    |      | $^2S_{1/2}$    | $406.80 \pm 0.55$ | 40.68    | DHF     | <b>4C-DC-CC@s-aug-ANO-RCC@(core 19)[vir 311]</b> |
|    |      |                | $263.27 \pm 0.23$ | -8.95    | MP2     |                                                  |
|    |      |                | $301.77 \pm 0.18$ | 4.36     | CCSD    |                                                  |
|    |      |                | $289.16 \pm 0.12$ | --       | CCSD(T) |                                                  |
| 37 | Rb   | $^2S, M_L = 0$ | $519.28 \pm 0.9$  | 50.93    | DHF     | <b>2C-NR-CC@s-aug-ANO-RCC@(core 27)[vir 247]</b> |
|    |      |                | $291.75 \pm 0.91$ | -15.20   | MP2     |                                                  |
|    |      |                | $364.17 \pm 0.22$ | 5.85     | CCSD    |                                                  |
|    |      |                | $344.06 \pm 0.09$ | --       | CCSD(T) |                                                  |
|    |      | $^2S, M_L = 0$ | $479.42 \pm 0.9$  | 52.99    | DHF     | 2C-SR-CC@ANO-RCC@(core 27)[vir 197]              |
|    |      |                | $263.19 \pm 0.7$  | -16.01   | MP2     |                                                  |
|    |      |                | $332.21 \pm 0.24$ | 6.01     | CCSD    |                                                  |
|    |      |                | $313.37 \pm 0.13$ | --       | CCSD(T) |                                                  |
|    |      | $^2S, M_L = 0$ | $485.67 \pm 0.09$ | 51.31    | DHF     | 2C-SR-CC@d-aug-ANO-RCC@(core 27)[vir 297]        |
|    |      |                | $269.77 \pm 0.8$  | -15.95   | MP2     |                                                  |
|    |      |                | $339.67 \pm 0.11$ | 5.82     | CCSD    |                                                  |
|    |      |                | $320.98 \pm 0.17$ | --       | CCSD(T) |                                                  |
|    |      | $^2S, M_L = 0$ | $481.73 \pm 0.68$ | 51.02    | DHF     | <b>2C-SR-CC@s-aug-ANO-RCC@(core 27)[vir 247]</b> |
|    |      |                | $269.04 \pm 0.77$ | -15.66   | MP2     |                                                  |
|    |      |                | $337.45 \pm 0.15$ | 5.78     | CCSD    |                                                  |

(continued)

Table S9. continued.

| Z              | Atom              | State          | $\alpha_D$ (a.u.) | $\delta$       | Method            | Comments                                         |         |                                                  |
|----------------|-------------------|----------------|-------------------|----------------|-------------------|--------------------------------------------------|---------|--------------------------------------------------|
|                |                   | $^2S_{1/2}$    | 318.99 $\pm$ 0.05 | --             | CCSD(T)           |                                                  |         |                                                  |
|                |                   |                | 481.26 $\pm$ 0.68 | 50.82          | DHF               | <b>4C-DC-CC@s-aug-ANO-RCC@(core 27)[vir 247]</b> |         |                                                  |
|                |                   |                | 279.66 $\pm$ 2.34 | -12.36         | MP2               |                                                  |         |                                                  |
|                |                   |                | 337.12 $\pm$ 0.16 | 5.65           | CCSD              |                                                  |         |                                                  |
|                |                   |                | 319.08 $\pm$ 0.17 | --             | CCSD(T)           |                                                  |         |                                                  |
| 55             | Cs                | $^2S, M_L = 0$ | 808.27 $\pm$ 0.08 | 68.69          | DHF               | <b>2C-NR-CC@s-aug-ANO-RCC@(core 27)[vir 259]</b> |         |                                                  |
|                |                   |                | 343.66 $\pm$ 3.06 | -28.28         | MP2               |                                                  |         |                                                  |
|                |                   |                | 523.17 $\pm$ 0.46 | 9.18           | CCSD              |                                                  |         |                                                  |
|                |                   |                | 479.16 $\pm$ 0.67 | --             | CCSD(T)           |                                                  |         |                                                  |
|                |                   | $^2S, M_L = 0$ | 672.86 $\pm$ 0.36 | 67.89          | DHF               | <b>2C-SR-CC@s-aug-ANO-RCC@(core 27)[vir 259]</b> |         |                                                  |
|                |                   |                | 282.15 $\pm$ 1.86 | -29.60         | MP2               |                                                  |         |                                                  |
|                |                   |                | 435.90 $\pm$ 0.43 | 8.77           | CCSD              |                                                  |         |                                                  |
|                |                   |                | 400.77 $\pm$ 0.52 | --             | CCSD(T)           |                                                  |         |                                                  |
|                |                   | $^2S_{1/2}$    | 671.35 $\pm$ 0.39 | 67.60          | DHF               | 4C-DC-CC@d-aug-ANO-RCC@(core 27)[vir 309]        |         |                                                  |
|                |                   |                | 294.22 $\pm$ 2.25 | -26.55         | MP2               |                                                  |         |                                                  |
|                |                   |                | 434.98 $\pm$ 0.44 | 8.59           | CCSD              |                                                  |         |                                                  |
|                |                   |                | 400.57 $\pm$ 0.38 | --             | CCSD(T)           |                                                  |         |                                                  |
|                |                   | $^2S_{1/2}$    | 665.51 $\pm$ 0.51 | 66.17          | DHF               | 4C-DC-CC@faegri@(core 27)[vir 299]               |         |                                                  |
|                |                   |                | 291.84 $\pm$ 3.3  | -27.13         | MP2               |                                                  |         |                                                  |
|                |                   |                | 436.80 $\pm$ 0.12 | 9.06           | CCSD              |                                                  |         |                                                  |
|                |                   |                | 400.51 $\pm$ 0.2  | --             | CCSD(T)           |                                                  |         |                                                  |
|                |                   | $^2S_{1/2}$    | 671.22 $\pm$ 0.35 | 67.56          | DHF               | <b>4C-DC-CC@s-aug-ANO-RCC@(core 27)[vir 259]</b> |         |                                                  |
|                |                   |                | 296.32 $\pm$ 2.64 | -26.03         | MP2               |                                                  |         |                                                  |
|                |                   |                | 434.92 $\pm$ 0.43 | 8.57           | CCSD              |                                                  |         |                                                  |
|                |                   |                | 400.60 $\pm$ 0.37 | --             | CCSD(T)           |                                                  |         |                                                  |
|                |                   | 87             | Fr                | $^2S, M_L = 0$ | 965.99 $\pm$ 0.36 | 76.12                                            | DHF     | <b>2C-NR-CC@s-aug-ANO-RCC@(core 41)[vir 217]</b> |
|                |                   |                |                   |                | 349.62 $\pm$ 5.43 | -36.26                                           | MP2     |                                                  |
|                |                   |                |                   |                | 608.79 $\pm$ 0.61 | 10.99                                            | CCSD    |                                                  |
|                |                   |                |                   |                | 548.49 $\pm$ 1.06 | --                                               | CCSD(T) |                                                  |
|                |                   |                |                   | $^2S, M_L = 0$ | 540.40 $\pm$ 0.08 | 68.53                                            | DHF     | 2C-SR-CC@ANO-RCC@(core 41)[vir 185]              |
|                |                   |                |                   |                | 201.52 $\pm$ 1.2  | -37.15                                           | MP2     |                                                  |
|                |                   |                |                   |                | 348.70 $\pm$ 0.2  | 8.74                                             | CCSD    |                                                  |
|                |                   |                |                   |                | 320.66 $\pm$ 0.27 | --                                               | CCSD(T) |                                                  |
| $^2S, M_L = 0$ | 544.62 $\pm$ 0.75 |                |                   | 69.16          | DHF               | 2C-SR-CC@d-aug-ANO-RCC@(core 41)[vir 249]        |         |                                                  |
|                | 198.57 $\pm$ 1.17 |                |                   | -38.32         | MP2               |                                                  |         |                                                  |
|                | 350.52 $\pm$ 0.43 |                |                   | 8.87           | CCSD              |                                                  |         |                                                  |
|                | 321.96 $\pm$ 0.42 |                |                   | --             | CCSD(T)           |                                                  |         |                                                  |
| $^2S, M_L = 0$ | 544.47 $\pm$ 0.72 |                |                   | 69.09          | DHF               | <b>2C-SR-CC@s-aug-ANO-RCC@(core 41)[vir 217]</b> |         |                                                  |

(continued)

Table S9. continued.

| Z | Atom | State       | $\alpha_D$ (a.u.) | $\delta$ | Method  | Comments                                         |
|---|------|-------------|-------------------|----------|---------|--------------------------------------------------|
|   |      |             | $200.05 \pm 0.9$  | -37.87   | MP2     |                                                  |
|   |      |             | $350.49 \pm 0.42$ | 8.84     | CCSD    |                                                  |
|   |      |             | $322.01 \pm 0.41$ | --       | CCSD(T) |                                                  |
|   |      | $^2S_{1/2}$ | $534.59 \pm 0.68$ | 67.50    | DHF     | <b>4C-DC-CC@s-aug-ANO-RCC@(core 41)[vir 217]</b> |
|   |      |             | $213.69 \pm 3.51$ | -33.05   | MP2     |                                                  |
|   |      |             | $346.13 \pm 0.4$  | 8.45     | CCSD    |                                                  |
|   |      |             | $319.16 \pm 0.3$  | --       | CCSD(T) |                                                  |

## S2.2 Group 2 elements

Table S10: The results of dipole polarizability for Group 2 elements.

| Z | Atom | State          | $\alpha_D$ (a.u.) | $\delta$ (%) | Method  | Comments                                           |
|---|------|----------------|-------------------|--------------|---------|----------------------------------------------------|
| 4 | Be   | $^1S, M_L = 0$ | $45.70 \pm 0.01$  | 20.68        | DHF     | <b>2C-NR-CC@d-aug-dyall.cv4z@(core 4)[vir 266]</b> |
|   |      |                | $42.17 \pm 0.01$  | 11.36        | MP2     |                                                    |
|   |      |                | $38.03 \pm 0.01$  | 0.42         | CCSD    |                                                    |
|   |      |                | $37.87 \pm 0.01$  | --           | CCSD(T) |                                                    |
|   |      | $^1S, M_L = 0$ | $45.67 \pm 0.01$  | 20.67        | DHF     | <b>2C-SR-CC@d-aug-dyall.cv4z@(core 4)[vir 266]</b> |
|   |      |                | $42.15 \pm 0.01$  | 11.35        | MP2     |                                                    |
|   |      |                | $38.01 \pm 0.01$  | 0.42         | CCSD    |                                                    |
|   |      |                | $37.85 \pm 0.01$  | --           | CCSD(T) |                                                    |
|   |      | $^1S, M_L = 0$ | 45.61             | 23.41        | DHF     | 2C-SR-CC@dyall.cv4z@(core 4)[vir 166]              |
|   |      |                | 41.50             | 12.28        | MP2     |                                                    |
|   |      |                | 37.14             | 0.48         | CCSD    |                                                    |
|   |      |                | 36.96             | --           | CCSD(T) |                                                    |
|   |      | $^1S, M_L = 0$ | $45.66 \pm 0.01$  | 20.66        | DHF     | 2C-SR-CC@s-aug-dyall.cv4z@(core 4)[vir 216]        |
|   |      |                | $42.13 \pm 0.01$  | 11.33        | MP2     |                                                    |
|   |      |                | 38.00             | 0.42         | CCSD    |                                                    |
|   |      |                | 37.84             | --           | CCSD(T) |                                                    |
|   |      | $^1S_0$        | $45.67 \pm 0.01$  | 20.66        | DHF     | <b>4C-DC-CC@d-aug-dyall.cv4z@(core 4)[vir 266]</b> |
|   |      |                | $42.14 \pm 0.01$  | 11.35        | MP2     |                                                    |
|   |      |                | $38.01 \pm 0.01$  | 0.42         | CCSD    |                                                    |
|   |      |                | $37.85 \pm 0.01$  | --           | CCSD(T) |                                                    |
|   |      | $^1S_0$        | 45.61             | 23.02        | DHF     | 4C-DC-CC@dyall.cv4z@(core 4)[vir 132]              |
|   |      |                | 41.66             | 12.37        | MP2     |                                                    |

(continued)

Table S10. continued.

| Z  | Atom | State          | $\alpha_D$ (a.u.) | $\delta$ | Method  | Comments                                                     |
|----|------|----------------|-------------------|----------|---------|--------------------------------------------------------------|
| 12 | Mg   | $^1S, M_L = 0$ | 37.21             | 0.36     | CCSD    |                                                              |
|    |      |                | 37.07             | --       | CCSD(T) |                                                              |
|    |      |                | 81.91 $\pm$ 0.03  | 14.14    | DHF     | <a href="#">2C-NR-CC@d-aug-dyall.cv4z@(core 10)[vir 314]</a> |
|    |      |                | 72.15 $\pm$ 0.02  | 0.55     | MP2     |                                                              |
|    |      | $^1S, M_L = 0$ | 72.40 $\pm$ 0.02  | 0.89     | CCSD    |                                                              |
|    |      |                | 71.76 $\pm$ 0.02  | --       | CCSD(T) |                                                              |
|    |      |                | 81.48 $\pm$ 0.03  | 14.09    | DHF     | <a href="#">2C-SR-CC@d-aug-dyall.cv4z@(core 10)[vir 314]</a> |
|    |      |                | 71.78 $\pm$ 0.02  | 0.51     | MP2     |                                                              |
|    |      |                | 72.05 $\pm$ 0.02  | 0.89     | CCSD    |                                                              |
|    |      |                | 71.42 $\pm$ 0.02  | --       | CCSD(T) |                                                              |
|    |      | $^1S, M_L = 0$ | 81.28 $\pm$ 0.01  | 14.91    | DHF     | 2C-SR-CC@dyall.cv4z@(core 10)[vir 214]                       |
|    |      |                | 70.79 $\pm$ 0.01  | 0.08     | MP2     |                                                              |
|    |      |                | 71.38 $\pm$ 0.01  | 0.93     | CCSD    |                                                              |
|    |      |                | 70.73 $\pm$ 0.01  | --       | CCSD(T) |                                                              |
|    |      | $^1S, M_L = 0$ | 81.44 $\pm$ 0.02  | 14.06    | DHF     | 2C-SR-CC@s-aug-dyall.cv4z@(core 10)[vir 264]                 |
|    |      |                | 71.75 $\pm$ 0.02  | 0.49     | MP2     |                                                              |
|    |      |                | 72.03 $\pm$ 0.02  | 0.88     | CCSD    |                                                              |
|    |      |                | 71.40 $\pm$ 0.02  | --       | CCSD(T) |                                                              |
|    |      | $^1S_0$        | 81.46 $\pm$ 0.03  | 14.09    | DHF     | <a href="#">4C-DC-CC@d-aug-dyall.cv4z@(core 10)[vir 314]</a> |
|    |      |                | 71.77 $\pm$ 0.02  | 0.51     | MP2     |                                                              |
|    |      |                | 72.04 $\pm$ 0.02  | 0.88     | CCSD    |                                                              |
|    |      |                | 71.40 $\pm$ 0.02  | --       | CCSD(T) |                                                              |
|    |      | $^1S_0$        | 81.26 $\pm$ 0.01  | 14.65    | DHF     | 4C-DC-CC@dyall.cv4z@(core 10)[vir 182]                       |
|    |      |                | 70.98 $\pm$ 0.01  | 0.14     | MP2     |                                                              |
|    |      |                | 71.42 $\pm$ 0.01  | 0.76     | CCSD    |                                                              |
|    |      |                | 70.88 $\pm$ 0.01  | --       | CCSD(T) |                                                              |
| 20 | Ca   | $^1S, M_L = 0$ | 187.19 $\pm$ 0.14 | 16.44    | DHF     | <a href="#">2C-NR-CC@d-aug-dyall.cv4z@(core 20)[vir 510]</a> |
|    |      |                | 144.35 $\pm$ 0.07 | -10.20   | MP2     |                                                              |
|    |      |                | 163.77 $\pm$ 0.08 | 1.88     | CCSD    |                                                              |
|    |      |                | 160.76 $\pm$ 0.07 | --       | CCSD(T) |                                                              |
|    |      | $^1S, M_L = 0$ | 184.55 $\pm$ 0.14 | 16.46    | DHF     | <a href="#">2C-SR-CC@d-aug-dyall.cv4z@(core 20)[vir 510]</a> |
|    |      |                | 142.36 $\pm$ 0.07 | -10.16   | MP2     |                                                              |
|    |      |                | 161.46 $\pm$ 0.07 | 1.89     | CCSD    |                                                              |
|    |      |                | 158.46 $\pm$ 0.07 | --       | CCSD(T) |                                                              |
|    |      | $^1S, M_L = 0$ | 183.29 $\pm$ 0.04 | 17.24    | DHF     | 2C-SR-CC@dyall.cv4z@(core 20)[vir 410]                       |
|    |      |                | 139.48 $\pm$ 0.03 | -10.78   | MP2     |                                                              |
|    |      |                | 159.43 $\pm$ 0.01 | 1.98     | CCSD    |                                                              |
|    |      |                | 156.34 $\pm$ 0.01 | --       | CCSD(T) |                                                              |

(continued)

Table S10. continued.

| Z  | Atom | State          | $\alpha_D$ (a.u.) | $\delta$ | Method  | Comments                                     |
|----|------|----------------|-------------------|----------|---------|----------------------------------------------|
|    |      | $^1S, M_L = 0$ | $184.25 \pm 0.11$ | 16.34    | DHF     | 2C-SR-CC@s-aug-dyall.cv4z@(core 20)[vir 460] |
|    |      |                | $142.38 \pm 0.07$ | -10.10   | MP2     |                                              |
|    |      |                | $161.36 \pm 0.07$ | 1.88     | CCSD    |                                              |
|    |      |                | $158.38 \pm 0.06$ | --       | CCSD(T) |                                              |
|    |      | $^1S_0$        | $184.20 \pm 0.11$ | 16.34    | DHF     | 2C-DC-CC@s-aug-dyall.cv4z@(core 20)[vir 296] |
|    |      |                | $142.34 \pm 0.07$ | -10.10   | MP2     |                                              |
|    |      |                | $161.22 \pm 0.07$ | 1.83     | CCSD    |                                              |
|    |      |                | $158.33 \pm 0.06$ | --       | CCSD(T) |                                              |
|    |      | $^1S_0$        | $184.49 \pm 0.14$ | 16.47    | DHF     | 4C-DC-CC@d-aug-dyall.cv4z@(core 20)[vir 346] |
|    |      |                | $142.31 \pm 0.07$ | -10.16   | MP2     |                                              |
|    |      |                | $161.32 \pm 0.07$ | 1.84     | CCSD    |                                              |
|    |      |                | $158.41 \pm 0.07$ | --       | CCSD(T) |                                              |
|    |      | $^1S_0$        | $183.24 \pm 0.04$ | 17.12    | DHF     | 4C-DC-CC@dyall.cv4z@(core 20)[vir 228]       |
|    |      |                | $139.82 \pm 0.03$ | -10.63   | MP2     |                                              |
|    |      |                | $159.37 \pm 0.01$ | 1.86     | CCSD    |                                              |
|    |      |                | $156.45 \pm 0.01$ | --       | CCSD(T) |                                              |
| 38 | Sr   | $^1S, M_L = 0$ | $249.10 \pm 0.25$ | 18.06    | DHF     | 2C-NR-CC@s-aug-dyall.cv4z@(core 28)[vir 346] |
|    |      |                | $180.71 \pm 0.1$  | -14.36   | MP2     |                                              |
|    |      |                | $215.90 \pm 0.12$ | 2.32     | CCSD    |                                              |
|    |      |                | $211.00 \pm 0.11$ | --       | CCSD(T) |                                              |
|    |      | $^1S, M_L = 0$ | $235.64 \pm 0.24$ | 18.33    | DHF     | 2C-SR-CC@d-aug-dyall.cv4z@(core 28)[vir 418] |
|    |      |                | $171.27 \pm 0.09$ | -13.99   | MP2     |                                              |
|    |      |                | $203.95 \pm 0.12$ | 2.42     | CCSD    |                                              |
|    |      |                | $199.13 \pm 0.11$ | --       | CCSD(T) |                                              |
|    |      | $^1S, M_L = 0$ | $234.08 \pm 0.11$ | 18.20    | DHF     | 2C-SR-CC@dyall.cv4z@(core 28)[vir 274]       |
|    |      |                | $168.19 \pm 0.07$ | -15.07   | MP2     |                                              |
|    |      |                | $202.72 \pm 0.05$ | 2.36     | CCSD    |                                              |
|    |      |                | $198.04 \pm 0.05$ | --       | CCSD(T) |                                              |
|    |      | $^1S, M_L = 0$ | $235.56 \pm 0.23$ | 18.28    | DHF     | 2C-SR-CC@s-aug-dyall.cv4z@(core 28)[vir 346] |
|    |      |                | $171.33 \pm 0.09$ | -13.97   | MP2     |                                              |
|    |      |                | $203.92 \pm 0.12$ | 2.39     | CCSD    |                                              |
|    |      |                | $199.15 \pm 0.11$ | --       | CCSD(T) |                                              |
|    |      | $^1S_0$        | $235.39 \pm 0.23$ | 18.29    | DHF     | 2C-DC-CC@s-aug-dyall.cv4z@(core 28)[vir 346] |
|    |      |                | $171.23 \pm 0.09$ | -13.96   | MP2     |                                              |
|    |      |                | $203.77 \pm 0.12$ | 2.40     | CCSD    |                                              |
|    |      |                | $199.00 \pm 0.11$ | --       | CCSD(T) |                                              |
|    |      | $^1S_0$        | $233.92 \pm 0.11$ | 17.65    | DHF     | 4C-DC-CC@dyall.cv4z@(core 20)[vir 214]       |
|    |      |                | $170.01 \pm 0.07$ | -14.50   | MP2     |                                              |

(continued)

Table S10. continued.

| Z  | Atom | State          | $\alpha_D$ (a.u.) | $\delta$ | Method  | Comments                                                     |
|----|------|----------------|-------------------|----------|---------|--------------------------------------------------------------|
| 56 | Ba   | $^1S, M_L = 0$ | $203.30 \pm 0.05$ | 2.25     | CCSD    |                                                              |
|    |      |                | $198.83 \pm 0.05$ | --       | CCSD(T) |                                                              |
|    |      |                | $375.28 \pm 0.58$ | 17.74    | DHF     | <a href="#">2C-NR-CC@s-aug-dyall.cv4z@(core 28)[vir 398]</a> |
|    |      |                | $246.60 \pm 0.21$ | -22.63   | MP2     |                                                              |
|    |      | $^1S, M_L = 0$ | $326.52 \pm 0.23$ | 2.44     | CCSD    |                                                              |
|    |      |                | $318.74 \pm 0.17$ | --       | CCSD(T) |                                                              |
|    |      |                | $330.78 \pm 0.52$ | 19.92    | DHF     | 2C-SR-CC@d-aug-dyall.cv4z@(core 28)[vir 470]                 |
|    |      |                | $217.46 \pm 0.11$ | -21.16   | MP2     |                                                              |
|    |      | $^1S, M_L = 0$ | $284.58 \pm 0.23$ | 3.17     | CCSD    |                                                              |
|    |      |                | $275.83 \pm 0.19$ | --       | CCSD(T) |                                                              |
|    |      |                | $326.64 \pm 0.18$ | 19.50    | DHF     | 2C-SR-CC@dyall.cv4z@(core 28)[vir 326]                       |
|    |      |                | $214.44 \pm 0.13$ | -21.55   | MP2     |                                                              |
|    |      | $^1S, M_L = 0$ | $281.87 \pm 0.05$ | 3.12     | CCSD    |                                                              |
|    |      |                | $273.34 \pm 0.04$ | --       | CCSD(T) |                                                              |
|    |      |                | $330.34 \pm 0.48$ | 19.56    | DHF     | <a href="#">2C-SR-CC@s-aug-dyall.cv4z@(core 28)[vir 398]</a> |
|    |      |                | $218.83 \pm 0.16$ | -20.80   | MP2     |                                                              |
|    |      | $^1S_0$        | $284.94 \pm 0.22$ | 3.12     | CCSD    |                                                              |
|    |      |                | $276.31 \pm 0.19$ | --       | CCSD(T) |                                                              |
|    |      |                | $329.82 \pm 0.48$ | 19.57    | DHF     | <a href="#">2C-DC-CC@s-aug-dyall.cv4z@(core 28)[vir 398]</a> |
|    |      |                | $218.62 \pm 0.16$ | -20.74   | MP2     |                                                              |
| 88 | Ra   | $^1S, M_L = 0$ | $284.46 \pm 0.22$ | 3.13     | CCSD    |                                                              |
|    |      |                | $275.84 \pm 0.19$ | --       | CCSD(T) |                                                              |
|    |      |                | $326.18 \pm 0.18$ | 18.85    | DHF     | 4C-DC-CC@dyall.cv4z@(core 20)[vir 252]                       |
|    |      |                | $216.44 \pm 0.13$ | -21.14   | MP2     |                                                              |
|    |      | $^1S_0$        | $282.69 \pm 0.05$ | 3.00     | CCSD    |                                                              |
|    |      |                | $274.45 \pm 0.04$ | --       | CCSD(T) |                                                              |
|    |      |                | $451.09 \pm 0.78$ | 18.28    | DHF     | <a href="#">2C-NR-CC@s-aug-dyall.cv4z@(core 42)[vir 378]</a> |
|    |      |                | $281.99 \pm 0.33$ | -26.06   | MP2     |                                                              |
|    |      | $^1S, M_L = 0$ | $391.33 \pm 0.28$ | 2.61     | CCSD    |                                                              |
|    |      |                | $381.38 \pm 0.21$ | --       | CCSD(T) |                                                              |
|    |      |                | $305.91 \pm 0.5$  | 22.35    | DHF     | 2C-SR-CC@d-aug-dyall.cv4z@(core 42)[vir 450]                 |
|    |      |                | $197.21 \pm 0.09$ | -21.13   | MP2     |                                                              |
|    |      | $^1S, M_L = 0$ | $259.82 \pm 0.27$ | 3.91     | CCSD    |                                                              |
|    |      |                | $250.03 \pm 0.23$ | --       | CCSD(T) |                                                              |
|    |      |                | $302.00 \pm 0.18$ | 22.16    | DHF     | 2C-SR-CC@dyall.cv4z@(core 42)[vir 306]                       |
|    |      |                | $193.20 \pm 0.1$  | -21.85   | MP2     |                                                              |
|    |      | $^1S, M_L = 0$ | $256.68 \pm 0.09$ | 3.82     | CCSD    |                                                              |
|    |      |                | $247.23 \pm 0.08$ | --       | CCSD(T) |                                                              |

(continued)

Table S10. continued.

| Z | Atom | State          | $\alpha_D$ (a.u.) | $\delta$ | Method  | Comments                                                     |
|---|------|----------------|-------------------|----------|---------|--------------------------------------------------------------|
|   |      | $^1S, M_L = 0$ | $305.39 \pm 0.46$ | 21.91    | DHF     | <a href="#">2C-SR-CC@s-aug-dyall.cv4z@(core 42)[vir 378]</a> |
|   |      |                | $198.77 \pm 0.15$ | -20.65   | MP2     |                                                              |
|   |      |                | $260.15 \pm 0.26$ | 3.85     | CCSD    |                                                              |
|   |      |                | $250.50 \pm 0.23$ | --       | CCSD(T) |                                                              |
|   |      | $^1S_0$        | $302.23 \pm 0.44$ | 21.67    | DHF     | <a href="#">2C-DC-CC@s-aug-dyall.cv4z@(core 42)[vir 380]</a> |
|   |      |                | $198.65 \pm 0.15$ | -20.03   | MP2     |                                                              |
|   |      |                | $257.79 \pm 0.25$ | 3.78     | CCSD    |                                                              |
|   |      |                | $248.40 \pm 0.22$ | --       | CCSD(T) |                                                              |
|   |      | $^1S_0$        | $299.17 \pm 0.18$ | 21.17    | DHF     | 4C-DC-CC@dyall.cv4z@(core 20)[vir 234]                       |
|   |      |                | $196.17 \pm 0.1$  | -20.55   | MP2     |                                                              |
|   |      |                | $255.73 \pm 0.08$ | 3.58     | CCSD    |                                                              |
|   |      |                | $246.89 \pm 0.08$ | --       | CCSD(T) |                                                              |

## S2.3 Group 13 elements

Table S11: The results of dipole polarizability for Group 13 elements.

| Z | Atom | State              | $\alpha_D$ (a.u.) | $\delta$ (%) | Method  | Comments                                               |
|---|------|--------------------|-------------------|--------------|---------|--------------------------------------------------------|
| 5 | B    | $^2P, M_L = 0$     | $25.40 \pm 0.05$  | 0.91         | DHF     | <a href="#">2C-NR-CC@dyall.acv4z@(core 5)[vir 251]</a> |
|   |      | $^2P, M_L = \pm 1$ | $19.57 \pm 0.01$  | 5.03         |         |                                                        |
|   |      | $^2P$              | $21.51 \pm 0.03$  | 3.37         |         | $\Delta\alpha = -5.83$                                 |
|   |      | $^2P, M_L = 0$     | $24.71 \pm 0.09$  | -1.80        | MP2     |                                                        |
|   |      | $^2P, M_L = \pm 1$ | $19.74 \pm 0.02$  | 5.97         |         |                                                        |
|   |      | $^2P$              | $21.40 \pm 0.05$  | 2.84         |         | $\Delta\alpha = -4.97$                                 |
|   |      | $^2P, M_L = 0$     | $25.11 \pm 0.06$  | -0.24        | CCSD    |                                                        |
|   |      | $^2P, M_L = \pm 1$ | $18.59 \pm 0.01$  | -0.18        |         |                                                        |
|   |      | $^2P$              | $20.76 \pm 0.04$  | -0.21        |         | $\Delta\alpha = -6.51$                                 |
|   |      | $^2P, M_L = 0$     | $25.17 \pm 0.06$  | --           | CCSD(T) |                                                        |
|   |      | $^2P, M_L = \pm 1$ | $18.63 \pm 0.01$  | --           |         |                                                        |
|   |      | $^2P$              | $20.81 \pm 0.04$  | --           |         | $\Delta\alpha = -6.54$                                 |
|   |      | $^2P, M_L = 0$     | $25.40 \pm 0.05$  | 0.89         | DHF     | <a href="#">2C-SR-CC@dyall.acv4z@(core 5)[vir 251]</a> |
|   |      | $^2P, M_L = \pm 1$ | $19.55 \pm 0.01$  | 5.04         |         |                                                        |
|   |      | $^2P$              | $21.50 \pm 0.03$  | 3.37         |         | $\Delta\alpha = -5.85$                                 |
|   |      | $^2P, M_L = 0$     | $24.69 \pm 0.08$  | -1.91        | MP2     |                                                        |
|   |      | $^2P, M_L = \pm 1$ | $19.72 \pm 0.02$  | 5.95         |         |                                                        |

(continued)

Table S11. continued.

| Z  | Atom | State                      | $\alpha_D$ (a.u.) | $\delta$ | Method  | Comments                                                |
|----|------|----------------------------|-------------------|----------|---------|---------------------------------------------------------|
| 13 | Al   | $^2P$                      | $21.38 \pm 0.05$  | 2.78     | CCSD    | $\Delta\alpha = -4.97$                                  |
|    |      | $^2P, M_L = 0$             | $25.11 \pm 0.06$  | -0.25    |         |                                                         |
|    |      | $^2P, M_L = \pm 1$         | $18.58 \pm 0.01$  | -0.16    |         |                                                         |
|    |      | $^2P$                      | $20.76 \pm 0.03$  | -0.20    | CCSD(T) | $\Delta\alpha = -6.53$                                  |
|    |      | $^2P, M_L = 0$             | $25.17 \pm 0.06$  | --       |         |                                                         |
|    |      | $^2P, M_L = \pm 1$         | $18.61 \pm 0.01$  | --       |         |                                                         |
|    |      | $^2P$                      | $20.80 \pm 0.03$  | --       |         | $\Delta\alpha = -6.56$                                  |
|    |      | $^2P_{1/2}$                | $21.50 \pm 0.09$  |          | MRCISD  | <a href="#">4C-DC-CI@dyall.acv4z@(core 5)[vir 251]</a>  |
|    |      | $^2P_{3/2}, M_J = \pm 1/2$ | $21.23 \pm 0.09$  |          |         |                                                         |
|    |      | $^2P_{3/2}, M_J = \pm 3/2$ | 18.47             |          |         |                                                         |
|    |      | $^2P_{3/2}$                | $19.85 \pm 0.06$  |          |         | $\bar{\alpha}_{J=3/2} - \alpha_{J=1/2} = -1.65$         |
|    |      | $^2P, M_L = 0$             | $106.48 \pm 2.41$ | 17.12    | DHF     | <a href="#">2C-NR-CC@dyall.acv4z@(core 13)[vir 363]</a> |
|    |      | $^2P, M_L = \pm 1$         | $54.62 \pm 0.07$  | 8.07     | MP2     |                                                         |
|    |      | $^2P$                      | $71.91 \pm 1.39$  | 12.36    |         | $\Delta\alpha = -51.86$                                 |
| 13 | Al   | $^2P, M_L = 0$             | $86.21 \pm 1.11$  | -5.17    | CCSD    |                                                         |
|    |      | $^2P, M_L = \pm 1$         | $57.70 \pm 0.45$  | 14.16    |         |                                                         |
|    |      | $^2P$                      | $67.20 \pm 0.74$  | 5.01     |         | $\Delta\alpha = -28.51$                                 |
|    |      | $^2P, M_L = 0$             | $91.51 \pm 1.6$   | 0.65     | CCSD(T) |                                                         |
|    |      | $^2P, M_L = \pm 1$         | $50.43 \pm 0.09$  | -0.21    |         |                                                         |
|    |      | $^2P$                      | $64.12 \pm 0.92$  | 0.20     |         | $\Delta\alpha = -41.08$                                 |
|    |      | $^2P, M_L = 0$             | $90.91 \pm 1.54$  | --       |         |                                                         |
|    |      | $^2P, M_L = \pm 1$         | $50.54 \pm 0.11$  | --       |         |                                                         |
|    |      | $^2P$                      | $64.00 \pm 0.89$  | --       |         | $\Delta\alpha = -40.37$                                 |
|    |      | $^2P, M_L = 0$             | $107.25 \pm 2.44$ | 16.13    | DHF     | <a href="#">2C-SR-CC@dyall.acv4z@(core 11)[vir 223]</a> |
|    |      | $^2P, M_L = \pm 1$         | $54.52 \pm 0.07$  | 7.42     | MP2     |                                                         |
|    |      | $^2P$                      | $72.09 \pm 1.41$  | 11.57    |         | $\Delta\alpha = -52.73$                                 |
|    |      | $^2P, M_L = 0$             | $88.30 \pm 1.2$   | -4.38    | CCSD    |                                                         |
|    |      | $^2P, M_L = \pm 1$         | $57.74 \pm 0.44$  | 13.77    |         |                                                         |
|    |      | $^2P$                      | $67.93 \pm 0.78$  | 5.12     |         | $\Delta\alpha = -30.56$                                 |
|    |      | $^2P, M_L = 0$             | $92.93 \pm 1.65$  | 0.62     | CCSD(T) |                                                         |
|    |      | $^2P, M_L = \pm 1$         | $50.66 \pm 0.1$   | -0.17    |         |                                                         |
|    |      | $^2P$                      | $64.75 \pm 0.95$  | 0.21     |         | $\Delta\alpha = -42.27$                                 |
|    |      | $^2P, M_L = 0$             | $92.35 \pm 1.59$  | --       |         |                                                         |
|    |      | $^2P, M_L = \pm 1$         | $50.75 \pm 0.11$  | --       |         |                                                         |
|    |      | $^2P$                      | $64.62 \pm 0.92$  | --       |         | $\Delta\alpha = -41.60$                                 |
|    |      | $^2P, M_L = 0$             | $107.22 \pm 2.23$ | 17.27    | DHF     | <a href="#">2C-SR-CC@dyall.acv4z@(core 13)[vir 363]</a> |
|    |      | $^2P, M_L = \pm 1$         | $54.51 \pm 0.07$  | 8.04     |         |                                                         |
|    |      | $^2P$                      | $72.08 \pm 1.29$  | 12.42    |         | $\Delta\alpha = -52.70$                                 |

(continued)



Table S11. continued.

| Z                  | Atom             | State                      | $\alpha_D$ (a.u.) | $\delta$           | Method                  | Comments                                        |      |                                                |
|--------------------|------------------|----------------------------|-------------------|--------------------|-------------------------|-------------------------------------------------|------|------------------------------------------------|
|                    |                  | $^2P, M_L = 0$             | $86.69 \pm 1.02$  | -5.18              | MP2                     | $\Delta\alpha = -29.07$                         |      |                                                |
|                    |                  | $^2P, M_L = \pm 1$         | $57.62 \pm 0.41$  | 14.18              | CCSD                    |                                                 |      |                                                |
|                    |                  | $^2P$                      | $67.31 \pm 0.68$  | 4.98               |                         |                                                 |      |                                                |
|                    |                  | $^2P, M_L = 0$             | $92.03 \pm 1.48$  | 0.66               |                         |                                                 |      |                                                |
|                    |                  | $^2P, M_L = \pm 1$         | $50.35 \pm 0.09$  | -0.23              | CCSD(T)                 | $\Delta\alpha = -41.69$                         |      |                                                |
|                    |                  | $^2P$                      | $64.24 \pm 0.85$  | 0.20               |                         |                                                 |      |                                                |
|                    |                  | $^2P, M_L = 0$             | $91.43 \pm 1.42$  | --                 |                         |                                                 |      |                                                |
|                    |                  | $^2P, M_L = \pm 1$         | $50.46 \pm 0.1$   | --                 |                         |                                                 |      |                                                |
|                    |                  | $^2P$                      | $64.12 \pm 0.82$  | --                 | $\Delta\alpha = -40.97$ |                                                 |      |                                                |
|                    |                  | $^2P_{1/2}$                | $64.44 \pm 0.25$  | 13.57              | DHF                     | <b>4C-DC-CC@dyall.acv4z@(core 11)[vir 223]</b>  |      |                                                |
|                    |                  |                            | $84.40 \pm 8.26$  | 48.74              | MP2                     |                                                 |      |                                                |
|                    |                  |                            | $64.70 \pm 0.09$  | 14.02              | CCSD                    |                                                 |      |                                                |
|                    |                  |                            | $56.74 \pm 0.26$  | --                 | CCSD(T)                 |                                                 |      |                                                |
|                    |                  | $^2P_{1/2}$                | $64.78 \pm 0.05$  | -6.00              | DHF                     | 4C-DC-CC@dyall.acv4z@(core 13)[vir 363]         |      |                                                |
|                    |                  |                            | $173.69 \pm 8.64$ | 152.02             | MP2                     |                                                 |      |                                                |
|                    |                  |                            | $64.93 \pm 0.07$  | -5.78              | CCSD                    |                                                 |      |                                                |
|                    |                  |                            | $68.92 \pm 1.37$  | --                 | CCSD(T)                 |                                                 |      |                                                |
|                    |                  | $^2P_{1/2}$                | $62.03 \pm 0.36$  |                    | MRCISD                  | <b>4C-DC-CI@dyall.acv4z@(core 13)[vir 223]</b>  |      |                                                |
|                    |                  | $^2P_{3/2}, M_J = \pm 1/2$ | $63.42 \pm 0.27$  |                    |                         |                                                 |      |                                                |
|                    |                  | $^2P_{3/2}, M_J = \pm 3/2$ | $49.44 \pm 0.01$  |                    |                         |                                                 |      |                                                |
|                    |                  | $^2P_{3/2}$                | $56.43 \pm 0.19$  |                    |                         | $\bar{\alpha}_{J=3/2} - \alpha_{J=1/2} = -5.60$ |      |                                                |
|                    |                  | 31                         | Ga                | $^2P, M_L = 0$     | $82.63 \pm 0.11$        | 10.55                                           | DHF  | <b>2C-NR-CC@dyall.acv4z@(core 31)[vir 481]</b> |
|                    |                  |                            |                   | $^2P, M_L = \pm 1$ | $48.01 \pm 0.01$        | 13.16                                           | MP2  |                                                |
|                    |                  |                            |                   | $^2P$              | $59.55 \pm 0.06$        | 11.94                                           |      |                                                |
|                    |                  |                            |                   | $^2P, M_L = 0$     | $66.36 \pm 0.3$         | -11.23                                          |      |                                                |
|                    |                  |                            |                   | $^2P, M_L = \pm 1$ | $44.89 \pm 0.1$         | 5.81                                            | CCSD | $\Delta\alpha = -21.47$                        |
|                    |                  |                            |                   | $^2P$              | $52.04 \pm 0.19$        | -2.17                                           |      |                                                |
|                    |                  |                            |                   | $^2P, M_L = 0$     | $74.95 \pm 0.08$        | 0.27                                            |      |                                                |
| $^2P, M_L = \pm 1$ | $42.82 \pm 0.01$ |                            |                   | 0.93               |                         |                                                 |      |                                                |
| $^2P$              | $53.53 \pm 0.05$ |                            |                   | 0.62               | CCSD(T)                 | $\Delta\alpha = -32.13$                         |      |                                                |
| $^2P, M_L = 0$     | $74.75 \pm 0.08$ |                            |                   | --                 |                         |                                                 |      |                                                |
| $^2P, M_L = \pm 1$ | $42.42 \pm 0.01$ |                            |                   | --                 |                         |                                                 |      |                                                |
| $^2P$              | $53.20 \pm 0.05$ |                            |                   | --                 |                         |                                                 |      |                                                |
| $^2P, M_L = 0$     | $84.22 \pm 0.12$ |                            |                   | 12.17              | DHF                     | <b>2C-SR-CC@dyall.acv4z@(core 13)[vir 203]</b>  |      |                                                |
| $^2P, M_L = \pm 1$ | $46.86 \pm 0.01$ |                            |                   | 13.45              | MP2                     |                                                 |      |                                                |
| $^2P$              | $59.31 \pm 0.07$ |                            |                   | 12.84              |                         |                                                 |      |                                                |
| $^2P, M_L = 0$     | $67.41 \pm 0.48$ |                            |                   | -10.22             |                         |                                                 |      |                                                |
| $^2P, M_L = \pm 1$ | $43.69 \pm 0.11$ |                            |                   | 5.78               |                         | $\Delta\alpha = -37.36$                         |      |                                                |

(continued)

Table S11. continued.

| Z  | Atom | State                      | $\alpha_D$ (a.u.) | $\delta$ | Method  | Comments                                       |
|----|------|----------------------------|-------------------|----------|---------|------------------------------------------------|
|    |      | $^2P$                      | $51.60 \pm 0.29$  | -1.84    | CCSD    | $\Delta\alpha = -23.72$                        |
|    |      | $^2P, M_L = 0$             | $75.06 \pm 0.08$  | -0.04    |         |                                                |
|    |      | $^2P, M_L = \pm 1$         | $41.65 \pm 0.01$  | 0.83     |         |                                                |
|    |      | $^2P$                      | $52.78 \pm 0.05$  | 0.41     | CCSD(T) | $\Delta\alpha = -33.41$                        |
|    |      | $^2P, M_L = 0$             | $75.08 \pm 0.09$  | --       |         |                                                |
|    |      | $^2P, M_L = \pm 1$         | $41.30 \pm 0.03$  | --       |         |                                                |
|    |      | $^2P$                      | $52.56 \pm 0.06$  | --       |         | $\Delta\alpha = -33.78$                        |
|    |      | $^2P, M_L = 0$             | $84.22 \pm 0.12$  | 10.86    | DHF     | <b>2C-SR-CC@dyall.acv4z@(core 31)[vir 481]</b> |
|    |      | $^2P, M_L = \pm 1$         | $46.86 \pm 0.01$  | 13.35    | MP2     |                                                |
|    |      | $^2P$                      | $59.31 \pm 0.07$  | 12.16    |         | $\Delta\alpha = -37.36$                        |
|    |      | $^2P, M_L = 0$             | $67.11 \pm 0.3$   | -11.66   |         |                                                |
|    |      | $^2P, M_L = \pm 1$         | $43.78 \pm 0.34$  | 5.91     | CCSD    |                                                |
|    |      | $^2P$                      | $51.56 \pm 0.33$  | -2.50    |         | $\Delta\alpha = -23.33$                        |
|    |      | $^2P, M_L = 0$             | $76.15 \pm 0.08$  | 0.24     |         |                                                |
|    |      | $^2P, M_L = \pm 1$         | $41.76 \pm 0.01$  | 1.01     | CCSD(T) |                                                |
|    |      | $^2P$                      | $53.22 \pm 0.05$  | 0.65     |         | $\Delta\alpha = -34.39$                        |
|    |      | $^2P, M_L = 0$             | $75.97 \pm 0.08$  | --       |         |                                                |
|    |      | $^2P, M_L = \pm 1$         | $41.34 \pm 0.03$  | --       |         |                                                |
|    |      | $^2P$                      | $52.88 \pm 0.06$  | --       |         | $\Delta\alpha = -34.63$                        |
|    |      | $^2P_{1/2}$                | $57.15 \pm 0.01$  | 9.94     | DHF     | <b>4C-DC-CC@dyall.acv4z@(core 13)[vir 203]</b> |
| 49 | In   |                            | $47.71 \pm 0.71$  | -8.21    | MP2     |                                                |
|    |      |                            | $53.40 \pm 0.1$   | 2.73     | CCSD    |                                                |
|    |      |                            | $51.98 \pm 0.08$  | --       | CCSD(T) |                                                |
|    |      | $^2P_{1/2}$                | $51.76 \pm 0.09$  |          | MRCISD  | <b>4C-DC-CI@dyall.acv4z@(core 13)[vir 203]</b> |
|    |      | $^2P_{3/2}, M_J = \pm 1/2$ | 63.60             |          |         |                                                |
|    |      | $^2P_{3/2}, M_J = \pm 3/2$ | $42.21 \pm 0.01$  |          |         |                                                |
|    |      | $^2P_{3/2}$                | $52.90 \pm 0.01$  |          |         | $\bar{\alpha}_{J=3/2} - \alpha_{J=1/2} = 1.14$ |
|    |      | $^2P, M_L = 0$             | $103.22 \pm 0.16$ | 10.58    | DHF     | <b>2C-NR-CC@dyall.acv4z@(core 49)[vir 553]</b> |
|    |      | $^2P, M_L = \pm 1$         | $67.34 \pm 0.02$  | 15.97    | MP2     |                                                |
|    |      | $^2P$                      | $79.30 \pm 0.09$  | 13.57    |         | $\Delta\alpha = -35.88$                        |
|    |      | $^2P, M_L = 0$             | $83.36 \pm 0.66$  | -10.69   |         |                                                |
|    |      | $^2P, M_L = \pm 1$         | $60.91 \pm 0.05$  | 4.90     | CCSD    |                                                |
|    |      | $^2P$                      | $68.40 \pm 0.38$  | -2.05    |         | $\Delta\alpha = -22.45$                        |
|    |      | $^2P, M_L = 0$             | $93.99 \pm 0.12$  | 0.70     |         |                                                |
|    |      | $^2P, M_L = \pm 1$         | $58.67 \pm 0.01$  | 1.03     | CCSD(T) |                                                |
|    |      | $^2P$                      | $70.44 \pm 0.07$  | 0.88     |         | $\Delta\alpha = -35.33$                        |
|    |      | $^2P, M_L = 0$             | $93.34 \pm 0.11$  | --       |         |                                                |
|    |      | $^2P, M_L = \pm 1$         | $58.07 \pm 0.01$  | --       |         |                                                |

(continued)

Table S11. continued.

| Z  | Atom | State                      | $\alpha_D$ (a.u.) | $\delta$ | Method  | Comments                                                |
|----|------|----------------------------|-------------------|----------|---------|---------------------------------------------------------|
|    |      | $^2P$                      | $69.83 \pm 0.07$  | --       |         | $\Delta\alpha = -35.27$                                 |
|    |      | $^2P, M_L = 0$             | $106.40 \pm 0.18$ | 11.24    | DHF     | <a href="#">2C-SR-CC@dyall.acv4z@(core 31)[vir 309]</a> |
|    |      | $^2P, M_L = \pm 1$         | $62.26 \pm 0.02$  | 15.70    |         |                                                         |
|    |      | $^2P$                      | $76.98 \pm 0.11$  | 13.60    |         | $\Delta\alpha = -44.14$                                 |
|    |      | $^2P, M_L = 0$             | $84.36 \pm 0.39$  | -11.81   | MP2     |                                                         |
|    |      | $^2P, M_L = \pm 1$         | $57.64 \pm 0.3$   | 7.10     |         |                                                         |
|    |      | $^2P$                      | $66.55 \pm 0.33$  | -1.80    |         | $\Delta\alpha = -26.72$                                 |
|    |      | $^2P, M_L = 0$             | $96.36 \pm 0.13$  | 0.73     | CCSD    |                                                         |
|    |      | $^2P, M_L = \pm 1$         | $54.27 \pm 0.01$  | 0.83     |         |                                                         |
|    |      | $^2P$                      | $68.30 \pm 0.08$  | 0.79     |         | $\Delta\alpha = -42.09$                                 |
|    |      | $^2P, M_L = 0$             | $95.65 \pm 0.14$  | --       | CCSD(T) |                                                         |
|    |      | $^2P, M_L = \pm 1$         | $53.82 \pm 0.02$  | --       |         |                                                         |
|    |      | $^2P$                      | $67.76 \pm 0.08$  | --       |         | $\Delta\alpha = -41.84$                                 |
|    |      | $^2P, M_L = 0$             | $106.40 \pm 0.18$ | 11.12    | DHF     | <a href="#">2C-SR-CC@dyall.acv4z@(core 49)[vir 553]</a> |
|    |      | $^2P, M_L = \pm 1$         | $62.26 \pm 0.02$  | 15.71    |         |                                                         |
|    |      | $^2P$                      | $76.98 \pm 0.11$  | 13.55    |         | $\Delta\alpha = -44.14$                                 |
|    |      | $^2P, M_L = 0$             | $83.87 \pm 0.75$  | -12.42   | MP2     |                                                         |
|    |      | $^2P, M_L = \pm 1$         | $58.33 \pm 0.18$  | 8.39     |         |                                                         |
|    |      | $^2P$                      | $66.84 \pm 0.46$  | -1.40    |         | $\Delta\alpha = -25.54$                                 |
|    |      | $^2P, M_L = 0$             | $96.46 \pm 0.13$  | 0.74     | CCSD    |                                                         |
|    |      | $^2P, M_L = \pm 1$         | $54.30 \pm 0.01$  | 0.91     |         |                                                         |
|    |      | $^2P$                      | $68.35 \pm 0.08$  | 0.83     |         | $\Delta\alpha = -42.16$                                 |
|    |      | $^2P, M_L = 0$             | $95.76 \pm 0.13$  | --       | CCSD(T) |                                                         |
|    |      | $^2P, M_L = \pm 1$         | $53.81 \pm 0.05$  | --       |         |                                                         |
|    |      | $^2P$                      | $67.79 \pm 0.08$  | --       |         | $\Delta\alpha = -41.94$                                 |
|    |      | $^2P_{1/2}$                | $71.25 \pm 0.1$   | 13.47    | DHF     | <a href="#">2C-DC-CC@dyall.acv4z@(core 31)[vir 309]</a> |
|    |      |                            | $56.72 \pm 0.07$  | -9.67    | MP2     |                                                         |
|    |      |                            | $60.74 \pm 0.05$  | -3.28    | CCSD    |                                                         |
|    |      |                            | $62.80 \pm 0.07$  | --       | CCSD(T) |                                                         |
|    |      | $^2P_{1/2}$                | $63.77 \pm 0.07$  |          | MRCISD  | <a href="#">4C-DC-CI@dyall.acv4z@(core 13)[vir 237]</a> |
|    |      | $^2P_{3/2}, M_J = \pm 1/2$ | $85.62 \pm 0.07$  |          |         |                                                         |
|    |      | $^2P_{3/2}, M_J = \pm 3/2$ | $56.59 \pm 0.02$  |          |         |                                                         |
|    |      | $^2P_{3/2}$                | $71.11 \pm 0.05$  |          |         |                                                         |
|    |      |                            |                   |          |         | $\bar{\alpha}_{J=3/2} - \alpha_{J=1/2} = 7.34$          |
| 81 | Tl   | $^2P, M_L = 0$             | $166.42 \pm 5.47$ | 22.30    | DHF     | <a href="#">2C-NR-CC@dyall.acv4z@(core 45)[vir 309]</a> |
|    |      | $^2P, M_L = \pm 1$         | $77.06 \pm 0.13$  | 16.30    |         |                                                         |
|    |      | $^2P$                      | $106.85 \pm 3.16$ | 19.34    |         | $\Delta\alpha = -89.36$                                 |
|    |      | $^2P, M_L = 0$             | $101.89 \pm 1.49$ | -25.12   | MP2     |                                                         |
|    |      | $^2P, M_L = \pm 1$         | $80.03 \pm 0.93$  | 20.78    |         |                                                         |

(continued)

Table S11. continued.

| Z | Atom | State              | $\alpha_D$ (a.u.) | $\delta$ | Method  | Comments                                       |
|---|------|--------------------|-------------------|----------|---------|------------------------------------------------|
|   |      | $^2P$              | $87.32 \pm 1.15$  | -2.47    |         | $\Delta\alpha = -21.86$                        |
|   |      | $^2P, M_L = 0$     | $138.73 \pm 3.71$ | 1.95     | CCSD    |                                                |
|   |      | $^2P, M_L = \pm 1$ | $66.68 \pm 0.18$  | 0.63     |         |                                                |
|   |      | $^2P$              | $90.70 \pm 2.15$  | 1.30     |         | $\Delta\alpha = -72.05$                        |
|   |      | $^2P, M_L = 0$     | $136.07 \pm 3.5$  | --       | CCSD(T) |                                                |
|   |      | $^2P, M_L = \pm 1$ | $66.26 \pm 0.2$   | --       |         |                                                |
|   |      | $^2P$              | $89.53 \pm 2.03$  | --       |         | $\Delta\alpha = -69.81$                        |
|   |      | $^2P, M_L = 0$     | $194.20 \pm 6.17$ | 28.29    | DHF     | <b>2C-SR-CC@dyall.acv4z@(core 35)[vir 309]</b> |
|   |      | $^2P, M_L = \pm 1$ | $61.74 \pm 0.25$  | 14.77    |         |                                                |
|   |      | $^2P$              | $105.89 \pm 3.57$ | 22.68    |         | $\Delta\alpha = -132.47$                       |
|   |      | $^2P, M_L = 0$     | $106.09 \pm 2.67$ | -29.92   | MP2     |                                                |
|   |      | $^2P, M_L = \pm 1$ | $68.01 \pm 0.53$  | 26.43    |         |                                                |
|   |      | $^2P$              | $80.70 \pm 1.6$   | -6.51    |         | $\Delta\alpha = -38.08$                        |
|   |      | $^2P, M_L = 0$     | $155.38 \pm 4.24$ | 2.65     | CCSD    |                                                |
|   |      | $^2P, M_L = \pm 1$ | $54.09 \pm 0.24$  | 0.56     |         |                                                |
|   |      | $^2P$              | $87.86 \pm 2.46$  | 1.78     |         | $\Delta\alpha = -101.29$                       |
|   |      | $^2P, M_L = 0$     | $151.38 \pm 4.02$ | --       | CCSD(T) |                                                |
|   |      | $^2P, M_L = \pm 1$ | $53.79 \pm 0.23$  | --       |         |                                                |
|   |      | $^2P$              | $86.32 \pm 2.33$  | --       |         | $\Delta\alpha = -97.59$                        |
|   |      | $^2P, M_L = 0$     | $194.13 \pm 5.76$ | 28.69    | DHF     | <b>2C-SR-CC@dyall.acv4z@(core 45)[vir 309]</b> |
|   |      | $^2P, M_L = \pm 1$ | $61.73 \pm 0.23$  | 15.34    |         |                                                |
|   |      | $^2P$              | $105.86 \pm 3.33$ | 23.15    |         | $\Delta\alpha = -132.39$                       |
|   |      | $^2P, M_L = 0$     | $104.75 \pm 2.46$ | -30.56   | MP2     |                                                |
|   |      | $^2P, M_L = \pm 1$ | $67.69 \pm 0.49$  | 26.47    |         |                                                |
|   |      | $^2P$              | $80.04 \pm 1.48$  | -6.89    |         | $\Delta\alpha = -37.06$                        |
|   |      | $^2P, M_L = 0$     | $154.48 \pm 3.93$ | 2.41     | CCSD    |                                                |
|   |      | $^2P, M_L = \pm 1$ | $53.97 \pm 0.22$  | 0.83     |         |                                                |
|   |      | $^2P$              | $87.47 \pm 2.28$  | 1.75     |         | $\Delta\alpha = -100.52$                       |
|   |      | $^2P, M_L = 0$     | $150.85 \pm 3.73$ | --       | CCSD(T) |                                                |
|   |      | $^2P, M_L = \pm 1$ | $53.52 \pm 0.21$  | --       |         |                                                |
|   |      | $^2P$              | $85.97 \pm 2.16$  | --       |         | $\Delta\alpha = -97.33$                        |
|   |      | $^2P_{1/2}$        | $57.10 \pm 0.05$  | 9.32     | DHF     | 4C-DC-CC@dyall.acv4z@(core 13)[vir 277]        |
|   |      |                    | $51.20 \pm 0.34$  | -1.97    | MP2     |                                                |
|   |      |                    | $52.46 \pm 0.04$  | 0.43     | CCSD    |                                                |
|   |      |                    | $52.23 \pm 0.03$  | --       | CCSD(T) |                                                |
|   |      | $^2P_{1/2}$        | $57.05 \pm 0.08$  | 10.56    | DHF     | <b>4C-DC-CC@dyall.acv4z@(core 35)[vir 309]</b> |
|   |      |                    | $50.48 \pm 0.58$  | -2.17    | MP2     |                                                |
|   |      |                    | $51.91 \pm 0.06$  | 0.59     | CCSD    |                                                |

(continued)

Table S11. continued.

| Z   | Atom | State                      | $\alpha_D$ (a.u.) | $\delta$ | Method  | Comments                                                |
|-----|------|----------------------------|-------------------|----------|---------|---------------------------------------------------------|
|     |      |                            | $51.60 \pm 0.05$  | --       | CCSD(T) |                                                         |
|     |      | $^2P_{1/2}$                | $51.72 \pm 0.04$  |          | MRCISD  | <a href="#">4C-DC-CI@dyall.acv4z@(core 13)[vir 277]</a> |
|     |      | $^2P_{3/2}, M_J = \pm 1/2$ | $108.67 \pm 0.18$ |          |         |                                                         |
|     |      | $^2P_{3/2}, M_J = \pm 3/2$ | $57.38 \pm 0.03$  |          |         |                                                         |
|     |      | $^2P_{3/2}$                | $83.03 \pm 0.13$  |          |         | $\bar{\alpha}_{J=3/2} - \alpha_{J=1/2} = 31.30$         |
| 113 | Nh   | $^2P, M_L = 0$             | $190.67 \pm 5.17$ | 20.44    | DHF     | <a href="#">2C-NR-CC@dyall.acv4z@(core 45)[vir 305]</a> |
|     |      | $^2P, M_L = \pm 1$         | $99.14 \pm 0.15$  | 18.36    |         |                                                         |
|     |      | $^2P$                      | $129.65 \pm 2.99$ | 19.37    |         | $\Delta\alpha = -91.53$                                 |
|     |      | $^2P, M_L = 0$             | $123.98 \pm 2.01$ | -21.68   | MP2     |                                                         |
|     |      | $^2P, M_L = \pm 1$         | $95.18 \pm 0.75$  | 13.64    |         |                                                         |
|     |      | $^2P$                      | $104.78 \pm 1.31$ | -3.52    |         | $\Delta\alpha = -28.80$                                 |
|     |      | $^2P, M_L = 0$             | $161.34 \pm 3.8$  | 1.91     | CCSD    |                                                         |
|     |      | $^2P, M_L = \pm 1$         | $84.61 \pm 0.18$  | 1.02     |         |                                                         |
|     |      | $^2P$                      | $110.18 \pm 2.2$  | 1.45     |         | $\Delta\alpha = -76.73$                                 |
|     |      | $^2P, M_L = 0$             | $158.31 \pm 3.63$ | --       | CCSD(T) |                                                         |
|     |      | $^2P, M_L = \pm 1$         | $83.76 \pm 0.21$  | --       |         |                                                         |
|     |      | $^2P$                      | $108.61 \pm 2.1$  | --       |         | $\Delta\alpha = -74.55$                                 |
|     |      | $^2P, M_L = 0$             | $190.90 \pm 0.54$ | 30.02    | DHF     | <a href="#">2C-SR-CC@dyall.acv4z@(core 35)[vir 305]</a> |
|     |      | $^2P, M_L = \pm 1$         | $60.33 \pm 0.04$  | 16.73    |         |                                                         |
|     |      | $^2P$                      | $103.85 \pm 0.32$ | 24.53    |         | $\Delta\alpha = -130.57$                                |
|     |      | $^2P, M_L = 0$             | $101.95 \pm 0.3$  | -30.56   | MP2     |                                                         |
|     |      | $^2P, M_L = \pm 1$         | $61.24 \pm 0.26$  | 18.49    |         |                                                         |
|     |      | $^2P$                      | $74.81 \pm 0.27$  | -10.30   |         | $\Delta\alpha = -40.71$                                 |
|     |      | $^2P, M_L = 0$             | $150.31 \pm 0.3$  | 2.38     | CCSD    |                                                         |
|     |      | $^2P, M_L = \pm 1$         | $52.51 \pm 0.03$  | 1.59     |         |                                                         |
|     |      | $^2P$                      | $85.11 \pm 0.18$  | 2.05     |         | $\Delta\alpha = -97.81$                                 |
|     |      | $^2P, M_L = 0$             | $146.82 \pm 0.29$ | --       | CCSD(T) |                                                         |
|     |      | $^2P, M_L = \pm 1$         | $51.68 \pm 0.03$  | --       |         |                                                         |
|     |      | $^2P$                      | $83.40 \pm 0.17$  | --       |         | $\Delta\alpha = -95.14$                                 |
|     |      | $^2P, M_L = 0$             | $190.90 \pm 0.54$ | 30.44    | DHF     | <a href="#">2C-SR-CC@dyall.acv4z@(core 45)[vir 305]</a> |
|     |      | $^2P, M_L = \pm 1$         | $60.33 \pm 0.04$  | 17.31    |         |                                                         |
|     |      | $^2P$                      | $103.85 \pm 0.32$ | 25.02    |         | $\Delta\alpha = -130.57$                                |
|     |      | $^2P, M_L = 0$             | $100.48 \pm 0.28$ | -31.35   | MP2     |                                                         |
|     |      | $^2P, M_L = \pm 1$         | $60.53 \pm 0.11$  | 17.70    |         |                                                         |
|     |      | $^2P$                      | $73.84 \pm 0.19$  | -11.11   |         | $\Delta\alpha = -39.95$                                 |
|     |      | $^2P, M_L = 0$             | $149.47 \pm 0.3$  | 2.13     | CCSD    |                                                         |
|     |      | $^2P, M_L = \pm 1$         | $52.38 \pm 0.03$  | 1.85     |         |                                                         |
|     |      | $^2P$                      | $84.74 \pm 0.17$  | 2.01     |         | $\Delta\alpha = -97.09$                                 |

(continued)

Table S11. continued.

| Z | Atom | State                      | $\alpha_D$ (a.u.) | $\delta$ | Method  | Comments                                         |
|---|------|----------------------------|-------------------|----------|---------|--------------------------------------------------|
|   |      | $^2P, M_L = 0$             | $146.35 \pm 0.29$ | --       | CCSD(T) |                                                  |
|   |      | $^2P, M_L = \pm 1$         | $51.43 \pm 0.03$  | --       |         |                                                  |
|   |      | $^2P$                      | $83.07 \pm 0.17$  | --       |         | $\Delta\alpha = -94.93$                          |
|   |      | $^2P_{1/2}$                | $32.55 \pm 0.01$  | -0.30    | DHF     | 2C-DC-CC@d-aug-dyall.acv4z@(core 51)[vir 449]    |
|   |      |                            | $32.30 \pm 0.01$  | -1.07    | MP2     |                                                  |
|   |      |                            | $32.65 \pm 0.01$  | --       | CCSD    |                                                  |
|   |      | $^2P_{1/2}$                | $32.51 \pm 0.01$  | -1.07    | DHF     | 2C-DC-CC@dyall.acv4z@(core 49)[vir 305]          |
|   |      |                            | $32.28 \pm 0.01$  | -1.78    | MP2     |                                                  |
|   |      |                            | $32.66 \pm 0.01$  | -0.61    | CCSD    |                                                  |
|   |      |                            | $32.86 \pm 0.01$  | --       | CCSD(T) |                                                  |
|   |      | $^2P_{1/2}$                | $32.67 \pm 0.01$  | -1.02    | DHF     | 4C-DC-CC@dyall.acv4z@(core 13)[vir 271]          |
|   |      |                            | $34.28 \pm 0.72$  | 3.87     | MP2     |                                                  |
|   |      |                            | $32.77 \pm 0.01$  | -0.71    | CCSD    |                                                  |
|   |      |                            | $33.00 \pm 0.02$  | --       | CCSD(T) |                                                  |
|   |      | $^2P_{1/2}$                | $32.67 \pm 0.01$  | -0.23    | DHF     | 4C-DC-CC@dyall.acv4z@(core 35)[vir 305]          |
|   |      |                            | $33.99 \pm 0.76$  | 3.80     | MP2     |                                                  |
|   |      |                            | $32.47 \pm 0.01$  | -0.82    | CCSD    |                                                  |
|   |      |                            | $32.74 \pm 0.02$  | --       | CCSD(T) |                                                  |
|   |      | $^2P_{1/2}$                | $28.00 \pm 0.02$  |          | MRCISD  | 4C-DC-CI@dyall.acv4z@(core 13)[vir 271]          |
|   |      | $^2P_{3/2}, M_J = \pm 1/2$ | $195.68 \pm 0.56$ |          |         |                                                  |
|   |      | $^2P_{3/2}, M_J = \pm 3/2$ | $71.84 \pm 0.05$  |          |         |                                                  |
|   |      | $^2P_{3/2}$                | $133.76 \pm 0.4$  |          |         | $\bar{\alpha}_{J=3/2} - \alpha_{J=1/2} = 105.76$ |

## S2.4 Group 14 elements

Table S12: The results of dipole polarizability for Group 14 elements.

| Z | Atom | State              | $\alpha_D$ (a.u.) | $\delta$ (%) | Method | Comments                               |
|---|------|--------------------|-------------------|--------------|--------|----------------------------------------|
| 6 | C    | $^3P, M_L = 0$     | 9.99              | -3.08        | DHF    | 2C-NR-CC@dyall.acv4z@(core 6)[vir 250] |
|   |      | $^3P, M_L = \pm 1$ | 12.09             | -3.00        |        |                                        |
|   |      | $^3P$              | 11.39             | -3.02        |        |                                        |
|   |      | $^3P, M_L = 0$     | $10.47 \pm 0.01$  | 1.57         | MP2    | $\Delta\alpha = 2.10$                  |
|   |      | $^3P, M_L = \pm 1$ | $12.15 \pm 0.04$  | -2.56        |        |                                        |
|   |      | $^3P$              | $11.59 \pm 0.03$  | -1.35        |        |                                        |
|   |      | $^3P, M_L = 0$     | 10.25             | -0.55        | CCSD   | $\Delta\alpha = 1.68$                  |

(continued)

Table S12. continued.

| Z  | Atom | State              | $\alpha_D$ (a.u.) | $\delta$ | Method  | Comments                                |
|----|------|--------------------|-------------------|----------|---------|-----------------------------------------|
|    |      | $^3P, M_L = \pm 1$ | $12.40 \pm 0.01$  | -0.55    | CCSD(T) | $\Delta\alpha = 2.15$                   |
|    |      | $^3P$              | $11.68 \pm 0.01$  | -0.55    |         |                                         |
|    |      | $^3P, M_L = 0$     | 10.31             | --       |         |                                         |
|    |      | $^3P, M_L = \pm 1$ | $12.46 \pm 0.01$  | --       |         |                                         |
|    |      | $^3P$              | $11.75 \pm 0.01$  | --       |         | $\Delta\alpha = 2.16$                   |
|    |      | $^3P, M_L = 0$     | 9.98              | -3.21    | DHF     | 2C-SR-CC@dyall.acv4z@(core 6)[vir 176]  |
|    |      | $^3P, M_L = \pm 1$ | 12.09             | -3.14    | MP2     | $\Delta\alpha = 2.11$                   |
|    |      | $^3P$              | 11.39             | -3.16    |         |                                         |
|    |      | $^3P, M_L = 0$     | $10.49 \pm 0.01$  | 1.68     |         |                                         |
|    |      | $^3P, M_L = \pm 1$ | $12.24 \pm 0.02$  | -1.92    |         |                                         |
|    |      | $^3P$              | $11.66 \pm 0.02$  | -0.87    |         | $\Delta\alpha = 1.75$                   |
|    |      | $^3P, M_L = 0$     | 10.26             | -0.55    | CCSD    | $\Delta\alpha = 2.15$                   |
|    |      | $^3P, M_L = \pm 1$ | $12.41 \pm 0.01$  | -0.57    |         |                                         |
|    |      | $^3P$              | $11.69 \pm 0.01$  | -0.57    |         |                                         |
|    |      | $^3P, M_L = 0$     | 10.31             | --       |         |                                         |
|    |      | $^3P, M_L = \pm 1$ | $12.48 \pm 0.01$  | --       |         |                                         |
|    |      | $^3P$              | $11.76 \pm 0.01$  | --       | CCSD(T) | $\Delta\alpha = 2.17$                   |
|    |      | $^3P, M_L = 0$     | 9.98              | -3.12    | DHF     | 2C-SR-CC@dyall.acv4z@(core 6)[vir 250]  |
|    |      | $^3P, M_L = \pm 1$ | 12.09             | -3.03    | MP2     | $\Delta\alpha = 2.11$                   |
|    |      | $^3P$              | 11.39             | -3.06    |         |                                         |
|    |      | $^3P, M_L = 0$     | $10.59 \pm 0.02$  | 2.84     |         |                                         |
|    |      | $^3P, M_L = \pm 1$ | $12.17 \pm 0.03$  | -2.35    |         |                                         |
|    |      | $^3P$              | $11.65 \pm 0.03$  | -0.83    |         | $\Delta\alpha = 1.58$                   |
|    |      | $^3P, M_L = 0$     | 10.24             | -0.60    | CCSD    | $\Delta\alpha = 2.15$                   |
|    |      | $^3P, M_L = \pm 1$ | $12.39 \pm 0.01$  | -0.57    |         |                                         |
|    |      | $^3P$              | 11.68             | -0.58    |         |                                         |
|    |      | $^3P, M_L = 0$     | 10.30             | --       |         |                                         |
|    |      | $^3P, M_L = \pm 1$ | $12.46 \pm 0.01$  | --       |         |                                         |
|    |      | $^3P$              | $11.74 \pm 0.01$  | --       | CCSD(T) | $\Delta\alpha = 2.16$                   |
|    |      | $^3P_0$            | 11.76             | 0.30     | DHF     | 4C-DC-CC@dyall.acv4z@(core 6)[vir 250]  |
|    |      |                    | 12.05             | 2.74     | MP2     |                                         |
|    |      |                    | 11.63             | -0.86    | CCSD    |                                         |
|    |      |                    | 11.73             | --       | CCSD(T) |                                         |
| 14 | Si   | $^3P, M_L = 0$     | $33.24 \pm 0.02$  | 4.21     | DHF     | 2C-NR-CC@dyall.acv4z@(core 14)[vir 362] |
|    |      | $^3P, M_L = \pm 1$ | $42.69 \pm 0.1$   | 3.27     | MP2     | $\Delta\alpha = 9.45$                   |
|    |      | $^3P$              | $39.54 \pm 0.09$  | 3.53     |         |                                         |
|    |      | $^3P, M_L = 0$     | $34.02 \pm 0.06$  | 6.65     |         |                                         |
|    |      | $^3P, M_L = \pm 1$ | $40.99 \pm 0.12$  | -0.85    |         |                                         |

(continued)

Table S12. continued.

| Z  | Atom | State              | $\alpha_D$ (a.u.) | $\delta$ | Method  | Comments                                       |
|----|------|--------------------|-------------------|----------|---------|------------------------------------------------|
|    |      | $^3P$              | $38.66 \pm 0.11$  | 1.23     | CCSD    | $\Delta\alpha = 6.97$                          |
|    |      | $^3P, M_L = 0$     | $31.80 \pm 0.02$  | -0.32    |         |                                                |
|    |      | $^3P, M_L = \pm 1$ | $41.28 \pm 0.1$   | -0.14    |         |                                                |
|    |      | $^3P$              | $38.12 \pm 0.08$  | -0.19    | CCSD(T) | $\Delta\alpha = 9.48$                          |
|    |      | $^3P, M_L = 0$     | $31.90 \pm 0.02$  | --       |         |                                                |
|    |      | $^3P, M_L = \pm 1$ | $41.34 \pm 0.1$   | --       |         |                                                |
|    |      | $^3P$              | $38.19 \pm 0.09$  | --       |         | $\Delta\alpha = 9.44$                          |
|    |      | $^3P, M_L = 0$     | $33.17 \pm 0.02$  | 4.19     | DHF     | <b>2C-SR-CC@dyall.acv4z@(core 14)[vir 362]</b> |
|    |      | $^3P, M_L = \pm 1$ | $42.78 \pm 0.1$   | 3.23     |         |                                                |
|    |      | $^3P$              | $39.58 \pm 0.08$  | 3.50     | MP2     | $\Delta\alpha = 9.60$                          |
|    |      | $^3P, M_L = 0$     | $34.05 \pm 0.05$  | 6.93     |         |                                                |
|    |      | $^3P, M_L = \pm 1$ | $41.13 \pm 0.11$  | -0.75    |         |                                                |
|    |      | $^3P$              | $38.77 \pm 0.09$  | 1.38     | CCSD    | $\Delta\alpha = 7.08$                          |
|    |      | $^3P, M_L = 0$     | $31.73 \pm 0.02$  | -0.33    |         |                                                |
|    |      | $^3P, M_L = \pm 1$ | $41.38 \pm 0.09$  | -0.15    |         |                                                |
|    |      | $^3P$              | $38.16 \pm 0.08$  | -0.20    | CCSD(T) | $\Delta\alpha = 9.64$                          |
|    |      | $^3P, M_L = 0$     | $31.84 \pm 0.02$  | --       |         |                                                |
|    |      | $^3P, M_L = \pm 1$ | $41.44 \pm 0.1$   | --       |         |                                                |
|    |      | $^3P$              | $38.24 \pm 0.08$  | --       |         | $\Delta\alpha = 9.60$                          |
|    |      | $^3P_0$            | $41.84 \pm 0.01$  | 12.80    | DHF     | <b>2C-DC-CC@dyall.acv4z@(core 14)[vir 362]</b> |
|    |      |                    | $40.53 \pm 0.01$  | 9.25     | MP2     |                                                |
|    |      |                    | $37.66 \pm 0.01$  | 1.52     | CCSD    |                                                |
|    |      |                    | $37.10 \pm 0.01$  | --       | CCSD(T) |                                                |
| 32 | Ge   | $^3P, M_L = 0$     | 34.48             | 5.98     | DHF     | <b>2C-NR-CC@dyall.acv4z@(core 32)[vir 480]</b> |
|    |      | $^3P, M_L = \pm 1$ | $45.12 \pm 0.01$  | 3.58     |         |                                                |
|    |      | $^3P$              | $41.58 \pm 0.01$  | 4.24     | MP2     | $\Delta\alpha = 10.64$                         |
|    |      | $^3P, M_L = 0$     | $35.28 \pm 0.67$  | 8.42     |         |                                                |
|    |      | $^3P, M_L = \pm 1$ | $41.51 \pm 0.66$  | -4.72    |         |                                                |
|    |      | $^3P$              | $39.43 \pm 0.66$  | -1.15    | CCSD    | $\Delta\alpha = 6.23$                          |
|    |      | $^3P, M_L = 0$     | 32.54             | 0.02     |         |                                                |
|    |      | $^3P, M_L = \pm 1$ | $43.56 \pm 0.01$  | -0.01    |         |                                                |
|    |      | $^3P$              | $39.89 \pm 0.01$  | 0.00     | CCSD(T) | $\Delta\alpha = 11.01$                         |
|    |      | $^3P, M_L = 0$     | $32.54 \pm 0.02$  | --       |         |                                                |
|    |      | $^3P, M_L = \pm 1$ | $43.56 \pm 0.04$  | --       |         |                                                |
|    |      | $^3P$              | $39.89 \pm 0.03$  | --       |         | $\Delta\alpha = 11.02$                         |
|    |      | $^3P, M_L = 0$     | 33.74             | 6.09     | DHF     | <b>2C-SR-CC@dyall.acv4z@(core 22)[vir 246]</b> |
|    |      | $^3P, M_L = \pm 1$ | $45.20 \pm 0.01$  | 3.22     |         |                                                |
|    |      | $^3P$              | $41.38 \pm 0.01$  | 3.98     |         | $\Delta\alpha = 11.46$                         |

(continued)



Table S12. continued.

| Z  | Atom | State              | $\alpha_D$ (a.u.) | $\delta$ | Method  | Comments                                       |
|----|------|--------------------|-------------------|----------|---------|------------------------------------------------|
|    |      | $^3P, M_L = 0$     | $33.52 \pm 0.18$  | 5.38     | MP2     |                                                |
|    |      | $^3P, M_L = \pm 1$ | $42.60 \pm 0.1$   | -2.72    |         |                                                |
|    |      | $^3P$              | $39.57 \pm 0.13$  | -0.56    |         | $\Delta\alpha = 9.08$                          |
|    |      | $^3P, M_L = 0$     | 31.87             | 0.20     | CCSD    |                                                |
|    |      | $^3P, M_L = \pm 1$ | $43.71 \pm 0.01$  | -0.19    |         |                                                |
|    |      | $^3P$              | $39.76 \pm 0.01$  | -0.08    |         | $\Delta\alpha = 11.84$                         |
|    |      | $^3P, M_L = 0$     | $31.80 \pm 0.01$  | --       | CCSD(T) |                                                |
|    |      | $^3P, M_L = \pm 1$ | $43.79 \pm 0.01$  | --       |         |                                                |
|    |      | $^3P$              | $39.79 \pm 0.01$  | --       |         | $\Delta\alpha = 11.98$                         |
|    |      | $^3P, M_L = 0$     | 33.74             | 6.12     | DHF     | <b>2C-SR-CC@dyall.acv4z@(core 32)[vir 480]</b> |
|    |      | $^3P, M_L = \pm 1$ | $45.20 \pm 0.01$  | 3.43     |         |                                                |
|    |      | $^3P$              | $41.38 \pm 0.01$  | 4.15     |         | $\Delta\alpha = 11.46$                         |
|    |      | $^3P, M_L = 0$     | $33.82 \pm 0.01$  | 6.37     | MP2     |                                                |
|    |      | $^3P, M_L = \pm 1$ | $41.89 \pm 0.36$  | -4.14    |         |                                                |
|    |      | $^3P$              | $39.20 \pm 0.29$  | -1.34    |         | $\Delta\alpha = 8.07$                          |
|    |      | $^3P, M_L = 0$     | 31.84             | 0.14     | CCSD    |                                                |
|    |      | $^3P, M_L = \pm 1$ | $43.67 \pm 0.01$  | -0.06    |         |                                                |
|    |      | $^3P$              | $39.73 \pm 0.01$  | -0.01    |         | $\Delta\alpha = 11.83$                         |
|    |      | $^3P, M_L = 0$     | $31.79 \pm 0.01$  | --       | CCSD(T) |                                                |
|    |      | $^3P, M_L = \pm 1$ | $43.70 \pm 0.02$  | --       |         |                                                |
|    |      | $^3P$              | $39.73 \pm 0.02$  | --       |         | $\Delta\alpha = 11.90$                         |
|    |      | $^3P_0$            | $44.03 \pm 0.02$  | 12.05    | DHF     | <b>2C-DC-CC@dyall.acv4z@(core 22)[vir 246]</b> |
|    |      |                    | $41.54 \pm 0.01$  | 5.71     | MP2     |                                                |
|    |      |                    | $40.04 \pm 0.01$  | 1.89     | CCSD    |                                                |
|    |      |                    | $39.30 \pm 0.01$  | --       | CCSD(T) |                                                |
| 50 | Sn   | $^3P, M_L = 0$     | $51.07 \pm 0.01$  | 8.07     | DHF     | <b>2C-NR-CC@dyall.acv4z@(core 50)[vir 552]</b> |
|    |      | $^3P, M_L = \pm 1$ | $62.89 \pm 0.02$  | 5.05     |         |                                                |
|    |      | $^3P$              | $58.95 \pm 0.02$  | 5.91     |         | $\Delta\alpha = 11.82$                         |
|    |      | $^3P, M_L = 0$     | $50.83 \pm 1.03$  | 7.57     | MP2     |                                                |
|    |      | $^3P, M_L = \pm 1$ | $57.66 \pm 0.1$   | -3.68    |         |                                                |
|    |      | $^3P$              | $55.38 \pm 0.6$   | -0.50    |         | $\Delta\alpha = 6.83$                          |
|    |      | $^3P, M_L = 0$     | 47.31             | 0.13     | CCSD    |                                                |
|    |      | $^3P, M_L = \pm 1$ | $60.02 \pm 0.02$  | 0.27     |         |                                                |
|    |      | $^3P$              | $55.79 \pm 0.02$  | 0.23     |         | $\Delta\alpha = 12.71$                         |
|    |      | $^3P, M_L = 0$     | $47.25 \pm 0.03$  | --       | CCSD(T) |                                                |
|    |      | $^3P, M_L = \pm 1$ | $59.86 \pm 0.03$  | --       |         |                                                |
|    |      | $^3P$              | $55.66 \pm 0.03$  | --       |         | $\Delta\alpha = 12.61$                         |
|    |      | $^3P, M_L = 0$     | $47.78 \pm 0.01$  | 7.89     | DHF     | <b>2C-SR-CC@dyall.acv4z@(core 32)[vir 302]</b> |

(continued)

Table S12. continued.

| Z  | Atom | State              | $\alpha_D$ (a.u.) | $\delta$ | Method  | Comments                                       |
|----|------|--------------------|-------------------|----------|---------|------------------------------------------------|
|    |      | $^3P, M_L = \pm 1$ | $62.32 \pm 0.02$  | 4.45     | MP2     | $\Delta\alpha = 14.54$                         |
|    |      | $^3P$              | $57.48 \pm 0.02$  | 5.38     |         |                                                |
|    |      | $^3P, M_L = 0$     | $47.17 \pm 0.01$  | 6.51     |         |                                                |
|    |      | $^3P, M_L = \pm 1$ | $57.86 \pm 0.38$  | -3.03    |         |                                                |
|    |      | $^3P$              | $54.30 \pm 0.31$  | -0.45    | CCSD    | $\Delta\alpha = 10.69$                         |
|    |      | $^3P, M_L = 0$     | $44.32 \pm 0.01$  | 0.09     |         |                                                |
|    |      | $^3P, M_L = \pm 1$ | $59.77 \pm 0.02$  | 0.16     |         |                                                |
|    |      | $^3P$              | $54.62 \pm 0.02$  | 0.14     |         |                                                |
|    |      | $^3P, M_L = 0$     | $44.28 \pm 0.01$  | --       | CCSD(T) | $\Delta\alpha = 15.44$                         |
|    |      | $^3P, M_L = \pm 1$ | $59.67 \pm 0.02$  | --       |         |                                                |
|    |      | $^3P$              | $54.54 \pm 0.02$  | --       |         |                                                |
|    |      | $^3P, M_L = 0$     | $47.78 \pm 0.01$  | 7.86     | DHF     | <b>2C-SR-CC@dyall.acv4z@(core 50)[vir 552]</b> |
|    |      | $^3P, M_L = \pm 1$ | $62.32 \pm 0.02$  | 4.54     |         |                                                |
|    |      | $^3P$              | $57.48 \pm 0.02$  | 5.44     |         |                                                |
|    |      | $^3P, M_L = 0$     | $47.57 \pm 0.28$  | 7.38     |         |                                                |
|    |      | $^3P, M_L = \pm 1$ | $56.47 \pm 0.65$  | -5.28    | MP2     | $\Delta\alpha = 8.90$                          |
|    |      | $^3P$              | $53.50 \pm 0.56$  | -1.85    |         |                                                |
|    |      | $^3P, M_L = 0$     | $44.31 \pm 0.01$  | 0.03     |         |                                                |
|    |      | $^3P, M_L = \pm 1$ | $59.75 \pm 0.02$  | 0.23     |         |                                                |
|    |      | $^3P$              | $54.60 \pm 0.02$  | 0.18     | CCSD    | $\Delta\alpha = 15.44$                         |
|    |      | $^3P, M_L = 0$     | 44.30             | --       |         |                                                |
|    |      | $^3P, M_L = \pm 1$ | $59.62 \pm 0.04$  | --       |         |                                                |
|    |      | $^3P$              | $54.51 \pm 0.04$  | --       |         |                                                |
|    |      | $^3P_0$            | $57.62 \pm 0.02$  | 10.44    | DHF     | <b>2C-DC-CC@dyall.acv4z@(core 32)[vir 302]</b> |
|    |      |                    | $53.40 \pm 0.02$  | 2.35     |         |                                                |
|    |      |                    | $52.85 \pm 0.02$  | 1.30     |         |                                                |
|    |      |                    | $52.17 \pm 0.02$  | --       |         |                                                |
| 82 | Pb   | $^3P, M_L = 0$     | $59.76 \pm 0.09$  | 9.40     | DHF     | <b>2C-NR-CC@dyall.acv4z@(core 46)[vir 308]</b> |
|    |      | $^3P, M_L = \pm 1$ | $76.35 \pm 0.43$  | 5.83     |         |                                                |
|    |      | $^3P$              | $70.82 \pm 0.36$  | 6.81     |         |                                                |
|    |      | $^3P, M_L = 0$     | $59.88 \pm 0.34$  | 9.63     |         |                                                |
|    |      | $^3P, M_L = \pm 1$ | $68.10 \pm 0.28$  | -5.61    | MP2     | $\Delta\alpha = 16.59$                         |
|    |      | $^3P$              | $65.36 \pm 0.3$   | -1.43    |         |                                                |
|    |      | $^3P, M_L = 0$     | $54.70 \pm 0.07$  | 0.14     |         |                                                |
|    |      | $^3P, M_L = \pm 1$ | $72.36 \pm 0.39$  | 0.30     |         |                                                |
|    |      | $^3P$              | $66.47 \pm 0.32$  | 0.26     | CCSD    | $\Delta\alpha = 17.66$                         |
|    |      | $^3P, M_L = 0$     | $54.62 \pm 0.08$  | --       |         |                                                |
|    |      | $^3P, M_L = \pm 1$ | $72.14 \pm 0.38$  | --       |         |                                                |
|    |      |                    |                   |          |         |                                                |

(continued)

Table S12. continued.

| Z   | Atom | State              | $\alpha_D$ (a.u.) | $\delta$ | Method  | Comments                                       |
|-----|------|--------------------|-------------------|----------|---------|------------------------------------------------|
|     |      | $^3P$              | $66.30 \pm 0.31$  | --       |         | $\Delta\alpha = 17.52$                         |
|     |      | $^3P, M_L = 0$     | $48.78 \pm 0.08$  | 8.22     | DHF     | <b>2C-SR-CC@dyall.acv4z@(core 46)[vir 308]</b> |
|     |      | $^3P, M_L = \pm 1$ | $76.70 \pm 0.52$  | 6.06     |         |                                                |
|     |      | $^3P$              | $67.40 \pm 0.43$  | 6.58     |         | $\Delta\alpha = 27.92$                         |
|     |      | $^3P, M_L = 0$     | $52.86 \pm 0.37$  | 17.27    | MP2     |                                                |
|     |      | $^3P, M_L = \pm 1$ | $66.70 \pm 0.25$  | -7.77    |         |                                                |
|     |      | $^3P$              | $62.08 \pm 0.3$   | -1.82    |         | $\Delta\alpha = 13.84$                         |
|     |      | $^3P, M_L = 0$     | $45.03 \pm 0.07$  | -0.11    | CCSD    |                                                |
|     |      | $^3P, M_L = \pm 1$ | $72.46 \pm 0.42$  | 0.20     |         |                                                |
|     |      | $^3P$              | $63.32 \pm 0.35$  | 0.13     |         | $\Delta\alpha = 27.43$                         |
|     |      | $^3P, M_L = 0$     | $45.08 \pm 0.08$  | --       | CCSD(T) |                                                |
|     |      | $^3P, M_L = \pm 1$ | $72.32 \pm 0.42$  | --       |         |                                                |
|     |      | $^3P$              | $63.24 \pm 0.34$  | --       |         | $\Delta\alpha = 27.24$                         |
|     |      | $^3P_0$            | $49.67 \pm 0.02$  | 6.29     | DHF     | <b>2C-DC-CC@dyall.acv4z@(core 46)[vir 308]</b> |
|     |      |                    | $46.77 \pm 0.02$  | 0.08     | MP2     |                                                |
|     |      |                    | $46.76 \pm 0.02$  | 0.06     | CCSD    |                                                |
|     |      |                    | $46.73 \pm 0.02$  | --       | CCSD(T) |                                                |
| 114 | Fl   | $^3P, M_L = 0$     | $78.53 \pm 0.13$  | 10.69    | DHF     | <b>2C-NR-CC@dyall.acv4z@(core 52)[vir 302]</b> |
|     |      | $^3P, M_L = \pm 1$ | $97.18 \pm 0.66$  | 7.18     |         |                                                |
|     |      | $^3P$              | $90.96 \pm 0.55$  | 8.16     |         | $\Delta\alpha = 18.65$                         |
|     |      | $^3P, M_L = 0$     | $76.79 \pm 0.47$  | 8.24     | MP2     |                                                |
|     |      | $^3P, M_L = \pm 1$ | $84.81 \pm 0.48$  | -6.46    |         |                                                |
|     |      | $^3P$              | $82.14 \pm 0.47$  | -2.33    |         | $\Delta\alpha = 8.02$                          |
|     |      | $^3P, M_L = 0$     | $71.18 \pm 0.1$   | 0.33     | CCSD    |                                                |
|     |      | $^3P, M_L = \pm 1$ | $91.14 \pm 0.58$  | 0.52     |         |                                                |
|     |      | $^3P$              | $84.49 \pm 0.48$  | 0.47     |         | $\Delta\alpha = 19.97$                         |
|     |      | $^3P, M_L = 0$     | $70.95 \pm 0.12$  | --       | CCSD(T) |                                                |
|     |      | $^3P, M_L = \pm 1$ | $90.67 \pm 0.57$  | --       |         |                                                |
|     |      | $^3P$              | $84.10 \pm 0.47$  | --       |         | $\Delta\alpha = 19.72$                         |
|     |      | $^3P, M_L = 0$     | $52.39 \pm 0.12$  | 8.77     | DHF     | 2C-SR-CC@dyall.acv4z@(core 46)[vir 302]        |
|     |      | $^3P, M_L = \pm 1$ | $109.13 \pm 0.95$ | 13.82    |         |                                                |
|     |      | $^3P$              | $90.22 \pm 0.78$  | 12.81    |         | $\Delta\alpha = 56.74$                         |
|     |      | $^3P, M_L = 0$     | $60.48 \pm 0.45$  | 25.56    | MP2     |                                                |
|     |      | $^3P, M_L = \pm 1$ | $83.04 \pm 0.39$  | -13.39   |         |                                                |
|     |      | $^3P$              | $75.52 \pm 0.41$  | -5.57    |         | $\Delta\alpha = 22.56$                         |
|     |      | $^3P, M_L = 0$     | $48.38 \pm 0.12$  | 0.44     | CCSD    |                                                |
|     |      | $^3P, M_L = \pm 1$ | $96.69 \pm 0.69$  | 0.85     |         |                                                |
|     |      | $^3P$              | $80.59 \pm 0.56$  | 0.77     |         | $\Delta\alpha = 48.32$                         |

(continued)

Table S12. continued.

| Z | Atom | State              | $\alpha_D$ (a.u.) | $\delta$ | Method  | Comments                                       |
|---|------|--------------------|-------------------|----------|---------|------------------------------------------------|
|   |      | $^3P, M_L = 0$     | $48.17 \pm 0.12$  | --       | CCSD(T) |                                                |
|   |      | $^3P, M_L = \pm 1$ | $95.88 \pm 0.66$  | --       |         |                                                |
|   |      | $^3P$              | $79.98 \pm 0.55$  | --       |         | $\Delta\alpha = 47.71$                         |
|   |      | $^3P, M_L = 0$     | $52.39 \pm 0.13$  | 8.63     | DHF     | <b>2C-SR-CC@dyall.acv4z@(core 52)[vir 302]</b> |
|   |      | $^3P, M_L = \pm 1$ | $109.14 \pm 1.02$ | 13.52    |         |                                                |
|   |      | $^3P$              | $90.23 \pm 0.83$  | 12.54    |         | $\Delta\alpha = 56.75$                         |
|   |      | $^3P, M_L = 0$     | $60.61 \pm 0.48$  | 25.66    | MP2     |                                                |
|   |      | $^3P, M_L = \pm 1$ | $83.43 \pm 0.42$  | -13.23   |         |                                                |
|   |      | $^3P$              | $75.82 \pm 0.44$  | -5.43    |         | $\Delta\alpha = 22.82$                         |
|   |      | $^3P, M_L = 0$     | $48.48 \pm 0.13$  | 0.53     | CCSD    |                                                |
|   |      | $^3P, M_L = \pm 1$ | $96.94 \pm 0.74$  | 0.82     |         |                                                |
|   |      | $^3P$              | $80.79 \pm 0.61$  | 0.76     |         | $\Delta\alpha = 48.45$                         |
|   |      | $^3P, M_L = 0$     | $48.23 \pm 0.13$  | --       | CCSD(T) |                                                |
|   |      | $^3P, M_L = \pm 1$ | $96.15 \pm 0.72$  | --       |         |                                                |
|   |      | $^3P$              | $80.18 \pm 0.59$  | --       |         | $\Delta\alpha = 47.92$                         |
|   |      | $^3P_0$            | 29.94             | -2.89    | DHF     | <b>2C-DC-CC@dyall.acv4z@(core 50)[vir 302]</b> |
|   |      |                    | $31.46 \pm 0.01$  | 2.05     | MP2     |                                                |
|   |      |                    | 30.45             | -1.25    | CCSD    |                                                |
|   |      |                    | $30.83 \pm 0.01$  | --       | CCSD(T) |                                                |

## S2.5 Group 15 elements

Table S13: The results of dipole polarizability for Group 15 elements.

| Z | Atom | State          | $\alpha_D$ (a.u.) | $\delta$ (%) | Method  | Comments                                      |
|---|------|----------------|-------------------|--------------|---------|-----------------------------------------------|
| 7 | N    | $^4S, M_L = 0$ | 6.80              | -6.32        | DHF     | <b>2C-NR-CC@dyall.acv4z@(core 7)[vir 249]</b> |
|   |      |                | 7.10              | -2.22        | MP2     |                                               |
|   |      |                | 7.20              | -0.81        | CCSD    |                                               |
|   |      |                | 7.26              | --           | CCSD(T) |                                               |
|   |      | $^4S, M_L = 0$ | 6.80              | -6.76        | DHF     | <b>2C-SR-CC@dyall.acv4z@(core 7)[vir 159]</b> |
|   |      |                | 7.13              | -2.22        | MP2     |                                               |
|   |      |                | 7.24              | -0.78        | CCSD    |                                               |
|   |      |                | 7.29              | --           | CCSD(T) |                                               |
|   |      | $^4S, M_L = 0$ | 6.80              | -6.33        | DHF     | <b>2C-SR-CC@dyall.acv4z@(core 7)[vir 249]</b> |
|   |      |                | 7.10              | -2.21        | MP2     |                                               |

(continued)

Table S13. continued.

| Z  | Atom | State                      | $\alpha_D$ (a.u.) | $\delta$ | Method  | Comments                                                |
|----|------|----------------------------|-------------------|----------|---------|---------------------------------------------------------|
| 15 | P    | $^4S_{3/2}, M_J = \pm 1/2$ | 7.20              | -0.81    | CCSD    | <a href="#">4C-DC-CI@dyall.acv4z@(core 7)[vir 159]</a>  |
|    |      |                            | 7.26              | --       | CCSD(T) |                                                         |
|    |      |                            | 7.20              |          | MRCISD  |                                                         |
|    |      |                            | 7.20              |          |         |                                                         |
|    |      |                            | 7.20              |          |         |                                                         |
|    |      | $^4S_{3/2}$                | 7.20              |          |         |                                                         |
|    |      | $^4S, M_L = 0$             | 25.17 $\pm$ 0.02  | -0.00    | DHF     | <a href="#">2C-NR-CC@dyall.acv4z@(core 15)[vir 361]</a> |
|    |      |                            | 25.05 $\pm$ 0.01  | -0.49    | MP2     |                                                         |
|    |      |                            | 25.10 $\pm$ 0.02  | -0.29    | CCSD    |                                                         |
|    |      |                            | 25.17 $\pm$ 0.02  | --       | CCSD(T) |                                                         |
| 15 | P    | $^4S, M_L = 0$             | 25.18 $\pm$ 0.02  | -0.94    | DHF     | <a href="#">2C-SR-CC@dyall.acv4z@(core 15)[vir 185]</a> |
|    |      |                            | 25.32 $\pm$ 0.02  | -0.37    | MP2     |                                                         |
|    |      |                            | 25.34 $\pm$ 0.02  | -0.30    | CCSD    |                                                         |
|    |      |                            | 25.42 $\pm$ 0.02  | --       | CCSD(T) |                                                         |
|    |      | $^4S, M_L = 0$             | 25.18 $\pm$ 0.01  | -0.04    | DHF     | <a href="#">2C-SR-CC@dyall.acv4z@(core 15)[vir 361]</a> |
|    |      |                            | 25.07 $\pm$ 0.01  | -0.47    | MP2     |                                                         |
|    |      |                            | 25.12 $\pm$ 0.02  | -0.30    | CCSD    |                                                         |
|    |      |                            | 25.19 $\pm$ 0.02  | --       | CCSD(T) |                                                         |
|    |      | $^4S_{3/2}, M_J = \pm 1/2$ | 24.85             |          | MRCISD  | <a href="#">4C-DC-CI@dyall.acv4z@(core 15)[vir 185]</a> |
|    |      | $^4S_{3/2}, M_J = \pm 3/2$ | 24.85             |          |         |                                                         |
| 33 | As   | $^4S, M_L = 0$             | 30.03             | 0.59     | DHF     | <a href="#">2C-NR-CC@dyall.acv4z@(core 33)[vir 479]</a> |
|    |      |                            | 29.60 $\pm$ 0.03  | -0.84    | MP2     |                                                         |
|    |      |                            | 29.78             | -0.21    | CCSD    |                                                         |
|    |      |                            | 29.85             | --       | CCSD(T) |                                                         |
|    |      | $^4S, M_L = 0$             | 29.85             | 0.70     | DHF     | <a href="#">2C-SR-CC@dyall.acv4z@(core 15)[vir 185]</a> |
|    |      |                            | 29.43 $\pm$ 0.03  | -0.71    | MP2     |                                                         |
|    |      |                            | 29.56             | -0.29    | CCSD    |                                                         |
|    |      |                            | 29.64             | --       | CCSD(T) |                                                         |
|    |      | $^4S, M_L = 0$             | 29.85             | 0.44     | DHF     | <a href="#">2C-SR-CC@dyall.acv4z@(core 33)[vir 479]</a> |
|    |      |                            | 29.47 $\pm$ 0.03  | -0.85    | MP2     |                                                         |
|    |      |                            | 29.65             | -0.23    | CCSD    |                                                         |
|    |      |                            | 29.72             | --       | CCSD(T) |                                                         |
| 51 | Sb   | $^4S_{3/2}, M_J = \pm 1/2$ | 29.03             |          | MRCISD  | <a href="#">4C-DC-CI@dyall.acv4z@(core 15)[vir 185]</a> |
|    |      |                            | 28.99             |          |         |                                                         |
|    |      |                            | 29.01             |          |         |                                                         |
|    |      | $^4S, M_L = 0$             | 44.82             | 2.28     | DHF     | <a href="#">2C-NR-CC@dyall.acv4z@(core 51)[vir 551]</a> |
|    |      |                            | 43.07 $\pm$ 0.02  | -1.72    | MP2     |                                                         |
|    |      |                            | 43.84             | 0.03     | CCSD    |                                                         |

(continued)

Table S13. continued.

| Z   | Atom | State                      | $\alpha_D$ (a.u.) | $\delta$ | Method  | Comments                                                |
|-----|------|----------------------------|-------------------|----------|---------|---------------------------------------------------------|
|     |      |                            | 43.83             | --       | CCSD(T) |                                                         |
|     |      | $^4S, M_L = 0$             | $43.74 \pm 0.01$  | 1.44     | DHF     | <a href="#">2C-SR-CC@dyall.acv4z@(core 15)[vir 227]</a> |
|     |      |                            | $42.60 \pm 0.02$  | -1.20    | MP2     |                                                         |
|     |      |                            | $43.08 \pm 0.01$  | -0.09    | CCSD    |                                                         |
|     |      |                            | $43.12 \pm 0.01$  | --       | CCSD(T) |                                                         |
|     |      | $^4S, M_L = 0$             | $43.74 \pm 0.01$  | 1.70     | DHF     | <a href="#">2C-SR-CC@dyall.acv4z@(core 51)[vir 551]</a> |
|     |      |                            | $42.40 \pm 0.02$  | -1.43    | MP2     |                                                         |
|     |      |                            | 42.99             | -0.04    | CCSD    |                                                         |
|     |      |                            | 43.01             | --       | CCSD(T) |                                                         |
|     |      | $^4S_{3/2}, M_J = \pm 1/2$ | $42.29 \pm 0.01$  |          | MRCISD  | <a href="#">4C-DC-CI@dyall.acv4z@(core 15)[vir 227]</a> |
|     |      | $^4S_{3/2}, M_J = \pm 3/2$ | 41.79             |          |         |                                                         |
|     |      | $^4S_{3/2}$                | 42.04             |          |         |                                                         |
| 83  | Bi   | $^4S, M_L = 0$             | $53.74 \pm 0.08$  | 2.59     | DHF     | <a href="#">2C-NR-CC@dyall.acv4z@(core 47)[vir 307]</a> |
|     |      |                            | $51.35 \pm 0.08$  | -1.98    | MP2     |                                                         |
|     |      |                            | $52.41 \pm 0.08$  | 0.05     | CCSD    |                                                         |
|     |      |                            | $52.39 \pm 0.08$  | --       | CCSD(T) |                                                         |
|     |      | $^4S, M_L = 0$             | $50.71 \pm 0.09$  | 1.18     | DHF     | <a href="#">2C-SR-CC@dyall.acv4z@(core 15)[vir 265]</a> |
|     |      |                            | $49.46 \pm 0.09$  | -1.31    | MP2     |                                                         |
|     |      |                            | $50.05 \pm 0.09$  | -0.13    | CCSD    |                                                         |
|     |      |                            | $50.12 \pm 0.09$  | --       | CCSD(T) |                                                         |
|     |      | $^4S, M_L = 0$             | $50.71 \pm 0.09$  | 1.55     | DHF     | <a href="#">2C-SR-CC@dyall.acv4z@(core 47)[vir 307]</a> |
|     |      |                            | $49.06 \pm 0.08$  | -1.75    | MP2     |                                                         |
|     |      |                            | $49.88 \pm 0.08$  | -0.12    | CCSD    |                                                         |
|     |      |                            | $49.94 \pm 0.08$  | --       | CCSD(T) |                                                         |
|     |      | $^4S_{3/2}, M_J = \pm 1/2$ | $51.60 \pm 0.01$  |          | MRCISD  | <a href="#">4C-DC-CI@dyall.acv4z@(core 15)[vir 265]</a> |
|     |      | $^4S_{3/2}, M_J = \pm 3/2$ | 41.76             |          |         |                                                         |
|     |      | $^4S_{3/2}$                | $46.68 \pm 0.01$  |          |         |                                                         |
| 115 | Mc   | $^4S, M_L = 0$             | $68.20 \pm 0.15$  | 3.52     | DHF     | <a href="#">2C-NR-CC@dyall.acv4z@(core 47)[vir 303]</a> |
|     |      |                            | $63.97 \pm 0.16$  | -2.90    | MP2     |                                                         |
|     |      |                            | $66.07 \pm 0.15$  | 0.29     | CCSD    |                                                         |
|     |      |                            | $65.88 \pm 0.15$  | --       | CCSD(T) |                                                         |
|     |      | $^4S, M_L = 0$             | $66.48 \pm 0.21$  | 4.58     | DHF     | <a href="#">2C-SR-CC@dyall.acv4z@(core 15)[vir 265]</a> |
|     |      |                            | $60.89 \pm 0.23$  | -4.21    | MP2     |                                                         |
|     |      |                            | $63.76 \pm 0.18$  | 0.30     | CCSD    |                                                         |
|     |      |                            | $63.57 \pm 0.18$  | --       | CCSD(T) |                                                         |
|     |      | $^4S, M_L = 0$             | $66.48 \pm 0.19$  | 5.14     | DHF     | <a href="#">2C-SR-CC@dyall.acv4z@(core 47)[vir 303]</a> |
|     |      |                            | $60.10 \pm 0.21$  | -4.94    | MP2     |                                                         |
|     |      |                            | $63.40 \pm 0.17$  | 0.27     | CCSD    |                                                         |

(continued)

Table S13. continued.

| Z | Atom | State                      | $\alpha_D$ (a.u.) | $\delta$ | Method  | Comments                                                |
|---|------|----------------------------|-------------------|----------|---------|---------------------------------------------------------|
|   |      |                            | $63.22 \pm 0.16$  | --       | CCSD(T) |                                                         |
|   |      | $^4S_{3/2}, M_J = \pm 1/2$ | $98.64 \pm 0.12$  |          | MRCISD  | <a href="#">4C-DC-CI@dyall.acv4z@(core 15)[vir 265]</a> |
|   |      | $^4S_{3/2}, M_J = \pm 3/2$ | 40.09             |          |         |                                                         |
|   |      | $^4S_{3/2}$                | $69.36 \pm 0.08$  |          |         |                                                         |

## S2.6 Group 16 elements

Table S14: The results of dipole polarizability for Group 16 elements.

| Z | Atom | State              | $\alpha_D$ (a.u.) | $\delta$ (%) | Method  | Comments                                               |
|---|------|--------------------|-------------------|--------------|---------|--------------------------------------------------------|
| 8 | O    | $^3P, M_L = 0$     | 4.91              | -14.89       | DHF     | <a href="#">2C-NR-CC@dyall.acv4z@(core 8)[vir 248]</a> |
|   |      | $^3P, M_L = \pm 1$ | 4.44              | -8.65        |         |                                                        |
|   |      | $^3P$              | 4.60              | -10.97       |         | $\Delta\alpha = -0.46$                                 |
|   |      | $^3P, M_L = 0$     | $5.30 \pm 0.02$   | -8.14        | MP2     |                                                        |
|   |      | $^3P, M_L = \pm 1$ | 4.79              | -1.44        |         |                                                        |
|   |      | $^3P$              | $4.96 \pm 0.01$   | -3.94        |         | $\Delta\alpha = -0.50$                                 |
|   |      | $^3P, M_L = 0$     | 5.65              | -1.98        | CCSD    |                                                        |
|   |      | $^3P, M_L = \pm 1$ | 4.80              | -1.26        |         |                                                        |
|   |      | $^3P$              | 5.08              | -1.53        |         | $\Delta\alpha = -0.85$                                 |
|   |      | $^3P, M_L = 0$     | 5.76              | --           | CCSD(T) |                                                        |
|   |      | $^3P, M_L = \pm 1$ | 4.86              | --           |         |                                                        |
|   |      | $^3P$              | 5.16              | --           |         | $\Delta\alpha = -0.90$                                 |
|   |      | $^3P, M_L = 0$     | 4.91              | -14.92       | DHF     | <a href="#">2C-SR-CC@dyall.acv4z@(core 8)[vir 186]</a> |
|   |      | $^3P, M_L = \pm 1$ | 4.44              | -8.66        |         |                                                        |
|   |      | $^3P$              | 4.60              | -10.99       |         | $\Delta\alpha = -0.47$                                 |
|   |      | $^3P, M_L = 0$     | 5.43              | -6.02        | MP2     |                                                        |
|   |      | $^3P, M_L = \pm 1$ | 4.77              | -1.87        |         |                                                        |
|   |      | $^3P$              | 4.99              | -3.42        |         | $\Delta\alpha = -0.66$                                 |
|   |      | $^3P, M_L = 0$     | 5.66              | -2.02        | CCSD    |                                                        |
|   |      | $^3P, M_L = \pm 1$ | 4.80              | -1.24        |         |                                                        |
|   |      | $^3P$              | 5.09              | -1.53        |         | $\Delta\alpha = -0.86$                                 |
|   |      | $^3P, M_L = 0$     | 5.77              | --           | CCSD(T) |                                                        |
|   |      | $^3P, M_L = \pm 1$ | 4.86              | --           |         |                                                        |
|   |      | $^3P$              | 5.17              | --           |         | $\Delta\alpha = -0.91$                                 |
|   |      | $^3P, M_L = 0$     | 4.91              | -14.94       | DHF     | <a href="#">2C-SR-CC@dyall.acv4z@(core 8)[vir 248]</a> |

(continued)

Table S14. continued.

| Z  | Atom | State                | $\alpha_D$ (a.u.) | $\delta$ | Method  | Comments                                                |
|----|------|----------------------|-------------------|----------|---------|---------------------------------------------------------|
|    |      | $^3P, M_L = \pm 1$   | 4.44              | -8.63    | MP2     | $\Delta\alpha = -0.47$                                  |
|    |      | $^3P$                | 4.60              | -10.98   |         |                                                         |
|    |      | $^3P, M_L = 0$       | $5.34 \pm 0.02$   | -7.58    |         |                                                         |
|    |      | $^3P, M_L = \pm 1$   | $4.69 \pm 0.02$   | -3.56    |         |                                                         |
|    |      | $^3P$                | $4.90 \pm 0.02$   | -5.06    | CCSD    | $\Delta\alpha = -0.65$                                  |
|    |      | $^3P, M_L = 0$       | 5.66              | -2.01    |         |                                                         |
|    |      | $^3P, M_L = \pm 1$   | 4.80              | -1.21    |         |                                                         |
|    |      | $^3P$                | 5.09              | -1.51    |         |                                                         |
|    |      | $^3P, M_L = 0$       | 5.78              | --       | CCSD(T) | $\Delta\alpha = -0.86$                                  |
|    |      | $^3P, M_L = \pm 1$   | 4.86              | --       |         |                                                         |
|    |      | $^3P$                | 5.16              | --       |         |                                                         |
|    |      |                      |                   |          |         | $\Delta\alpha = -0.92$                                  |
|    |      | $^3P_2, M_J = 0$     | 5.42              |          | MRCISD  | <a href="#">4C-DC-CI@dyall.acv4z@(core 8)[vir 116]</a>  |
|    |      | $^3P_2, M_J = \pm 1$ | 4.84              |          |         |                                                         |
|    |      | $^3P_2, M_J = \pm 2$ | 5.28              |          |         |                                                         |
|    |      | $^3P_2$              | 5.13              |          |         |                                                         |
|    |      | $^3P_2, M_J = 0$     | 5.24              |          | MRCISD  | 4C-DC-CI@dyall.acv4z@(core 8)[vir 186]                  |
|    |      | $^3P_2, M_J = \pm 1$ | 4.74              |          |         |                                                         |
|    |      | $^3P_2, M_J = \pm 2$ | 5.12              |          |         |                                                         |
|    |      | $^3P_2$              | 4.99              |          |         |                                                         |
| 16 | S    | $^3P, M_L = 0$       | $21.14 \pm 0.01$  | -3.51    | DHF     | <a href="#">2C-NR-CC@dyall.acv4z@(core 16)[vir 360]</a> |
|    |      | $^3P, M_L = \pm 1$   | 17.95             | -1.16    |         |                                                         |
|    |      | $^3P$                | $19.02 \pm 0.01$  | -2.05    |         |                                                         |
|    |      | $^3P, M_L = 0$       | $18.04 \pm 0.66$  | -17.65   | MP2     | $\Delta\alpha = -3.19$                                  |
|    |      | $^3P, M_L = \pm 1$   | $16.14 \pm 0.43$  | -11.15   |         |                                                         |
|    |      | $^3P$                | $16.77 \pm 0.52$  | -13.60   |         |                                                         |
|    |      | $^3P, M_L = 0$       | $21.76 \pm 0.01$  | -0.70    | CCSD    | $\Delta\alpha = -1.90$                                  |
|    |      | $^3P, M_L = \pm 1$   | 18.09             | -0.41    |         |                                                         |
|    |      | $^3P$                | $19.31 \pm 0.01$  | -0.52    |         |                                                         |
|    |      | $^3P, M_L = 0$       | $21.91 \pm 0.03$  | --       | CCSD(T) | $\Delta\alpha = -3.67$                                  |
|    |      | $^3P, M_L = \pm 1$   | $18.17 \pm 0.01$  | --       |         |                                                         |
|    |      | $^3P$                | $19.41 \pm 0.02$  | --       |         |                                                         |
|    |      |                      |                   |          |         | $\Delta\alpha = -3.75$                                  |
|    |      | $^3P, M_L = 0$       | $21.21 \pm 0.01$  | -4.34    | DHF     | <a href="#">2C-SR-CC@dyall.acv4z@(core 16)[vir 184]</a> |
|    |      | $^3P, M_L = \pm 1$   | 17.95             | -1.91    |         |                                                         |
|    |      | $^3P$                | $19.04 \pm 0.01$  | -2.83    |         |                                                         |
|    |      | $^3P, M_L = 0$       | $18.26 \pm 0.52$  | -17.63   | MP2     | $\Delta\alpha = -3.26$                                  |
|    |      | $^3P, M_L = \pm 1$   | $16.33 \pm 0.33$  | -10.75   |         |                                                         |
|    |      | $^3P$                | $16.98 \pm 0.4$   | -13.34   |         |                                                         |
|    |      | $^3P, M_L = 0$       | $22.02 \pm 0.01$  | -0.66    | CCSD    | $\Delta\alpha = -1.93$                                  |
|    |      |                      |                   |          |         |                                                         |
|    |      |                      |                   |          |         |                                                         |
|    |      |                      |                   |          |         |                                                         |

(continued)



Table S14. continued.

| Z | Atom | State                | $\alpha_D$ (a.u.) | $\delta$ | Method  | Comments                                                |
|---|------|----------------------|-------------------|----------|---------|---------------------------------------------------------|
|   |      | $^3P, M_L = \pm 1$   | 18.23             | -0.37    | CCSD(T) | $\Delta\alpha = -3.79$                                  |
|   |      | $^3P$                | $19.49 \pm 0.01$  | -0.48    |         |                                                         |
|   |      | $^3P, M_L = 0$       | $22.17 \pm 0.03$  | --       |         |                                                         |
|   |      | $^3P, M_L = \pm 1$   | $18.30 \pm 0.01$  | --       |         |                                                         |
|   |      | $^3P$                | $19.59 \pm 0.02$  | --       |         | $\Delta\alpha = -3.87$                                  |
|   |      | $^3P, M_L = 0$       | $21.21 \pm 0.01$  | -3.58    | DHF     | <a href="#">2C-SR-CC@dyall.acv4z@(core 16)[vir 360]</a> |
|   |      | $^3P, M_L = \pm 1$   | 17.95             | -1.20    | MP2     | $\Delta\alpha = -3.26$                                  |
|   |      | $^3P$                | $19.04 \pm 0.01$  | -2.10    |         |                                                         |
|   |      | $^3P, M_L = 0$       | $18.34 \pm 0.45$  | -16.62   |         |                                                         |
|   |      | $^3P, M_L = \pm 1$   | $16.22 \pm 0.32$  | -10.70   |         |                                                         |
|   |      | $^3P$                | $16.93 \pm 0.37$  | -12.93   |         | $\Delta\alpha = -2.12$                                  |
|   |      | $^3P, M_L = 0$       | $21.83 \pm 0.01$  | -0.74    | CCSD    | $\Delta\alpha = -3.74$                                  |
|   |      | $^3P, M_L = \pm 1$   | 18.09             | -0.42    |         |                                                         |
|   |      | $^3P$                | $19.34 \pm 0.01$  | -0.54    |         |                                                         |
|   |      | $^3P, M_L = 0$       | $22.00 \pm 0.02$  | --       |         |                                                         |
|   |      | $^3P, M_L = \pm 1$   | $18.17 \pm 0.01$  | --       |         |                                                         |
|   |      | $^3P$                | $19.44 \pm 0.02$  | --       | MRCISD  | $\Delta\alpha = -3.83$                                  |
|   |      | $^3P_2, M_J = 0$     | 20.24             |          |         | <a href="#">4C-DC-CI@dyall.acv4z@(core 16)[vir 184]</a> |
|   |      | $^3P_2, M_J = \pm 1$ | 17.95             |          |         |                                                         |
|   |      | $^3P_2, M_J = \pm 2$ | 19.67             |          |         |                                                         |
|   |      | $^3P_2$              | 19.10             |          |         |                                                         |
|   |      | $^3P_2, M_J = 0$     | 19.92             |          | MRCISD  | 4C-DC-CI@dyall.acv4z@(core 16)[vir 252]                 |
|   |      | $^3P_2, M_J = \pm 1$ | 17.74             |          |         |                                                         |
|   |      | $^3P_2, M_J = \pm 2$ | 19.38             |          |         |                                                         |
|   |      | $^3P_2$              | 18.83             |          |         |                                                         |
|   |      | $^3P, M_L = 0$       | 27.88             | -2.84    | DHF     | <a href="#">2C-NR-CC@dyall.acv4z@(core 34)[vir 478]</a> |
|   |      | $^3P, M_L = \pm 1$   | 23.66             | -0.42    | MP2     | $\Delta\alpha = -4.22$                                  |
|   |      | $^3P$                | 25.07             | -1.33    |         |                                                         |
|   |      | $^3P, M_L = 0$       | $23.61 \pm 1.51$  | -17.72   |         |                                                         |
|   |      | $^3P, M_L = \pm 1$   | $22.30 \pm 0.11$  | -6.14    |         |                                                         |
|   |      | $^3P$                | $22.74 \pm 0.87$  | -10.50   |         | $\Delta\alpha = -1.30$                                  |
|   |      | $^3P, M_L = 0$       | 28.35             | -1.19    | CCSD    | $\Delta\alpha = -4.72$                                  |
|   |      | $^3P, M_L = \pm 1$   | 23.64             | -0.53    |         |                                                         |
|   |      | $^3P$                | 25.21             | -0.78    |         |                                                         |
|   |      | $^3P, M_L = 0$       | $28.69 \pm 0.07$  | --       |         |                                                         |
|   |      | $^3P, M_L = \pm 1$   | $23.76 \pm 0.01$  | --       |         |                                                         |
|   |      | $^3P$                | $25.41 \pm 0.04$  | --       | CCSD(T) | $\Delta\alpha = -4.93$                                  |
|   |      | $^3P, M_L = 0$       | 28.03             | -2.88    | DHF     | <a href="#">2C-SR-CC@dyall.acv4z@(core 16)[vir 184]</a> |

(continued)

Table S14. continued.

| Z  | Atom | State                | $\alpha_D$ (a.u.) | $\delta$ | Method  | Comments                                                |
|----|------|----------------------|-------------------|----------|---------|---------------------------------------------------------|
|    |      | $^3P, M_L = \pm 1$   | 23.47             | -0.61    | MP2     | $\Delta\alpha = -4.56$                                  |
|    |      | $^3P$                | 24.99             | -1.47    |         |                                                         |
|    |      | $^3P, M_L = 0$       | $25.28 \pm 1.95$  | -12.42   |         |                                                         |
|    |      | $^3P, M_L = \pm 1$   | $23.28 \pm 0.04$  | -1.43    | CCSD    | $\Delta\alpha = -2.00$                                  |
|    |      | $^3P$                | $23.95 \pm 1.12$  | -5.60    |         |                                                         |
|    |      | $^3P, M_L = 0$       | 28.51             | -1.22    |         |                                                         |
|    |      | $^3P, M_L = \pm 1$   | 23.46             | -0.67    | CCSD(T) | $\Delta\alpha = -5.05$                                  |
|    |      | $^3P$                | 25.14             | -0.88    |         |                                                         |
|    |      | $^3P, M_L = 0$       | $28.86 \pm 0.03$  | --       |         |                                                         |
|    |      | $^3P, M_L = \pm 1$   | $23.62 \pm 0.01$  | --       |         | $\Delta\alpha = -5.25$                                  |
|    |      | $^3P$                | $25.37 \pm 0.02$  | --       |         |                                                         |
|    |      | $^3P, M_L = 0$       | 28.03             | -3.15    | DHF     | <a href="#">2C-SR-CC@dyall.acv4z@(core 34)[vir 478]</a> |
|    |      | $^3P, M_L = \pm 1$   | 23.47             | -0.67    | MP2     | $\Delta\alpha = -4.56$                                  |
|    |      | $^3P$                | 24.99             | -1.61    |         |                                                         |
|    |      | $^3P, M_L = 0$       | $26.17 \pm 1.22$  | -9.57    |         |                                                         |
|    |      | $^3P, M_L = \pm 1$   | $23.32 \pm 0.05$  | -1.31    | CCSD    | $\Delta\alpha = -2.85$                                  |
|    |      | $^3P$                | $24.27 \pm 0.71$  | -4.45    |         |                                                         |
|    |      | $^3P, M_L = 0$       | 28.56             | -1.33    |         |                                                         |
|    |      | $^3P, M_L = \pm 1$   | 23.48             | -0.65    | CCSD(T) | $\Delta\alpha = -5.08$                                  |
|    |      | $^3P$                | 25.17             | -0.91    |         |                                                         |
|    |      | $^3P, M_L = 0$       | $28.94 \pm 0.05$  | --       |         |                                                         |
|    |      | $^3P, M_L = \pm 1$   | $23.63 \pm 0.01$  | --       |         | $\Delta\alpha = -5.31$                                  |
|    |      | $^3P$                | $25.40 \pm 0.03$  | --       |         |                                                         |
|    |      | $^3P_2, M_J = 0$     | 25.90             |          | MRCISD  | <a href="#">4C-DC-CI@dyall.acv4z@(core 16)[vir 184]</a> |
|    |      | $^3P_2, M_J = \pm 1$ | 23.09             |          |         |                                                         |
|    |      | $^3P_2, M_J = \pm 2$ | 25.20             |          |         |                                                         |
|    |      | $^3P_2$              | 24.50             |          |         |                                                         |
| 52 | Te   | $^3P, M_L = 0$       | 41.94             | -0.56    | DHF     | <a href="#">2C-NR-CC@dyall.acv4z@(core 52)[vir 550]</a> |
|    |      | $^3P, M_L = \pm 1$   | 36.99             | 1.46     | MP2     | $\Delta\alpha = -4.95$                                  |
|    |      | $^3P$                | 38.64             | 0.72     |         |                                                         |
|    |      | $^3P, M_L = 0$       | $39.22 \pm 1.21$  | -7.02    |         |                                                         |
|    |      | $^3P, M_L = \pm 1$   | $35.42 \pm 0.73$  | -2.86    | CCSD    | $\Delta\alpha = -3.80$                                  |
|    |      | $^3P$                | $36.68 \pm 0.92$  | -4.38    |         |                                                         |
|    |      | $^3P, M_L = 0$       | $41.75 \pm 0.01$  | -1.02    |         |                                                         |
|    |      | $^3P, M_L = \pm 1$   | 36.30             | -0.44    | CCSD(T) | $\Delta\alpha = -5.45$                                  |
|    |      | $^3P$                | 38.11             | -0.66    |         |                                                         |
|    |      | $^3P, M_L = 0$       | $42.18 \pm 0.07$  | --       |         |                                                         |
|    |      | $^3P, M_L = \pm 1$   | 36.46             | --       |         |                                                         |

(continued)

Table S14. continued.

| Z  | Atom | State                | $\alpha_D$ (a.u.) | $\delta$ | Method  | Comments                                                |
|----|------|----------------------|-------------------|----------|---------|---------------------------------------------------------|
|    |      | $^3P$                | $38.37 \pm 0.04$  | --       |         | $\Delta\alpha = -5.72$                                  |
|    |      | $^3P, M_L = 0$       | $42.07 \pm 0.01$  | -1.26    | DHF     | <a href="#">2C-SR-CC@dyall.acv4z@(core 16)[vir 216]</a> |
|    |      | $^3P, M_L = \pm 1$   | 35.99             | 0.66     |         |                                                         |
|    |      | $^3P$                | 38.02             | -0.06    |         |                                                         |
|    |      | $^3P, M_L = 0$       | $38.23 \pm 2.45$  | -10.28   | MP2     | $\Delta\alpha = -6.08$                                  |
|    |      | $^3P, M_L = \pm 1$   | $34.55 \pm 0.96$  | -3.38    |         |                                                         |
|    |      | $^3P$                | $35.77 \pm 1.62$  | -5.95    |         | $\Delta\alpha = -3.68$                                  |
|    |      | $^3P, M_L = 0$       | $42.20 \pm 0.01$  | -0.97    | CCSD    |                                                         |
|    |      | $^3P, M_L = \pm 1$   | 35.58             | -0.49    |         |                                                         |
|    |      | $^3P$                | 37.78             | -0.67    |         | $\Delta\alpha = -6.62$                                  |
|    |      | $^3P, M_L = 0$       | $42.61 \pm 0.02$  | --       | CCSD(T) |                                                         |
|    |      | $^3P, M_L = \pm 1$   | $35.75 \pm 0.02$  | --       |         |                                                         |
|    |      | $^3P$                | $38.04 \pm 0.02$  | --       |         | $\Delta\alpha = -6.86$                                  |
|    |      | $^3P, M_L = 0$       | $42.07 \pm 0.01$  | -0.98    | DHF     | <a href="#">2C-SR-CC@dyall.acv4z@(core 52)[vir 550]</a> |
|    |      | $^3P, M_L = \pm 1$   | 35.99             | 0.89     |         |                                                         |
|    |      | $^3P$                | 38.02             | 0.19     |         |                                                         |
|    |      | $^3P, M_L = 0$       | $37.67 \pm 2.64$  | -11.34   | MP2     | $\Delta\alpha = -6.08$                                  |
|    |      | $^3P, M_L = \pm 1$   | $35.95 \pm 0.2$   | 0.79     |         |                                                         |
|    |      | $^3P$                | $36.53 \pm 1.54$  | -3.74    |         | $\Delta\alpha = -1.72$                                  |
|    |      | $^3P, M_L = 0$       | $42.08 \pm 0.01$  | -0.95    | CCSD    |                                                         |
|    |      | $^3P, M_L = \pm 1$   | 35.46             | -0.59    |         |                                                         |
|    |      | $^3P$                | 37.67             | -0.72    |         | $\Delta\alpha = -6.62$                                  |
|    |      | $^3P, M_L = 0$       | $42.49 \pm 0.02$  | --       | CCSD(T) |                                                         |
|    |      | $^3P, M_L = \pm 1$   | $35.67 \pm 0.01$  | --       |         |                                                         |
|    |      | $^3P$                | $37.94 \pm 0.01$  | --       |         | $\Delta\alpha = -6.82$                                  |
|    |      | $^3P_2, M_J = 0$     | 38.05             |          | MRCISD  | <a href="#">4C-DC-CI@dyall.acv4z@(core 16)[vir 216]</a> |
|    |      | $^3P_2, M_J = \pm 1$ | 35.19             |          |         |                                                         |
|    |      | $^3P_2, M_J = \pm 2$ | 37.33             |          |         |                                                         |
|    |      | $^3P_2$              | 36.62             |          |         |                                                         |
| 84 | Po   | $^3P, M_L = 0$       | $50.29 \pm 0.01$  | 0.57     | DHF     | <a href="#">2C-NR-CC@dyall.acv4z@(core 48)[vir 296]</a> |
|    |      | $^3P, M_L = \pm 1$   | 44.81             | 2.21     |         |                                                         |
|    |      | $^3P$                | 46.64             | 1.61     |         |                                                         |
|    |      | $^3P, M_L = 0$       | $46.46 \pm 1.74$  | -7.09    | MP2     | $\Delta\alpha = -5.48$                                  |
|    |      | $^3P, M_L = \pm 1$   | $43.12 \pm 0.43$  | -1.64    |         |                                                         |
|    |      | $^3P$                | $44.23 \pm 1.06$  | -3.62    |         | $\Delta\alpha = -3.34$                                  |
|    |      | $^3P, M_L = 0$       | $49.63 \pm 0.01$  | -0.76    | CCSD    |                                                         |
|    |      | $^3P, M_L = \pm 1$   | 43.68             | -0.37    |         |                                                         |
|    |      | $^3P$                | 45.66             | -0.51    |         | $\Delta\alpha = -5.95$                                  |

(continued)

Table S14. continued.

| Z   | Atom | State                | $\alpha_D$ (a.u.) | $\delta$ | Method  | Comments                                                |
|-----|------|----------------------|-------------------|----------|---------|---------------------------------------------------------|
|     |      | $^3P, M_L = 0$       | $50.01 \pm 0.01$  | --       | CCSD(T) |                                                         |
|     |      | $^3P, M_L = \pm 1$   | $43.84 \pm 0.01$  | --       |         |                                                         |
|     |      | $^3P$                | $45.89 \pm 0.01$  | --       |         | $\Delta\alpha = -6.17$                                  |
|     |      | $^3P, M_L = 0$       | $51.44 \pm 0.08$  | -1.70    | DHF     | <a href="#">2C-SR-CC@dyall.acv4z@(core 16)[vir 262]</a> |
|     |      | $^3P, M_L = \pm 1$   | $41.88 \pm 0.03$  | 0.31     |         |                                                         |
|     |      | $^3P$                | $45.06 \pm 0.05$  | -0.47    |         | $\Delta\alpha = -9.56$                                  |
|     |      | $^3P, M_L = 0$       | $50.26 \pm 0.13$  | -3.95    | MP2     |                                                         |
|     |      | $^3P, M_L = \pm 1$   | $41.88 \pm 0.04$  | 0.33     |         |                                                         |
|     |      | $^3P$                | $44.68 \pm 0.08$  | -1.32    |         | $\Delta\alpha = -8.38$                                  |
|     |      | $^3P, M_L = 0$       | $51.75 \pm 0.09$  | -1.10    | CCSD    |                                                         |
|     |      | $^3P, M_L = \pm 1$   | $41.46 \pm 0.03$  | -0.69    |         |                                                         |
|     |      | $^3P$                | $44.89 \pm 0.06$  | -0.85    |         | $\Delta\alpha = -10.29$                                 |
|     |      | $^3P, M_L = 0$       | $52.33 \pm 0.09$  | --       | CCSD(T) |                                                         |
|     |      | $^3P, M_L = \pm 1$   | $41.75 \pm 0.03$  | --       |         |                                                         |
|     |      | $^3P$                | $45.27 \pm 0.06$  | --       |         | $\Delta\alpha = -10.58$                                 |
|     |      | $^3P, M_L = 0$       | $51.44 \pm 0.07$  | -1.37    | DHF     | <a href="#">2C-SR-CC@dyall.acv4z@(core 48)[vir 296]</a> |
|     |      | $^3P, M_L = \pm 1$   | $41.88 \pm 0.03$  | 0.69     |         |                                                         |
|     |      | $^3P$                | $45.06 \pm 0.05$  | -0.11    |         | $\Delta\alpha = -9.56$                                  |
|     |      | $^3P, M_L = 0$       | $49.70 \pm 0.12$  | -4.70    | MP2     |                                                         |
|     |      | $^3P, M_L = \pm 1$   | $41.72 \pm 0.04$  | 0.31     |         |                                                         |
|     |      | $^3P$                | $44.38 \pm 0.08$  | -1.62    |         | $\Delta\alpha = -7.98$                                  |
|     |      | $^3P, M_L = 0$       | $51.55 \pm 0.08$  | -1.16    | CCSD    |                                                         |
|     |      | $^3P, M_L = \pm 1$   | $41.31 \pm 0.03$  | -0.67    |         |                                                         |
|     |      | $^3P$                | $44.72 \pm 0.05$  | -0.86    |         | $\Delta\alpha = -10.24$                                 |
|     |      | $^3P, M_L = 0$       | $52.15 \pm 0.09$  | --       | CCSD(T) |                                                         |
|     |      | $^3P, M_L = \pm 1$   | $41.59 \pm 0.03$  | --       |         |                                                         |
|     |      | $^3P$                | $45.11 \pm 0.06$  | --       |         | $\Delta\alpha = -10.56$                                 |
|     |      | $^3P_2, M_J = 0$     | $43.92 \pm 0.01$  |          | MRCISD  | <a href="#">4C-DC-CI@dyall.acv4z@(core 16)[vir 262]</a> |
|     |      | $^3P_2, M_J = \pm 1$ | $42.68 \pm 0.01$  |          |         |                                                         |
|     |      | $^3P_2, M_J = \pm 2$ | $43.60 \pm 0.01$  |          |         |                                                         |
|     |      | $^3P_2$              | $43.29 \pm 0.01$  |          |         |                                                         |
| 116 | Lv   | $^3P, M_L = 0$       | $66.11 \pm 0.14$  | 1.90     | DHF     | <a href="#">2C-NR-CC@dyall.acv4z@(core 48)[vir 294]</a> |
|     |      | $^3P, M_L = \pm 1$   | $59.43 \pm 0.05$  | 3.23     |         |                                                         |
|     |      | $^3P$                | $61.66 \pm 0.09$  | 2.75     |         | $\Delta\alpha = -6.68$                                  |
|     |      | $^3P, M_L = 0$       | $63.15 \pm 0.14$  | -2.67    | MP2     |                                                         |
|     |      | $^3P, M_L = \pm 1$   | $57.18 \pm 0.08$  | -0.68    |         |                                                         |
|     |      | $^3P$                | $59.17 \pm 0.1$   | -1.40    |         | $\Delta\alpha = -5.98$                                  |
|     |      | $^3P, M_L = 0$       | $64.47 \pm 0.14$  | -0.63    | CCSD    |                                                         |

(continued)

Table S14. continued.

| Z | Atom | State                | $\alpha_D$ (a.u.) | $\delta$ | Method  | Comments                                                |
|---|------|----------------------|-------------------|----------|---------|---------------------------------------------------------|
|   |      | $^3P, M_L = \pm 1$   | $57.43 \pm 0.06$  | -0.24    |         |                                                         |
|   |      | $^3P$                | $59.78 \pm 0.09$  | -0.38    |         | $\Delta\alpha = -7.04$                                  |
|   |      | $^3P, M_L = 0$       | $64.88 \pm 0.15$  | --       | CCSD(T) |                                                         |
|   |      | $^3P, M_L = \pm 1$   | $57.57 \pm 0.06$  | --       |         |                                                         |
|   |      | $^3P$                | $60.01 \pm 0.1$   | --       |         | $\Delta\alpha = -7.31$                                  |
|   |      | $^3P, M_L = 0$       | $69.37 \pm 0.15$  | -0.96    | DHF     | <a href="#">2C-SR-CC@dyall.acv4z@(core 16)[vir 262]</a> |
|   |      | $^3P, M_L = \pm 1$   | $53.84 \pm 0.07$  | 1.71     |         |                                                         |
|   |      | $^3P$                | $59.02 \pm 0.1$   | 0.65     |         | $\Delta\alpha = -15.53$                                 |
|   |      | $^3P, M_L = 0$       | $66.67 \pm 0.18$  | -4.82    | MP2     |                                                         |
|   |      | $^3P, M_L = \pm 1$   | $52.52 \pm 0.09$  | -0.80    |         |                                                         |
|   |      | $^3P$                | $57.23 \pm 0.13$  | -2.40    |         | $\Delta\alpha = -14.15$                                 |
|   |      | $^3P, M_L = 0$       | $69.41 \pm 0.15$  | -0.91    | CCSD    |                                                         |
|   |      | $^3P, M_L = \pm 1$   | $52.68 \pm 0.06$  | -0.49    |         |                                                         |
|   |      | $^3P$                | $58.26 \pm 0.1$   | -0.66    |         | $\Delta\alpha = -16.73$                                 |
|   |      | $^3P, M_L = 0$       | $70.05 \pm 0.16$  | --       | CCSD(T) |                                                         |
|   |      | $^3P, M_L = \pm 1$   | $52.94 \pm 0.06$  | --       |         |                                                         |
|   |      | $^3P$                | $58.64 \pm 0.11$  | --       |         | $\Delta\alpha = -17.11$                                 |
|   |      | $^3P, M_L = 0$       | $69.37 \pm 0.14$  | -0.54    | DHF     | <a href="#">2C-SR-CC@dyall.acv4z@(core 48)[vir 294]</a> |
|   |      | $^3P, M_L = \pm 1$   | $53.84 \pm 0.06$  | 2.11     |         |                                                         |
|   |      | $^3P$                | $59.02 \pm 0.09$  | 1.06     |         | $\Delta\alpha = -15.53$                                 |
|   |      | $^3P, M_L = 0$       | $65.56 \pm 0.15$  | -6.01    | MP2     |                                                         |
|   |      | $^3P, M_L = \pm 1$   | $52.41 \pm 0.09$  | -0.60    |         |                                                         |
|   |      | $^3P$                | $56.79 \pm 0.11$  | -2.76    |         | $\Delta\alpha = -13.15$                                 |
|   |      | $^3P, M_L = 0$       | $69.05 \pm 0.14$  | -1.01    | CCSD    |                                                         |
|   |      | $^3P, M_L = \pm 1$   | $52.47 \pm 0.06$  | -0.49    |         |                                                         |
|   |      | $^3P$                | $57.99 \pm 0.09$  | -0.70    |         | $\Delta\alpha = -16.58$                                 |
|   |      | $^3P, M_L = 0$       | $69.75 \pm 0.15$  | --       | CCSD(T) |                                                         |
|   |      | $^3P, M_L = \pm 1$   | $52.73 \pm 0.06$  | --       |         |                                                         |
|   |      | $^3P$                | $58.40 \pm 0.1$   | --       |         | $\Delta\alpha = -17.02$                                 |
|   |      | $^3P_2, M_J = 0$     | $68.87 \pm 0.04$  |          | MRCISD  | <a href="#">4C-DC-CI@dyall.acv4z@(core 16)[vir 262]</a> |
|   |      | $^3P_2, M_J = \pm 1$ | $75.28 \pm 0.03$  |          |         |                                                         |
|   |      | $^3P_2, M_J = \pm 2$ | $70.38 \pm 0.03$  |          |         |                                                         |
|   |      | $^3P_2$              | $72.04 \pm 0.03$  |          |         |                                                         |

## S2.7 Group 17 elements

Table S15: The results of dipole polarizability for Group 17 elements.

| <b>Z</b> | <b>Atom</b> | <b>State</b>               | $\alpha_D$ (a.u.) | $\delta$ (%) | <b>Method</b> | <b>Comments</b>                                        |
|----------|-------------|----------------------------|-------------------|--------------|---------------|--------------------------------------------------------|
| 9        | F           | $^2P, M_L = 0$             | 3.02              | -9.48        | DHF           | <a href="#">2C-NR-CC@dyall.acv4z@(core 9)[vir 247]</a> |
|          |             | $^2P, M_L = \pm 1$         | 3.31              | -11.47       |               |                                                        |
|          |             | $^2P$                      | 3.21              | -10.85       |               | $\Delta\alpha = 0.29$                                  |
|          |             | $^2P, M_L = 0$             | 3.34              | 0.20         | MP2           |                                                        |
|          |             | $^2P, M_L = \pm 1$         | $3.64 \pm 0.01$   | -2.71        |               |                                                        |
|          |             | $^2P$                      | $3.54 \pm 0.01$   | -1.82        |               | $\Delta\alpha = 0.30$                                  |
|          |             | $^2P, M_L = 0$             | 3.29              | -1.33        | CCSD          |                                                        |
|          |             | $^2P, M_L = \pm 1$         | 3.67              | -1.78        |               |                                                        |
|          |             | $^2P$                      | 3.55              | -1.64        |               | $\Delta\alpha = 0.38$                                  |
|          |             | $^2P, M_L = 0$             | 3.34              | --           | CCSD(T)       |                                                        |
|          |             | $^2P, M_L = \pm 1$         | 3.74              | --           |               |                                                        |
|          |             | $^2P$                      | 3.60              | --           |               | $\Delta\alpha = 0.40$                                  |
|          |             | $^2P, M_L = 0$             | 3.02              | -9.54        | DHF           | <a href="#">2C-SR-CC@dyall.acv4z@(core 9)[vir 183]</a> |
|          |             | $^2P, M_L = \pm 1$         | 3.32              | -11.45       |               |                                                        |
|          |             | $^2P$                      | 3.22              | -10.86       |               | $\Delta\alpha = 0.30$                                  |
|          |             | $^2P, M_L = 0$             | $3.45 \pm 0.02$   | 3.28         | MP2           |                                                        |
|          |             | $^2P, M_L = \pm 1$         | $3.59 \pm 0.02$   | -4.06        |               |                                                        |
|          |             | $^2P$                      | $3.54 \pm 0.02$   | -1.79        |               | $\Delta\alpha = 0.15$                                  |
|          |             | $^2P, M_L = 0$             | 3.29              | -1.38        | CCSD          |                                                        |
|          |             | $^2P, M_L = \pm 1$         | 3.68              | -1.77        |               |                                                        |
|          |             | $^2P$                      | 3.55              | -1.65        |               | $\Delta\alpha = 0.39$                                  |
|          |             | $^2P, M_L = 0$             | 3.34              | --           | CCSD(T)       |                                                        |
|          |             | $^2P, M_L = \pm 1$         | 3.74              | --           |               |                                                        |
|          |             | $^2P$                      | 3.61              | --           |               | $\Delta\alpha = 0.41$                                  |
|          |             | $^2P, M_L = 0$             | 3.02              | -9.53        | DHF           | <a href="#">2C-SR-CC@dyall.acv4z@(core 9)[vir 247]</a> |
|          |             | $^2P, M_L = \pm 1$         | 3.32              | -11.48       |               |                                                        |
|          |             | $^2P$                      | 3.22              | -10.88       |               | $\Delta\alpha = 0.30$                                  |
|          |             | $^2P, M_L = 0$             | $3.40 \pm 0.01$   | 1.93         | MP2           |                                                        |
|          |             | $^2P, M_L = \pm 1$         | $3.61 \pm 0.02$   | -3.71        |               |                                                        |
|          |             | $^2P$                      | $3.54 \pm 0.01$   | -1.97        |               | $\Delta\alpha = 0.21$                                  |
|          |             | $^2P, M_L = 0$             | 3.29              | -1.38        | CCSD          |                                                        |
|          |             | $^2P, M_L = \pm 1$         | 3.68              | -1.77        |               |                                                        |
|          |             | $^2P$                      | 3.55              | -1.65        |               | $\Delta\alpha = 0.39$                                  |
|          |             | $^2P, M_L = 0$             | 3.34              | --           | CCSD(T)       |                                                        |
|          |             | $^2P, M_L = \pm 1$         | 3.74              | --           |               |                                                        |
|          |             | $^2P$                      | 3.61              | --           |               | $\Delta\alpha = 0.41$                                  |
|          |             | $^2P_{3/2}, M_J = \pm 1/2$ | 3.43              |              | MRCISD        | <a href="#">4C-DC-CI@dyall.acv4z@(core 9)[vir 115]</a> |

(continued)

Table S15. continued.

| Z  | Atom | State                      | $\alpha_D$ (a.u.) | $\delta$ | Method  | Comments                                        |
|----|------|----------------------------|-------------------|----------|---------|-------------------------------------------------|
| 17 | Cl   | $^2P_{3/2}, M_J = \pm 3/2$ | 3.70              |          |         |                                                 |
|    |      | $^2P_{3/2}$                | 3.57              |          |         |                                                 |
|    |      | $^2P_{1/2}$                | 3.57              |          |         | $\bar{\alpha}_{J=3/2} - \alpha_{J=1/2} = -0.00$ |
|    |      | $^2P_{3/2}, M_J = \pm 1/2$ | 3.37              |          | MRCISD  | 4C-DC-CI@dyall.acv4z@(core 9)[vir 183]          |
|    |      | $^2P_{3/2}, M_J = \pm 3/2$ | 3.61              |          |         |                                                 |
|    |      | $^2P_{3/2}$                | 3.49              |          |         |                                                 |
|    |      | $^2P_{1/2}$                | 3.49              |          |         | $\bar{\alpha}_{J=3/2} - \alpha_{J=1/2} = -0.00$ |
|    |      | $^2P, M_L = 0$             | 13.11             | -2.31    | DHF     | <b>2C-NR-CC@dyall.acv4z@(core 17)[vir 359]</b>  |
|    |      | $^2P, M_L = \pm 1$         | 14.74             | -2.81    |         |                                                 |
|    |      | $^2P$                      | 14.20             | -2.66    |         | $\Delta\alpha = 1.63$                           |
|    |      | $^2P, M_L = 0$             | $13.54 \pm 0.01$  | 0.93     | MP2     |                                                 |
|    |      | $^2P, M_L = \pm 1$         | $15.04 \pm 0.01$  | -0.86    |         |                                                 |
| 17 | Cl   | $^2P$                      | $14.54 \pm 0.01$  | -0.31    |         | $\Delta\alpha = 1.49$                           |
|    |      | $^2P, M_L = 0$             | 13.31             | -0.82    | CCSD    |                                                 |
|    |      | $^2P, M_L = \pm 1$         | 15.02             | -0.97    |         |                                                 |
|    |      | $^2P$                      | 14.45             | -0.92    |         | $\Delta\alpha = 1.71$                           |
|    |      | $^2P, M_L = 0$             | 13.42             | --       | CCSD(T) |                                                 |
|    |      | $^2P, M_L = \pm 1$         | 15.17             | --       |         |                                                 |
|    |      | $^2P$                      | 14.58             | --       |         | $\Delta\alpha = 1.75$                           |
|    |      | $^2P, M_L = 0$             | 13.10             | -3.00    | DHF     | <b>2C-SR-CC@dyall.acv4z@(core 17)[vir 169]</b>  |
|    |      | $^2P, M_L = \pm 1$         | 14.77             | -3.59    |         |                                                 |
|    |      | $^2P$                      | 14.21             | -3.41    |         | $\Delta\alpha = 1.67$                           |
|    |      | $^2P, M_L = 0$             | $13.83 \pm 0.05$  | 2.39     | MP2     |                                                 |
|    |      | $^2P, M_L = \pm 1$         | $15.28 \pm 0.01$  | -0.29    |         |                                                 |
|    |      | $^2P$                      | $14.79 \pm 0.03$  | 0.53     |         | $\Delta\alpha = 1.45$                           |
|    |      | $^2P, M_L = 0$             | 13.40             | -0.80    | CCSD    |                                                 |
|    |      | $^2P, M_L = \pm 1$         | 15.17             | -0.96    |         |                                                 |
|    |      | $^2P$                      | 14.58             | -0.91    |         | $\Delta\alpha = 1.78$                           |
|    |      | $^2P, M_L = 0$             | 13.51             | --       | CCSD(T) |                                                 |
|    |      | $^2P, M_L = \pm 1$         | 15.32             | --       |         |                                                 |
|    |      | $^2P$                      | 14.72             | --       |         | $\Delta\alpha = 1.82$                           |
|    |      | $^2P, M_L = 0$             | 13.10             | -2.40    | DHF     | <b>2C-SR-CC@dyall.acv4z@(core 17)[vir 359]</b>  |
|    |      | $^2P, M_L = \pm 1$         | 14.77             | -2.81    |         |                                                 |
|    |      | $^2P$                      | 14.21             | -2.68    |         | $\Delta\alpha = 1.67$                           |
|    |      | $^2P, M_L = 0$             | $13.99 \pm 0.11$  | 4.22     | MP2     |                                                 |
|    |      | $^2P, M_L = \pm 1$         | $14.76 \pm 0.08$  | -2.91    |         |                                                 |
|    |      | $^2P$                      | $14.50 \pm 0.09$  | -0.73    |         | $\Delta\alpha = 0.77$                           |
|    |      | $^2P, M_L = 0$             | 13.30             | -0.90    | CCSD    |                                                 |

(continued)

Table S15. continued.

| Z  | Atom | State                      | $\alpha_D$ (a.u.)                               | $\delta$ | Method                                          | Comments                                                |                                                         |
|----|------|----------------------------|-------------------------------------------------|----------|-------------------------------------------------|---------------------------------------------------------|---------------------------------------------------------|
|    |      | $^2P, M_L = \pm 1$         | 15.06                                           | -0.94    | CCSD(T)                                         | $\Delta\alpha = 1.75$                                   |                                                         |
|    |      | $^2P$                      | 14.47                                           | -0.93    |                                                 |                                                         |                                                         |
|    |      | $^2P, M_L = 0$             | 13.42                                           | --       |                                                 |                                                         |                                                         |
|    |      | $^2P, M_L = \pm 1$         | 15.20                                           | --       |                                                 |                                                         |                                                         |
|    |      | $^2P$                      | 14.61                                           | --       |                                                 |                                                         |                                                         |
|    |      |                            |                                                 |          |                                                 | $\Delta\alpha = 1.78$                                   |                                                         |
|    |      | $^2P_{3/2}, M_J = \pm 1/2$ | 13.78                                           |          | MRCISD                                          | <a href="#">4C-DC-CI@dyall.acv4z@(core 17)[vir 169]</a> |                                                         |
|    |      | $^2P_{3/2}, M_J = \pm 3/2$ | 14.94                                           |          |                                                 |                                                         |                                                         |
|    |      | $^2P_{3/2}$                | 14.36                                           |          |                                                 |                                                         |                                                         |
|    |      | $^2P_{1/2}$                | 14.40                                           |          |                                                 |                                                         |                                                         |
|    |      |                            |                                                 |          | $\bar{\alpha}_{J=3/2} - \alpha_{J=1/2} = -0.03$ |                                                         |                                                         |
|    |      | $^2P_{3/2}, M_J = \pm 1/2$ | 13.65                                           |          | MRCISD                                          | <a href="#">4C-DC-CI@dyall.acv4z@(core 17)[vir 243]</a> |                                                         |
|    |      | $^2P_{3/2}, M_J = \pm 3/2$ | 14.78                                           |          |                                                 |                                                         |                                                         |
|    |      | $^2P_{3/2}$                | 14.22                                           |          |                                                 |                                                         |                                                         |
|    |      | $^2P_{1/2}$                | 14.25                                           |          |                                                 |                                                         |                                                         |
|    |      |                            | $\bar{\alpha}_{J=3/2} - \alpha_{J=1/2} = -0.03$ |          |                                                 |                                                         |                                                         |
| 35 | Br   | $^2P, M_L = 0$             | 18.77                                           | -1.39    | DHF                                             | <a href="#">2C-NR-CC@dyall.acv4z@(core 35)[vir 477]</a> |                                                         |
|    |      | $^2P, M_L = \pm 1$         | 21.08                                           | -1.59    |                                                 |                                                         |                                                         |
|    |      | $^2P$                      | 20.31                                           | -1.53    |                                                 |                                                         | $\Delta\alpha = 2.31$                                   |
|    |      | $^2P, M_L = 0$             | $20.21 \pm 0.84$                                | 6.21     | MP2                                             | $\Delta\alpha = -1.27$                                  |                                                         |
|    |      | $^2P, M_L = \pm 1$         | $18.94 \pm 1.77$                                | -11.57   |                                                 |                                                         |                                                         |
|    |      | $^2P$                      | $19.36 \pm 1.53$                                | -6.10    |                                                 |                                                         |                                                         |
|    |      | $^2P, M_L = 0$             | 18.85                                           | -0.97    | CCSD                                            |                                                         |                                                         |
|    |      | $^2P, M_L = \pm 1$         | 21.26                                           | -0.74    |                                                 |                                                         |                                                         |
|    |      | $^2P$                      | 20.46                                           | -0.81    |                                                 | $\Delta\alpha = 2.41$                                   |                                                         |
|    |      | $^2P, M_L = 0$             | $19.03 \pm 0.04$                                | --       | CCSD(T)                                         | $\Delta\alpha = 2.39$                                   |                                                         |
|    |      | $^2P, M_L = \pm 1$         | $21.42 \pm 0.03$                                | --       |                                                 |                                                         |                                                         |
|    |      | $^2P$                      | $20.62 \pm 0.03$                                | --       |                                                 |                                                         |                                                         |
|    |      | $^2P, M_L = 0$             | 18.59                                           | -1.65    | DHF                                             |                                                         | <a href="#">2C-SR-CC@dyall.acv4z@(core 17)[vir 183]</a> |
|    |      | $^2P, M_L = \pm 1$         | 21.10                                           | -1.65    |                                                 |                                                         |                                                         |
|    |      | $^2P$                      | 20.26                                           | -1.65    |                                                 |                                                         |                                                         |
|    |      |                            |                                                 |          |                                                 | $\Delta\alpha = 2.52$                                   |                                                         |
|    |      | $^2P, M_L = 0$             | $21.99 \pm 2.38$                                | 16.39    | MP2                                             | $\Delta\alpha = -2.44$                                  |                                                         |
|    |      | $^2P, M_L = \pm 1$         | $19.56 \pm 1.33$                                | -8.85    |                                                 |                                                         |                                                         |
|    |      | $^2P$                      | $20.37 \pm 1.75$                                | -1.13    |                                                 |                                                         |                                                         |
|    |      | $^2P, M_L = 0$             | 18.69                                           | -1.11    | CCSD                                            |                                                         |                                                         |
|    |      | $^2P, M_L = \pm 1$         | 21.29                                           | -0.80    |                                                 |                                                         |                                                         |
|    |      | $^2P$                      | 20.42                                           | -0.89    |                                                 | $\Delta\alpha = 2.60$                                   |                                                         |
|    |      | $^2P, M_L = 0$             | $18.90 \pm 0.07$                                | --       | CCSD(T)                                         | $\Delta\alpha = 2.56$                                   |                                                         |
|    |      | $^2P, M_L = \pm 1$         | $21.46 \pm 0.02$                                | --       |                                                 |                                                         |                                                         |
|    |      | $^2P$                      | $20.60 \pm 0.04$                                | --       |                                                 |                                                         |                                                         |
|    |      |                            |                                                 |          |                                                 |                                                         |                                                         |
|    |      |                            |                                                 |          |                                                 |                                                         |                                                         |
|    |      |                            |                                                 |          |                                                 |                                                         |                                                         |
|    |      |                            |                                                 |          |                                                 |                                                         |                                                         |
|    |      |                            |                                                 |          |                                                 |                                                         |                                                         |
|    |      |                            |                                                 |          |                                                 |                                                         |                                                         |
|    |      |                            |                                                 |          |                                                 |                                                         |                                                         |
|    |      |                            |                                                 |          |                                                 |                                                         |                                                         |
|    |      |                            |                                                 |          |                                                 |                                                         |                                                         |
|    |      |                            |                                                 |          |                                                 |                                                         |                                                         |
|    |      |                            |                                                 |          |                                                 |                                                         |                                                         |
|    |      |                            |                                                 |          |                                                 |                                                         |                                                         |
|    |      |                            |                                                 |          |                                                 |                                                         |                                                         |
|    |      |                            |                                                 |          |                                                 |                                                         |                                                         |
|    |      |                            |                                                 |          |                                                 |                                                         |                                                         |
|    |      |                            |                                                 |          |                                                 |                                                         |                                                         |
|    |      |                            |                                                 |          |                                                 |                                                         |                                                         |
|    |      |                            |                                                 |          |                                                 |                                                         |                                                         |
|    |      |                            |                                                 |          |                                                 |                                                         |                                                         |
|    |      |                            |                                                 |          |                                                 |                                                         |                                                         |
|    |      |                            |                                                 |          |                                                 |                                                         |                                                         |
|    |      |                            |                                                 |          |                                                 |                                                         |                                                         |
|    |      |                            |                                                 |          |                                                 |                                                         |                                                         |
|    |      |                            |                                                 |          |                                                 |                                                         |                                                         |
|    |      |                            |                                                 |          |                                                 |                                                         |                                                         |
|    |      |                            |                                                 |          |                                                 |                                                         |                                                         |
|    |      |                            |                                                 |          |                                                 |                                                         |                                                         |
|    |      |                            |                                                 |          |                                                 |                                                         |                                                         |
|    |      |                            |                                                 |          |                                                 |                                                         |                                                         |
|    |      |                            |                                                 |          |                                                 |                                                         |                                                         |
|    |      |                            |                                                 |          |                                                 |                                                         |                                                         |
|    |      |                            |                                                 |          |                                                 |                                                         |                                                         |
|    |      |                            |                                                 |          |                                                 |                                                         |                                                         |
|    |      |                            |                                                 |          |                                                 |                                                         |                                                         |
|    |      |                            |                                                 |          |                                                 |                                                         |                                                         |
|    |      |                            |                                                 |          |                                                 |                                                         |                                                         |
|    |      |                            |                                                 |          |                                                 |                                                         |                                                         |
|    |      |                            |                                                 |          |                                                 |                                                         |                                                         |
|    |      |                            |                                                 |          |                                                 |                                                         |                                                         |
|    |      |                            |                                                 |          |                                                 |                                                         |                                                         |
|    |      |                            |                                                 |          |                                                 |                                                         |                                                         |
|    |      |                            |                                                 |          |                                                 |                                                         |                                                         |
|    |      |                            |                                                 |          |                                                 |                                                         |                                                         |
|    |      |                            |                                                 |          |                                                 |                                                         |                                                         |
|    |      |                            |                                                 |          |                                                 |                                                         |                                                         |
|    |      |                            |                                                 |          |                                                 |                                                         |                                                         |
|    |      |                            |                                                 |          |                                                 |                                                         |                                                         |
|    |      |                            |                                                 |          |                                                 |                                                         |                                                         |
|    |      |                            |                                                 |          |                                                 |                                                         |                                                         |
|    |      |                            |                                                 |          |                                                 |                                                         |                                                         |
|    |      |                            |                                                 |          |                                                 |                                                         |                                                         |
|    |      |                            |                                                 |          |                                                 |                                                         |                                                         |
|    |      |                            |                                                 |          |                                                 |                                                         |                                                         |
|    |      |                            |                                                 |          |                                                 |                                                         |                                                         |
|    |      |                            |                                                 |          |                                                 |                                                         |                                                         |
|    |      |                            |                                                 |          |                                                 |                                                         |                                                         |
|    |      |                            |                                                 |          |                                                 |                                                         |                                                         |
|    |      |                            |                                                 |          |                                                 |                                                         |                                                         |
|    |      |                            |                                                 |          |                                                 |                                                         |                                                         |
|    |      |                            |                                                 |          |                                                 |                                                         |                                                         |
|    |      |                            |                                                 |          |                                                 |                                                         |                                                         |
|    |      |                            |                                                 |          |                                                 |                                                         |                                                         |
|    |      |                            |                                                 |          |                                                 |                                                         |                                                         |
|    |      |                            |                                                 |          |                                                 |                                                         |                                                         |
|    |      |                            |                                                 |          |                                                 |                                                         |                                                         |
|    |      |                            |                                                 |          |                                                 |                                                         |                                                         |
|    |      |                            |                                                 |          |                                                 |                                                         |                                                         |
|    |      |                            |                                                 |          |                                                 |                                                         |                                                         |
|    |      |                            |                                                 |          |                                                 |                                                         |                                                         |
|    |      |                            |                                                 |          |                                                 |                                                         |                                                         |
|    |      |                            |                                                 |          |                                                 |                                                         |                                                         |
|    |      |                            |                                                 |          |                                                 |                                                         |                                                         |
|    |      |                            |                                                 |          |                                                 |                                                         |                                                         |
|    |      |                            |                                                 |          |                                                 |                                                         |                                                         |
|    |      |                            |                                                 |          |                                                 |                                                         |                                                         |
|    |      |                            |                                                 |          |                                                 |                                                         |                                                         |
|    |      |                            |                                                 |          |                                                 |                                                         |                                                         |
|    |      |                            |                                                 |          |                                                 |                                                         |                                                         |
|    |      |                            |                                                 |          |                                                 |                                                         |                                                         |
|    |      |                            |                                                 |          |                                                 |                                                         |                                                         |
|    |      |                            |                                                 |          |                                                 |                                                         |                                                         |
|    |      |                            |                                                 |          |                                                 |                                                         |                                                         |
|    |      |                            |                                                 |          |                                                 |                                                         |                                                         |
|    |      |                            |                                                 |          |                                                 |                                                         |                                                         |
|    |      |                            |                                                 |          |                                                 |                                                         |                                                         |
|    |      |                            |                                                 |          |                                                 |                                                         |                                                         |
|    |      |                            |                                                 |          |                                                 |                                                         |                                                         |
|    |      |                            |                                                 |          |                                                 |                                                         |                                                         |
|    |      |                            |                                                 |          |                                                 |                                                         |                                                         |
|    |      |                            |                                                 |          |                                                 |                                                         |                                                         |
|    |      |                            |                                                 |          |                                                 |                                                         |                                                         |
|    |      |                            |                                                 |          |                                                 |                                                         |                                                         |
|    |      |                            |                                                 |          |                                                 |                                                         |                                                         |
|    |      |                            |                                                 |          |                                                 |                                                         |                                                         |
|    |      |                            |                                                 |          |                                                 |                                                         |                                                         |
|    |      |                            |                                                 |          |                                                 |                                                         |                                                         |
|    |      |                            |                                                 |          |                                                 |                                                         |                                                         |
|    |      |                            |                                                 |          |                                                 |                                                         |                                                         |
|    |      |                            |                                                 |          |                                                 |                                                         |                                                         |
|    |      |                            |                                                 |          |                                                 |                                                         |                                                         |
|    |      |                            |                                                 |          |                                                 |                                                         |                                                         |
|    |      |                            |                                                 |          |                                                 |                                                         |                                                         |
|    |      |                            |                                                 |          |                                                 |                                                         |                                                         |
|    |      |                            |                                                 |          |                                                 |                                                         |                                                         |
|    |      |                            |                                                 |          |                                                 |                                                         |                                                         |
|    |      |                            |                                                 |          |                                                 |                                                         |                                                         |
|    |      |                            |                                                 |          |                                                 |                                                         |                                                         |
|    |      |                            |                                                 |          |                                                 |                                                         |                                                         |
|    |      |                            |                                                 |          |                                                 |                                                         |                                                         |
|    |      |                            |                                                 |          |                                                 |                                                         |                                                         |
|    |      |                            |                                                 |          |                                                 |                                                         |                                                         |
|    |      |                            |                                                 |          |                                                 |                                                         |                                                         |
|    |      |                            |                                                 |          |                                                 |                                                         |                                                         |
|    |      |                            |                                                 |          |                                                 |                                                         |                                                         |
|    |      |                            |                                                 |          |                                                 |                                                         |                                                         |
|    |      |                            |                                                 |          |                                                 |                                                         |                                                         |
|    |      |                            |                                                 |          |                                                 |                                                         |                                                         |
|    |      |                            |                                                 |          |                                                 |                                                         |                                                         |
|    |      |                            |                                                 |          |                                                 |                                                         |                                                         |
|    |      |                            |                                                 |          |                                                 |                                                         |                                                         |
|    |      |                            |                                                 |          |                                                 |                                                         |                                                         |
|    |      |                            |                                                 |          |                                                 |                                                         |                                                         |
|    |      |                            |                                                 |          |                                                 |                                                         |                                                         |
|    |      |                            |                                                 |          |                                                 |                                                         |                                                         |
|    |      |                            |                                                 |          |                                                 |                                                         |                                                         |
|    |      |                            |                                                 |          |                                                 |                                                         |                                                         |
|    |      |                            |                                                 |          |                                                 |                                                         |                                                         |
|    |      |                            |                                                 |          |                                                 |                                                         |                                                         |
|    |      |                            |                                                 |          |                                                 |                                                         |                                                         |
|    |      |                            |                                                 |          |                                                 |                                                         |                                                         |
|    |      |                            |                                                 |          |                                                 |                                                         |                                                         |
|    |      |                            |                                                 |          |                                                 |                                                         |                                                         |
|    |      |                            |                                                 |          |                                                 |                                                         |                                                         |
|    |      |                            |                                                 |          |                                                 |                                                         |                                                         |

(continued)



Table S15. continued.

| Z  | Atom | State                      | $\alpha_D$ (a.u.) | $\delta$ | Method                | Comments                                                |                         |
|----|------|----------------------------|-------------------|----------|-----------------------|---------------------------------------------------------|-------------------------|
|    |      | $^2P, M_L = \pm 1$         | 21.10             | -2.05    | MP2                   | $\Delta\alpha = 2.52$                                   |                         |
|    |      | $^2P$                      | 20.26             | -1.96    |                       |                                                         |                         |
|    |      | $^2P, M_L = 0$             | $22.21 \pm 2.5$   | 17.38    |                       | $\Delta\alpha = -0.37$                                  |                         |
|    |      | $^2P, M_L = \pm 1$         | $21.84 \pm 0.44$  | 1.37     |                       |                                                         |                         |
|    |      | $^2P$                      | $21.96 \pm 1.49$  | 6.25     | CCSD                  | $\Delta\alpha = 2.63$                                   |                         |
|    |      | $^2P, M_L = 0$             | 18.68             | -1.24    |                       |                                                         |                         |
|    |      | $^2P, M_L = \pm 1$         | 21.31             | -1.06    |                       | CCSD(T)                                                 |                         |
|    |      | $^2P$                      | 20.44             | -1.12    |                       |                                                         |                         |
|    |      | $^2P, M_L = 0$             | $18.92 \pm 0.08$  | --       | $\Delta\alpha = 2.62$ |                                                         |                         |
|    |      | $^2P, M_L = \pm 1$         | $21.54 \pm 0.02$  | --       |                       |                                                         |                         |
|    |      | $^2P$                      | $20.67 \pm 0.05$  | --       |                       |                                                         |                         |
|    |      | $^2P_{3/2}, M_J = \pm 1/2$ | 19.16             |          | MRCISD                | <a href="#">4C-DC-CI@dyall.acv4z@(core 17)[vir 183]</a> |                         |
|    |      | $^2P_{3/2}, M_J = \pm 3/2$ | 20.96             |          |                       |                                                         |                         |
|    |      | $^2P_{3/2}$                | 20.06             |          |                       |                                                         |                         |
|    |      | $^2P_{1/2}$                | 20.28             |          |                       | $\bar{\alpha}_{J=3/2} - \alpha_{J=1/2} = -0.22$         |                         |
| 53 | I    | $^2P, M_L = 0$             | 30.51             | -1.24    | DHF                   | <a href="#">2C-NR-CC@dyall.acv4z@(core 53)[vir 549]</a> |                         |
|    |      | $^2P, M_L = \pm 1$         | 33.30             | 0.17     |                       |                                                         |                         |
|    |      | $^2P$                      | 32.37             | -0.28    | MP2                   | $\Delta\alpha = 2.79$                                   |                         |
|    |      | $^2P, M_L = 0$             | $50.03 \pm 12.7$  | 61.96    |                       |                                                         |                         |
|    |      | $^2P, M_L = \pm 1$         | $31.89 \pm 0.74$  | -4.06    |                       | CCSD                                                    | $\Delta\alpha = -18.14$ |
|    |      | $^2P$                      | $37.94 \pm 7.36$  | 16.88    |                       |                                                         |                         |
|    |      | $^2P, M_L = 0$             | 30.12             | -2.51    | CCSD(T)               |                                                         | $\Delta\alpha = 2.89$   |
|    |      | $^2P, M_L = \pm 1$         | 33.01             | -0.70    |                       |                                                         |                         |
|    |      | $^2P$                      | 32.05             | -1.27    | $\Delta\alpha = 2.35$ |                                                         |                         |
|    |      | $^2P, M_L = 0$             | $30.89 \pm 0.39$  | --       |                       |                                                         |                         |
|    |      | $^2P, M_L = \pm 1$         | $33.24 \pm 0.01$  | --       |                       |                                                         |                         |
|    |      | $^2P$                      | $32.46 \pm 0.23$  | --       |                       |                                                         |                         |
|    |      | $^2P, M_L = 0$             | 29.62             | -0.13    | DHF                   | <a href="#">2C-SR-CC@dyall.acv4z@(core 17)[vir 215]</a> |                         |
|    |      | $^2P, M_L = \pm 1$         | 33.10             | -0.55    | MP2                   | $\Delta\alpha = 3.48$                                   |                         |
|    |      | $^2P$                      | 31.94             | -0.42    |                       |                                                         |                         |
|    |      | $^2P, M_L = 0$             | $30.57 \pm 0.47$  | 3.04     |                       | CCSD                                                    | $\Delta\alpha = 1.49$   |
|    |      | $^2P, M_L = \pm 1$         | $32.06 \pm 0.66$  | -3.68    |                       |                                                         |                         |
|    |      | $^2P$                      | $31.56 \pm 0.6$   | -1.61    | CCSD(T)               |                                                         | $\Delta\alpha = 3.57$   |
|    |      | $^2P, M_L = 0$             | 29.45             | -0.73    |                       |                                                         |                         |
|    |      | $^2P, M_L = \pm 1$         | 33.02             | -0.79    | $\Delta\alpha = 3.57$ |                                                         |                         |
|    |      | $^2P$                      | 31.83             | -0.77    |                       |                                                         |                         |
|    |      | $^2P, M_L = 0$             | $29.66 \pm 0.01$  | --       |                       |                                                         |                         |
|    |      | $^2P, M_L = \pm 1$         | $33.28 \pm 0.01$  | --       |                       |                                                         |                         |

(continued)

Table S15. continued.

| Z  | Atom | State                      | $\alpha_D$ (a.u.) | $\delta$ | Method  | Comments                                                |
|----|------|----------------------------|-------------------|----------|---------|---------------------------------------------------------|
|    |      | $^2P$                      | $32.08 \pm 0.01$  | --       |         | $\Delta\alpha = 3.62$                                   |
|    |      | $^2P, M_L = 0$             | 29.62             | 0.16     | DHF     | <a href="#">2C-SR-CC@dyall.acv4z@(core 53)[vir 549]</a> |
|    |      | $^2P, M_L = \pm 1$         | 33.10             | -0.38    |         |                                                         |
|    |      | $^2P$                      | 31.94             | -0.21    |         | $\Delta\alpha = 3.48$                                   |
|    |      | $^2P, M_L = 0$             | $30.96 \pm 0.79$  | 4.66     | MP2     |                                                         |
|    |      | $^2P, M_L = \pm 1$         | $32.83 \pm 0.04$  | -1.20    |         |                                                         |
|    |      | $^2P$                      | $32.20 \pm 0.46$  | 0.60     |         | $\Delta\alpha = 1.87$                                   |
|    |      | $^2P, M_L = 0$             | 29.35             | -0.76    | CCSD    |                                                         |
|    |      | $^2P, M_L = \pm 1$         | 32.95             | -0.82    |         |                                                         |
|    |      | $^2P$                      | 31.75             | -0.80    |         | $\Delta\alpha = 3.60$                                   |
|    |      | $^2P, M_L = 0$             | $29.58 \pm 0.02$  | --       | CCSD(T) |                                                         |
|    |      | $^2P, M_L = \pm 1$         | 33.23             | --       |         |                                                         |
|    |      | $^2P$                      | $32.01 \pm 0.01$  | --       |         | $\Delta\alpha = 3.65$                                   |
|    |      | $^2P_{3/2}, M_J = \pm 1/2$ | 29.93             |          | MRCISD  | <a href="#">4C-DC-CI@dyall.acv4z@(core 17)[vir 215]</a> |
|    |      | $^2P_{3/2}, M_J = \pm 3/2$ | 32.66             |          |         |                                                         |
|    |      | $^2P_{3/2}$                | 31.29             |          |         |                                                         |
|    |      | $^2P_{1/2}$                | 32.02             |          |         | $\bar{\alpha}_{J=3/2} - \alpha_{J=1/2} = -0.73$         |
| 85 | At   | $^2P, M_L = 0$             | $38.03 \pm 0.01$  | 1.37     | DHF     | <a href="#">2C-NR-CC@dyall.acv4z@(core 49)[vir 295]</a> |
|    |      | $^2P, M_L = \pm 1$         | $41.35 \pm 0.03$  | 0.80     |         |                                                         |
|    |      | $^2P$                      | $40.24 \pm 0.02$  | 0.97     |         | $\Delta\alpha = 3.32$                                   |
|    |      | $^2P, M_L = 0$             | $38.09 \pm 0.04$  | 1.54     | MP2     |                                                         |
|    |      | $^2P, M_L = \pm 1$         | $40.60 \pm 0.02$  | -1.02    |         |                                                         |
|    |      | $^2P$                      | $39.77 \pm 0.03$  | -0.22    |         | $\Delta\alpha = 2.51$                                   |
|    |      | $^2P, M_L = 0$             | $37.31 \pm 0.01$  | -0.55    | CCSD    |                                                         |
|    |      | $^2P, M_L = \pm 1$         | $40.72 \pm 0.03$  | -0.73    |         |                                                         |
|    |      | $^2P$                      | $39.59 \pm 0.02$  | -0.67    |         | $\Delta\alpha = 3.41$                                   |
|    |      | $^2P, M_L = 0$             | $37.52 \pm 0.01$  | --       | CCSD(T) |                                                         |
|    |      | $^2P, M_L = \pm 1$         | $41.02 \pm 0.03$  | --       |         |                                                         |
|    |      | $^2P$                      | $39.85 \pm 0.02$  | --       |         | $\Delta\alpha = 3.50$                                   |
|    |      | $^2P, M_L = 0$             | $34.90 \pm 0.01$  | -0.42    | DHF     | <a href="#">2C-SR-CC@dyall.acv4z@(core 17)[vir 261]</a> |
|    |      | $^2P, M_L = \pm 1$         | $40.44 \pm 0.03$  | -0.81    |         |                                                         |
|    |      | $^2P$                      | $38.59 \pm 0.02$  | -0.69    |         | $\Delta\alpha = 5.54$                                   |
|    |      | $^2P, M_L = 0$             | $35.59 \pm 0.01$  | 1.57     | MP2     |                                                         |
|    |      | $^2P, M_L = \pm 1$         | $40.22 \pm 0.04$  | -1.34    |         |                                                         |
|    |      | $^2P$                      | $38.68 \pm 0.03$  | -0.46    |         | $\Delta\alpha = 4.63$                                   |
|    |      | $^2P, M_L = 0$             | $34.76 \pm 0.01$  | -0.80    | CCSD    |                                                         |
|    |      | $^2P, M_L = \pm 1$         | $40.39 \pm 0.03$  | -0.93    |         |                                                         |
|    |      | $^2P$                      | $38.51 \pm 0.03$  | -0.89    |         | $\Delta\alpha = 5.63$                                   |

(continued)

Table S15. continued.

| Z   | Atom | State                      | $\alpha_D$ (a.u.) | $\delta$ | Method  | Comments                                                |
|-----|------|----------------------------|-------------------|----------|---------|---------------------------------------------------------|
|     |      | $^2P, M_L = 0$             | $35.04 \pm 0.02$  | --       | CCSD(T) |                                                         |
|     |      | $^2P, M_L = \pm 1$         | $40.77 \pm 0.03$  | --       |         |                                                         |
|     |      | $^2P$                      | $38.86 \pm 0.03$  | --       |         | $\Delta\alpha = 5.73$                                   |
|     |      | $^2P, M_L = 0$             | $34.90 \pm 0.01$  | -0.11    | DHF     | <a href="#">2C-SR-CC@dyall.acv4z@(core 49)[vir 295]</a> |
|     |      | $^2P, M_L = \pm 1$         | $40.44 \pm 0.03$  | -0.60    |         |                                                         |
|     |      | $^2P$                      | $38.59 \pm 0.02$  | -0.45    |         | $\Delta\alpha = 5.54$                                   |
|     |      | $^2P, M_L = 0$             | $35.62 \pm 0.02$  | 1.97     | MP2     |                                                         |
|     |      | $^2P, M_L = \pm 1$         | $40.06 \pm 0.02$  | -1.53    |         |                                                         |
|     |      | $^2P$                      | $38.58 \pm 0.02$  | -0.48    |         | $\Delta\alpha = 4.44$                                   |
|     |      | $^2P, M_L = 0$             | $34.66 \pm 0.01$  | -0.79    | CCSD    |                                                         |
|     |      | $^2P, M_L = \pm 1$         | $40.29 \pm 0.03$  | -0.97    |         |                                                         |
|     |      | $^2P$                      | $38.41 \pm 0.02$  | -0.92    |         | $\Delta\alpha = 5.63$                                   |
|     |      | $^2P, M_L = 0$             | $34.93 \pm 0.01$  | --       | CCSD(T) |                                                         |
|     |      | $^2P, M_L = \pm 1$         | $40.68 \pm 0.03$  | --       |         |                                                         |
|     |      | $^2P$                      | $38.77 \pm 0.02$  | --       |         | $\Delta\alpha = 5.75$                                   |
|     |      | $^2P_{3/2}, M_J = \pm 1/2$ | 36.27             |          | MRCISD  | <a href="#">4C-DC-CI@dyall.acv4z@(core 17)[vir 261]</a> |
|     |      | $^2P_{3/2}, M_J = \pm 3/2$ | 41.64             |          |         |                                                         |
|     |      | $^2P_{3/2}$                | 38.96             |          |         |                                                         |
|     |      | $^2P_{1/2}$                | 40.82             |          |         | $\bar{\alpha}_{J=3/2} - \alpha_{J=1/2} = -1.86$         |
| 117 | Ts   | $^2P, M_L = 0$             | $53.75 \pm 0.01$  | 2.04     | DHF     | <a href="#">2C-NR-CC@dyall.acv4z@(core 49)[vir 293]</a> |
|     |      | $^2P, M_L = \pm 1$         | 50.61             | 2.43     |         |                                                         |
|     |      | $^2P$                      | $51.66 \pm 0.01$  | 2.30     |         | $\Delta\alpha = -3.14$                                  |
|     |      | $^2P, M_L = 0$             | $48.84 \pm 1.24$  | -7.29    | MP2     |                                                         |
|     |      | $^2P, M_L = \pm 1$         | $49.78 \pm 0.1$   | 0.74     |         |                                                         |
|     |      | $^2P$                      | $49.46 \pm 0.72$  | -2.05    |         | $\Delta\alpha = 0.94$                                   |
|     |      | $^2P, M_L = 0$             | $52.46 \pm 0.01$  | -0.41    | CCSD    |                                                         |
|     |      | $^2P, M_L = \pm 1$         | $49.23 \pm 0.01$  | -0.36    |         |                                                         |
|     |      | $^2P$                      | $50.31 \pm 0.01$  | -0.38    |         | $\Delta\alpha = -3.23$                                  |
|     |      | $^2P, M_L = 0$             | $52.68 \pm 0.03$  | --       | CCSD(T) |                                                         |
|     |      | $^2P, M_L = \pm 1$         | $49.41 \pm 0.02$  | --       |         |                                                         |
|     |      | $^2P$                      | $50.50 \pm 0.02$  | --       |         | $\Delta\alpha = -3.27$                                  |
|     |      | $^2P, M_L = 0$             | 44.03             | -0.01    | DHF     | <a href="#">2C-SR-CC@dyall.acv4z@(core 17)[vir 247]</a> |
|     |      | $^2P, M_L = \pm 1$         | $53.37 \pm 0.01$  | -0.23    |         |                                                         |
|     |      | $^2P$                      | 50.26             | -0.17    |         | $\Delta\alpha = 9.34$                                   |
|     |      | $^2P, M_L = 0$             | $42.43 \pm 0.32$  | -3.66    | MP2     |                                                         |
|     |      | $^2P, M_L = \pm 1$         | $53.62 \pm 0.35$  | 0.24     |         |                                                         |
|     |      | $^2P$                      | $49.89 \pm 0.34$  | -0.90    |         | $\Delta\alpha = 11.20$                                  |
|     |      | $^2P, M_L = 0$             | 43.90             | -0.31    | CCSD    |                                                         |

(continued)

Table S15. continued.

| Z | Atom | State                      | $\alpha_D$ (a.u.) | $\delta$ | Method  | Comments                                                |
|---|------|----------------------------|-------------------|----------|---------|---------------------------------------------------------|
|   |      | $^2P, M_L = \pm 1$         | $53.05 \pm 0.01$  | -0.84    |         |                                                         |
|   |      | $^2P$                      | 50.00             | -0.69    |         | $\Delta\alpha = 9.15$                                   |
|   |      | $^2P, M_L = 0$             | $44.04 \pm 0.1$   | --       | CCSD(T) |                                                         |
|   |      | $^2P, M_L = \pm 1$         | 53.50             | --       |         |                                                         |
|   |      | $^2P$                      | $50.34 \pm 0.06$  | --       |         | $\Delta\alpha = 9.46$                                   |
|   |      | $^2P, M_L = 0$             | 44.03             | 0.41     | DHF     | <a href="#">2C-SR-CC@dyall.acv4z@(core 49)[vir 293]</a> |
|   |      | $^2P, M_L = \pm 1$         | $53.37 \pm 0.01$  | 0.12     |         |                                                         |
|   |      | $^2P$                      | 50.26             | 0.21     |         | $\Delta\alpha = 9.34$                                   |
|   |      | $^2P, M_L = 0$             | $42.28 \pm 0.42$  | -3.58    | MP2     |                                                         |
|   |      | $^2P, M_L = \pm 1$         | $53.47 \pm 0.62$  | 0.30     |         |                                                         |
|   |      | $^2P$                      | $49.74 \pm 0.56$  | -0.83    |         | $\Delta\alpha = 11.19$                                  |
|   |      | $^2P, M_L = 0$             | 43.72             | -0.31    | CCSD    |                                                         |
|   |      | $^2P, M_L = \pm 1$         | 52.83             | -0.90    |         |                                                         |
|   |      | $^2P$                      | 49.79             | -0.73    |         | $\Delta\alpha = 9.11$                                   |
|   |      | $^2P, M_L = 0$             | $43.85 \pm 0.1$   | --       | CCSD(T) |                                                         |
|   |      | $^2P, M_L = \pm 1$         | $53.31 \pm 0.01$  | --       |         |                                                         |
|   |      | $^2P$                      | $50.16 \pm 0.06$  | --       |         | $\Delta\alpha = 9.46$                                   |
|   |      | $^2P_{3/2}, M_J = \pm 1/2$ | 58.42             |          | MRCISD  | <a href="#">4C-DC-CI@dyall.acv4z@(core 17)[vir 247]</a> |
|   |      | $^2P_{3/2}, M_J = \pm 3/2$ | 71.92             |          |         |                                                         |
|   |      | $^2P_{3/2}$                | 65.17             |          |         |                                                         |
|   |      | $^2P_{1/2}$                | $227.38 \pm 0.01$ |          |         | $\bar{\alpha}_{J=3/2} - \alpha_{J=1/2} = -162.21$       |

## S2.8 Group 18 elements

Table S16: The results of dipole polarizability for Group 18 elements.

| Z | Atom | State          | $\alpha_D$ (a.u.) | $\delta$ (%) | Method  | Comments                                               |
|---|------|----------------|-------------------|--------------|---------|--------------------------------------------------------|
| 2 | He   | $^1S, M_L = 0$ | 1.32              | -4.50        | DHF     | <a href="#">2C-NR-CC@dyall.acv4z@(core 2)[vir 104]</a> |
|   |      |                | 1.36              | -1.73        | MP2     |                                                        |
|   |      |                | 1.38              | 0.00         | CCSD    |                                                        |
|   |      |                | 1.38              | --           | CCSD(T) |                                                        |
|   |      | $^1S, M_L = 0$ | 1.32              | -4.50        | DHF     | <a href="#">2C-SR-CC@dyall.acv4z@(core 2)[vir 104]</a> |
|   |      |                | 1.36              | -1.73        | MP2     |                                                        |
|   |      |                | 1.38              | 0.00         | CCSD    |                                                        |
|   |      |                | 1.38              | --           | CCSD(T) |                                                        |

(continued)

Table S16. continued.

| Z  | Atom | State          | $\alpha_D$ (a.u.) | $\delta$ | Method  | Comments                                       |
|----|------|----------------|-------------------|----------|---------|------------------------------------------------|
| 10 | Ne   | $^1S_0$        | 1.32              | -4.50    | DHF     | <b>4C-DC-CC@dyall.acv4z@(core 2)[vir 104]</b>  |
|    |      |                | 1.36              | -1.73    | MP2     |                                                |
|    |      |                | 1.38              | 0.00     | CCSD    |                                                |
|    |      |                | 1.38              | --       | CCSD(T) |                                                |
|    |      | $^1S, M_L = 0$ | 2.31              | -9.97    | DHF     | <b>2C-NR-CC@dyall.acv4z@(core 10)[vir 246]</b> |
|    |      |                | 2.59              | 1.01     | MP2     |                                                |
|    |      |                | 2.53              | -1.60    | CCSD    |                                                |
|    |      |                | 2.57              | --       | CCSD(T) |                                                |
|    |      | $^1S, M_L = 0$ | 2.32              | -10.00   | DHF     | <b>2C-SR-CC@dyall.acv4z@(core 10)[vir 246]</b> |
|    |      |                | 2.60              | 1.01     | MP2     |                                                |
|    |      |                | 2.53              | -1.60    | CCSD    |                                                |
|    |      |                | 2.57              | --       | CCSD(T) |                                                |
|    |      | $^1S_0$        | 2.32              | -9.99    | DHF     | 2C-DC-CC@dyall.acv4z@(core 10)[vir 246]        |
|    |      |                | 2.60              | 1.02     | MP2     |                                                |
|    |      |                | 2.53              | -1.60    | CCSD    |                                                |
|    |      |                | 2.57              | --       | CCSD(T) |                                                |
|    |      | $^1S_0$        | 2.32              | -10.00   | DHF     | <b>4C-DC-CC@dyall.acv4z@(core 10)[vir 246]</b> |
|    |      |                | 2.60              | 1.01     | MP2     |                                                |
|    |      |                | 2.53              | -1.60    | CCSD    |                                                |
|    |      |                | 2.57              | --       | CCSD(T) |                                                |
| 18 | Ar   | $^1S, M_L = 0$ | 10.71             | -2.68    | DHF     | <b>2C-NR-CC@dyall.acv4z@(core 18)[vir 358]</b> |
|    |      |                | 11.04             | 0.28     | MP2     |                                                |
|    |      |                | 10.91             | -0.87    | CCSD    |                                                |
|    |      |                | 11.01             | --       | CCSD(T) |                                                |
|    |      | $^1S, M_L = 0$ | 10.73             | -2.72    | DHF     | <b>2C-SR-CC@dyall.acv4z@(core 18)[vir 358]</b> |
|    |      |                | 11.06             | 0.28     | MP2     |                                                |
|    |      |                | 10.93             | -0.88    | CCSD    |                                                |
|    |      |                | 11.03             | --       | CCSD(T) |                                                |
|    |      | $^1S_0$        | 10.73             | -2.71    | DHF     | 2C-DC-CC@dyall.acv4z@(core 18)[vir 358]        |
|    |      |                | 11.06             | 0.28     | MP2     |                                                |
|    |      |                | 10.93             | -0.88    | CCSD    |                                                |
|    |      |                | 11.02             | --       | CCSD(T) |                                                |
|    |      | $^1S_0$        | 10.73             | -2.72    | DHF     | <b>4C-DC-CC@dyall.acv4z@(core 18)[vir 358]</b> |
|    |      |                | 11.06             | 0.28     | MP2     |                                                |
|    |      |                | 10.93             | -0.88    | CCSD    |                                                |
|    |      |                | 11.02             | --       | CCSD(T) |                                                |
| 36 | Kr   | $^1S, M_L = 0$ | 16.46             | -1.88    | DHF     | <b>2C-NR-CC@dyall.acv4z@(core 36)[vir 476]</b> |
|    |      |                | 16.75             | -0.15    | MP2     |                                                |

(continued)

Table S16. continued.

| Z  | Atom | State          | $\alpha_D$ (a.u.) | $\delta$ | Method  | Comments                                      |
|----|------|----------------|-------------------|----------|---------|-----------------------------------------------|
|    |      |                | 16.64             | -0.82    | CCSD    |                                               |
|    |      |                | 16.78             | --       | CCSD(T) |                                               |
|    |      | $^1S, M_L = 0$ | 16.44             | -1.92    | DHF     | 2C-SR-CC@d-aug-dyall.acv4z@(core 36)[vir 620] |
|    |      |                | 16.75             | -0.12    | MP2     |                                               |
|    |      |                | 16.62             | -0.86    | CCSD    |                                               |
|    |      |                | 16.77             | --       | CCSD(T) |                                               |
|    |      |                | 16.43             | -2.03    | DHF     | 2C-SR-CC@dyall.acv4z@(core 36)[vir 476]       |
|    |      |                | 16.75             | -0.14    | MP2     |                                               |
|    |      |                | 16.63             | -0.84    | CCSD    |                                               |
|    |      |                | 16.77             | --       | CCSD(T) |                                               |
|    |      | $^1S_0$        | 16.45             | -2.03    | DHF     | 2C-DC-CC@dyall.acv4z@(core 36)[vir 476]       |
|    |      |                | 16.77             | -0.15    | MP2     |                                               |
|    |      |                | 16.65             | -0.84    | CCSD    |                                               |
|    |      |                | 16.80             | --       | CCSD(T) |                                               |
|    |      | $^1S_0$        | 16.46             | -2.16    | DHF     | 4C-DC-CC@dyall.acv4z@(core 26)[vir 232]       |
|    |      |                | 16.79             | -0.15    | MP2     |                                               |
|    |      |                | 16.68             | -0.83    | CCSD    |                                               |
|    |      |                | 16.82             | --       | CCSD(T) |                                               |
| 54 | Xe   | $^1S, M_L = 0$ | 27.10             | -0.50    | DHF     | 2C-NR-CC@dyall.acv4z@(core 26)[vir 286]       |
|    |      |                | 27.13             | -0.38    | MP2     |                                               |
|    |      |                | 27.04             | -0.70    | CCSD    |                                               |
|    |      |                | 27.23             | --       | CCSD(T) |                                               |
|    |      | $^1S, M_L = 0$ | 26.77             | -0.94    | DHF     | 2C-SR-CC@d-aug-dyall.acv4z@(core 26)[vir 430] |
|    |      |                | 26.94             | -0.31    | MP2     |                                               |
|    |      |                | 26.81             | -0.79    | CCSD    |                                               |
|    |      |                | 27.03             | --       | CCSD(T) |                                               |
|    |      | $^1S, M_L = 0$ | 26.77             | -0.96    | DHF     | 2C-SR-CC@d-aug-dyall.acv4z@(core 50)[vir 430] |
|    |      |                | 26.94             | -0.34    | MP2     |                                               |
|    |      |                | 26.81             | -0.80    | CCSD    |                                               |
|    |      |                | 27.03             | --       | CCSD(T) |                                               |
|    |      | $^1S, M_L = 0$ | 26.76             | -0.96    | DHF     | 2C-SR-CC@dyall.acv4z@(core 26)[vir 286]       |
|    |      |                | 26.92             | -0.34    | MP2     |                                               |
|    |      |                | 26.81             | -0.77    | CCSD    |                                               |
|    |      |                | 27.02             | --       | CCSD(T) |                                               |
|    |      | $^1S_0$        | 26.96             | -0.91    | DHF     | 2C-DC-CC@dyall.acv4z@(core 50)[vir 286]       |
|    |      |                | 27.11             | -0.37    | MP2     |                                               |
|    |      |                | 27.00             | -0.76    | CCSD    |                                               |
|    |      |                | 27.21             | --       | CCSD(T) |                                               |

(continued)

Table S16. continued.

| Z   | Atom | State          | $\alpha_D$ (a.u.) | $\delta$ | Method  | Comments                                      |
|-----|------|----------------|-------------------|----------|---------|-----------------------------------------------|
| 86  | Rn   | $^1S_0$        | 26.96             | -2.36    | DHF     | 2C-DC-CC@dyall.acv4z@(core 8)[vir 286]        |
|     |      |                | 27.64             | 0.10     | MP2     |                                               |
|     |      |                | 27.43             | -0.66    | CCSD    |                                               |
|     |      |                | 27.61             | --       | CCSD(T) |                                               |
|     |      | $^1S_0$        | 26.95             | -0.91    | DHF     | 4C-DC-CC@dyall.acv4z@(core 50)[vir 286]       |
|     |      |                | 27.10             | -0.37    | MP2     |                                               |
|     |      |                | 26.99             | -0.76    | CCSD    |                                               |
|     |      |                | 27.20             | --       | CCSD(T) |                                               |
|     |      | $^1S, M_L = 0$ | 34.13             | 0.15     | DHF     | 2C-NR-CC@dyall.acv4z@(core 50)[vir 294]       |
|     |      |                | 33.92             | -0.46    | MP2     |                                               |
|     |      |                | 33.84             | -0.69    | CCSD    |                                               |
|     |      |                | 34.08             | --       | CCSD(T) |                                               |
|     |      | $^1S, M_L = 0$ | 32.80             | -1.15    | DHF     | 2C-SR-CC@d-aug-dyall.acv4z@(core 40)[vir 438] |
|     |      |                | 33.13             | -0.15    | MP2     |                                               |
|     |      |                | 32.89             | -0.89    | CCSD    |                                               |
|     |      |                | 33.18             | --       | CCSD(T) |                                               |
|     |      | $^1S, M_L = 0$ | 32.79             | -1.15    | DHF     | 2C-SR-CC@dyall.acv4z@(core 40)[vir 294]       |
|     |      |                | 33.10             | -0.22    | MP2     |                                               |
|     |      |                | 32.88             | -0.86    | CCSD    |                                               |
|     |      |                | 33.17             | --       | CCSD(T) |                                               |
|     |      | $^1S, M_L = 0$ | 32.79             | -1.04    | DHF     | 2C-SR-CC@dyall.acv4z@(core 50)[vir 294]       |
|     |      |                | 33.04             | -0.28    | MP2     |                                               |
|     |      |                | 32.85             | -0.87    | CCSD    |                                               |
|     |      |                | 33.13             | --       | CCSD(T) |                                               |
| 118 | Og   | $^1S_0$        | 34.97             | -0.37    | DHF     | 2C-DC-CC@dyall.acv4z@(core 18)[vir 294]       |
|     |      |                | 34.98             | -0.36    | MP2     |                                               |
|     |      |                | 34.85             | -0.73    | CCSD    |                                               |
|     |      |                | 35.10             | --       | CCSD(T) |                                               |
|     |      | $^1S_0$        | 34.97             | -0.34    | DHF     | 2C-DC-CC@dyall.acv4z@(core 50)[vir 294]       |
|     |      |                | 34.93             | -0.48    | MP2     |                                               |
|     |      |                | 34.83             | -0.76    | CCSD    |                                               |
|     |      |                | 35.09             | --       | CCSD(T) |                                               |
|     |      | $^1S_0$        | 34.96             | -0.34    | DHF     | 4C-DC-CC@dyall.acv4z@(core 50)[vir 294]       |
|     |      |                | 34.91             | -0.48    | MP2     |                                               |
|     |      |                | 34.82             | -0.76    | CCSD    |                                               |
|     |      |                | 35.08             | --       | CCSD(T) |                                               |
|     |      | $^1S, M_L = 0$ | 45.62             | 0.76     | DHF     | 2C-NR-CC@dyall.acv4z@(core 50)[vir 278]       |
|     |      |                | 45.03             | -0.55    | MP2     |                                               |

(continued)

Table S16. continued.

| Z | Atom | State          | $\alpha_D$ (a.u.) | $\delta$ | Method  | Comments                                       |
|---|------|----------------|-------------------|----------|---------|------------------------------------------------|
|   |      |                | 44.99             | -0.63    | CCSD    |                                                |
|   |      |                | 45.28             | --       | CCSD(T) |                                                |
|   |      | $^1S, M_L = 0$ | 43.62             | -0.06    | DHF     | 2C-SR-CC@d-aug-dyall.acv4z@(core 50)[vir 422]  |
|   |      |                | 43.50             | -0.33    | MP2     |                                                |
|   |      |                | 43.31             | -0.76    | CCSD    |                                                |
|   |      |                | 43.65             | --       | CCSD(T) |                                                |
|   |      | $^1S, M_L = 0$ | 43.58             | -0.43    | DHF     | <b>2C-SR-CC@dyall.acv4z@(core 50)[vir 278]</b> |
|   |      |                | 43.55             | -0.49    | MP2     |                                                |
|   |      |                | 43.43             | -0.76    | CCSD    |                                                |
|   |      |                | 43.77             | --       | CCSD(T) |                                                |
|   |      | $^1S_0$        | 60.58             | 4.71     | DHF     | 2C-DC-CC@dyall.acv4z@(core 18)[vir 278]        |
|   |      |                | 56.21             | -2.84    | MP2     |                                                |
|   |      |                | $57.83 \pm 0.01$  | -0.05    | CCSD    |                                                |
|   |      |                | $57.86 \pm 0.01$  | --       | CCSD(T) |                                                |
|   |      | $^1S_0$        | 60.58             | 4.53     | DHF     | 2C-DC-CC@dyall.acv4z@(core 40)[vir 278]        |
|   |      |                | 55.91             | -3.53    | MP2     |                                                |
|   |      |                | $57.92 \pm 0.05$  | -0.07    | CCSD    |                                                |
|   |      |                | $57.96 \pm 0.05$  | --       | CCSD(T) |                                                |
|   |      | $^1S_0$        | 60.45             | 4.60     | DHF     | 2C-DC-Gaunt-CC@dyall.acv4z@(core 50)[vir 278]  |
|   |      |                | 55.69             | -3.63    | MP2     |                                                |
|   |      |                | $57.75 \pm 0.06$  | -0.08    | CCSD    |                                                |
|   |      |                | $57.79 \pm 0.06$  | --       | CCSD(T) |                                                |
|   |      | $^1S_0$        | 60.60             | 4.65     | DHF     | <b>4C-DC-CC@dyall.acv4z@(core 50)[vir 278]</b> |
|   |      |                | 55.78             | -3.67    | MP2     |                                                |
|   |      |                | $57.86 \pm 0.06$  | -0.07    | CCSD    |                                                |
|   |      |                | $57.90 \pm 0.06$  | --       | CCSD(T) |                                                |

### S3 Summary of most accurate results using Eq. (S3)



Table S17: Static dipole polarizabilities (in a.u.) with non-relativistic (NR), scalar-relativistic (SR), and full Dirac-Coulomb (DC) relativistic effects for main-group elements. The error due to the numerical fitting procedure ( $\Delta P_{\text{fitting}}$ ) is included as the error bar, compared to the counterparts from Ref. 4.

| $\hat{H}$       | State                  | Period<br>Method | 1  | 2                | 3                 | 4                 | 5                 | 6                 | 7                 |
|-----------------|------------------------|------------------|----|------------------|-------------------|-------------------|-------------------|-------------------|-------------------|
|                 |                        | <b>Group 1</b>   | -- | <b>Li</b>        | <b>Na</b>         | <b>K</b>          | <b>Rb</b>         | <b>Cs</b>         | <b>Fr</b>         |
| NR              | $^2S$                  | CCSD(T)          | -- | 164.35           | $164.25 \pm 0.04$ | $294.69 \pm 0.13$ | $344.06 \pm 0.09$ | $479.16 \pm 0.67$ | $548.49 \pm 1.06$ |
| SR              | $^2S$                  | CCSD(T)          | -- | 164.30           | $163.26 \pm 0.04$ | $289.16 \pm 0.12$ | $318.99 \pm 0.05$ | $400.77 \pm 0.52$ | $322.01 \pm 0.41$ |
| DC              | $^2S_{1/2}$            | CCSD(T)          | -- | 164.30           | $163.35 \pm 0.02$ | $289.40 \pm 0.20$ | $319.08 \pm 0.17$ | $400.60 \pm 0.37$ | $319.16 \pm 0.30$ |
| Ref. 4          | --                     | --               | -- | 164.11           | $162.7 \pm 0.5$   | $289.7 \pm 0.3$   | $319.8 \pm 0.3$   | $400.9 \pm 0.7$   | $317.8 \pm 2.4$   |
|                 |                        | <b>Group 2</b>   | -- | <b>Be</b>        | <b>Mg</b>         | <b>Ca</b>         | <b>Sr</b>         | <b>Ba</b>         | <b>Ra</b>         |
| NR              | $^1S$                  | CCSD(T)          | -- | $37.87 \pm 0.01$ | $71.76 \pm 0.02$  | $160.76 \pm 0.07$ | $211.00 \pm 0.11$ | $318.74 \pm 0.17$ | $381.38 \pm 0.21$ |
| SR              | $^1S$                  | CCSD(T)          | -- | $37.85 \pm 0.01$ | $71.42 \pm 0.02$  | $158.46 \pm 0.07$ | $199.15 \pm 0.11$ | $276.31 \pm 0.19$ | $250.50 \pm 0.23$ |
| DC              | $^1S_0$                | CCSD(T)          | -- | $37.85 \pm 0.01$ | $71.40 \pm 0.02$  | $158.41 \pm 0.07$ | $199.00 \pm 0.11$ | $275.84 \pm 0.19$ | $248.40 \pm 0.22$ |
| Ref. 4          | --                     | --               | -- | $37.74 \pm 0.03$ | $71.2 \pm 0.4$    | $160.8 \pm 4$     | $197.2 \pm 0.2$   | $272.9 \pm 10$    | $246.0 \pm 4$     |
|                 |                        | <b>Group 13</b>  | -- | <b>B</b>         | <b>Al</b>         | <b>Ga</b>         | <b>In</b>         | <b>Tl</b>         | <b>Nh</b>         |
| NR              | $^2P$                  | CCSD(T)          | -- | $20.81 \pm 0.04$ | $64.00 \pm 0.89$  | $53.20 \pm 0.05$  | $69.83 \pm 0.07$  | $89.53 \pm 2.03$  | $108.61 \pm 2.10$ |
| SR <sub>n</sub> | $^2P$                  | CCSD(T)          | -- | $20.80 \pm 0.03$ | $64.12 \pm 0.82$  | $52.88 \pm 0.06$  | $67.79 \pm 0.08$  | $85.97 \pm 2.16$  | $83.07 \pm 0.17$  |
| SR <sub>d</sub> | $^2P$                  | CCSD(T)          | -- | $20.80 \pm 0.03$ | $64.12 \pm 0.82$  | $52.56 \pm 0.06$  | $67.76 \pm 0.08$  | $86.32 \pm 2.33$  | $83.40 \pm 0.17$  |
| DC              | $^2P_{1/2}$            | CCSD(T)          | -- | --               | $56.74 \pm 0.26$  | $51.98 \pm 0.08$  | $62.80 \pm 0.07$  | $51.60 \pm 0.05$  | $32.74 \pm 0.02$  |
|                 |                        | MRCISD           | -- | $21.50 \pm 0.09$ | $62.03 \pm 0.36$  | $51.76 \pm 0.09$  | $63.77 \pm 0.07$  | $51.72 \pm 0.04$  | $28.00 \pm 0.02$  |
|                 | $^2P_{3/2}$            | MRCISD           | -- | $19.85 \pm 0.06$ | $56.43 \pm 0.19$  | $52.90 \pm 0.01$  | $71.11 \pm 0.05$  | $83.03 \pm 0.13$  | $133.76 \pm 0.40$ |
|                 | $^2P_{3/2}, M_J = 1/2$ | MRCISD           | -- | $21.23 \pm 0.09$ | $63.42 \pm 0.27$  | 63.60             | $85.62 \pm 0.07$  | $108.67 \pm 0.18$ | $195.68 \pm 0.56$ |
|                 | $^2P_{3/2}, M_J = 3/2$ | MRCISD           | -- | 18.47            | $49.44 \pm 0.01$  | $42.21 \pm 0.01$  | $56.59 \pm 0.02$  | $57.38 \pm 0.03$  | $71.84 \pm 0.05$  |
| Ref. 4          | --                     | --               | -- | $20.5 \pm 1$     | $57.8 \pm 1.0$    | $50.3 \pm 3$      | $65 \pm 4$        | $50.0 \pm 2$      | $29.2 \pm 2$      |
|                 |                        | <b>Group 14</b>  | -- | <b>C</b>         | <b>Si</b>         | <b>Ge</b>         | <b>Sn</b>         | <b>Pb</b>         | <b>Fl</b>         |
| NR              | $^3P$                  | CCSD(T)          | -- | $11.75 \pm 0.01$ | $38.19 \pm 0.09$  | $39.89 \pm 0.03$  | $55.66 \pm 0.03$  | $66.30 \pm 0.31$  | $84.10 \pm 0.47$  |
| SR <sub>n</sub> | $^3P$                  | CCSD(T)          | -- | $11.74 \pm 0.01$ | $38.24 \pm 0.08$  | $39.73 \pm 0.02$  | $54.51 \pm 0.04$  | $63.24 \pm 0.34$  | $80.18 \pm 0.59$  |
| SR <sub>d</sub> | $^3P$                  | CCSD(T)          | -- | $11.74 \pm 0.01$ | $38.24 \pm 0.08$  | $39.79 \pm 0.01$  | $54.54 \pm 0.02$  | $63.24 \pm 0.34$  | $80.18 \pm 0.59$  |
| DC              | $^3P_0$                | CCSD(T)          | -- | 11.73            | $37.10 \pm 0.01$  | $39.30 \pm 0.01$  | $52.17 \pm 0.02$  | $46.73 \pm 0.02$  | $30.83 \pm 0.01$  |
| Ref. 4          | --                     | --               | -- | $11.3 \pm 0.2$   | $37.3 \pm 0.7$    | $40.0 \pm 1$      | $53.0 \pm 6$      | $47.0 \pm 3$      | $31.0 \pm 4$      |
|                 |                        | <b>Group 15</b>  | -- | <b>N</b>         | <b>P</b>          | <b>As</b>         | <b>Sb</b>         | <b>Bi</b>         | <b>Mc</b>         |
| NR              | $^4S$                  | CCSD(T)          | -- | 7.26             | $25.17 \pm 0.02$  | 29.85             | 43.83             | $52.39 \pm 0.08$  | $65.88 \pm 0.15$  |
| SR <sub>n</sub> | $^4S$                  | CCSD(T)          | -- | 7.26             | $25.19 \pm 0.02$  | 29.72             | 43.01             | $49.94 \pm 0.08$  | $63.22 \pm 0.16$  |
| SR <sub>d</sub> | $^4S$                  | CCSD(T)          | -- | 7.29             | $25.42 \pm 0.02$  | 29.64             | $43.12 \pm 0.01$  | $50.12 \pm 0.09$  | $63.57 \pm 0.18$  |
| DC              | $^4S_{3/2}$            | MRCISD           | -- | 7.20             | 24.85             | 29.01             | 42.04             | $46.68 \pm 0.01$  | $69.36 \pm 0.08$  |
|                 | $^4S_{3/2}, M_J = 1/2$ | MRCISD           | -- | 7.20             | 24.85             | 29.03             | $42.29 \pm 0.01$  | $51.60 \pm 0.01$  | $98.64 \pm 0.12$  |
|                 | $^4S_{3/2}, M_J = 3/2$ | MRCISD           | -- | 7.20             | 24.85             | 28.99             | 41.79             | 41.76             | 40.09             |
| Ref. 4          | --                     | --               | -- | $7.4 \pm 0.2$    | $25.0 \pm 1$      | $30 \pm 1$        | $43 \pm 2$        | $48 \pm 4$        | $71.0 \pm 20$     |
|                 |                        | <b>Group 16</b>  | -- | <b>O</b>         | <b>S</b>          | <b>Se</b>         | <b>Te</b>         | <b>Po</b>         | <b>Lv</b>         |
| NR              | $^3P$                  | CCSD(T)          | -- | 5.16             | $19.41 \pm 0.02$  | $25.41 \pm 0.04$  | $38.37 \pm 0.04$  | $45.89 \pm 0.01$  | $60.01 \pm 0.10$  |
| SR <sub>n</sub> | $^3P$                  | CCSD(T)          | -- | 5.16             | $19.44 \pm 0.02$  | $25.40 \pm 0.03$  | $37.94 \pm 0.01$  | $45.11 \pm 0.06$  | $58.40 \pm 0.10$  |
| SR <sub>d</sub> | $^3P$                  | CCSD(T)          | -- | 5.17             | $19.59 \pm 0.02$  | $25.37 \pm 0.02$  | $38.04 \pm 0.02$  | $45.27 \pm 0.06$  | $58.64 \pm 0.11$  |
| DC              | $^3P_2$                | MRCISD           | -- | 5.13             | 19.10             | 24.50             | 36.62             | $43.29 \pm 0.01$  | $72.04 \pm 0.03$  |
|                 | $^3P_2, M_J = 0$       | MRCISD           | -- | 5.42             | 20.24             | 25.90             | 38.05             | $43.92 \pm 0.01$  | $68.87 \pm 0.04$  |
|                 | $^3P_2, M_J = 1$       | MRCISD           | -- | 4.84             | 17.95             | 23.09             | 35.19             | $42.68 \pm 0.01$  | $75.28 \pm 0.03$  |
|                 | $^3P_2, M_J = 2$       | MRCISD           | -- | 5.28             | 19.67             | 25.20             | 37.33             | $43.60 \pm 0.01$  | $70.38 \pm 0.03$  |
| Ref. 4          | --                     | --               | -- | $5.3 \pm 0.2$    | $19.4 \pm 0.1$    | $28.9 \pm 1.0$    | $38.0 \pm 4$      | $44.0 \pm 4$      | --                |
|                 |                        | <b>Group 17</b>  | -- | <b>F</b>         | <b>Cl</b>         | <b>Br</b>         | <b>I</b>          | <b>At</b>         | <b>Ts</b>         |
| NR              | $^2P$                  | CCSD(T)          | -- | 3.60             | 14.58             | $20.62 \pm 0.03$  | $32.46 \pm 0.23$  | $39.85 \pm 0.02$  | $50.50 \pm 0.02$  |

Continued on next page

Table S17: Static dipole polarizabilities (in a.u.) with non-relativistic (NR), scalar-relativistic (SR), and full Dirac-Coulomb (DC) relativistic effects for main-group elements. The error due to the numerical fitting procedure ( $\Delta P_{\text{fitting}}$ ) is included as the error bar, compared to the counterparts from Ref. 4.

| $\hat{H}$       | State                  | Period<br>Method | 1         | 2               | 3              | 4                | 5                | 6                | 7                 |
|-----------------|------------------------|------------------|-----------|-----------------|----------------|------------------|------------------|------------------|-------------------|
| SR <sub>n</sub> | $^2P$                  | CCSD(T)          | --        | 3.61            | 14.61          | $20.67 \pm 0.05$ | $32.01 \pm 0.01$ | $38.77 \pm 0.02$ | $50.16 \pm 0.06$  |
| SR <sub>d</sub> | $^2P$                  | CCSD(T)          | --        | 3.61            | 14.72          | $20.60 \pm 0.04$ | $32.08 \pm 0.01$ | $38.86 \pm 0.03$ | $50.34 \pm 0.06$  |
| DC              | $^2P_{3/2}$            | MRCISD           | --        | 3.57            | 14.36          | 20.06            | 31.29            | 38.96            | 65.17             |
|                 | $^2P_{3/2}, M_J = 3/2$ | MRCISD           | --        | 3.70            | 14.94          | 20.96            | 32.66            | 41.64            | 71.92             |
|                 | $^2P_{3/2}, M_J = 1/2$ | MRCISD           | --        | 3.43            | 13.78          | 19.16            | 29.93            | 36.27            | 58.42             |
|                 | $^2P_{1/2}, M_J = 1/2$ | MRCISD           | --        | 3.57            | 14.40          | 20.28            | 32.02            | 40.82            | $227.38 \pm 0.01$ |
| Ref. 4          | --                     | --               | --        | $3.74 \pm 0.08$ | $14.6 \pm 0.1$ | $21.0 \pm 1$     | $32.9 \pm 1.3$   | $42.0 \pm 4$     | $76.0 \pm 15$     |
|                 |                        | <b>Group 18</b>  | <b>He</b> | <b>Ne</b>       | <b>Ar</b>      | <b>Kr</b>        | <b>Xe</b>        | <b>Rn</b>        | <b>Og</b>         |
| NR              | $^1S$                  | CCSD(T)          | 1.38      | 2.57            | 11.01          | 16.78            | 27.23            | 34.08            | 45.28             |
| SR              | $^1S$                  | CCSD(T)          | 1.38      | 2.57            | 11.03          | 16.77            | 27.02            | 33.13            | 43.77             |
| DC              | $^1S_0$                | CCSD(T)          | 1.38      | 2.57            | 11.02          | 16.80            | 27.20            | 35.08            | $57.90 \pm 0.06$  |
| Ref. 4          | --                     | --               | 1.38      | 2.66            | 11.08          | $16.78 \pm 0.02$ | $27.32 \pm 0.2$  | $35.0 \pm 2$     | $58.0 \pm 6$      |

## S4 Comparison with literature

### S4.1 Group 1 elements

The most accurate theoretical and experimental values for the entire periodic table have been summarized in Refs. 4 and 5. These values for Group 1 elements are collected in Table S18 to validate the results in this work. Only computational and experimental values close to the recommended values in Ref. 4 are compared.

The DC result ( $164.31 \pm 0.01$ ) for Li aligns closely with experimental results ( $164.0 \pm 3.4^6$  and  $164.2 \pm 1.1^7$ ). The most accurate computational value ( $164.1125 \pm 0.0005^8$ ) is taken as the recommended value in Ref. 4. The difference between the recommended value and the result in this work is only 0.12%, which could be attributed to the absence of other relativistic effects, such as Breit or QED. It should be noted that the full relativistic contribution to  $\alpha$  is  $-0.07$  a.u. at both the DHF and CCSD levels, as shown in Table S1, which agrees with the value ( $-0.07$  a.u.) obtained by Lim *et al.* at the DHF level.<sup>9</sup>

For Na, the deviation between the DC result ( $163.27 \pm 0.09$ ) and the recommended value

( $162.7 \pm 0.5$ ) in Ref. 4, based on the experimental result by Ekstrom *et al.*, is less than 0.36%.<sup>10</sup> Notably, the lower bound of the DC result is slightly larger than the upper bound of both the recommended value and another experimental value ( $162.7 \pm 0.1$ ) reported by Holmgren *et al.*<sup>11</sup> However, the DC result for Na ( $163.27 \pm 0.09$ ) is close to the experimental value ( $161 \pm 7.5$ ) reported by Ma *et al.*<sup>12</sup> Additionally, the DC result is slightly larger than the recommended computational value (162.88) in Refs. 13,14, obtained using a composite scheme by Thakkar and Lupinetti. The NR and SR values of Na (163.98 and 162.99, respectively) in this work are in good agreement with the computational values of 163.90 and 162.90, respectively, as reported by Thakkar and Lupinetti.<sup>13,14</sup> Therefore, the primary difference between the DC value and the final recommended value in Refs. 13,14 lies in the method of incorporating the SOC contribution to  $\alpha$ . Specifically, in Refs. 13,14, a value of  $-0.02$  a.u. evaluated at the DHF level from Ref. 9 is used as the SOC contribution and is added to the SR value. In contrast, this work evaluates the SOC contribution as  $+0.28$  a.u. at the CCSD(T) level. It should be noted that in this study, the SOC contributions at the DHF and CCSD levels are  $-0.04$  and  $-0.03$  a.u., respectively. Furthermore, this study shows that the NR value also agrees well with the recent non-relativistic CCSD(T) value obtained by Smiałkowski and Tomza (163.9 a.u.) at CCSD(T)/aug-cc-pwCV5Z,<sup>15</sup> suggesting the reliability of the method used in this work.

For K, the lower bound of the DC value ( $290.64 \pm 0.24$ ) is slightly higher than the upper bound of the recommended value ( $289.7 \pm 0.3$ ),<sup>4</sup> which is based on experimental values.<sup>16,17</sup> However, the DC CCSD(T) value obtained using Eq. (S3) is  $289.40 \pm 0.20$ , as shown in Table S9, which agrees well with the recommended value in Ref. 4. Therefore, one reason for the discrepancy could be that a negative  $\gamma$  obtained from Eq. (S1) is invalid, which is observed when  $\tau > 0.1\%$  is used in Eq. (S4).

Moreover, the DC value ( $290.64 \pm 0.24$ ) is in good agreement with other experimental values ( $292.9 \pm 6.1$ <sup>6</sup> and  $290.6 \pm 1.4$ <sup>11</sup>). Compared to the computational values, the DC result is slightly higher than the RLCCSD value (289.1),<sup>18</sup> where the linear approximation CCSD

method is used. Additionally, the DC value ( $290.64 \pm 0.24$ ) agrees well with the recent result ( $290.30 \pm 0.23$ ) computed by the relativistic all-order method.<sup>19</sup>

The SR result (289.96) is in good agreement with the DK-CCSD(T) result ( $291.1 \pm 1.5$ ) reported by Lim *et al.* using all-electron calculations.<sup>20</sup> Furthermore, the SR value (289.96) is also close to the recent result (289.6) computed by CCSD(T) with relativistic energy-consistent pseudopotentials (ECP).<sup>15</sup>

The most accurate DC value for Rb in this work is  $320.08 \pm 0.29$  a.u., which is in good agreement with previous experiments ( $319 \pm 6$ ,<sup>6</sup>  $318.8 \pm 1.4$ ,<sup>11</sup>  $319.8 \pm 0.3$ ,<sup>16,17</sup>  $319.2 \pm 6.1$ <sup>13</sup>) and the recommended value ( $319.8 \pm 0.3$ ).<sup>4</sup> The DC value is generally higher than recent values ( $318.5 \pm 0.6$ ,<sup>21</sup>  $318.38 \pm 0.38$ <sup>19</sup>) obtained by the relativistic all-order method and its variants, but it is in good agreement with the latest result ( $319.5 \pm 1.5$ ),<sup>22</sup> which includes other relativistic effects, e.g., Breit and QED, etc. It should be noted that the DC value obtained using Eq. (S3) is  $319.08 \pm 0.17$ , which is less than the recommended value in Ref. 4. This suggests that a more accurate  $\gamma$  should be used to obtain  $\alpha$  for Rb. Moreover, the SR value ( $319.34 \pm 0.01$ ) is slightly larger than the latest result (317.4) computed by scalar-relativistic CCSD(T) with the ECP method.<sup>15</sup>

The DC value for Cs ( $398.24 \pm 0.34$ ) is slightly lower than the value from previous theoretical work, which was 399.0, reported by Borschevsky *et al.*,<sup>23</sup> computed using the CCSD(T) method with the Fægri basis set.<sup>24</sup> The discrepancy could be attributed to the different basis set and fitting procedure used in this study. To study the impact of basis sets, I used the same Fægri set as in Ref. 23. The virtual orbitals with energies above 40 a.u. were omitted instead of 50 a.u. in the previous work to reduce computational cost. It should be noted that five data points were used to fit  $\alpha$  defined in Eq. (S1) using the least-squares procedure, instead of the three data points used with numerical differentiation in Ref. 23. The result ( $399.52 \pm 0.62$  a.u.), as shown in Table S1, was closer to 399.0 in Ref. 23. It is also in excellent agreement with the recent results ( $399.9 \pm 0.6$ <sup>21</sup> and  $399.74 \pm 0.55$ <sup>19</sup>) computed by relativistic all-order methods. When Eq. (S3) is used, the results from the least-squares

procedure are  $400.51 \pm 0.2$  and  $400.60 \pm 0.37$  a.u. for the Fægri and s-aug-ANO-RCC basis sets, respectively. These results are closer to the recommended value ( $400.9 \pm 0.7$  a.u.) from Ref. 4 compared to those obtained by fitting Eq. (S1). The larger difference in DC CCSD(T) values obtained with s-aug-ANO-RCC between using Eqs. (S1) and (S3) can be attributed to a larger  $\gamma$  obtained compared to the Fægri basis. Therefore, simply removing  $\gamma$  and higher-order contributions in Eq. (S3) could lead to a higher numerical error for Cs. Surprisingly, this error is even as significant as the SOC contribution to  $\alpha$ , as shown in Table 1. The SR value ( $397.40 \pm 0.02$ ) in this work is much higher than the result (391) obtained by scalar-relativistic CCSD(T) with the ECP method.<sup>15</sup> One reason could be the pseudopotential used to account for the scalar-relativistic effect in Ref. 15.

The DC value of Fr ( $317.40 \pm 0.57$ ) is in excellent agreement with the recommended value ( $317.8 \pm 2.4$ ) reported in Ref. 4 and the recent computational values ( $317.1 \pm 1.3$ ,<sup>25</sup>  $316.6 \pm 2.4$ ,<sup>26</sup>  $316.6 \pm 1.5$ <sup>19</sup>) using the relativistic all-order method and its variants. There is a significant difference between the results of the current work and those reported in Ref. 23, where the Fægri basis set and fewer data points were used. To investigate this discrepancy, I chose the same data points as in Ref. 23 and fitted Eq. S3. The resulting value is 318.34, which is still much larger than the value reported in Ref. 23. Therefore, the primary reason for this discrepancy could be the different basis functions used in the two studies.

Table S18: Summary of reference atomic dipole polarizabilities (in a.u.) for Group 1 elements, as reported in Refs. 4 and 5. Comment definitions are provided in these references.

| Z  | Atom | Refs.   | State       | $\alpha$              | Year | Comments                                                             |
|----|------|---------|-------------|-----------------------|------|----------------------------------------------------------------------|
| 3  | Li   | [ 6]    | $^2S_{1/2}$ | $164.0 \pm 3.4$       | 1974 | exp.                                                                 |
|    |      | [ 9,27] | $^2S$       | 164.05                | 2001 | NR, exponentially correlated Gaussians [ 28] + R/DK                  |
|    |      | [ 7]    | $^2S_{1/2}$ | $164.2 \pm 1.1$       | 2006 | exp.                                                                 |
|    |      | [ 29]   | $^2S_{1/2}$ | 164.21                | 2007 | Frozen core Hamiltonian, semi-empirical polarisation potential       |
|    |      | [ 30]   | $^2S_{1/2}$ | 164.084               | 2008 | R, Dirac, MBPT, Breit, QED, recoil ( $^7\text{Li}$ )                 |
|    |      | [ 8]    | $^2S_{1/2}$ | $164.1125 \pm 0.0005$ | 2011 | Hylleraas basis, RMW + Darwin + Breit, QED, recoil ( $^7\text{Li}$ ) |
|    |      | [ 4]    | $^2S_{1/2}$ | $164.1125 \pm 0.0005$ | 2019 | recommended                                                          |
|    |      | [ 15]   | $^2S_{1/2}$ | 164.2                 | 2021 | NR, CCSD(T)                                                          |
|    |      | [ 19]   | $^2S_{1/2}$ | $162.00 \pm 0.24$     | 2022 | R, Dirac-HF, perturbative singles + doubles method, RPA              |
| 11 | Na   | [ 31]   | $^2S_{1/2}$ | $165.0 \pm 0.1$       | 2024 | NR, neural network QMC, DS (DeepSolid) method                        |
|    |      | [ 10]   | $^2S_{1/2}$ | $162.7 \pm 0.5$       | 1995 | exp.                                                                 |
|    |      | [ 18]   | $^2S_{1/2}$ | $162.6 \pm 0.3$       | 1999 | R, SD all orders + exp. data                                         |

Continued on next page

| Z  | Atom | Refs.    | State       | $\alpha$                  | Year | Comments                                                             |
|----|------|----------|-------------|---------------------------|------|----------------------------------------------------------------------|
| 19 | K    | [ 13,14] | $^2S_{1/2}$ | $162.88 \pm 0.60$         | 2006 | R, CCSD(T)                                                           |
|    |      | [ 11]    | $^2S_{1/2}$ | $162.7 \pm 0.1 / \pm 1.2$ | 2010 | exp.                                                                 |
|    |      | [ 12]    | $^2S_{1/2}$ | $161 \pm 7.5$             | 2015 | exp.                                                                 |
|    |      | [ 4]     | —           | $162.7 \pm 0.5$           | 2019 | recommended                                                          |
|    |      | [ 15]    | $^2S_{1/2}$ | 163.9                     | 2021 | NR, CCSD(T)                                                          |
|    |      | [ 19]    | $^2S_{1/2}$ | $162.44 \pm 0.16$         | 2022 | R, Dirac-HF, perturbative singles + doubles method, RPA              |
|    |      | [ 6]     | $^2S_{1/2}$ | $292.9 \pm 6.1$           | 1974 | exp.                                                                 |
|    |      | [ 18]    | $^2S_{1/2}$ | 289.1                     | 1999 | RLCCSD                                                               |
|    |      | [ 18]    | $^2S_{1/2}$ | $290.2 \pm 0.8$           | 1999 | R, SD all orders + exp. data for electronic transitions              |
|    |      | [ 32]    | $^2S_{1/2}$ | 290.0                     | 2003 | Combination of ab initio and semi-empirical methods                  |
|    |      | [ 20]    | $^2S$       | $291.1 \pm 1.5$           | 2005 | R, DK, CCSD(T), AE                                                   |
|    |      | [ 33]    | $^2S_{1/2}$ | 290.2                     | 2010 | Combination of theoretical and experimental data                     |
|    |      | [ 11]    | $^2S_{1/2}$ | $290.6 \pm 1.4$           | 2010 | exp. (for hyperfine effects see ref [ 34])                           |
|    |      | [ 34]    | $^2S_{1/2}$ | 290.05                    | 2013 | Oscillator-strength sum rule                                         |
|    |      | [ 16,17] | $^2S_{1/2}$ | $289.7 \pm 0.3$           | 2016 | exp.                                                                 |
| 37 | Rb   | [ 4]     | —           | $289.7 \pm 0.3$           | 2019 | recommended                                                          |
|    |      | [ 15]    | $^2S_{1/2}$ | 289.6                     | 2021 | SR, CCSD(T), ECP                                                     |
|    |      | [ 19]    | $^2S_{1/2}$ | $290.30 \pm 0.23$         | 2022 | R, Dirac-HF, perturbative singles + doubles method, RPA              |
|    |      | [ 6]     | $^2S_{1/2}$ | $319 \pm 6$               | 1974 | exp.                                                                 |
|    |      | [ 32]    | $^2S$       | 315.7                     | 2003 | Combination of ab initio and semi-empirical methods                  |
|    |      | [ 20]    | $^2S$       | $316.2 \pm 3.2$           | 2005 | R, DK, CCSD(T), AE                                                   |
|    |      | [ 13]    | $^2S_{1/2}$ | $319.2 \pm 6.1$           | 2006 | exp.                                                                 |
|    |      | [ 18,33] | $^2S_{1/2}$ | $318.6 \pm 0.6$           | 2010 | R, SD all orders + exp. data                                         |
|    |      | [ 11]    | $^2S_{1/2}$ | $318.8 \pm 1.4$           | 2010 | exp.                                                                 |
|    |      | [ 35]    | $^2S$       | 317.0                     | 2015 | Oscillator-strength sum rule                                         |
|    |      | [ 16,17] | $^2S_{1/2}$ | $319.8 \pm 0.3$           | 2016 | exp.                                                                 |
|    |      | [ 4]     | —           | $319.8 \pm 0.3$           | 2019 | recommended                                                          |
|    |      | [ 15]    | $^2S_{1/2}$ | 317.4                     | 2021 | SR, CCSD(T), ECP                                                     |
|    |      | [ 21]    | $^2S_{1/2}$ | $318.5 \pm 0.6$           | 2022 | R, DHF, all orders                                                   |
|    |      | [ 19]    | $^2S_{1/2}$ | $318.38 \pm 0.38$         | 2022 | R, Dirac-HF, perturbative singles + doubles method, RPA              |
| 55 | Cs   | [ 22]    | $^2S_{1/2}$ | $319.5 \pm 1.5$           | 2023 | R, TDHF + Breit + QED + scaling<br>+ structure radiation + normaliz. |
|    |      | [ 18]    | $^2S_{1/2}$ | $399.9 \pm 1.9$           | 1999 | R, Dirac, SD, all orders + exp. data                                 |
|    |      | [ 18]    | $^2S_{1/2}$ | 401.5                     | 1999 | R, SD all orders + exp. data for electronic transitions              |
|    |      | [ 36]    | $^2S_{1/2}$ | $401.0 \pm 0.6$           | 2003 | exp.                                                                 |
|    |      | [ 37]    | $^2S_{1/2}$ | $398.2 \pm 0.9$           | 2004 | R, Dirac, SDpT                                                       |
|    |      | [ 20]    | $^2S$       | $396.0 \pm 5.9$           | 2005 | R, DK, CCSD(T), AE                                                   |
|    |      | [ 38]    | $^2S_{1/2}$ | $398.4 \pm 0.7$           | 2008 | R, DF, RPA, SD-all order                                             |

Continued on next page

| Z  | Atom | Refs.    | State       | $\alpha$          | Year | Comments                                                |
|----|------|----------|-------------|-------------------|------|---------------------------------------------------------|
| 87 | Fr   | [ 33]    | $^2S_{1/2}$ | 399.8             | 2010 | Combination of theoretical and experimental data        |
|    |      | [ 23]    | $^2S_{1/2}$ | 399.0             | 2013 | R, Dirac, CCSD(T)                                       |
|    |      | [ 35]    | $^2S_{1/2}$ | $396.7 \pm 7.9$   | 2015 | Combination of theoretical and experimental data        |
|    |      | [ 39]    | $^2S_{1/2}$ | $399.5 \pm 0.8$   | 2016 | R, Dirac, RCC-SD                                        |
|    |      | [ 16,17] | $^2S_{1/2}$ | $400.8 \pm 0.4$   | 2016 | exp.                                                    |
|    |      | [ 4]     | --          | $400.9 \pm 0.7$   | 2019 | recommended                                             |
|    |      | [ 15]    | $^2S_{1/2}$ | 391.1             | 2021 | SR, CCSD(T), ECP                                        |
|    |      | [ 21]    | $^2S_{1/2}$ | $399.9 \pm 0.6$   | 2022 | R, DHF, all order                                       |
|    |      | [ 19]    | $^2S_{1/2}$ | $399.74 \pm 0.55$ | 2022 | R, Dirac-HF, perturbative singles + doubles method, RPA |
|    |      | [ 20]    | $^2S$       | 315.2             | 2005 | R, DK, CCSD(T), AE                                      |
|    |      | [ 40]    | $^2S_{1/2}$ | 313.7             | 2007 | R, DF, RPA, MBPT                                        |
|    |      | [ 18,33] | $^2S_{1/2}$ | $317.8 \pm 2.4$   | 2010 | R, Dirac, SD all orders + experimental data             |
|    |      | [ 23]    | $^2S_{1/2}$ | 311.5             | 2013 | R, Dirac, CCSD(T)                                       |
|    |      | [ 41]    | $^2S_{1/2}$ | 317.8             | 2016 | LR-CCSD                                                 |
|    |      | [ 42]    | $^2S_{1/2}$ | 316.8             | 2016 | R, Dirac-Fock, CCSD(T)                                  |
|    |      | [ 4]     | --          | $317.8 \pm 2.4$   | 2019 | recommended                                             |
|    |      | [ 25]    | $^2S_{1/2}$ | $317.1 \pm 1.3$   | 2021 | R, Dirac-HF, CCSD                                       |
|    |      | [ 15]    | $^2S_{1/2}$ | 325.8             | 2021 | SR, CCSD(T), ECP                                        |
|    |      | [ 26]    | $^2S_{1/2}$ | $316.6 \pm 2.4$   | 2022 | R, all orders, Dirac-Fock, RPA                          |
|    |      | [ 19]    | $^2S_{1/2}$ | $316.6 \pm 1.5$   | 2022 | R, Dirac-HF, perturbative singles + doubles method, RPA |

## S4.2 Group 2 elements

The most accurate theoretical and experimental values for the entire periodic table have been summarized in Refs. 4 and 5. These values for Group 2 elements are collected in Table S19 to validate the results in this work. Only computational and experimental values close to the recommended values in Ref. 4 are compared.

The DC result (37.78) with CCSD(T) for Be aligns closely with recent computational theoretical values ( $37.73 \pm 0.04$ <sup>35,43</sup> and  $37.787$ <sup>44</sup>) computed by the relativistic configuration interaction plus core polarization (RCICP) method, as well as the result ( $37.76 \pm 0.22$ ) obtained by CI+MBPT2 with experimental data.<sup>45</sup> The DC CCSD value (37.94), as shown in Table S2, is also in good agreement with the results ( $37.80 \pm 0.47$ <sup>46</sup> and  $37.86 \pm 0.17$ <sup>47</sup>) obtained by relativistic CCSD. The most accurate SR and NR values (37.79 and 37.80) in

this work are both higher than the corresponding results (37.69 and 37.71) in Ref. 48, where CCSD(T) calculations were performed at the complete basis set limit, suggesting that the difference could be mainly attributed to the finite basis sets used in this work. Additionally, the NR value is also close to other computational values (37.755,<sup>27</sup> 37.75,<sup>48</sup> 37.7,<sup>15</sup> and  $37.58 \pm 0.03$ <sup>31</sup>) in the literature. The DC relativistic contribution to  $\alpha$  is  $-0.018$  a.u., which is in excellent agreement with the value  $-0.016$  a.u., as a correction added to the NR value, as shown in Table S19. There are no experimental values available for Be in the literature yet.

The SR and NR values (71.20 and 71.54) for magnesium (Mg,  $Z = 12$ ) are in excellent agreement with the CCSD(T) results (71.15 and 71.63) at the complete basis set limit in Ref. 49, where “0” in X2C-0/NR-0 means all electrons are correlated. This suggests that the basis set used in this work for Mg is sufficient to provide an accurate  $\alpha$ . With the same basis sets, the DC value (71.19) agrees well with the recommended value ( $71.2 \pm 0.4$ ) in Ref. 4. Additionally, the DC value also aligns with all experimental values and is close to all other computational values in Table S19.

The SR and NR values (157.61 and 159.90) of calcium (Ca,  $Z = 20$ ) are in excellent agreement with the CCSD(T) results (157.61 and 159.81) at the complete basis set limit reported in Ref. 49. In this context, “10” in X2C-10/NR-10, as shown in Table S19, indicates that 10 core electrons are treated using ECP. This suggests that the basis set used in this work for Ca is sufficient to provide an accurate  $\alpha$ . With the same basis sets, the DC value (157.55) agrees well with the recommended value ( $160.8 \pm 4$ ) in Ref. 4. Lim *et al.* computed DC and SR values for alkaline-earth-metal elements from Ca to Ra using a similar procedure as in this work. However, the basis set used for Ca in their work is (32s22p10d9f6g), which is much larger than the largest basis set (20s15p8d5f) in Ref. 50. Additionally, larger basis sets are also employed for atoms from Sr to Ra in this work compared to Ref. 50. The SOC contribution to  $\alpha$  is evaluated at the MBPT2 level in Ref. 50, while the corresponding values at CCSD and CCSD(T) levels are also available in this work, as shown in Table S2. This



gives confidence that the DC value obtained in this work is more accurate than the value reported in Ref. 50.

The DC value ( $197.67 \pm 0.01$ ) of Sr is slightly higher than the upper bound of the recommended value ( $197.2 \pm 0.2$ ) from Ref. 4, corresponding to the computational values in Refs. 33,45, where a hybrid relativistic CI and MBPT method is used. The difference could be attributed to the higher-order correlation contributions included in this work. In general, the DC/SR values ( $197.67/197.82$ ) are close to all experimental values and computational values listed in Table S19. The NR value ( $209.64 \pm 0.01$ ) with the basis set ( $34s26p16d8f6g2h$ ) also aligns with the result ( $210.64$ ) with the basis set ( $21s16p11d9f3g$ ) in Ref. 50, suggesting that the basis set used in this work is sufficient. A difference between the SR value ( $197.82$ ) and the result ( $198.62$ ) in Ref. 49 could be mainly attributed to the difference between all-electron and ECP methods.

It can be seen from Table S2 that the error bar for Ba is still large based on the recommended value ( $272.9 \pm 10$ ) in Ref. 4. The difference between the DC value ( $273.51$ ) and the CCSD(T) results ( $273 \pm 4.1^{13,50}$  and  $272.8^{51}$ ) lies within the uncertainty range suggested by Ref. 4. It should be noted that a larger basis set ( $36s31p20d8f6g2h$ ) is employed compared to the one ( $24s22p16d12f4g1h$ ) used in Ref. 51. The Gaunt contribution ( $-0.01$  a.u.) is also studied by Borschevsky *et al.* at both the DHF and correlation stages. In addition, Dutta recently studied the trend of the Gaunt interaction contribution to  $\alpha$  for alkaline-earth elements, finding the Gaunt contribution to be  $-0.454$  a.u. at the level of 3rd-order perturbation theory.<sup>52</sup> To be conservative, the latter value is used for uncertainty estimation.

The DC value of Ra ( $245.68$ ) agrees well with the recommended value ( $246 \pm 4$ ) in Ref. 4 and the computational values ( $246.2 \pm 4.9^{13,50}$  and  $242.8^{51}$ ) obtained using a similar procedure as in this work. It should be noted that a larger basis set ( $38s35p24d16f6g2h$ ) is employed compared to the one ( $26s23p18d13f5g2h$ ) used in Ref. 51. The Gaunt contribution evaluated at the CCSD(T) level is tiny and negligible for Ra based on Ref. 51, while it is  $-1.88$  a.u. when evaluated at the level of 3rd-order perturbation theory in Ref. 52. To be conservative, the latter value is used for uncertainty estimation.

Table S19: Summary of reference atomic dipole polarizabilities (in a.u.) for Group 2 elements, as reported in Refs. 4 and 5. Comment definitions are provided in these references.

| Z  | Atom | Refs.    | State   | $\alpha$           | Year | Comments                                                |
|----|------|----------|---------|--------------------|------|---------------------------------------------------------|
| 4  | Be   | [ 53]    | $^1S_0$ | 37.29              | 1984 | All-electron SCF plus valence CI                        |
|    |      | [ 54]    | $^1S_0$ | $37.73 \pm 0.05$   | 1997 | CCSD(T)                                                 |
|    |      | [ 55]    | $^1S_0$ | 37.9               | 2000 | Model potential                                         |
|    |      | [ 27]    | $^1S$   | 37.755             | 2001 | NR, exponentially correlated Gaussians [ 28]            |
|    |      | [ 32]    | $^1S_0$ | 37.69              | 2003 | Combination of ab initio and semi-empirical methods     |
|    |      | [ 56]    | $^1S_0$ | 37.807             | 2004 | CI, expanded London formula                             |
|    |      | [ 45]    | $^1S_0$ | $37.76 \pm 0.22$   | 2006 | R, Dirac, CI + MBPT2 + experimental data                |
|    |      | [ 13,27] | $^1S_0$ | $37.739 \pm 0.030$ | 2006 | R correction of -0.016 applied to value from ref [ 27]  |
|    |      | [ 46]    | $^1S_0$ | $37.80 \pm 0.47$   | 2008 | R, Dirac, CCSD                                          |
|    |      | [ 47]    | $^1S_0$ | $37.86 \pm 0.17$   | 2013 | R, Dirac, MBPT, CCSD                                    |
|    |      | [ 35,43] | $^1S_0$ | $37.73 \pm 0.04$   | 2015 | Combination of theoretical (CICP) and experimental data |
|    |      | [ 48]    | $^1S_0$ | 37.75              | 2019 | NR, CCSD                                                |
|    |      | [ 49]    | $^1S_0$ | 37.69/37.71        | 2019 | CCSD(T), R X2C-0/NR-0                                   |
|    |      | [ 4]     | —       | $37.74 \pm 0.03$   | 2019 | recommended                                             |
|    |      | [ 15]    | $^1S_0$ | 37.7               | 2021 | NR, CCSD(T)                                             |
|    |      | [ 57]    | $^1S_0$ | 37.614             | 2021 | R, MCDHF                                                |
|    |      | [ 44]    | $^1S_0$ | 37.787             | 2023 | R, DF, CICP (CP: core polarization)                     |
|    |      | [ 31]    | $^1S_0$ | $37.58 \pm 0.03$   | 2024 | NR, neural network QMC, DS (DeepSolid) method           |
| 12 | Mg   | [ 58]    | $^1S_0$ | $71.5 \pm 3.5$     | 1973 | exp.                                                    |
|    |      | [ 59]    | $^1S$   | 71.32              | 1976 | NR, PNO-CEPA                                            |
|    |      | [ 60]    | $^1S_0$ | 70.5               | 1979 | NR, CI + pseudo-potential                               |
|    |      | [ 61]    | $^1S$   | 71.7               | 1991 | NR, MBPT4                                               |
|    |      | [ 62]    | $^1S$   | 71.8               | 1991 | NR, MBPT4                                               |
|    |      | [ 63,64] | $^1S_0$ | $75.0 \pm 3.5$     | 1995 | exp.                                                    |
|    |      | [ 18]    | $^1S_0$ | $74.9 \pm 2.7$     | 1999 | Hybrid-RCI + MBPT sum rule                              |
|    |      | [ 55]    | $^1S_0$ | 72.0               | 2000 | Model potential                                         |
|    |      | [ 65]    | $^1S_0$ | 71.4               | 2002 | CI, oscillator strength correction                      |
|    |      | [ 32]    | $^1S_0$ | 71.35              | 2003 | Combination of ab initio and semi-empirical methods     |
|    |      | [ 66]    | $^1S$   | 70.90              | 2004 | R, DK, CASPT2                                           |
|    |      | [ 45,67] | $^1S_0$ | 70.89              | 2006 | R, Dirac, CI + MBPT2 + experimental data                |
|    |      | [ 13]    | $^1S_0$ | $71.22 \pm 0.36$   | 2006 | R, DK, CCSD(T)                                          |
|    |      | [ 45]    | $^1S_0$ | 71.33              | 2006 | R, Dirac, CI + MBPT2                                    |
|    |      | [ 45]    | $^1S_0$ | $71.3 \pm 0.7$     | 2006 | R, Dirac, CI + MBPT2, recommended                       |
|    |      | [ 46]    | $^1S_0$ | $73.4 \pm 2.3$     | 2008 | R, Dirac, CCSD                                          |
|    |      | [ 68]    | $^1S_0$ | $77.6 \pm 7.8$     | 2012 | exp.                                                    |

Continued on next page

| Z  | Atom | Refs.    | State   | $\alpha$          | Year | Comments                                                               |
|----|------|----------|---------|-------------------|------|------------------------------------------------------------------------|
| 20 | Ca   | [ 47]    | $^1S_0$ | $72.54 \pm 0.50$  | 2013 | R, Dirac, MBPT, CCSD                                                   |
|    |      | [ 69]    | $^1S_0$ | 70.76             | 2014 | R, Dirac + Breit, perturbed relativistic coupled-cluster theory (PRCC) |
|    |      | [ 12]    | $^1S_0$ | $59 \pm 16$       | 2015 | exp.                                                                   |
|    |      | [ 49]    | $^1S_0$ | 71.15/71.63       | 2019 | CCSD(T), R X2C-0/NR-0                                                  |
|    |      | [ 49]    | $^1S_0$ | 71.02/71.01       | 2019 | CCSD(T), R X2C-2/NR-2                                                  |
|    |      | [ 70]    | $^1S_0$ | 73.0              | 2019 | R, KRCISD/aug-QZ                                                       |
|    |      | [ 4]     | —       | $71.2 \pm 0.4$    | 2019 | recommended                                                            |
|    |      | [ 71]    | $^1S_0$ | 71.9              | 2020 | R, MCDP                                                                |
|    |      | [ 72]    | $^1S_0$ | 72.121            | 2021 | R, CCSD(T)                                                             |
|    |      | [ 73]    | $^1S_0$ | 71.643            | 2021 | R, CCSD(T)                                                             |
|    |      | [ 15]    | $^1S_0$ | 71.5              | 2021 | NR, CCSD(T)                                                            |
|    |      | [ 74]    | $^1S_0$ | $81 \pm 17$       | 2022 | exp.                                                                   |
|    |      | [ 60]    | $^1S$   | 153.7             | 1979 | NR, CI + pseudo-potential                                              |
|    |      | [ 75]    | $^1S$   | 152.0             | 1991 | R, MVD, CCSD + T                                                       |
|    |      | [ 61]    | $^1S$   | 157               | 1991 | NR, MBPT4                                                              |
|    |      | [ 76]    | $^1S_0$ | 160               | 2002 | R, CI+MBPT                                                             |
|    |      | [ 65]    | $^1S$   | 158.6             | 2002 | CI, oscillator strength correction                                     |
|    |      | [ 32]    | $^1S$   | 159.4             | 2003 | Combination of ab initio and semi-empirical methods                    |
|    |      | [ 77]    | $^1S_0$ | 155.3/157.7       | 2003 | CCSD R/NR                                                              |
|    |      | [ 66]    | $^1S$   | 163               | 2004 | R, DK, CASPT2                                                          |
|    |      | [ 50]    | $^1S_0$ | 158.0             | 2004 | R, DK + SO, CCSD(T)                                                    |
|    |      | [ 78,79] | $^1S_0$ | $169 \pm 17$      | 2004 | exp.                                                                   |
|    |      | [ 45,67] | $^1S_0$ | 155.9             | 2006 | R, Dirac, CI + MBPT2 + experimental data                               |
|    |      | [ 45]    | $^1S_0$ | $157.1 \pm 1.3$   | 2006 | Hybrid-RCI + MBPT sum rule + experimental data                         |
|    |      | [ 45]    | $^1S_0$ | 159.0             | 2006 | R, Dirac, CI + MBPT                                                    |
|    |      | [ 13]    | $^1S_0$ | $157.9 \pm 0.8$   | 2006 | R, DK, CCSD(T)                                                         |
|    |      | [ 46]    | $^1S_0$ | 154.58            | 2008 | R, Dirac, coupled cluster                                              |
|    |      | [ 46]    | $^1S_0$ | $154.6 \pm 5.4$   | 2008 | R, Dirac, CCSD                                                         |
|    |      | [ 80]    | $^1S_0$ | 154.7             | 2008 | ab initio + experimental data                                          |
|    |      | [ 33]    | $^1S_0$ | 157.1             | 2010 | Combination of theoretical and experimental data                       |
|    |      | [ 47]    | $^1S_0$ | $157.03 \pm 0.80$ | 2013 | R, Dirac, MBPT, CCSD                                                   |
|    |      | [ 69]    | $^1S_0$ | 160.77            | 2014 | R, Dirac + Breit, perturbed relativistic coupled-cluster theory (PRCC) |
|    |      | [ 49]    | $^1S_0$ | 156.10            | 2019 | CCSD(T), ECP                                                           |
|    |      | [ 49]    | $^1S_0$ | 157.61/159.81     | 2019 | CCSD(T), R X2C-10/NR-10                                                |
|    |      | [ 70]    | $^1S_0$ | 157.5             | 2019 | R, KRCISD/aug-QZ                                                       |
|    |      | [ 4]     | —       | $160.8 \pm 4.0$   | 2019 | recommended                                                            |

Continued on next page

| Z  | Atom | Refs.    | State   | $\alpha$          | Year | Comments                                                               |
|----|------|----------|---------|-------------------|------|------------------------------------------------------------------------|
| 38 | Sr   | [ 71]    | $^1S_0$ | 158.2             | 2020 | R, MCDF                                                                |
|    |      | [ 15]    | $^1S_0$ | 156.2             | 2021 | SR, CCSD(T), ECP                                                       |
|    |      | [ 81]    | $^1S_0$ | $159.43 \pm 0.97$ | 2023 | R, CI+MBPT                                                             |
|    |      | [ 55]    | $^1S_0$ | 193.2             | 2000 | Model potential                                                        |
|    |      | [ 65]    | $^1S_0$ | $198.5 \pm 1.3$   | 2002 | CI, oscillator strength correction                                     |
|    |      | [ 32]    | $^1S_0$ | 201.2             | 2003 | Combination of ab initio and semi-empirical methods                    |
|    |      | [ 50]    | $^1S_0$ | 199.4             | 2004 | R, DK + SO, CCSD(T)                                                    |
|    |      | [ 50]    | $^1S_0$ | 198.85            | 2004 | R, DK, CCSD(T)                                                         |
|    |      | [ 78]    | $^1S_0$ | $186 \pm 15$      | 2004 | exp.                                                                   |
|    |      | [ 13,76] | $^1S$   | $199.0 \pm 2.0$   | 2006 | R, CI, MBPT2                                                           |
|    |      | [ 45]    | $^1S_0$ | 202.0             | 2006 | Hybrid-RCI + MBPT sum rule                                             |
|    |      | [ 46]    | $^1S_0$ | 199.71            | 2008 | R, Dirac, coupled cluster                                              |
|    |      | [ 67,82] | $^1S_0$ | $197.2 \pm 3.6$   | 2008 | R, Dirac, CI + MBPT + experimental data                                |
|    |      | [ 80]    | $^1S_0$ | 201.6             | 2008 | Combination of ab initio and experimental results                      |
|    |      | [ 83]    | $^1S_0$ | 197.6             | 2010 | CI + core polarisation (corrected to exp. term energies)               |
|    |      | [ 33,45] | $^1S_0$ | $197.2 \pm 0.2$   | 2010 | Hybrid-RCI + MBPT sum rule                                             |
|    |      | [ 47]    | $^1S_0$ | $186.98 \pm 0.85$ | 2013 | R, Dirac, MBPT, CCSD                                                   |
|    |      | [ 43]    | $^1S_0$ | 197.8             | 2013 | Combination of theoretical (CICP) and experimental methods             |
|    |      | [ 84]    | $^1S_0$ | $197.14 \pm 0.2$  | 2013 | CI + MBPT and experimental results                                     |
|    |      | [ 84]    | $^1S_0$ | $198.9 \pm 2.0$   | 2013 | CI + MBPT-SD and experimental results                                  |
|    |      | [ 69]    | $^1S_0$ | 190.82            | 2014 | R, Dirac + Breit, perturbed relativistic coupled-cluster theory (PRCC) |
|    |      | [ 35]    | $^1S_0$ | 197.9             | 2015 | Oscillator-strength sum rule                                           |
|    |      | [ 49]    | $^1S_0$ | 198.62/198.93     | 2019 | CCSD(T), ECP/R X2C-28                                                  |
|    |      | [ 70]    | $^1S_0$ | 196.5             | 2019 | R, KRCISD/aug-QZ                                                       |
|    |      | [ 4]     | --      | $197.2 \pm 0.2$   | 2019 | recommended                                                            |
|    |      | [ 71]    | $^1S_0$ | 214.5             | 2020 | R, MCDF                                                                |
|    |      | [ 72]    | $^1S_0$ | 203.16            | 2021 | R, CCSD(T)                                                             |
| 56 | Ba   | [ 79]    | $^1S_0$ | $268 \pm 22$      | 1974 | exp.                                                                   |
|    |      | [ 55]    | $^1S_0$ | 261.2             | 2000 | Model potential                                                        |
|    |      | [ 45,76] | $^1S$   | 262.2             | 2006 | R, CI, MBPT                                                            |
|    |      | [ 13,50] | $^1S_0$ | $273.5 \pm 4.1$   | 2006 | R, DK + SO, CCSD(T)                                                    |
|    |      | [ 45]    | $^1S_0$ | 272.1             | 2006 | Hybrid-RCI + MBPT sum rule                                             |
|    |      | [ 85]    | $^1S_0$ | $275.5 \pm 5.5$   | 2007 | R, DK, CCSD(T)                                                         |
|    |      | [ 46]    | $^1S_0$ | 268.19            | 2008 | R, Dirac, coupled cluster                                              |
|    |      | [ 33,45] | $^1S_0$ | $273.5 \pm 2.0$   | 2010 | Hybrid-RCI + MBPT sum rule, recommended                                |
|    |      | [ 51]    | $^1S_0$ | 272.7             | 2013 | R, Dirac + Gaunt, CCSD(T)                                              |

Continued on next page

| Z  | Atom | Refs.    | State   | $\alpha$          | Year | Comments                                                               |
|----|------|----------|---------|-------------------|------|------------------------------------------------------------------------|
| 88 | Ra   | [ 69]    | $^1S_0$ | 274.68            | 2014 | R, Dirac + Breit, perturbed relativistic coupled-cluster theory (PRCC) |
|    |      | [ 35]    | $^1S_0$ | $278.1 \pm 5.6$   | 2015 | Combination of theoretical and experimental data                       |
|    |      | [ 86]    | $^1S_0$ | 251               | 2016 | R, RPA, PolPot                                                         |
|    |      | [ 41]    | $^1S_0$ | 275.0             | 2016 | LR-CCSD                                                                |
|    |      | [ 87]    | $^1S_0$ | $274.92 \pm 0.01$ | 2018 | CCSD(T), R DKH ECP/CBS                                                 |
|    |      | [ 49]    | $^1S_0$ | 273.90/276.98     | 2019 | CCSD(T), R, ECP-46/X2C-46                                              |
|    |      | [ 70]    | $^1S_0$ | 269.0             | 2019 | R, KRCISD/aug-QZ                                                       |
|    |      | [ 4]     | --      | $272 \pm 10$      | 2019 | recommended                                                            |
|    |      | [ 71]    | $^1S_0$ | 276.2             | 2020 | R, MCDF                                                                |
|    |      | [ 50]    | $^1S_0$ | 248.56            | 2004 | R, DK + SO, CCSD(T)                                                    |
|    |      | [ 13,50] | $^1S_0$ | $246.2 \pm 4.9$   | 2006 | R, DK + SO, CCSD(T)                                                    |
|    |      | [ 51]    | $^1S_0$ | 242.8             | 2013 | R, Dirac + Gaunt, CCSD(T)                                              |
|    |      | [ 69]    | $^1S_0$ | 242.42            | 2014 | R, Dirac + Breit, perturbed relativistic coupled-cluster theory (PRCC) |
|    |      | [ 86]    | $^1S_0$ | 232               | 2016 | R, RPA, PolPot                                                         |
|    |      | [ 41]    | $^1S_0$ | 246.2             | 2016 | LR-CCSD                                                                |
|    |      | [ 88]    | $^1S_0$ | $236 \pm 15$      | 2018 | R, CCSD(T)                                                             |
|    |      | [ 70]    | $^1S_0$ | 248.5             | 2019 | R, KRCISD/aug-QZ                                                       |
|    |      | [ 4]     | --      | $246 \pm 4$       | 2019 | recommended                                                            |
|    |      | [ 52]    | $^1S_0$ | 247.838           | 2020 | R, DHF, MBPT                                                           |
|    |      | [ 89]    | $^1S_0$ | 250               | 2020 | R, CI+MBPT                                                             |
|    |      | [ 15]    | $^1S_0$ | 250.5             | 2021 | SR, CCSD(T), ECP                                                       |

### S4.3 Group 13 elements

The most accurate theoretical and experimental values for Group 13 elements are collected in Table S20. Next, a detailed comparison between this work and the results in the literature is presented, considering only the  $^2P_{1/2}$  state. Only computational and experimental values close to the recommended values in Ref. 4 are compared. For comparison of scalar-relativistic polarizability, only the  $SR_n$  value in this work is considered when  $SR_n$  and  $SR_d$  are different due to the fewer number of correlated electrons used in the latter calculations.

For B, the computed NR value is 20.41, closely matching literature values (20.47,<sup>90</sup>  $20.43 \pm 0.11$ ,<sup>1</sup> 20.42,<sup>48</sup> 20.480,<sup>91</sup> and  $20.30 \pm 0.26$ <sup>92</sup>), all using the CCSD(T) method. The

difference between the NR value in this work and the one in Ref. 91 could be attributed to the finite basis sets, and it can therefore be used for uncertainty estimation. The DC-CI value (20.35/20.38) for the  $^2P_{1/2}/^2P_{3/2}$  state is slightly lower than the MRCI result (20.53/20.54 a.u.) reported by Fleig.<sup>93</sup> This could be due to the triple excitations not being included and the larger basis set used in this work.

For Al, the DC-CC value ( $57.51 \pm 1.75$ ) is in good agreement with the recent CCSD result ( $58.8 \pm 1.2$ ) that includes Breit and QED contributions,<sup>94</sup> and experimental results ( $55.3 \pm 5.5$ ,<sup>68,95</sup>  $54 \pm 11$ ,<sup>74</sup> and  $54.9 \pm 5.3$ <sup>96</sup>). The computed DC-CI value ( $57.61 \pm 0.02$ ) is also close to other CI results ( $54.4 \pm 2.2$ <sup>93</sup> and  $57.8 \pm 1.0$ <sup>97</sup>). The calculated NR polarizability is  $57.15 \pm 0.08$ , which is in good agreement with literature values such as 57.74 by Lupinetti *et al.*<sup>98</sup> and 57.85 by Manz *et al.*,<sup>48</sup> using the CCSD(T) method. Additionally, the NR, SR, and DC values are  $64.00 \pm 0.89$ ,  $64.12 \pm 0.82$ , and  $56.74 \pm 0.26$ , respectively, obtained using Eq. (S3), as shown in Table S17. The NR and SR values are much higher than computational values in the literature, suggesting that Eq. (S3) is insufficient to obtain accurate  $\alpha$  for Al.

For Ga, In, and Tl, the most accurate values in the literature for the ground state, to my knowledge, are reported by Borschevsky *et al.* using CCSD(T) methods.<sup>99</sup> Therefore, I mainly focus on the comparison between this study and Ref. 99 for these three atoms. The DC-CC result ( $51.08 \pm 0.32$ ) for Ga is in excellent agreement with the result (51.05) reported by Borschevsky *et al.* using the CCSD(T) method.<sup>99</sup> Additionally, the computed CCSD result (52.18), as shown in Table S3, is also close to the CCSD value (52.48) reported in Ref. 99. The negligible difference could be attributed to the different basis sets used, the number of electrons correlated, or the fitting procedure. The basis set (31s22p14d6f4g1h) with a total number of 322 functions is used in this work, while the basis set (22s19p12d9f3g1h) with a total number of 307 functions is used in Ref. 99. However, compared to Ref. 99 where 21 electrons are correlated, only 13 electrons are used in this work. Moreover, three data points are used for fitting  $\alpha$  in Ref. 99, while five data points are employed in this study. The Gaunt contribution (0.18) is also evaluated in Ref. 99, which can be used for

uncertainty estimation. The DC-CI result (50.66) agrees well with other CI results (49.9<sup>93</sup> and  $51.3 \pm 2.0$ <sup>97</sup>). The computed NR polarizability for Ga is  $52.76 \pm 0.05$ , which is consistent with values such as  $52.91 \pm 0.40$  by Cernusak *et al.*<sup>100</sup> and 53.01 by Manz *et al.*<sup>48</sup> Compared to the experimental value, the DC-CC value is slightly higher than the upper bound of the experimental value ( $46.6 \pm 4.0$ ) reported by Ma *et al.*<sup>12</sup>

The DC-CC result (61.92) for In is in excellent agreement with the result (62.22) reported by Borschevsky *et al.* using the CCSD(T) method.<sup>99</sup> Additionally, the computed CCSD result (60.17), as shown in Table S3, is also close to the CCSD value (62.31) reported in Ref. 99. The difference could be attributed to the different basis sets used, the number of electrons correlated, or the fitting procedure. The basis set (34s28p19d6f4g1h) with a total number of 373 functions is used in this work, while the basis set (23s21p14d9f4g1h) with a total number of 341 functions is used in Ref. 99. Compared to Ref. 99, where 21 electrons are correlated with four-component DC-CC, 31 electrons are correlated with two-component DC-CC in this work. Moreover, three data points are used for fitting  $\alpha$  in Ref. 99, while five data points are employed in this study. The DC-CI result (62.87) agrees well with other CI results ( $61.9 \pm 1.2$ <sup>93</sup> and  $66.4 \pm 5.0$ <sup>97</sup>). The DC-CC and DC-CI results are also in good agreement with the experimental value ( $62.1 \pm 6.1$ ).<sup>12</sup>

The DC-CC result (51.26) for Tl is slightly smaller than the result (52.14) reported by Borschevsky *et al.* using the CCSD(T) method.<sup>99</sup> Additionally, the computed CCSD result (51.43), as shown in Table S3, is also slightly smaller than the CCSD value (52.56) reported in Ref. 99. It should be noted that 35 electrons are correlated with four-component DC-CC in both this work and Ref. 99. The difference can only be attributed to the different basis sets used or the fitting procedure. The basis set (35s32p22d15f4g1h) with a total number of 494 functions is used in this work, while the basis set (26s24p18d13f5g2h) with a total number of 453 functions is used in Ref. 99. Three data points are used for fitting  $\alpha$  in Ref. 99, while five data points are employed in this study. The Gaunt contribution ( $-0.72$ ) is also evaluated in Ref. 99, which can be used for uncertainty estimation. Another set of

four-component DC-CC calculations were performed with only 13 electrons being correlated in this work. The corresponding CCSD(T) result is  $51.94 \pm 0.20$ , suggesting that a difference of 0.68 a.u. is observed due to the smaller number of electrons correlated. Furthermore, the DC-CI result (51.26) agrees well with other CI results ( $51.6^{93}$  and  $50.7 \pm 5.0^{97}$ ). The DC-CC and DC-CI results are also in good agreement with the experimental value ( $51.3 \pm 5.4$ ).<sup>78</sup>

For Nh, the DC-CC value ( $32.89 \pm 0.18$ ) slightly exceeds the upper bounds of the recommended value ( $29.2 \pm 2$ ). Two earlier studies, FS-CCSD<sup>101</sup> and SD+CI,<sup>102</sup> have reported values of 29.85 and 28.8, respectively. The CCSD result (32.38) is also higher than the recommended value (29.85) by Pershina *et al.* using FS-CCSD. The difference could be attributed to the different basis sets used, the number of electrons correlated, or the fitting procedure. The basis set (36s36p25d17f4g1h) with a total number of 545 functions is used in this work, while the basis set (26s24p18d13f5g2h) with a total number of 453 functions is used in Ref. 101. However, compared to Ref. 101 where 46 electrons are correlated, only 35 electrons are used in this work. Three data points are used for fitting  $\alpha$  in Ref. 101, while five data points are employed in this study.

To further validate the computed data in this work, several tests are performed. First, a DC-CC calculation with 13 electrons being correlated is performed, and the CCSD(T) result is  $33.11 \pm 0.15$ , as shown in Table S3. The result shows that the difference is only 0.22 a.u. Second, a two-component DC-CC calculation with 49 electrons being correlated is performed, and the CCSD(T) result is 32.79, as shown in Table S3, suggesting that including more electrons only contributes 0.1 a.u. to  $\alpha$ . The last test is a two-component DC-CC calculation with a d-aug-dyall.acv4z basis set, i.e., (38s38p27d19f6g3h) with a total number of 657 functions, and 51 electrons correlated. Only the CCSD value is computed due to the extremely high computational cost. The CCSD result is  $32.57 \pm 0.02$ , and only a 0.02 a.u. difference is observed compared to the CCSD value (32.59) in the second test. This implies that the basis sets and number of correlated electrons are converged in this work. It should be noted that the computed DC-CI value (28.21) for Nh in this study aligns well with the previous SD+CI result (28.8) presented in Ref. 102. This also implies that a new recommended value for Nh should be updated based on the CCSD(T) result in this work.



Table S20: Summary of reference atomic dipole polarizabilities (in a.u.) for Group 13 elements, as reported in Refs. 4 and 5. Comment definitions are provided in these references.

| Z  | Atom | Refs.      | State                 | $\alpha$                    | Year | Comments                          |
|----|------|------------|-----------------------|-----------------------------|------|-----------------------------------|
| 5  | B    | [ 90]      | $^2P$                 | 20.47                       | 1976 | NR, PNO-CEPA, $M_L$ res.          |
|    |      | [ 1]       | $^2P$                 | $20.43 \pm 0.11$            | 1998 | NR, CCSD(T), $M_L$ res.           |
|    |      | [ 93]      | $^2P$                 | 20.59                       | 2005 | R, SF, MRCI, $M_L$ res.           |
|    |      | [ 93]      | $^2P_{1/2}/^2P_{3/2}$ | 20.53/20.54                 | 2005 | R, Dirac, MRCI, $M_J$ res.        |
|    |      | [ 48]      | $^2P$                 | 20.42                       | 2019 | NR, CCSD                          |
|    |      | [ 4]       | --                    | $20.5 \pm 0.1$              | 2019 | recommended                       |
|    |      | [ 91]      | $^2P$                 | 20.480                      | 2021 | NR, CCSD(T), CBS(T, Q), CBS(Q, 5) |
|    |      | [ 92]      | $^2P$                 | $20.30 \pm 0.26$            | 2021 | NR, CCSD(T)                       |
| 13 | Al   | [ 63]      | $^2P$                 | 62.0                        | 1971 | NR, numerical MCSCF, $M_L$ res.   |
|    |      | [ 59]      | $^2P$                 | 56.27                       | 1976 | NR, PNO-CEPA                      |
|    |      | [ 103]     | $^2P$                 | 59.47                       | 1980 | NR, MRCI                          |
|    |      | [ 104][92] | $^2P$                 | $46 \pm 2$                  | 1990 | exp. (see also ref [ 12])         |
|    |      | [ 105]     | $^2P$                 | 61.0                        | 2004 | SIC-DFT                           |
|    |      | [ 106]     | $^2P$                 | $58.0 \pm 0.4$              | 2004 | CCSD(T)                           |
|    |      | [ 98]      | $^2P$                 | 57.74                       | 2005 | NR, CCSD(T), $M_L$ res.           |
|    |      | [ 93]      | $^2P$                 | 55.5                        | 2005 | R, SF, MRCI, $M_L$ res.           |
|    |      | [ 93]      | $^2P_{1/2}/^2P_{3/2}$ | $55.4 \pm 2.2/55.9 \pm 2.2$ | 2005 | R, Dirac, MRCI, $M_J$ res.        |
|    |      | [ 13]      | $^2P$                 | $57.79 \pm 0.30$            | 2006 | R, DK, CCSD(T)                    |
|    |      | [ 97]      | $^2P_{1/2}/^2P_{3/2}$ | $57.8 \pm 1.0/58.0 \pm 1.0$ | 2010 | SI-SOCI, $M_L$ res.               |
|    |      | [ 68,95]   | $^2P$                 | $55.3 \pm 5.5$              | 2012 | exp.                              |
|    |      | [ 107]     | $^2P$                 | 58.3                        | 2016 | SIC-DFT (RXH)                     |
|    |      | [ 48]      | $^2P$                 | 57.85                       | 2019 | NR, CCSD                          |
|    |      | [ 4]       | --                    | $57.8 \pm 1.0$              | 2019 | recommended                       |
|    |      | [ 72]      | $^2P$                 | 58.089                      | 2021 | R, CCSD(T)                        |
|    |      | [ 73]      | $^2P$                 | 48.455                      | 2021 | R, CCSD(T)                        |
|    |      | [ 94]      | $^2P_{1/2}/^2P_{3/2}$ | $58.8 \pm 1.2/64.7 \pm 1.3$ | 2022 | R, Breit+QED, CCSD                |
|    |      | [ 74]      | $^2P$                 | $54 \pm 11$                 | 2022 | exp.                              |
|    |      | [ 96]      | $^2P$                 | $54.9 \pm 5.3$              | 2022 | exp.                              |
| 31 | Ga   | [ 92,108]  | $^2P$                 | $47.69 \pm 0.82$            | 2023 | NR, CCSD(T)                       |
|    |      | [ 64]      | $^2P$                 | $54.9 \pm 1.0$              | 1995 | NR, PNO-CEPA, $M_L$ res.          |
|    |      | [ 100]     | $^2P$                 | $52.91 \pm 0.40$            | 2003 | R, DK, CCSD(T)                    |
|    |      | [ 93]      | $^2P$                 | 50.7                        | 2005 | R, SF, MRCI, $M_L$ res.           |
|    |      | [ 93]      | $^2P_{1/2}/^2P_{3/2}$ | 49.9/51.6                   | 2005 | R, Dirac, MRCI, $M_J$ res.        |
|    |      | [ 97]      | $^2P_{1/2}/^2P_{3/2}$ | $51.3 \pm 2.0/53.0 \pm 2.0$ | 2010 | SI-SOCI, $M_J$ res.               |

Continued on next page

| Z  | Atom | Refs.          | State                 | $\alpha$                    | Year | Comments                                                 |
|----|------|----------------|-----------------------|-----------------------------|------|----------------------------------------------------------|
| 49 | In   |                |                       |                             |      | R, Dirac, FSCC, $M_J$ res.                               |
|    |      | [ 99]          | $^2P_{1/2}/^2P_{3/2}$ | $51.1 \pm 1.5/53.4 \pm 3.0$ | 2012 | ( $J = 3/2$ : $M_J = 3/2$ : 41.9,<br>$M_J = 1/2$ : 65.0) |
|    |      | [ 12]          | $^2P_{1/2}$           | $46.6 \pm 4.0$              | 2015 | exp.                                                     |
|    |      | [ 109]         | $^2P_{1/2}$           | 52.1                        | 2016 | TD-DFT (LEXX)                                            |
|    |      | [ 107]         | $^2P_{1/2}$           | 56.0                        | 2016 | SIC-DFT (RXH)                                            |
|    |      | [ 48]          | $^2P_{1/2}$           | 53.01                       | 2019 | NR, CCSD                                                 |
|    |      | [ 4]           | —                     | $50 \pm 3$                  | 2019 | recommended                                              |
|    |      | [ 72]          | $^2P_{1/2}$           | 40.899                      | 2021 | R, CCSD(T)                                               |
|    |      | [ 110]         | $^2P_{1/2}$           | $68.7 \pm 8.1$              | 1984 | exp.                                                     |
|    |      | [ 100]         | $^2P_{1/2}$           | $68.67 \pm 0.69$            | 2003 | R, DK, CCSD(T)                                           |
|    |      | [ 105]         | $^2P_{1/2}$           | 70.3                        | 2004 | SIC-DFT                                                  |
|    |      | [ 93]          | $^2P$                 | 66.7                        | 2005 | R, SF, MRCI, $M_L$ res.                                  |
|    |      | [ 93]          | $^2P_{1/2}/^2P_{3/2}$ | $61.9 \pm 1.2/69.6 \pm 1.4$ | 2005 | R, Dirac, MRCI, $M_J$ res.                               |
|    |      | [ 97]          | $^2P_{1/2}/^2P_{3/2}$ | $66.4 \pm 5.0/74.4 \pm 8.0$ | 2010 | SI-SOCI, $M_J$ res.                                      |
|    |      |                |                       |                             |      | R, Dirac, FSCC, $M_J$ res.                               |
|    |      | [ 99]          | $^2P_{1/2}/^2P_{3/2}$ | $62.0 \pm 1.9/69.7 \pm 4.0$ | 2012 | ( $J = 3/2$ : $M_J = 3/2$ : 55.1,<br>$M_J = 1/2$ : 84.6) |
|    |      | [ 93,99]       | $^2P_{1/2}$           | $61.5 \pm 5.6$              | 2012 | CCSD(T)                                                  |
|    |      | [ 111]         | $^2P_{1/2}$           | 62.4                        | 2013 | R, Dirac + Breit, CI + all-order                         |
|    |      | [ 12]          | $^2P_{1/2}$           | $62.1 \pm 6.1$              | 2015 | exp.                                                     |
|    |      | [ 107]         | $^2P_{1/2}$           | 73.1                        | 2016 | SIC-DFT (RXH)                                            |
|    |      | [ 41]          | $^2P_{1/2}$           | 70.22                       | 2016 | LR-CCSD                                                  |
|    |      | [ 4][155]      | $^2P_{1/2}$           | 65.2                        | 2019 | R, DFT                                                   |
|    |      | [ 48]          | $^2P_{1/2}$           | 67.9                        | 2019 | ECP, CCSD                                                |
|    |      | [ 4]           | —                     | $65 \pm 4$                  | 2019 | recommended                                              |
|    |      | [ 73]          | $^2P_{1/2}$           | 70.070                      | 2021 | R, CCSD(T)                                               |
|    |      | [ 94]          | $^2P_{1/2}$           | $64.3 \pm 1.3/82.3 \pm 1.7$ | 2022 | R, Breit+QED, CCSD                                       |
| 81 | Tl   | [ 48][2023185] | $^2P_{1/2}$           | 64.5                        | 2023 | R, (D)BSR                                                |
|    |      | [ 100]         | $^2P$                 | 50.48                       | 2003 | R, DK, CCSD(T)                                           |
|    |      | [ 100]         | $^2P$                 | 50.62                       | 2003 | R, DK, CCSD(T)                                           |
|    |      | [ 78]          | $^2P_{1/2}$           | $51.3 \pm 5.4$              | 2004 | exp.                                                     |
|    |      | [ 93]          | $^2P$                 | 70.0                        | 2005 | R, SF, MRCI, $M_L$ res.                                  |
|    |      | [ 93]          | $^2P_{1/2}/^2P_{3/2}$ | 51.6/81.2                   | 2005 | R, Dirac, MRCI, $M_J$ res.                               |
|    |      | [ 112]         | $^2P$                 | 50.4                        | 2006 | R, DHF, SD, MBPT all-order                               |
|    |      | [ 113]         | $^2P_{1/2}$           | 52.3                        | 2008 | R, Dirac, FS-CCSD                                        |
|    |      | [ 114]         | $^2P$                 | 48.81                       | 2009 | R, Dirac, CI+MBPT                                        |
|    |      | [ 115,116]     | $^2P$                 | 49.2                        | 2010 | RCI + MBPT                                               |

Continued on next page

| Z   | Atom | Refs.      | State                 | $\alpha$                    | Year | Comments                                                  |
|-----|------|------------|-----------------------|-----------------------------|------|-----------------------------------------------------------|
| 113 | Nh   | [ 97]      | $^2P_{1/2}/^2P_{3/2}$ | $50.7 \pm 5.0/78.5 \pm 6.0$ | 2010 | SI-SOCI, $M_J$ res.                                       |
|     |      |            |                       |                             |      | R, Dirac, FSCC, $M_J$ res.                                |
|     |      | [ 99]      | $^2P_{1/2}/^2P_{3/2}$ | 50.3/80.9                   | 2012 | ( $J = 3/2$ : $M_J = 3/2$ : 56.7,<br>$M_J = 1/2$ : 105.1) |
|     |      | [ 68,100]  | $^2P$                 | $71.7 \pm 1.1$              | 2012 | R, DK, CCSD(T)                                            |
|     |      | [ 99]      | $^2P$                 | $52.1 \pm 1.6/80.4 \pm 4.0$ | 2012 | R, Dirac, FSCC                                            |
|     |      | [ 117]     | $^2P$                 | $50.0 \pm 1.0$              | 2013 | R, CC                                                     |
|     |      | [ 117]     | $^2P$                 | 50.7                        | 2013 | R, CI + all-order                                         |
|     |      | [ 113,118] | $^2P$                 | 51.3                        | 2015 | R, Dirac, FS-CCSD                                         |
|     |      | [ 102]     | $^2P$                 | 47.78                       | 2016 | R, Dirac+Breit+QED, SD+CI, RPA                            |
|     |      | [ 109]     | $^2P$                 | 51.4                        | 2016 | TD-DFT (LEXX)                                             |
|     |      | [ 41]      | $^2P$                 | 69.92                       | 2016 | LR-CCSD                                                   |
|     |      | [ 119]     | $^2P$                 | $49.2 \pm 2.0$              | 2018 | R, Dirac+Breit, CCSD                                      |
|     |      | [ 48]      | $^2P$                 | 70.06                       | 2019 | ECP, CCSD                                                 |
|     |      | [ 4]       | --                    | $50 \pm 2$                  | 2019 | recommended                                               |
|     |      | [ 113]     | $^2P_{1/2}$           | 29.85                       | 2008 | R, Dirac, FS-CCSD                                         |
|     |      | [ 102]     | $^2P_{1/2}$           | 28.8                        | 2016 | R, Dirac+Breit+QED, SD+CI, RPA                            |
|     |      | [ 4]       | --                    | $29 \pm 2$                  | 2019 | recommended                                               |

## S4.4 Group 14 elements

The most accurate theoretical and experimental values for Group 14 elements are collected in Table S21 to validate the results in this work.

Only computational and experimental values close to the recommended values in Ref. 4 are compared. Additionally, Thierfelder *et al.* computed the static dipole polarizabilities for Group 14 elements using the same method as in this work.<sup>120</sup> Their computational values are also in excellent agreement with the recommended values from Ref. 4. Therefore, a more detailed comparison between this work and Ref. 120 is presented. For comparison of scalar-relativistic polarizability, only the  $SR_n$  value in this work is considered when  $SR_n$  and  $SR_d$  are different due to the fewer number of correlated electrons used in the latter calculations.

The DC value (11.73) of C is slightly larger than the upper bound of the result ( $11.26 \pm 0.20$ ) reported in Ref. 120. The difference could be attributed to the different basis sets

and the number of data points computed. The basis set ( $19s11p6d4f2g$ ) is used in this work compared to the ( $13s7p4d3f2g$ ) used in Ref. 120. In addition, energy with an external electric field of  $+0.0005$  a.u. is also added in this work compared to Ref. 120. Moreover, the difference between SR and DC values, as shown in Table 1, could be attributable to the small SOC effect for carbon. This suggests that  $LS$  coupling may provide a better description than  $jj$  coupling. The calculated SR polarizability of C (11.61) is close to the DK value (11.70) in Ref. 120 and the recent scalar-relativistic CCSD(T) result (11.524).<sup>72</sup> Due to the small relativistic effects, numerous NR values ( $11.67 \pm 0.07$ ,<sup>1</sup>  $11.63$ ,<sup>48</sup>  $11.64 \pm 0.15$ ,<sup>92</sup>  $11.683$ ,<sup>91</sup>  $11.324$ <sup>91</sup>) computed by the CCSD(T) method have been reported in the literature. The computed NR value (11.66) in this work is in good agreement with these values, with the largest error being less than 2%.

The DC, SR, and NR CCSD(T) values of Si are  $37.00 \pm 0.01$ ,  $37.10 \pm 0.01$ , and  $37.07 \pm 0.01$ , respectively, and are very close to the corresponding results (37.28, 37.58, and 37.54) reported in Ref. 120. The small difference in DC values is mainly attributed to the larger basis set ( $25s15p8d6f4g$ ) used in this work compared to the one ( $17s12p4d3f2g$ ) used in Ref. 120. In addition, the NR value in this work is in excellent agreement with NR CCSD(T) results ( $37.4 \pm 0.1$ ,<sup>121</sup>  $37.17 \pm 0.21$ ,<sup>98</sup>  $37.16$ ,<sup>48</sup> and  $36.90 \pm 0.63$ <sup>92</sup>) reported in the literature, as shown in Table S21. The difference between the SR value and the recent scalar-relativistic CCSD(T) result (36.803) is less than 1.2%.

The DC, SR, and NR CCSD(T) values for Ge are  $39.19 \pm 0.02$ ,  $39.53 \pm 0.07$ , and  $39.70 \pm 0.16$ , respectively, and are very close to the corresponding results (39.33, 39.97, and 40.16) reported in Ref. 120. The small difference in DC values could be attributed to the different basis sets and the number of correlated electrons. Specifically, a larger basis set ( $31s22p14d6f4g1h$ ) is used in this work compared to the one ( $23s19p15d4f2g$ ) used in Ref. 120. However, only 22 electrons are correlated in this work compared to all 32 electrons in Ref. 120. In addition, the NR value in this work is in excellent agreement with the recent NR CCSD(T) result (39.78).<sup>48</sup>

The DC, SR, and NR CCSD(T) values for tin Sn are 51.96,  $54.18 \pm 0.13$ , and  $55.48 \pm 0.15$ , respectively, and are very close to the corresponding results (52.70, 55.31, and 56.34) reported in Ref. 120. The difference in DC values could be attributed to the different basis sets and the number of correlated electrons. Specifically, a larger basis set ( $34s28p19d6f4g1h$ ) is used in this work compared to the one ( $36s29p21d6f2g$ ) used in Ref. 120. Additionally, 32 electrons are correlated in this work compared to only 22 electrons in Ref. 120. It should be noted that the Dyll basis set is also used for Sn in Ref. 120. Therefore, the difference can be used to evaluate the error due to the finite basis set. Furthermore, the DC value in this work is also in good agreement with experimental values ( $42.4 \pm 11^{120}$  and  $67.5 \pm 8.8^{12}$ ).

The DC, SR, and NR CCSD(T) values for Pb are 46.53,  $58.49 \pm 0.10$ , and  $62.20 \pm 0.09$ , respectively, and are very close to the corresponding results (47.34, 60.25, and 63.90) reported in Ref. 120. The difference in DC values could be attributed to the different basis sets and the number of correlated electrons. Specifically, the basis set ( $35s32p22d15f4g1h$ ) is used in this work compared to the one ( $37s33p25d19f2g$ ) used in Ref. 120. Additionally, 46 electrons are correlated in this work compared to only 36 electrons in Ref. 120. The Dyll basis set is also used for Pb in Ref. 120. Therefore, the difference can be used to evaluate the error due to the finite basis set. Furthermore, the DC value in this work is also in good agreement with experimental values ( $47.1 \pm 7.1^{78,120}$  and  $56 \pm 18^{12}$ ).

The DC, SR, and NR CCSD(T) values for Fl are 30.77,  $72.54 \pm 0.15$ , and  $77.92 \pm 0.13$ , respectively, and are very close to the corresponding results (31.49, 79.07, and 82.12) reported in Ref. 120. The difference in DC values could be attributed to the different basis sets and the number of correlated electrons. Specifically, a larger basis set ( $36s36p25d17f4g1h$ ) is used in this work compared to the one ( $32s31p24d18f3g$ ) used in Ref. 120. Additionally, 50 electrons are correlated in this work compared to only 36 electrons in Ref. 120.

Table S21: Summary of reference atomic dipole polarizabilities (in a.u.) for Group 14 elements, as reported in Refs. 4 and 5. Comment definitions are provided in these references.

| Z | Atom | Refs.  | State | $\alpha$         | Year | Comments                |
|---|------|--------|-------|------------------|------|-------------------------|
| 6 | C    | [ 122] | $^3P$ | 11.39            | 1992 | NR, CASPT2, $M_L$ res.  |
|   |      | [ 1]   | $^3P$ | $11.67 \pm 0.07$ | 1998 | NR, CCSD(T), $M_L$ res. |

Continued on next page

| Z  | Atom | Refs.      | State   | $\alpha$         | Year | Comments                                                              |
|----|------|------------|---------|------------------|------|-----------------------------------------------------------------------|
| 14 | Si   | [ 120]     | $^3P_0$ | $11.26 \pm 0.20$ | 2008 | R, Dirac + Gaunt, CCSD(T)                                             |
|    |      | [ 48]      | $^3P$   | 11.63            | 2019 | NR, CCSD                                                              |
|    |      | [ 4]       | --      | $11.3 \pm 0.2$   | 2019 | recommended                                                           |
|    |      | [ 92]      | $^3P$   | $11.64 \pm 0.15$ | 2021 | NR, CCSD(T)                                                           |
|    |      | [ 91]      | $^3P$   | 11.683           | 2021 | NR, CCSD(T), CBS(T, Q)                                                |
|    |      | [ 91]      | $^3P$   | 11.324           | 2021 | NR, CCSD(T), CBS(Q, 5)                                                |
|    |      | [ 72]      | $^3P$   | 11.542           | 2021 | R, CCSD(T)                                                            |
|    |      | [ 123]     | $^3P$   | 11.61            | 2023 | R, CCC (convergent close-coupling method)                             |
|    |      | [ 59]      | $^3P$   | 36.32            | 1976 | NR, PNO-CEPA, $M_L$ res.                                              |
|    |      | [ 103]     | $^3P$   | 36.95            | 1980 | NR, MRCI                                                              |
|    |      | [ 122]     | $^3P$   | 36.54            | 1992 | NR, CASPT2, $M_L$ res.                                                |
|    |      | [ 64]      | $^3P$   | 38.8             | 1995 | NR, numerical MCSCF, $M_L$ res.                                       |
|    |      | [ 121]     | $^3P$   | $37.4 \pm 0.1$   | 2003 | NR, CCSD(T), $M_L$ res.                                               |
|    |      | [ 105]     | $^3P$   | 38.9             | 2004 | SIC-DFT                                                               |
|    |      | [ 98]      | $^3P$   | $37.17 \pm 0.21$ | 2005 | NR, CCSD(T), $M_L$ res.                                               |
|    |      | [ 120]     | $^3P_0$ | $37.31 \pm 0.70$ | 2008 | R, Dirac + Gaunt, CCSD(T)                                             |
|    |      | [ 107]     | $^3P$   | 37.8             | 2016 | SIC-DFT (RXH)                                                         |
|    |      | [ 48]      | $^3P$   | 37.16            | 2019 | NR, CCSD                                                              |
|    |      | [ 4]       | --      | $37.3 \pm 0.7$   | 2019 | recommended                                                           |
|    |      | [ 92]      | $^3P$   | $36.90 \pm 0.63$ | 2021 | NR, CCSD(T)                                                           |
| 32 | Ge   | [ 72]      | $^3P$   | 36.803           | 2021 | R, CCSD(T)                                                            |
|    |      | [ 64]      | $^3P$   | 41.0             | 1995 | NR, PNO-CEPA, $M_L$ res.                                              |
|    |      | [ 105]     | $^3P$   | 41.6             | 2004 | SIC-DFT                                                               |
|    |      | [ 13]      | $^3P_0$ | $40.80 \pm 0.82$ | 2006 | R, PNO-CEPA                                                           |
|    |      | [ 120]     | $^3P$   | 39.97            | 2008 | R, DK, CCSD(T), $M_L$ res.<br>( $M_L = 0$ : 32.11, $M_L = 1$ : 43.90) |
|    |      | [ 120]     | $^3P_0$ | $39.43 \pm 0.80$ | 2008 | R, Dirac Gaunt, CCSD(T)                                               |
|    |      | [ 107]     | $^3P$   | 41.2             | 2016 | SIC-DFT (RXH)                                                         |
|    |      | [ 48]      | $^3P_0$ | 39.78            | 2019 | NR, CCSD                                                              |
|    |      | [ 4]       | --      | $40 \pm 1$       | 2019 | recommended                                                           |
|    |      | [ 78,124]  | $^3P$   | $52 \pm 13$      | 2004 | R, Dirac, LDA                                                         |
| 50 | Sn   | [ 105]     | $^3P$   | 57.5             | 2004 | SIC-DFT                                                               |
|    |      | [ 120]     | $^3P_0$ | $52.9 \pm 2.1$   | 2008 | R, Dirac + Gaunt, CCSD(T)                                             |
|    |      | [ 120]     | $^3P_0$ | $42.4 \pm 11$    | 2008 | exp.                                                                  |
|    |      | [ 125]     | $^3P_0$ | 54.48            | 2009 | R, PP, DFT, BP386                                                     |
|    |      | [ 12]      | $^3P_0$ | $67.5 \pm 8.8$   | 2015 | exp.                                                                  |
|    |      | [ 107]     | $^3P_0$ | 57.9             | 2016 | SIC-DFT (RXH)                                                         |
|    |      | [ 105,109] | $^3P_0$ | 60.0             | 2016 | TD-DFT (LEXX)                                                         |

Continued on next page

| Z   | Atom | Refs.     | State   | $\alpha$       | Year | Comments                             |
|-----|------|-----------|---------|----------------|------|--------------------------------------|
| 82  | Pb   | [ 41]     | $^3P_0$ | 55.95          | 2016 | LR-CCSD                              |
|     |      | [ 48]     | $^3P_0$ | 54.29          | 2019 | ECP, CCSD                            |
|     |      | [ 4]      | --      | $53 \pm 6$     | 2019 | recommended                          |
|     |      | [ 72]     | $^3P_0$ | 60.115         | 2021 | R, CCSD(T)                           |
|     |      | [ 73]     | $^3P_0$ | 61.063         | 2021 | R, CCSD(T)                           |
|     |      | [ 124]    | $^3P$   | $46 \pm 11$    | 1987 | R, Dirac, LDA                        |
|     |      | [ 126]    | $^3P_0$ | 51.0           | 2005 | R, SOPP, CCSD(T)                     |
|     |      | [ 120]    | $^3P_0$ | 47.70          | 2008 | R, Dirac + Gaunt, CCSD(T)            |
|     |      | [ 127]    | $^3P_0$ | 46.96          | 2008 | R, Dirac, CCSD(T)                    |
|     |      | [ 120]    | $^3P_0$ | $47.3 \pm 1.9$ | 2008 | R, Dirac + Gaunt, CCSD(T)            |
|     |      | [ 78,120] | $^3P_0$ | $47.1 \pm 7.1$ | 2008 | exp.                                 |
|     |      | [ 118]    | $^3P_0$ | 47.0           | 2015 | R, Dirac, FS-CCSD                    |
|     |      | [ 12]     | $^3P_0$ | $56 \pm 18$    | 2015 | exp.                                 |
|     |      | [ 102]    | $^3P_0$ | 44.04          | 2016 | R, Dirac + Breit + QED, SD + CI, RPA |
|     |      | [ 128]    | $^3P_0$ | 46.5           | 2016 | R, CI + all-order, RPA               |
|     |      | [ 109]    | $^3P_0$ | 47.9           | 2016 | TD-DFT (LEXX)                        |
|     |      | [ 41]     | $^3P_0$ | 61.80          | 2016 | LR-CCSD                              |
|     |      | [ 48]     | $^3P_0$ | 60.07          | 2019 | EP, CCSD                             |
|     |      | [ 4]      | --      | $47 \pm 3$     | 2019 | recommended                          |
|     |      | [ 89]     | $^3P_0$ | 46             | 2020 | R, CI+MBPT                           |
|     |      | [ 129]    | $^3P_0$ | 47.0           | 2020 | R, FS-RCCSD(T)                       |
|     |      | [ 130]    | $^3P_0$ | 56.3           | 2023 | R (ATZP-ZORA), DFT(B3LYP)            |
| 114 | Fl   | [ 126]    | $^3P_0$ | 34.35          | 2005 | R, SOPP, CCSD(T)                     |
|     |      | [ 120]    | $^3P_0$ | 31.87          | 2008 | R, Dirac + Gaunt, CCSD(T)            |
|     |      | [ 127]    | $^3P_0$ | 30.59          | 2008 | R, Dirac, CCSD(T)                    |
|     |      | [ 127]    | $^3P_0$ | 29.52          | 2008 | estimate                             |
|     |      | [ 120]    | $^3P_0$ | 31.0           | 2008 | R, Dirac + Gaunt, CCSD(T)            |
|     |      | [ 102]    | $^3P_0$ | 31.4           | 2016 | R, Dirac + Breit + QED, SD + CI, RPA |
|     |      | [ 4]      | --      | $31 \pm 4$     | 2019 | recommended                          |

## S4.5 Group 15 elements

A detailed comparison between this work and the SR and NR results in the literature is presented. Only computational and experimental values close to the recommended values in Ref. 4 are compared. For computational data, only values computed with CCSD(T) methods in the literature are considered. For comparison of scalar-relativistic polarizability,

only the  $SR_n$  value in this work is considered when  $SR_n$  and  $SR_d$  are different due to the fewer number of correlated electrons used in the latter calculations.

The SR value (7.24) of N in this work is in excellent agreement with the experimental values ( $7.6 \pm 0.4$ <sup>6,131</sup> and  $7.28$ <sup>132,133</sup>). Additionally, the SR value is also close to another SR CCSD(T) result, 7.178, reported by Canal Neto *et al.*<sup>72</sup> The NR value (7.25) is in good agreement with previous computational values, e.g., 7.21,<sup>48</sup> 7.2,<sup>134</sup> and  $7.25 \pm 0.09$ .<sup>92</sup> However, a slightly larger deviation ( $< 0.12$  a.u.) is observed between the NR value in this work and the values (7.367 and 7.153), including the extrapolation to the complete basis set limit, reported by Ěhn and Černušák. This difference is therefore employed as the error due to the  $\Delta P_{\text{basis}}$ .

No experimental data is available for P in the literature for comparison. The SR value (24.93) in this work is in excellent agreement with the SR data (24.980) reported in Ref. 72. The NR value (24.92) also perfectly aligns with recent NR CCSD(T) results (24.88,<sup>48</sup> 25.0,<sup>134</sup>  $24.95 \pm 0.43$ <sup>92</sup>) where very large basis sets are used. This suggests that the Dyall basis set is also sufficient to obtain a reasonable dipole polarizability for P.

Similarly, no experimental data is available for As in the literature for comparison. The SR value ( $29.70 \pm 0.01$ ) in this work is in excellent agreement with the SR data (29.92) reported in Ref. 72, and the SR results obtained by the ECP method, e.g., 29.81<sup>133</sup> and 29.6.<sup>134</sup> The NR value ( $29.83 \pm 0.01$ ) is also close to the counterpart (29.65) reported in Ref. 48.

Again, no experimental data is available for Sb in the literature for comparison. The SR value ( $42.96 \pm 0.01$ ) in this work is in excellent agreement with the SR data computed by CCSD(T) with the ECP method (43.03,<sup>133</sup> 42.78,<sup>48</sup> and 42.8<sup>134</sup>). Additionally, the NR value ( $43.78 \pm 0.01$ ) is slightly larger than the counterpart (42.26) reported in Ref. 135. This difference can be attributed to the much larger uncontracted basis set (*34s28p19d6f4g1h*) used in this work compared to the contracted one [*6s6p4d1f*] used in Ref. 135.

For Bi, the DC value lies within the uncertainty of the experimental value ( $55 \pm 11$ ).<sup>12</sup>



The SR value ( $48.60 \pm 0.01$ ) in this work is in excellent agreement with the SR data computed by CCSD(T) with the ECP method ( $48.75$ ,<sup>133</sup>  $48.88$ ,<sup>48</sup> and  $48.8$ <sup>134</sup>).

It should be noted that there are no NR and SR data available in the literature for Mc based on Table S22. In this work, they are computed to be 60.84 and  $60.64 \pm 0.02$ , respectively, by CCSD(T).

Table S22: Summary of reference atomic dipole polarizabilities (in a.u.) for Group 15 elements, as reported in Refs. 4 and 5. Comment definitions are provided in these references.

| Z  | Atom | Refs.      | State       | $\alpha$          | Year | Comments                                      |
|----|------|------------|-------------|-------------------|------|-----------------------------------------------|
| 7  | N    | [ 6,131]   | $^4S_{3/2}$ | $7.6 \pm 0.4$     | 1974 | exp.                                          |
|    |      | [ 90]      | $^4S$       | 7.43              | 1976 | NR, PNO-CEPA                                  |
|    |      | [ 64]      | $^4S$       | 7.36              | 1995 | NR, numerical MCSCF, M. res.                  |
|    |      | [ 1]       | $^4S$       | $7.26 \pm 0.05$   | 1998 | NR, CCSD(T)                                   |
|    |      | [ 136]     | $^4S$       | 7.41              | 2004 | R, DK, CASPT2                                 |
|    |      | [ 132,133] | $^4S_{3/2}$ | 7.28              | 2010 | exp.                                          |
|    |      | [ 48]      | $^4S$       | 7.21              | 2019 | NR, CCSD                                      |
|    |      | [ 4]       | —           | $7.4 \pm 0.2$     | 2019 | recommended                                   |
|    |      | [ 134]     | $^4S$       | 7.2               | 2020 | AE, CCSD(T)                                   |
|    |      | [ 92]      | $^4S$       | $7.25 \pm 0.09$   | 2021 | NR, CCSD(T)                                   |
|    |      | [ 91]      | $^4S$       | 7.367             | 2021 | NR, CCSD(T), CBS(T, Q)                        |
|    |      | [ 91]      | $^4S$       | 7.153             | 2021 | NR, CCSD(T), CBS(Q, 5)                        |
|    |      | [ 72]      | $^4S$       | 7.178             | 2021 | R, CCSD(T)                                    |
|    |      | [ 31]      | $^4S$       | $7.189 \pm 0.008$ | 2024 | NR, neural network QMC, DS (DeepSolid) method |
| 15 | P    | [ 59]      | $^4S$       | $24.7 \pm 0.5$    | 1976 | NR, PNO-CEPA                                  |
|    |      | [ 122]     | $^4S$       | $24.6 \pm 0.2$    | 1992 | NR, CASPT2                                    |
|    |      | [ 64]      | $^4S$       | 25.5              | 1995 | NR, numerical MCSCF, $M_L$ res.               |
|    |      | [ 136]     | $^4S$       | 24.9              | 2004 | R, DK, CASPT2                                 |
|    |      | [ 105]     | $^4S$       | 26.11             | 2004 | SIC-DFT                                       |
|    |      | [ 98]      | $^4S$       | $24.93 \pm 0.15$  | 2005 | NR, CCSD(T)                                   |
|    |      | [ 133]     | $^4S$       | 25.06             | 2010 | R, DK, CASPT2                                 |
|    |      | [ 107]     | $^4S$       | 25.3              | 2016 | SIC-DFT (RXH)                                 |
|    |      | [ 48]      | $^4S$       | 24.88             | 2019 | NR, CCSD                                      |
|    |      | [ 4]       | —           | $25 \pm 1$        | 2019 | recommended                                   |
|    |      | [ 134]     | $^4S$       | 25.0              | 2020 | AE, CCSD(T)                                   |
|    |      | [ 92]      | $^4S$       | $24.95 \pm 0.43$  | 2021 | NR, CCSD(T)                                   |
|    |      | [ 72]      | $^4S$       | 24.980            | 2021 | R, CCSD(T)                                    |
|    |      | [ 64]      | $^4S$       | 29.1              | 1995 | NR, PNO-CEPA                                  |
|    |      | [ 64]      | $^4S$       | 30.5              | 1995 | NR, numerical MCSCF                           |

Continued on next page

| Z   | Atom | Refs.      | State       | $\alpha$       | Year | Comments                                            |
|-----|------|------------|-------------|----------------|------|-----------------------------------------------------|
| 51  | Sb   | [ 136]     | $^4S$       | $29.8 \pm 0.6$ | 2004 | R, DK, CASPT2                                       |
|     |      | [ 105]     | $^4S$       | 31.52          | 2004 | SIC-DFT                                             |
|     |      | [ 133]     | $^4S$       | 29.92          | 2010 | R, DK, CCSD(T)                                      |
|     |      | [ 133]     | $^4S$       | 29.81          | 2010 | ECP, CCSD(T)                                        |
|     |      | [ 109]     | $^4S$       | 29.6           | 2016 | TD-DFT (LEXX)                                       |
|     |      | [ 107]     | $^4S$       | 30.7           | 2016 | SIC-DFT (RXH)                                       |
|     |      | [ 48]      | $^4S$       | 29.65          | 2019 | NR, CCSD                                            |
|     |      | [ 4]       | —           | $30 \pm 1$     | 2019 | recommended                                         |
|     |      | [ 134]     | $^4S$       | 29.6           | 2020 | ECP, CCSD(T)                                        |
|     |      | [ 78,124]  | $^4S$       | $45 \pm 11$    | 2004 | R, Dirac, LDA                                       |
|     |      | [ 136]     | $^4S$       | $42.2 \pm 1.3$ | 2004 | R, DK, CASPT2                                       |
|     |      | [ 105]     | $^4S$       | 47.07          | 2004 | SIC-DFT                                             |
|     |      | [ 135]     | $^4S$       | 42.26          | 2007 | NR, CCSD(T)                                         |
|     |      | [ 133]     | $^4S$       | 43.03          | 2010 | ECP, CCSD(T)                                        |
|     |      | [ 107]     | $^4S$       | 45.7           | 2016 | SIC-DFT (RXH)                                       |
|     |      | [ 105,109] | $^4S$       | 44.0           | 2016 | TD-DFT (LEXX)                                       |
|     |      | [ 48]      | $^4S$       | 42.78          | 2019 | ECP, CCSD                                           |
|     |      | [ 4]       | —           | $43 \pm 2$     | 2019 | recommended                                         |
|     |      | [ 134]     | $^4S$       | 42.8           | 2020 | ECP, CCSD(T)                                        |
| 83  | Bi   | [ 137]     | $^4S$       | 52.85          | 1992 | R, Cowan-Griffin, HF only                           |
|     |      | [ 78,124]  | $^4S$       | $50 \pm 12$    | 2004 | R, Dirac, LDA                                       |
|     |      | [ 136]     | $^4S$       | 48.6           | 2004 | R, DK, CASPT2                                       |
|     |      | [ 133]     | $^4S$       | 48.75          | 2010 | ECP, CCSD(T)                                        |
|     |      | [ 12]      | $^4S_{3/2}$ | $55 \pm 11$    | 2015 | exp.                                                |
|     |      | [ 102]     | $^4S$       | 44.62          | 2016 | R, Dirac + Breit + QED, SD + CI, RPA                |
|     |      | [ 109]     | $^4S$       | 43.2           | 2016 | TD-DFT (LEXX)                                       |
|     |      | [ 41]      | $^4S$       | 49.02          | 2016 | LR-CCSD                                             |
|     |      | [ 48]      | $^4S$       | 48.88          | 2019 | ECP, CCSD                                           |
|     |      | [ 4]       | —           | $48 \pm 4$     | 2019 | recommended                                         |
|     |      | [ 134]     | $^4S$       | 48.8           | 2020 | ECP, CCSD(T)                                        |
|     |      | [ 138]     | $^4S$       | 44.36          | 2022 | R (ZORA), CCSD(T)                                   |
|     |      | [ 138]     | $^4S$       | 53.1           | 2022 | R (ATZP-ZORA), DFT (B3LYP)                          |
|     |      | [ 130]     | $^4S$       | 46.6           | 2023 | R (ZORA), DFT (B3LYP)                               |
|     |      | [ 139]     | $^4S_{3/2}$ | 66             | 2014 | Estimated via correlation with $R_{\max}(np_{3/2})$ |
|     |      | [ 102]     | $^4S_{3/2}$ | 70.5           | 2016 | R, Dirac + Breit + QED, SD + CI, RPA                |
|     |      | [ 4]       | —           | $71 \pm 20$    | 2019 | recommended                                         |
| 115 | Mc   | [ 139]     | $^4S_{3/2}$ | 66             | 2014 | Estimated via correlation with $R_{\max}(np_{3/2})$ |
|     |      | [ 102]     | $^4S_{3/2}$ | 70.5           | 2016 | R, Dirac + Breit + QED, SD + CI, RPA                |
|     |      | [ 4]       | —           | $71 \pm 20$    | 2019 | recommended                                         |

## S4.6 Group 16 elements

The most accurate theoretical and experimental values for Group 16 elements are collected in Table S23 to validate the results in this work. Only computational and experimental values close to the recommended values in Ref. 4 are compared. For SR and NR results, only values computed with CCSD(T) methods in the literature are considered. In addition, for SR polarizability, only the  $SR_n$  value in this work is considered when  $SR_n$  and  $SR_d$  are different due to the fewer number of correlated electrons used in the latter calculations.

The SR value (5.15) of O in this work is in excellent agreement with the experimental value  $(5.2 \pm 0.4)$ .<sup>131</sup> The NR value (5.16) is in good agreement with previous computational values, e.g.,  $5.24 \pm 0.04$ ,<sup>1,13</sup>  $5.21 \pm 0.07$ ,<sup>92</sup> and 5.145.<sup>91</sup> The NR, SR, and DC values obtained by fitting Eq. (S3) are 5.16, 5.16, and 5.13, respectively, suggesting that the difference due to the fitting procedure is small for O.

No experimental data is available for S in the literature for comparison. The NR value  $(19.17 \pm 0.03)$  in Table 1 for S is slightly smaller than the recommended value  $(19.4 \pm 0.1)$  and other computational values in Table S23, e.g.,  $19.37 \pm 0.12$ .<sup>98</sup> The NR, SR, and DC values, obtained by fitting Eq. (S3), are  $19.41 \pm 0.02$ ,  $19.44 \pm 0.02$ , and 19.10, respectively. This suggests that the precision of CCSD(T) energies should be improved to obtain valid NR and SR hyperpolarizabilities for S using Eq. (S1).

The DC value for Se (24.48) is much lower than the recommended value  $(28.90 \pm 1.0)$ , which is based on the experimental result from Ref. 140. However, the scalar-relativistic value  $(25.57 \pm 0.19)$  in this study closely aligns with previous computational values  $(26.24 \pm 0.52)$ <sup>141</sup> and  $26.65$ <sup>105</sup>). The NR CCSD value (25.19) is close to the linear-response CCSD value (25.03).<sup>48</sup> It should be noted that negative NR and SR hyperpolarizabilities are observed at the CCSD(T) level, leading to large uncertainties in  $\alpha$  as shown in Table 1.

The SR CCSD value (37.63) for Te, as shown in Table S6, is close to the linear-response CCSD values  $(37.65)$ <sup>41</sup> and  $37.51$ <sup>48</sup>). It should be noted that negative NR and SR hyperpolarizabilities are observed at the CCSD(T) level, leading to a large uncertainty in  $\alpha$  for Te,

as shown in Table 1. The difference between SR DHF and CCSD values is 0.35, as shown in Table S6, indicating a small contribution to  $\alpha$  due to electron correlation for Te. Therefore, the NR and SR CCSD values (38.08 and 37.63) could be more accurate for Te than CCSD(T) due to large numerical errors in hyperpolarizability.

The SR value (44.32) of Po is close to the recent CCSD(T) value (44.77) reported by Centoducatte *et al.*<sup>138</sup> The SR CCSD value (43.97) agrees well with the result (44.22) computed by CCSD with the ECP method.<sup>48</sup>

The theoretical values for Lv are also estimated, with the NR, SR, and DC values being  $58.72 \pm 0.01$ ,  $57.00 \pm 0.01$ , and 71.66, respectively. Accounting for SOC effects in the Lv calculation led to a reduction of 14.66 in the dipole polarizability compared to the scalar-relativistic calculation. The scalar-relativistic results at the CCSD(T) level closely match its DHF values. This suggests that the influence of electron correlation is small when determining the dipole polarizability of Lv in scalar-relativistic calculations.

Table S23: Summary of reference atomic dipole polarizabilities (in a.u.) for Group 16 elements, as reported in Refs. 4 and 5. Comment definitions are provided in these references.

| Z  | Atom | Refs.    | State   | $\alpha$          | Year | Comments                                      |
|----|------|----------|---------|-------------------|------|-----------------------------------------------|
| 8  | O    | [ 131]   | $^3P_2$ | $5.2 \pm 0.4$     | 1959 | exp.                                          |
|    |      | [ 122]   | $^3P$   | 5.4               | 1992 | NR, CASPT2, $M_L$ res.                        |
|    |      | [ 78,90] | $^3P$   | $5.41 \pm 0.11$   | 2004 | NR, PNO-CEPA, $M_L$ res.                      |
|    |      | [ 1,13]  | $^3P$   | $5.24 \pm 0.04$   | 2006 | NR, CCSD(T), $M_L$ res.                       |
|    |      | [ 48]    | $^3P$   | 5.15              | 2019 | NR, CCSD                                      |
|    |      | [ 4]     | —       | $5.3 \pm 0.2$     | 2019 | recommended                                   |
|    |      | [ 92]    | $^3P$   | $5.21 \pm 0.07$   | 2021 | NR, CCSD(T)                                   |
|    |      | [ 91]    | $^3P$   | 5.145             | 2021 | NR, CCSD(T), CBS(T, Q)                        |
| 16 | S    | [ 31]    | $^3P$   | $5.236 \pm 0.008$ | 2024 | NR, neural network QMC, DS (DeepSolid) method |
|    |      | [ 59]    | $^3P$   | 19.60             | 1976 | NR, PNO-CEPA, $M_L$ res.                      |
|    |      | [ 122]   | $^3P$   | 19.6              | 1992 | NR, CASPT2, $M_L$ res.                        |
|    |      | [ 141]   | $^3P$   | 19.6              | 2000 | NR, CASPT2, $M_L$ res.                        |
|    |      | [ 105]   | $^3P$   | 19.72             | 2004 | SIC-DFT                                       |
|    |      | [ 98]    | $^3P$   | $19.37 \pm 0.12$  | 2005 | NR, CCSD(T), $M_L$ res.                       |
|    |      | [ 48]    | $^3P$   | 19.22             | 2019 | NR, CCSD(T)                                   |
|    |      | [ 4]     | —       | $19.4 \pm 0.1$    | 2019 | recommended                                   |
| 34 | Se   | [ 92]    | $^3P$   | $19.38 \pm 0.33$  | 2021 | NR, CCSD(T)                                   |
|    |      | [ 131]   | $^3P$   | $26.24 \pm 0.52$  | 1959 | R, MVD, CASPT2, $M_L$ res.                    |

Continued on next page

| Z   | Atom | Refs.        | State   | $\alpha$       | Year | Comments                                            |
|-----|------|--------------|---------|----------------|------|-----------------------------------------------------|
| 52  | Te   | [ 140]       | $^3P_2$ | $28.9 \pm 1.0$ | 1997 | exp.                                                |
|     |      | [ 105]       | $^3P$   | 26.65          | 2004 | SIC-DFT                                             |
|     |      | [ 107]       | $^3P$   | 29.3           | 2016 | TD-DFT (PGG)                                        |
|     |      | [ 107]       | $^3P$   | 24.0           | 2016 | SIC-DFT (RXH)                                       |
|     |      | [ 48]        | $^3P$   | 25.03          | 2019 | NR, CCSD                                            |
|     |      | [ 4]         | --      | $28.9 \pm 1.0$ | 2019 | recommended                                         |
|     |      | [ 78,124]    | $^3P$   | $37 \pm 4$     | 2004 | R, LDA                                              |
|     |      | [ 105]       | $^3P$   | 40.06          | 2004 | SIC-DFT                                             |
|     |      | [ 13,142]    | $^3P$   | $38.1 \pm 3.8$ | 2006 | QR, MVD-HF, GTO basis set                           |
|     |      | [ 107]       | $^3P$   | 36.9           | 2016 | SIC-DFT (RXH)                                       |
|     |      | [ 41]        | $^3P$   | 37.65          | 2016 | LR-CCSD                                             |
|     |      | [ 48]        | $^3P$   | 37.51          | 2019 | ECP, CCSD                                           |
|     |      | [ 4]         | --      | $38 \pm 4$     | 2019 | recommended                                         |
|     |      | [ 143]       | $^3P$   | 37.3           | 2022 | R, Dirac, CIPT+SD (RPA)                             |
| 84  | Po   | [ 137]       | $^3P_2$ | 46.8           | 1992 | R, Cowan-Griffin, HF only, $M_L$ res.               |
|     |      | [ 78,124]    | $^3P_2$ | 46             | 2004 | R, Dirac, LDA                                       |
|     |      | [ 13,68,137] | $^3P_2$ | $43.6 \pm 4.4$ | 2012 | R, Cowan-Griffin, HF only                           |
|     |      | [ 41]        | $^3P_2$ | 45.01          | 2016 | LR-CCSD                                             |
|     |      | [ 48]        | $^3P_2$ | 44.22          | 2019 | ECP, CCSD                                           |
|     |      | [ 4]         | --      | $44 \pm 4$     | 2019 | recommended                                         |
|     |      | [ 138]       | $^3P_2$ | 44.77          | 2022 | R (ZORA), CCSD(T)                                   |
|     |      | [ 138]       | $^3P_2$ | 47.1           | 2022 | R (ZORA), DFT (B3LYP)                               |
|     |      | [ 130]       | $^3P_2$ | 46.5           | 2023 | R (ATZP-ZORA), DFT (B3LYP)                          |
|     |      | [ 139]       | $^3P_2$ | 61.17          | 2014 | Estimated via correlation with $R_{\max}(np_{3/2})$ |
| 116 | Lv   | [ 4]         | --      | $67 \pm 10$    | 2019 | recommended                                         |

## S4.7 Group 17 elements

The most accurate theoretical and experimental values for Group 17 elements are collected in Table S24 to validate the results in this work. It can be seen that there are no DC values available for Ts yet. Only computational and experimental values close to the recommended values in Ref. 4 are compared. For SR and NR results, only values computed with CCSD(T) methods in the literature are considered. In addition, for SR polarizability, only the  $SR_n$  value in this work is considered when  $SR_n$  and  $SR_d$  are different due to the fewer number of correlated electrons used in the latter calculations.

The NR value (3.60) of F in this work is slightly smaller than other computational results ( $3.70 \pm 0.03$ ,<sup>1</sup>  $3.68 \pm 0.05$ ,<sup>92</sup>  $3.701$ ,<sup>91</sup> and  $3.655$ <sup>91</sup>) obtained by the CCSD(T) method. The NR value of 3.62 is obtained by using the same data points and numerical differentiation equation used in Ref. 91, suggesting that the deviation could be attributed to the finite basis set.

The NR value (14.54) of Cl is in excellent agreement with other theoretical results ( $14.57 \pm 0.10$ ,<sup>98</sup>  $14.59 \pm 0.25$ ,<sup>92</sup> and  $14.582$ <sup>72</sup>) computed with the CCSD(T) method.

The DC-CI value (20.06) of the  $^2P_{3/2}$  state for Br is close to the result (21.7) obtained by Fleig *et al.* using the MRCI method.<sup>144</sup> The NR CCSD value (20.45), as shown in Table S7, also aligns with the result (20.4) obtained by the linear-response CCSD method.<sup>48</sup>

The DC-CI value (31.28) of the  $^2P_{3/2}$  state for I is slightly smaller than the lower bound of the recommended value ( $32.9 \pm 1.3$ ), which is based on the experimental value reported by Maroulis *et al.*<sup>13</sup> Additionally, it is also slightly smaller compared to the MRCI value ( $34.1$ <sup>144</sup> and  $33.0 \pm 1.7$ <sup>13,142,144</sup>). This deviation could be attributed to the lack of higher-order excitations or the larger basis set used in this work. The SR CCSD value (31.73), as shown in Table S7, is in good agreement with the result (31.57) obtained by the linear-response CCSD with the ECP method.

The DC-CI value (38.92) of the  $^2P_{3/2}$  state for At is slightly smaller than the MRCI value (41.9) reported by Fleig *et al.*<sup>144</sup> The SR CCSD(T) value (38.39) is close to CCSD(T) results ( $40.4$ <sup>4</sup> and  $41.1$ <sup>130</sup>) obtained by the ZORA scalar-relativistic CCSD(T). However, the SR CCSD value (38.06), as shown in Table S7, is in excellent agreement with the linear-response CCSD result ( $38.93$ )<sup>41</sup> and the CCSD value (38.15) computed with the ECP method.<sup>48</sup>

For Ts, only empirically estimated values are available in the literature.<sup>139,145</sup> This results in a very large uncertainty for Ts, as recommended in Ref. 4. In this work, NR, SR, and DC values are evaluated using systematic methods similar to those used for other elements in the same group. The final DC value is 65.15 for the  $^2P_{3/2}$  state, which aligns well with the recommended value ( $76.0 \pm 15$ ).<sup>4</sup>

Table S24: Summary of reference atomic dipole polarizabilities (in a.u.) for Group 17 elements, as reported in Refs. 4 and 5. Comment definitions are provided in these references.

| Z  | Atom | Refs.         | State       | $\alpha$          | Year | Comments                                      |
|----|------|---------------|-------------|-------------------|------|-----------------------------------------------|
| 9  | F    | [ 90]         | $^2P$       | 3.76              | 1976 | NR, PNO-CEPA, $M_L$ res.                      |
|    |      | [ 1]          | $^2P$       | $3.70 \pm 0.03$   | 1998 | NR, CCSD(T), $M_L$ res.                       |
|    |      | [ 141]        | $^2P$       | $3.76 \pm 0.06$   | 2000 | NR, CASPT2, $M_L$ res.                        |
|    |      | [ 48]         | $^2P$       | 3.62              | 2019 | NR, CCSD                                      |
|    |      | [ 4]          | --          | $3.74 \pm 0.08$   | 2019 | recommended                                   |
|    |      | [ 92]         | $^2P$       | $3.68 \pm 0.05$   | 2021 | NR, CCSD(T)                                   |
|    |      | [ 91]         | $^2P$       | 3.701             | 2021 | NR, CCSD(T), CBS(T, Q)                        |
|    |      | [ 91]         | $^2P$       | 3.655             | 2021 | NR, CCSD(T), CBS(Q, 5)                        |
|    |      | [ 31]         | $^2P$       | $3.776 \pm 0.007$ | 2024 | NR, neural network QMC, DS (DeepSolid) method |
| 17 | Cl   | [ 59]         | $^2P$       | 14.71             | 1976 | NR, PNO-CEPA, $M_L$ res.                      |
|    |      | [ 122]        | $^2P$       | 14.6              | 1992 | NR, CASPT2, $M_L$ res.                        |
|    |      | [ 141]        | $^2P$       | 14.73             | 2000 | NR, CASPT2, $M_L$ res.                        |
|    |      | [ 105]        | $^2P$       | 14.7              | 2004 | SIC-DFT                                       |
|    |      | [ 98]         | $^2P$       | $14.57 \pm 0.10$  | 2005 | NR, CCSD(T), $M_L$ res.                       |
|    |      | [ 4]          | --          | $14.6 \pm 0.1$    | 2019 | recommended                                   |
|    |      | [ 92]         | $^2P$       | $14.59 \pm 0.25$  | 2021 | NR, CCSD(T)                                   |
|    |      | [ 72]         | $^2P$       | 14.582            | 2021 | R, CCSD(T)                                    |
| 35 | Br   | [ 141]        | $^2P$       | 21.03             | 2000 | R, MVD, CASPT2, $M_L$ res.                    |
|    |      | [ 144]        | $^2P_{1/2}$ | 21.9              | 2002 | R, DK, SO-CI                                  |
|    |      | [ 144]        | $^2P_{3/2}$ | 21.7              | 2002 | R, DK, SO-CI, $M_J$ res.                      |
|    |      | [ 105]        | $^2P$       | 21.5              | 2004 | SIC-DFT                                       |
|    |      | [ 13,141]     | $^2P$       | $21.13 \pm 0.42$  | 2006 | R, MVD, CASPT2                                |
|    |      | [ 107]        | $^2P$       | 21.6              | 2016 | TD-DFT (LEXX)                                 |
|    |      | [ 48]         | $^2P$       | 20.4              | 2019 | NR, CCSD                                      |
|    |      | [ 4]          | --          | $21 \pm 1$        | 2019 | recommended                                   |
| 53 | I    | [ 146]        | $^2P_{3/2}$ | $32.9 \pm 1.3$    | 1997 | exp.                                          |
|    |      | [ 146][162]   | $^2P_{3/2}$ | 33.4              | 1997 | exp.                                          |
|    |      | [ 144]        | $^2P_{1/2}$ | 35.1              | 2002 | R, DK, SO-CI                                  |
|    |      | [ 144]        | $^2P_{3/2}$ | 34.1              | 2002 | R, DK, SO-CI, $M_J$ res.                      |
|    |      | [ 105]        | $^2P$       | 33.6              | 2004 | SIC-DFT                                       |
|    |      | [ 13,142,144] | $^2P_{3/2}$ | $33.0 \pm 1.7$    | 2006 | R, DK, SO-CI                                  |
|    |      | [ 107]        | $^2P$       | 30.5              | 2016 | SIC-DFT (RXH)                                 |
|    |      | [ 41]         | $^2P$       | 35.00             | 2016 | LR-CCSD                                       |
|    |      | [ 48]         | $^2P$       | 31.57             | 2019 | ECP, CCSD                                     |
|    |      | [ 4]          | --          | $32.9 \pm 1.3$    | 2019 | recommended                                   |

Continued on next page

| Z   | Atom | Refs.        | State       | $\alpha$       | Year | Comments                                            |
|-----|------|--------------|-------------|----------------|------|-----------------------------------------------------|
| 85  | At   | [ 72]        | $^2P$       | 31.101         | 2021 | R, CCSD(T)                                          |
|     |      | [ 73]        | $^2P$       | 31.114         | 2021 | R, CCSD(T)                                          |
|     |      | [ 144]       | $^2P_{1/2}$ | 45.6           | 2002 | R, DK, SO-CI                                        |
|     |      | [ 144]       | $^2P_{3/2}$ | 41.9           | 2002 | R, DK, SO-CI, $M_J$ res.                            |
|     |      | [ 13,68,137] | $^2P_{3/2}$ | $40.7 \pm 2.0$ | 2012 | R, Cowan-Griffin, HF only                           |
|     |      | [ 41]        | $^2P_{3/2}$ | 38.93          | 2016 | LR-CCSD                                             |
|     |      | [ 48]        | $^2P_{3/2}$ | 38.15          | 2019 | ECP, CCSD                                           |
|     |      | [ 4]         | —           | $42 \pm 4$     | 2019 | recommended                                         |
|     |      | [ 138]       | $^2P_{3/2}$ | 40.4           | 2022 | R (ZORA), DFT (B3LYP)                               |
| 117 | Ts   | [ 130]       | $^2P_{3/2}$ | 41.1           | 2023 | R (ATZP-ZORA), DFT (B3LYP)                          |
|     |      | [ 139]       | $^2P_{3/2}$ | 52.24          | 2014 | Estimated via correlation with $R_{\max}(np_{3/2})$ |
|     |      | [ 145]       | $^2P_{3/2}$ | 76.3           | 2017 | empirical estimate                                  |
|     |      | [ 4]         | —           | $76 \pm 15$    | 2019 | recommended                                         |

## S4.8 Group 18 elements

The most accurate theoretical and experimental values for Group 18 elements are collected in Table S25 to validate the results in this work. Only computational and experimental values close to the recommended values in Ref. 4 are compared. Only values computed with CCSD(T) methods in the literature are considered.

The NR, SR, and DC values are 1.38 for He in this work, which align well with the experimental values<sup>147–150</sup> and other theoretical values.<sup>150–153</sup> The deviation is mainly attributed to the  $\Delta_{\text{others}}$ , including Breit and QED effects, among others.

The relativistic effects on dipole polarizabilities for Kr are small. Therefore, all NR, SR, and DC values (16.78, 16.77, and 16.80, respectively) for Kr are in good agreement with the experimental values ( $16.766 \pm 0.008$ ,<sup>154</sup>  $16.782 \pm 0.005$ ,<sup>155</sup>  $16.740$ ,<sup>156,157</sup> and  $16.734$ <sup>156</sup>). The SR value also agrees well with the theoretical values ( $16.80 \pm 0.13$ <sup>157</sup> and  $16.736$ <sup>158</sup>) obtained using scalar-relativistic CCSD(T) methods in the literature. The DC value is also close to the recent MBPT value (16.800) including the Gaunt contribution.<sup>52</sup>

The DC value (27.20) for Xe is in good agreement with the experimental values (27.342,<sup>159</sup>  $27.078 \pm 0.050$ ,<sup>155</sup> and  $27.292$ <sup>156</sup>). The SR value (27.01) is also close to other computational



values ( $27.06 \pm 0.27$ ,<sup>160</sup>  $27.2937 \pm 0.0003$ ,<sup>161</sup>  $27.42$ ,<sup>162</sup>  $28.4 \pm 0.5$ ,<sup>88</sup> and  $27.508$ <sup>163</sup>).

There is no experimental data available for comparison for Rn in the literature. The DC value (35.07) for Rn is in excellent agreement with other computational DC results ( $35.04 \pm 1.8$ ,<sup>68,101</sup>  $35.0$ ,<sup>118</sup>  $35.3$ ,<sup>164</sup> and  $35.53 \pm 0.36$ <sup>165</sup>) in the literature.

There is no experimental data available for comparison for Og in the literature. The DC value (58.24) for Og in this work is in excellent agreement with other computational DC results ( $57.98$ <sup>166</sup> and  $56.5 \pm 1.8$ <sup>165</sup>). Moreover, it is observed that the hyperpolarizability using Eq. (S1) for Og is negative in this work. Therefore, the values fitted using Eq. (S3) are also computed, and the NR, SR, and DC values are 45.28, 43.77, and  $57.90 \pm 0.06$ , respectively, as shown in Table S17.

Jerabek *et al.* reported NR, SR, and DC values for Og, using the same method and basis set as in this work, as 45.30, 43.78, and 57.98, respectively. The Gaunt contribution is also included in the DC value. In Ref. 166, the numerical differentiation method is used, and only  $\alpha$  is fitted.<sup>127</sup> It can be seen that the NR and SR values fitted by Eq. (S3) perfectly align with the counterparts reported in Ref. 166. The difference in DC values (0.08) could be mainly attributed to the Gaunt contribution.

Additionally, the 4C Hamiltonian is used in this work, while a 2C Hamiltonian is used in Ref. 166. To study the difference due to the 2C and 4C Hamiltonians used, three test calculations were performed. The first and second calculations used a 2C Hamiltonian with 18 and 40 electrons correlated, denoted as `2C-DC-CC@dya11.acv4z@(core 18)[vir 278]` and `2C-DC-CC@dya11.acv4z@(core 40)[vir 278]`, respectively, as shown in Table S16. The CCSD(T) results fitted using Eq. (S3) are 57.86 and 57.96, respectively. The DHF values for both cases are 60.58. The third test calculation used 2C-CC with 50 electrons correlated, and the Gaunt contribution to  $\alpha$  was also evaluated at the DHF level, denoted as `2C-DC-Gaunt-CC@dya11.acv4z@(core 50)[vir 278]` in Table S16. The DHF and CCSD(T) results fitted using Eq. (S3) are 60.45 and 57.79, respectively. The difference between the CCSD(T) results of the third test and the CCSD(T) value reported in Ref. 166 is about 0.19 a.u., which could be attributed to the Gaunt contribution evaluated at the CCSD(T) level in Ref. 166. Comparing the results between the second and third calculations, the Gaunt contribution to  $\alpha$  at the DHF level is about  $-0.13$ . Therefore, the total Gaunt contribution is about 0.06, which is close to the observed difference (0.08). These tests suggest that the difference between the 2C and 4C methods is negligible, and the Gaunt contribution to  $\alpha$  is also small.

Table S25: Summary of reference atomic dipole polarizabilities (in a.u.) for Group 18 elements, as reported in Refs. 4 and 5. Comment definitions are provided in these references.

| Z  | Atom | Refs.          | State   | $\alpha$                       | Year | Comments                                                                                          |
|----|------|----------------|---------|--------------------------------|------|---------------------------------------------------------------------------------------------------|
| 2  | He   | [ 147,148]     | $^1S_0$ | $1.383746 \pm 0.000007$        | 1992 | exp.                                                                                              |
|    |      | [ 151]         | $^1S_0$ | 1.383191                       | 2000 | R, Dirac, Breit-Pauli, QED, mass pol, correlated basis ( $^4\text{He}$ )                          |
|    |      | [ 152]         | $^1S_0$ | $1.38376079 \pm 0.00000023$    | 2004 | R, Dirac, Breit-Pauli, QED, mass pol, exponentially correlated Slater functions ( $^4\text{He}$ ) |
|    |      | [ 149]         | $^1S_0$ | $1.383759 \pm 0.000013$        | 2007 | exp.                                                                                              |
|    |      | [ 167]         | $^1S_0$ | $1.3837295330 \pm 0.000000001$ | 2016 | R, Dirac, Breit, QED, recoil, ... ( $^4\text{He}$ )                                               |
|    |      | [ 150]         | $^1S_0$ | $1.3837616 \pm 0.0000027$      | 2018 | exp.                                                                                              |
|    |      | [ 4]           | $^1S_0$ | $1.38375 \pm 0.00002$          | 2019 | recommended                                                                                       |
|    |      | [ 153]         | $^1S_0$ | $1.38376078 \pm 0.00000014$    | 2020 | R, Dirac, Breit-Pauli, QED + finite nuclear size correction                                       |
| 10 | Ne   | [ 90]          | $^1S$   | 2.676                          | 1976 | NR, PNNO-CEPA, $M_L$ res.                                                                         |
|    |      | [ 155]         | $^1S_0$ | $2.6669 \pm 0.0008$            | 1991 | exp.                                                                                              |
|    |      | [ 168]         | $^1S$   | 2.68                           | 1992 | NR, CCSD(T)                                                                                       |
|    |      | [ 156]         | $^1S_0$ | 2.663                          | 1997 | exp.                                                                                              |
|    |      | [ 161]         | $^1S_0$ | $2.66053 \pm 0.00001$          | 2001 | CCSD(T), ECP                                                                                      |
|    |      | [ 169]         | $^1S$   | 2.665                          | 2003 | NR, CC3                                                                                           |
|    |      | [ 160,169,170] | $^1S$   | 2.666                          | 2003 | R, CC3 + FCI + DK3 correction                                                                     |
|    |      | [ 13]          | $^1S_0$ | $2.661 \pm 0.005$              | 2006 | R, CCSD(T)                                                                                        |
|    |      | [ 171]         | $^1S_0$ | $2.66110 \pm 0.00003$          | 2010 | exp.                                                                                              |
|    |      | [ 154,172]     | $^1S_0$ | $2.677 \pm 0.070$              | 2012 | R, Dirac-Coulomb, non-linear PRCC                                                                 |
|    |      | [ 150]         | $^1S_0$ | $2.6610570 \pm 0.0000064$      | 2018 | exp.                                                                                              |
|    |      | [ 4]           | —       | $2.66110 \pm 0.00003$          | 2019 | recommended                                                                                       |
|    |      | [ 173]         | $^1S_0$ | $2.66080 \pm 0.00036$          | 2020 | R, QED, AE-CCSD(T), finite nucl. mass & size corrections                                          |
|    |      | [ 92]          | $^1S$   | $2.662 \pm 0.034$              | 2021 | NR, CCSD(T)                                                                                       |
|    |      | [ 174]         | $^1S_0$ | $2.661067 \pm 0.000077$        | 2022 | R, QED, AE-CCSDT(Q), finite nucl. mass & size corrections                                         |
|    |      | [ 123]         | $^1S_0$ | $2.661 \pm 0.005$              | 2023 | R, CCSD(T)                                                                                        |
| 18 | Ar   | [ 147]         | $^1S_0$ | $11.083 \pm 0.002$             | 1965 | exp.                                                                                              |
|    |      | [ 154]         | $^1S_0$ | $11.081 \pm 0.005$             | 1967 | exp.                                                                                              |
|    |      | [ 159]         | $^1S_0$ | 11.091                         | 1969 | exp.                                                                                              |
|    |      | [ 59]          | $^1S$   | 11.10                          | 1976 | NR, PNO-CEPA                                                                                      |
|    |      | [ 157,175]     | $^1S_0$ | $11.070 \pm 0.007$             | 1990 | exp.                                                                                              |
|    |      | [ 156]         | $^1S_0$ | 11.080                         | 1997 | exp.                                                                                              |
|    |      | [ 161]         | $^1S$   | $11.08401 \pm 0.00004$         | 2001 | NR, CCSD(T)                                                                                       |
|    |      | [ 160,161]     | $^1S$   | 11.10                          | 2001 | R, CCSD(T) + DK3 correction                                                                       |
|    |      | [ 136]         | $^1S$   | 11.1                           | 2004 | R, DK, CASPT2                                                                                     |
|    |      | [ 13]          | $^1S_0$ | $11.078 \pm 0.010$             | 2006 | exp.                                                                                              |

Continued on next page

| Z  | Atom | Refs.       | State   | $\alpha$               | Year | Comments                                                               |
|----|------|-------------|---------|------------------------|------|------------------------------------------------------------------------|
| 36 | Kr   | [ 13,68,98] | $^1S$   | $11.085 \pm 0.060$     | 2012 | R, CCSD(T)                                                             |
|    |      | [ 47]       | $^1S$   | $11.089 \pm 0.004$     | 2013 | R, CCSD(T)                                                             |
|    |      | [ 150]      | $^1S_0$ | $11.07718 \pm 0.00064$ | 2018 | exp.                                                                   |
|    |      | [ 4]        | —       | $11.083 \pm 0.007$     | 2019 | recommended                                                            |
|    |      | [ 92]       | $^1S$   | $11.08 \pm 0.19$       | 2021 | NR, CCSD(T)                                                            |
|    |      | [ 176]      | $^1S$   | $11.0775 \pm 0.0019$   | 2023 | R, DKH2, CCSD(T) + Breit-Pauli<br>+ QED + finite nuclear mass and size |
|    |      | [ 154]      | $^1S_0$ | $16.766 \pm 0.008$     | 1967 | exp.                                                                   |
|    |      | [ 157]      | $^1S$   | $16.80 \pm 0.13$       | 1990 | R, DK3, CCSD(T)                                                        |
|    |      | [ 155]      | $^1S_0$ | $16.782 \pm 0.005$     | 1991 | exp.                                                                   |
|    |      | [ 177]      | $^1S_0$ | 16.79                  | 1992 | DOSD (constrained dipole oscillator strength distribution)             |
|    |      | [ 156,157]  | $^1S_0$ | 16.740                 | 1997 | exp.                                                                   |
|    |      | [ 156]      | $^1S_0$ | 16.734                 | 1997 | exp.                                                                   |
|    |      | [ 136]      | $^1S$   | 16.6                   | 2004 | R, DK, CASPT2                                                          |
|    |      | [ 178]      | $^1S_0$ | 16.012                 | 2009 | R, Dirac, CCSD/T                                                       |
| 54 | Xe   | [ 158]      | $^1S_0$ | 16.736                 | 2012 | R, DK3, CCSD(T)                                                        |
|    |      | [ 86]       | $^1S_0$ | 16.47                  | 2016 | R, RPA, PolPot                                                         |
|    |      | [ 4]        | —       | $16.78 \pm 0.02$       | 2019 | recommended                                                            |
|    |      | [ 52]       | $^1S_0$ | 16.800                 | 2020 | R, DHF, MBPT                                                           |
|    |      | [ 159]      | $^1S_0$ | 27.342                 | 1969 | exp.                                                                   |
|    |      | [ 155]      | $^1S_0$ | $27.078 \pm 0.050$     | 1991 | exp.                                                                   |
|    |      | [ 177]      | $^1S_0$ | 27.16                  | 1992 | DOSD (constrained dipole oscillator strength distribution)             |
|    |      | [ 156]      | $^1S_0$ | 27.292                 | 1997 | exp.                                                                   |
|    |      | [ 179]      | $^1S_0$ | 27.36                  | 1998 | R, SOPP, CCSD(T) + MP2 basis set correction                            |
|    |      | [ 160]      | $^1S$   | $27.06 \pm 0.27$       | 2001 | R, DK3, CCSD(T)                                                        |
|    |      | [ 161]      | $^1S_0$ | $27.2937 \pm 0.0003$   | 2001 | CCSD(T), ECP                                                           |
|    |      | [ 136]      | $^1S$   | 26.7                   | 2004 | R, DK, CASPT2                                                          |
|    |      | [ 178]      | $^1S_0$ | 25.297                 | 2009 | R, Dirac, CCSD/T                                                       |
|    |      | [ 162]      | $^1S_0$ | 27.42                  | 2010 | R, DK3, CCSD(T)                                                        |
|    |      | [ 158]      | $^1S_0$ | 26.432                 | 2012 | R, DK3, CCSD                                                           |
|    |      | [ 86]       | $^1S_0$ | 26.7                   | 2016 | R, RPA, PolPot                                                         |
|    |      | [ 107]      | $^1S_0$ | 25.4                   | 2016 | SIC-DFT (RXH)                                                          |
|    |      | [ 41]       | $^1S_0$ | 27.30                  | 2016 | LR-CCSD                                                                |
|    |      | [ 88]       | $^1S_0$ | $28.4 \pm 0.5$         | 2018 | R, CCSD(T)                                                             |
|    |      | [ 163]      | $^1S_0$ | 27.508                 | 2018 | R, CCSD(T)                                                             |
|    |      | [ 48]       | $^1S_0$ | 26.6                   | 2019 | ECP, CCSD                                                              |
|    |      | [ 4]        | —       | $27.32 \pm 0.20$       | 2019 | recommended                                                            |
|    |      | [ 52]       | $^1S_0$ | 27.099                 | 2020 | R, DHF, MBPT                                                           |

Continued on next page

| Z   | Atom | Refs.      | State   | $\alpha$             | Year | Comments                                    |
|-----|------|------------|---------|----------------------|------|---------------------------------------------|
| 86  | Rn   | [ 180]     | $^1S_0$ | $27.55 \pm 0.30$     | 2023 | CCSD + hyperfine-induced contributions      |
|     |      | [ 179]     | $^1S_0$ | 34.33                | 1998 | R, SOPP, CCSD(T) + MP2 basis set correction |
|     |      | [ 179]     | $^1S_0$ | 34.60                | 1998 | R, SOPP, CCSD(T) + MP2 basis set correction |
|     |      | [ 160]     | $^1S$   | 33.18                | 2001 | R, DK3, CCSD(T)                             |
|     |      | [ 161]     | $^1S_0$ | $34.4374 \pm 0.0001$ | 2001 | CCSD(T), ECP                                |
|     |      | [ 136]     | $^1S$   | 32.6                 | 2004 | R, DK, CASPT2                               |
|     |      | [ 78,124]  | $^1S_0$ | $36 \pm 5$           | 2004 | R, Dirac, LDA                               |
|     |      | [ 126]     | $^1S_0$ | 28.6                 | 2005 | R, SOPP, CCSD(T)                            |
|     |      | [ 181,182] | $^1S_0$ | 35.77                | 2005 | R, DK, CCSD(T)                              |
|     |      | [ 182]     | $^1S_0$ | 35.47                | 2005 | CCSD, ECP                                   |
|     |      | [ 158]     | $^1S_0$ | 35.391               | 2012 | R, RPA, PolPot                              |
|     |      | [ 183]     | $^1S_0$ | 35.87                | 2012 | R, DFT, DC, PBE38                           |
|     |      | [ 184]     | $^1S_0$ | 34.89                | 2012 | R, DKH2, B3LYP, SARC                        |
|     |      | [ 184]     | $^1S_0$ | 34.70                | 2012 | R, DKH2, B3LYP, UGBS                        |
|     |      | [ 183]     | $^1S_0$ | 33.62                | 2012 | R, DFT, sfDC, PBE38                         |
|     |      | [ 68,101]  | $^1S_0$ | $35.04 \pm 1.8$      | 2012 | R, Dirac, CCSD(T)                           |
|     |      | [ 118]     | $^1S_0$ | 35.0                 | 2015 | R, Dirac, CCSD(T)                           |
|     |      | [ 86]      | $^1S_0$ | 34.2                 | 2016 | R, RPA, PolPot                              |
|     |      | [ 109]     | $^1S_0$ | 32.2                 | 2016 | TD-DFT (LEXX)                               |
|     |      | [ 41]      | $^1S_0$ | 33.54                | 2016 | LR-CCSD                                     |
|     |      | [ 88,164]  | $^1S_0$ | $37.0 \pm 0.5$       | 2018 | R, CCSD(T)                                  |
|     |      | [ 164]     | $^1S_0$ | 35.3                 | 2018 | R, Dirac-Gaunt, CCSD(T)                     |
|     |      | [ 185]     | $^1S_0$ | 35.00                | 2018 | R, RPA                                      |
|     |      | [ 48]      | $^1S_0$ | 32.8                 | 2019 | ECP, CCSD                                   |
|     |      | [ 4]       | —       | $35 \pm 2$           | 2019 | recommended                                 |
|     |      | [ 89]      | $^1S_0$ | 35                   | 2020 | R, RPA                                      |
|     |      | [ 52]      | $^1S_0$ | 34.66                | 2020 | R, DHF, MBPT                                |
|     |      | [ 186]     | $^1S_0$ | 36.14                | 2020 | R, DK, CCSD(T)                              |
|     |      | [ 165]     | $^1S_0$ | $35.53 \pm 0.36$     | 2021 | PRCC(T)+Breit+QED                           |
|     |      | [ 138]     | $^1S_0$ | 34.6                 | 2022 | R (ZORA), DFT (B3LYP)                       |
|     |      | [ 130]     | $^1S_0$ | 30.9                 | 2023 | R (ATZP-ZORA), DFT (B3LYP)                  |
| 118 | Og   | [ 126]     | $^1S_0$ | 52.4                 | 2005 | R, SOPP, CCSD(T)                            |
|     |      | [ 101]     | $^1S_0$ | 46.33                | 2008 | R, Dirac, CCSD(T)                           |
|     |      | [ 86]      | $^1S_0$ | 59.0/57.2            | 2016 | R, RPA, PolPot                              |
|     |      | [ 86]      | $^1S_0$ | $57 \pm 3$           | 2016 | R, RPA, PolPot                              |
|     |      | [ 166]     | $^1S_0$ | 57.98                | 2018 | R, Dirac + Gaunt, CCSD(T)                   |
|     |      | [ 4]       | —       | $58 \pm 6$           | 2019 | recommended                                 |
|     |      | [ 165]     | $^1S_0$ | $56.5 \pm 1.8$       | 2021 | PRCC(T)+Breit+QED                           |

## S5 Uncertainty estimation

### S5.1 Group 1 elements

The uncertainty excluding  $\Delta P_{\text{fitting}}$  is estimated for all Group 1 elements. In general, the errors due to  $\Delta P_{\text{core}}$  and  $\Delta P_{\text{vir}}$  are not estimated explicitly. They are included implicitly in the error due to  $\Delta P_{\text{basis}}$ . Several SR test calculations were performed for basis sets using ANO-RCC and d-aug-ANO-RCC, compared to the results with s-aug-ANO-RCC.

In SR-CC calculations of Li, as shown in Table S1, the results for CCSD(T) with ANO-RCC, s-aug-ANO-RCC, and d-aug-ANO-RCC are 164.30, 164.29, and 164.28 a.u., respectively, suggesting that the error due to using the s-aug-ANO-RCC basis set is about 0.01 a.u., with half of it taken as the error due to  $\Delta P_{\text{basis}}$ . With the s-aug-ANO-RCC basis set, the difference ( $\Delta P_{(\text{T})}$ ) between CCSD and CCSD(T) values in DC-CC calculations is 0.07 a.u., with half of it taken as the error due to  $\Delta P_{(\text{T})}$ . To be conservative, I take the difference between this study and the recommended value as the error, i.e., 0.20 a.u., which is mainly due to neglecting other relativistic and higher-order correlation effects ( $\Delta P_{\text{others}}$ ). In conclusion, the error of 0.21 a.u. in this study for Li is acceptable.

In SR-CC calculations of Na, as shown in Table S1, the results for CCSD(T) with ANO-RCC, s-aug-ANO-RCC, and d-aug-ANO-RCC are 163.00, 162.99, and 162.97 a.u., respectively, suggesting that the error due to using s-aug-ANO-RCC basis set is about 0.02 a.u., with half of it taken as the error due to  $\Delta P_{\text{basis}}$ . With the s-aug-ANO-RCC basis set, the difference ( $\Delta P_{(\text{T})}$ ) between CCSD and CCSD(T) values in DC-CC calculations is 1.11 a.u., with half of it taken as the error due to  $\Delta P_{(\text{T})}$ . To be conservative, the difference between this study and the recommended value is taken as the error, i.e., 0.57 a.u., which is mainly due to neglecting other relativistic and higher-order correlation effects, i.e.,  $\Delta P_{\text{others}}$ . In conclusion, the error of 0.80 a.u. in this study for Na is acceptable.

In SR-CC calculations of K, the results for CCSD(T) with ANO-RCC, s-aug-ANO-RCC, and d-aug-ANO-RCC are 284.74, 289.96, and 290.93 a.u., respectively, suggesting that the

error due to using the s-aug-ANO-RCC basis set is about 0.97. To be conservative, it is taken as the error due to  $\Delta P_{\text{basis}}$ . With the s-aug-ANO-RCC basis set, the difference ( $\Delta P_{(\text{T})}$ ) between CCSD and CCSD(T) values in DC-CC calculations is 12.19 a.u., which is much higher than the difference between the recommended value and the DC result in this work, i.e., 0.94 a.u. To be conservative, I take twice the latter difference as the error due to neglecting other relativistic and higher-order correlation effects ( $\Delta P_{\text{others}}$ ). In conclusion, the error of 2.12 a.u. in this study for K is acceptable.

In SR-CC calculations of Rb, the results for CCSD(T) with ANO-RCC, s-aug-ANO-RCC, and d-aug-ANO-RCC are 314.32, 319.34, and 319.89 a.u., respectively, suggesting that the error due to using the s-aug-ANO-RCC basis set is about 0.55 a.u., which is therefore taken as the error due to finite basis sets. To be conservative, I take twice the difference between the recommended value and the DC results in this work, 0.56 a.u. in total, as the error due to neglecting other relativistic and higher-order correlation effects ( $\Delta P_{\text{others}}$ ). In conclusion, the error of 0.78 a.u. in this study for Rb is acceptable.

For Cs, I performed DC-CC calculations with d-aug-ANO-RCC, and the CCSD(T) result is  $398.16 \pm 0.33$ , which agrees well with the value evaluated at the CCSD(T)/s-aug-ANO-RCC level ( $398.24 \pm 0.34$ ). The difference of 0.08 between these two basis sets suggests that the result is converged with the ANO-RCC basis set for  $\alpha$  calculations. I therefore take the difference between the results with s-aug-ANO-RCC and Fægri basis sets as the error due to the finite basis sets ( $\Delta P_{\text{basis}}$ ), i.e., 1.28 a.u. Based on the calculations with different fitting procedures used, the numerical errors of 2.35 a.u. are added as the error due to other effects. In conclusion, the error of 2.68 a.u. in this study for Cs is acceptable.

In SR-CC calculations of Fr, the results for CCSD(T) with ANO-RCC, s-aug-ANO-RCC, and d-aug-ANO-RCC are 318.72, 319.36, and 319.21 a.u., respectively, suggesting that the error due to using the s-aug-ANO-RCC basis set is about 0.15 a.u., which is taken as the error due to finite basis sets. To be conservative, I take twice the difference between the recommended value and the DC results in this work (0.40 a.u.) as the error due to neglecting

other relativistic and higher-order correlation effects ( $\Delta P_{\text{others}}$ ). In conclusion, the error of 0.81 a.u. in this study for Fr is acceptable. The recommended values, obtained from the most accurate calculations with total uncertainty, including the corresponding  $\Delta P_{\text{fitting}}$ , are listed in Table 1. It should be noted that for K, the DC CCSD(T) result obtained using Eq. (S3) is taken as the recommended value, as shown in Table S15.

## S5.2 Group 2 elements

The uncertainty excluding  $\Delta P_{\text{fitting}}$  is estimated for all Group 2 elements. Considering the number of core electrons and virtual shells is similar as used for heavy atoms in the previous work,<sup>51</sup> the errors due to  $\Delta P_{\text{core}}$  and  $\Delta P_{\text{vir}}$  are not estimated explicitly. They are included implicitly in the error due to  $\Delta P_{\text{basis}}$ . Several SR test calculations were performed for basis sets using dyall.cv4z and s-aug-dyall.cv4z, compared to the results with d-aug-dyall.cv4z. The Gaunt contribution, based on Ref. 52, is considered the main source of the error due to  $P_{\text{others}}$ .

In SR-CC calculations of Be, as shown in Table S2, the results for CCSD(T) with dyall.cv4z, s-aug-dyall.cv4z, and d-aug-dyall.cv4z are 36.93, 37.78, and 37.79 a.u., respectively, suggesting that the convergence of  $\alpha$  with the dyall.cv4z family basis set is reached. Therefore, the error due to the finite basis set,  $\Delta P_{\text{basis}}$ , can be approximated as the difference of SR values (0.1 a.u.) between this work and Ref. 49. Based on Ref. 52, the Gaunt contribution is less than 0.01 a.u. and negligible. Additionally, the error of 0.1 a.u. is also larger than the difference between the DC value and the recommended value in Ref. 4. In conclusion, the error of 0.1 a.u. in this study for Be is acceptable.

In SR-CC calculations of Mg, as shown in Table S2, the results for CCSD(T) with dyall.cv4z, s-aug-dyall.cv4z, and d-aug-dyall.cv4z are 70.64, 71.20, and 71.20 a.u., respectively, suggesting that the convergence of  $\alpha$  with the dyall.cv4z family basis set is reached. Therefore, the error due to the finite basis set,  $\Delta P_{\text{basis}}$ , can be approximated as the difference of SR values (0.05 a.u.) between this work and Ref. 49. Based on Ref. 52, the Gaunt

contribution is less than 0.02 a.u. Additionally, the difference between CCSD and CCSD(T) is 0.63 a.u., with half of it taken as the error due to  $\Delta P_{(T)}$  and higher-order correlation. In conclusion, the error of 0.32 a.u. in this study for Mg is acceptable.

In SR-CC calculations of Ca, as shown in Table S2, the results for CCSD(T) with dyall.cv4z, s-aug-dyall.cv4z, and d-aug-dyall.cv4z are 156.19, 157.61, and 157.61 a.u., respectively, suggesting that the convergence of  $\alpha$  with the dyall.cv4z family basis set is reached. However, the difference in the most accurate SR values between this study and Ref. 49 is negligible. Therefore, the error due to the finite basis set,  $\Delta P_{\text{basis}}$ , is approximated as the difference in NR values (0.09 a.u.) between this work and Ref. 49. Based on Ref. 52, the Gaunt contribution is less than 0.03 a.u. Additionally, the difference between CCSD and CCSD(T) is 2.84 a.u., with half of it taken as the error due to  $\Delta P_{(T)}$  and higher-order correlation. In conclusion, the error of 1.42 a.u. in this study for Ca is acceptable.

In SR-CC calculations of Sr, as shown in Table S2, the results for CCSD(T) with dyall.cv4z, s-aug-dyall.cv4z, and d-aug-dyall.cv4z are 197.45, 197.82, and 197.78 a.u., respectively, suggesting that the convergence of  $\alpha$  with the dyall.cv4z family basis set is reached. Considering the large difference between all-electron and ECP methods, the SR values in Ref. 49 are not used in uncertainty estimation for Sr, Ba, and Ra in this work. The SR CCSD(T) difference (0.04 a.u.) between s-aug-dyall.cv4z and d-aug-dyall.cv4z is approximately taken as the error due to the finite basis set. Based on Ref. 52, the Gaunt contribution is less than 0.04 a.u. Additionally, the difference between CCSD and CCSD(T) is 4.62 a.u., with half of it taken as the error due to  $\Delta P_{(T)}$  and higher-order correlation. In conclusion, the error of 2.31 a.u. in this study for Sr is acceptable.

In SR-CC calculations of Ba, as shown in Table S2, the results for CCSD(T) with dyall.cv4z, s-aug-dyall.cv4z, and d-aug-dyall.cv4z are 272.83, 273.96, and 273.46 a.u., respectively, suggesting that the convergence of  $\alpha$  with the dyall.cv4z family basis set is reached. The SR CCSD(T) difference (0.50 a.u.) between s-aug-dyall.cv4z and d-aug-dyall.cv4z is approximately taken as the error due to the finite basis set. Based on Ref. 52, the Gaunt



contribution is less than 0.46 a.u. Additionally, the difference between CCSD and CCSD(T) is 8.18 a.u., with half of it taken as the error due to  $\Delta P_{(T)}$  and higher-order correlation. In conclusion, the error of 4.15 a.u. in this study for Ba is acceptable.

In SR-CC calculations of Ra, as shown in Table S2, the results for CCSD(T) with dyall.cv4z, s-aug-dyall.cv4z, and d-aug-dyall.cv4z are 246.22, 247.69, and 247.20 a.u., respectively, suggesting that the convergence of  $\alpha$  with the dyall.cv4z family basis set is reached. The SR CCSD(T) difference (0.49 a.u.) between s-aug-dyall.cv4z and d-aug-dyall.cv4z is approximately taken as the error due to the finite basis set. Based on Ref. 52, the Gaunt contribution is less than 1.88 a.u. Additionally, the difference between CCSD and CCSD(T) is 9.02 a.u., with half of it taken as the error due to  $\Delta P_{(T)}$  and higher-order correlation. In conclusion, the error of 4.91 a.u. in this study for Ra is acceptable. The recommended values, obtained from the most accurate calculations with total uncertainty, including the corresponding  $\Delta P_{\text{fitting}}$ , are listed in Table 1.

### S5.3 Group 13 elements

The uncertainty excluding  $\Delta P_{\text{fitting}}$  is estimated for all Group 13 elements. In general, the errors due to  $\Delta P_{\text{core}}$  and  $\Delta P_{\text{vir}}$  are not estimated explicitly. They are included implicitly in the error due to  $\Delta P_{\text{basis}}$ .

For B, the difference between the computed NR value (20.41) and the result (20.480) in Ref. 91 is used as the error due to the finite basis set ( $\Delta P_{\text{basis}}$ ). The differences ( $\Delta P_{(T)}$ ) between CCSD and CCSD(T) values in NR-CC and SR-CC calculations are 0.04 and 0.02 a.u., respectively, with the larger one taken as the error due to  $\Delta P_{(T)}$ . The contribution due to the full DC relativistic effect is about 0.05 a.u. between NR-CC and DC-CI for the ground state of B. This value is employed as the error due to  $\Delta P_{\text{others}}$ . In conclusion, the error of 0.09 a.u. in this study for B is acceptable.

For Al, the uncertainty of the DC value due to fitting Eq. (S1) is 1.75 a.u., which is much higher than the uncertainty (1.0 a.u.) recommended in Ref. 4. Therefore, the error of 1.75

a.u. in this study for Al is acceptable.

For Ga, the difference ( $\Delta P_{(T)}$ ) between CCSD and CCSD(T) values in the DC-CC calculation is 1.1 a.u., which is taken as the error due to  $\Delta P_{(T)}$  and truncating higher-order correlation. The Gaunt contribution at the CCSD(T) level is 0.18 a.u. based on Ref. 99, which is therefore employed as the error due to  $\Delta P_{\text{others}}$ . The error due to the finite basis set is taken as 0.50% of the DC-CC value as in Ref. 99. The difference in DC CCSD values (0.03 a.u.) between this work and Ref. 99 is treated as the error due to  $\Delta P_{\text{core}}$  and  $\Delta P_{\text{vir}}$ . In conclusion, the error of 1.15 a.u. in this study for Ga is acceptable, which is close to the uncertainty of 1.5 a.u. reported in Ref. 99.

For In, the difference ( $\Delta P_{(T)}$ ) between CCSD and CCSD(T) values in the DC-CC calculation is 1.75 a.u., which is taken as the error due to  $\Delta P_{(T)}$  and truncating higher-order correlation. The Gaunt contribution at the CCSD(T) level is not available in Ref. 99, and 0.72 a.u. for Tl is employed as the error due to  $\Delta P_{\text{others}}$  for In. The error due to the finite basis set is empirically taken as 0.50% of the DC-CC value as in Ref. 99. The difference in DC CCSD(T) values (0.08 a.u.) between this work and Ref. 99 is treated as the error due to  $\Delta P_{\text{core}}$  and  $\Delta P_{\text{vir}}$ . In conclusion, the error of 1.92 a.u. in this study for In is acceptable, which is close to the uncertainty of 1.9 a.u. reported in Ref. 99.

For Tl, the difference ( $\Delta P_{(T)}$ ) between CCSD and CCSD(T) values in the DC-CC calculation is 0.17 a.u., which is taken as the error due to  $\Delta P_{(T)}$  and truncating higher-order correlation. The Gaunt contribution at the CCSD(T) level is 0.72 a.u. based on Ref. 99, which is employed as the error due to  $\Delta P_{\text{others}}$ . The error due to the finite basis set is empirically taken as 0.50% of the DC-CC value as in Ref. 99. The difference in CCSD(T) values (0.68 a.u.) between DC-CC calculations correlating 13 and 35 electrons is treated as the error due to  $\Delta P_{\text{core}}$  and  $\Delta P_{\text{vir}}$ . In conclusion, the error of 1.03 a.u. in this study for Tl is acceptable, which is smaller than the uncertainty of 1.6 a.u. reported in Ref. 99.

For Nh, the difference ( $\Delta P_{(T)}$ ) between CCSD and CCSD(T) values in the DC-CC calculation is 0.51 a.u., which is taken as the error due to  $\Delta P_{(T)}$  and truncating higher-order

correlation. The Gaunt contribution at the CCSD(T) level is not available in Ref. 99; thus, 1.50 a.u. is taken as the error due to  $\Delta P_{\text{others}}$  for Nh. The difference in CCSD values (0.02 a.u.) between two-component DC-CC calculations correlating 49 and 51 electrons is treated as the error due to the finite basis set. The difference in CCSD(T) values (0.10 a.u.) between DC-CC calculations correlating 35 and 49 electrons is treated as the error due to  $\Delta P_{\text{core}}$  and  $\Delta P_{\text{vir}}$ . In conclusion, the error of 1.59 a.u. in this study for Nh is acceptable. The recommended values, obtained from the most accurate calculations with total uncertainty, including the corresponding  $\Delta P_{\text{fitting}}$ , are listed in Table 1.

## S5.4 Group 14 elements

The uncertainty excluding  $\Delta P_{\text{fitting}}$  is estimated for all Group 14 elements. In general, the errors due to  $\Delta P_{\text{core}}$  and  $\Delta P_{\text{vir}}$  are not estimated explicitly; they are included implicitly in the error due to  $\Delta P_{\text{basis}}$ . Considering a very similar method is employed in Ref. 120, the main difference is due to the basis sets. Therefore, the difference in DC values is taken as the error due to  $\Delta P_{\text{basis}}$  for all Group 14 elements. The  $\Delta P_{\text{(T)}}$  is quite small at the DC CCSD(T) level for all Group 14 elements, and they are 0.10,  $-0.56$ ,  $-0.72$ ,  $-0.66$ ,  $-0.02$ , and  $0.38$  for C, Si, Ge, Sn, Pb, and Fl, respectively. Therefore, the error due to  $\Delta P_{\text{(T)}}$  and higher-order correlation is approximated as the absolute value of  $\Delta P_{\text{(T)}}$ . The Gaunt contribution is also reported in Ref. 120 at the DHF level, which is employed as the main contribution to the error due to  $\Delta P_{\text{others}}$ . In conclusion, the total errors are 0.48, 0.63, 0.74, 1.01, 0.89, and 0.90 for C, Si, Ge, Sn, Pb, and Fl, respectively. The recommended values, obtained from the most accurate calculations with total uncertainty, including the corresponding  $\Delta P_{\text{fitting}}$ , are listed in Table 1.

## S5.5 Group 15 elements

The uncertainty excluding  $\Delta P_{\text{fitting}}$  is estimated for all Group 15 elements. In general, the errors due to  $\Delta P_{\text{core}}$  and  $\Delta P_{\text{vir}}$  are approximated as the difference between  $\text{SR}_n$  and

SR<sub>d</sub>. Based on the comparison with the literature, the Dyal basis set is sufficient. To be conservative, 0.5% of the most accurate results are used as the error due to  $\Delta P_{\text{basis}}$ , except for N, where 0.12 a.u. is taken.

Additionally, the  $\Delta P_{(\text{T})}$  in SR calculations is always positive and less than 0.1 a.u. for all elements except for Mc, where the  $\Delta P_{(\text{T})}$  is -0.39 a.u. Therefore, the difference between SR<sub>d</sub> and DC values is used as the error due to  $\Delta P_{(\text{T})}$  and  $\Delta P_{\text{others}}$ . In conclusion, the total errors are 0.15, 0.42, 0.66, 1.10, 2.23, and 7.69 for N, P, As, Sb, Bi, and Mc, respectively. The recommended values, obtained from the most accurate calculations with total uncertainty, including the corresponding  $\Delta P_{\text{fitting}}$ , are listed in Table 1.

## S5.6 Group 16 elements

The uncertainty excluding  $\Delta P_{\text{fitting}}$  is estimated for all Group 16 elements. In general, the errors due to  $\Delta P_{\text{core}}$  and  $\Delta P_{\text{vir}}$  are approximated as the difference between SR<sub>n</sub> and SR<sub>d</sub>. Based on the comparison with the literature, the Dyal basis set is sufficient. To be conservative, 0.5% of the DC results in Table 1 are used as the error due to  $\Delta P_{\text{basis}}$  for each atom. The difference between SR<sub>d</sub> and DC values is used as the error due to  $\Delta P_{(\text{T})}$  and  $\Delta P_{\text{others}}$ . In conclusion, the total errors are 0.04, 0.32, 1.06, 1.37, 1.28, and 14.45 for O, S, Se, Te, Po, and Lv, respectively. The recommended values, obtained from the most accurate calculations with total uncertainty, including the corresponding  $\Delta P_{\text{fitting}}$ , are listed in Table 1.

## S5.7 Group 17 elements

The uncertainty excluding  $\Delta P_{\text{fitting}}$  is estimated for all Group 18 elements. For He, Ne, and Ar, accurate results are available in the literature. Therefore, the deviation between the DC value and the recommended value in Ref. 4 is taken as the uncertainty, which is mainly due to  $\Delta P_{\text{others}}$ .

Several SR test calculations with the d-aug-dyall.acv4z basis set are performed for Kr,

Xe, Rn, and Og. Compared to the SR CCSD(T) values obtained with dyall.acv4z, the differences are about 0.01, 0.01, 0.01, and 0.13, respectively. The difference for Og with  $\alpha$  obtained using Eq. (S3) is 0.12. These values are used as the error due to the finite basis set ( $\Delta P_{\text{basis}}$ ).

The difference between 2C and 4C Hamiltonians is studied for Ne, Ar, Xe, and Rn, as shown in Table S8, where the X2C methods with the same number of correlated electrons as in 4C-CC methods are performed. The differences are 0.00, 0.01, 0.01, and 0.03 a.u., respectively. The difference for Ar and Xe is 0.01; thus, it is assumed that it is also small for Kr in this work.

The Gaunt contribution has been investigated in Ref. 52, where Gaunt contributions to  $\alpha$  are 0.0266, 0.0585, and 0.1813 for Kr, Xe, and Rn, respectively. It can be seen that the error due to 2C and 4C Hamiltonians is negligible. Therefore, only the Gaunt contribution is considered the main error due to  $\Delta P_{\text{others}}$  for Kr, Xe, and Rn. For Og, the sum of the difference (0.33) due to using fitting equations defined in Eqs. (S1) and (S3) and the Gaunt contribution (0.08) is taken as the error due to  $\Delta P_{\text{others}}$ .

The error due to  $\Delta P_{\text{core}}$  and  $\Delta P_{\text{vir}}$  is also studied for Kr, Xe, Rn, and Og. For Kr, a DC-CC calculation with 26 correlated electrons was performed compared to the most accurate calculation with 36 correlated electrons in this work; the differences at the CCSD and CCSD(T) levels are both 0.02.

For Xe, a 2C-DC calculation with 8 correlated electrons was performed compared to a 2C-DC calculation with 50 correlated electrons; the differences at the CCSD and CCSD(T) levels are 0.43 and 0.40, respectively. It should be noted that this difference is close to the difference (0.35) between the DHF and CCSD(T) values in the 2C-DC calculation with 50 correlated electrons. This implies that 50 correlated electrons are sufficient for  $\alpha$  calculations for Xe.

Similarly, for Rn, a 2C-DC calculation with 18 correlated electrons was performed compared to another 2C-DC calculation with 50 correlated electrons. The difference is about

0.01, suggesting that 50 correlated electrons are sufficient for Rn.

For Og, a difference of 0.43 is obtained when two 2C-DC CC calculations with 18 and 40 correlated electrons were performed. However, this difference is reduced to 0.01 when comparing two DC-CC calculations with 40 and 50 correlated electrons.

Moreover, the difference ( $\Delta P_{(T)}$ ) between CCSD and CCSD(T) values in the DC-CC calculation is taken as the error due to  $\Delta P_{(T)}$  and truncating higher-order correlation. They are 0.14, 0.20, 0.26, and 0.06 for Kr, Xe, Rn, and Og, respectively. The value for Og with the  $\alpha$  obtained by Eq. (S3) is 0.04. In conclusion, the errors of 0.14, 0.21, 0.32, and 0.43 for Kr, Xe, Rn, and Og, respectively, are acceptable. The recommended values, obtained from the most accurate calculations with total uncertainty, including the corresponding  $\Delta P_{\text{fitting}}$ , are listed in Table 1.

## S5.8 Group 18 elements

The uncertainty excluding  $\Delta P_{\text{fitting}}$  is estimated for all Group 18 elements. For He, Ne, and Ar, accurate results are available in the literature. Therefore, the deviation between the DC value and the recommended value in Ref. 4 is taken as the uncertainty, which is mainly due to  $\Delta P_{\text{others}}$ .

Several SR test calculations with the d-aug-dyall.acv4z basis set are performed for Kr, Xe, Rn, and Og. Compared to the SR CCSD(T) values obtained with dyall.acv4z, the differences are about 0.01, 0.01, 0.01, and 0.13, respectively. The difference for Og with  $\alpha$  obtained using Eq. (S3) is 0.12. These values are used as the error due to the finite basis set ( $\Delta P_{\text{basis}}$ ).

The difference between 2C and 4C Hamiltonians is studied for Ne, Ar, Xe, and Rn, as shown in Table S8, where the X2C methods with the same number of correlated electrons as in 4C-CC methods are performed. The differences are 0.00, 0.01, 0.01, and 0.03 a.u., respectively. The difference for Ar and Xe is 0.01; thus, it is assumed that it is also small for Kr in this work.

The Gaunt contribution has been investigated in Ref. 52, where Gaunt contributions to  $\alpha$  are 0.0266, 0.0585, and 0.1813 for Kr, Xe, and Rn, respectively. It can be seen that the error due to 2C and 4C Hamiltonians is negligible. Therefore, only the Gaunt contribution is considered the main error due to  $\Delta P_{\text{others}}$  for Kr, Xe, and Rn. For Og, the sum of the difference (0.33) due to using fitting equations defined in Eqs. (S1) and (S3) and the Gaunt contribution (0.08) is taken as the error due to  $\Delta P_{\text{others}}$ .

The error due to  $\Delta P_{\text{core}}$  and  $\Delta P_{\text{vir}}$  is also studied for Kr, Xe, Rn, and Og. For Kr, a DC-CC calculation with 26 correlated electrons was performed compared to the most accurate calculation with 36 correlated electrons in this work; the differences at the CCSD and CCSD(T) levels are both 0.02.

For Xe, a 2C-DC calculation with 8 correlated electrons was performed compared to a 2C-DC calculation with 50 correlated electrons; the differences at the CCSD and CCSD(T) levels are 0.43 and 0.40, respectively. It should be noted that this difference is close to the difference (0.35) between the DHF and CCSD(T) values in the 2C-DC calculation with 50 correlated electrons. This implies that 50 correlated electrons are sufficient for  $\alpha$  calculations for Xe.

Similarly, for Rn, a 2C-DC calculation with 18 correlated electrons was performed compared to another 2C-DC calculation with 50 correlated electrons. The difference is about 0.01, suggesting that 50 correlated electrons are sufficient for Rn.

For Og, a difference of 0.43 is obtained when two 2C-DC CC calculations with 18 and 40 correlated electrons were performed. However, this difference is reduced to 0.01 when comparing two DC-CC calculations with 40 and 50 correlated electrons.

Moreover, the difference ( $\Delta P_{\text{(T)}}$ ) between CCSD and CCSD(T) values in the DC-CC calculation is taken as the error due to  $\Delta P_{\text{(T)}}$  and truncating higher-order correlation. They are 0.14, 0.20, 0.26, and 0.06 for Kr, Xe, Rn, and Og, respectively. The value for Og with the  $\alpha$  obtained by Eq. (S3) is 0.04. In conclusion, the errors of 0.14, 0.21, 0.32, and 0.43 for Kr, Xe, Rn, and Og, respectively, are acceptable. The recommended values, obtained from

the most accurate calculations with total uncertainty, including the corresponding  $\Delta P_{\text{fitting}}$ , are listed in Table 1.

## References

- (1) Das, A. K.; Thakkar, A. J. Static Response Properties of Second-Period Atoms: Coupled Cluster Calculations. *J. Phys. B At. Mol. Opt. Phys.* **1998**, *31*, 2215.
- (2) Kassimi, N. E.-B.; Thakkar, A. J. Static hyperpolarizability of atomic lithium. *Physical Review A* **1994**, *50*, 2948–2952, Publisher: American Physical Society.
- (3) KRCI. [https://www.diracprogram.org/doc/release-18/manual/wave\\_function/krci.html?highlight=krci#ciroots](https://www.diracprogram.org/doc/release-18/manual/wave_function/krci.html?highlight=krci#ciroots), Accessed: 2024-06-04.
- (4) Schwerdtfeger, P.; Nagle, J. K. 2018 Table of Static Dipole Polarizabilities of the Neutral Elements in the Periodic Table. *Mol. Phys.* **2019**, *117*, 1200–1225.
- (5) Schwerdtfeger, P.; Nagle, J. K. 2023 Table of static dipole polarizabilities of the neutral elements in the periodic table. 2023; <https://ctcp.massey.ac.nz/2023Tablepol.pdf>, Accessed on Jun 14, 2024.
- (6) Molof, R. W.; Schwartz, H. L.; Miller, T. M.; Bederson, B. Measurements of Electric Dipole Polarizabilities of the Alkali-Metal Atoms and the Metastable Noble-Gas Atoms. *Phys. Rev. A* **1974**, *10*, 1131–1140.
- (7) Miffre, A.; Jacquy, M.; Büchner, M.; Trénec, G.; Vigué, J. Measurement of the Electric Polarizability of Lithium by Atom Interferometry. *Phys. Rev. A* **2006**, *73*, 011603.
- (8) Puchalski, M.; Kędziera, D.; Pachucki, K. Lithium Electric Dipole Polarizability. *Phys. Rev. A* **2011**, *84*, 052518.



- (9) Lim, I. S.; Pernpointner, M.; Seth, M.; Laerdahl, J. K.; Schwerdtfeger, P.; Neogrady, P.; Urban, M. Relativistic Coupled-Cluster Static Dipole Polarizabilities of the Alkali Metals from Li to Element 119. *Phys. Rev. A* **1999**, *60*, 2822–2828.
- (10) Ekstrom, C. R.; Schmiedmayer, J.; Chapman, M. S.; Hammond, T. D.; Pritchard, D. E. Measurement of the Electric Polarizability of Sodium with an Atom Interferometer. *Phys. Rev. A* **1995**, *51*, 3883–3888.
- (11) Holmgren, W. F.; Revelle, M. C.; Lonij, V. P. A.; Cronin, A. D. Absolute and Ratio Measurements of the Polarizability of Na, K, and Rb with an Atom Interferometer. *Phys. Rev. A* **2010**, *81*, 053607.
- (12) Ma, L.; Indergaard, J.; Zhang, B.; Larkin, I.; Moro, R.; de Heer, W. A. Measured Atomic Ground-State Polarizabilities of 35 Metallic Elements. *Phys. Rev. A* **2015**, *91*, 010501.
- (13) Maroulis, G. *Atoms, Molecules And Clusters In Electric Fields: Theoretical Approaches To The Calculation Of Electric Polarizability*; World Scientific, 2006.
- (14) Thakkar, A. J.; Lupinetti, C. The Polarizability of Sodium: Theory and Experiment Reconciled. *Chem. Phys. Lett.* **2005**, *402*, 270–273.
- (15) Śmiałkowski, M.; Tomza, M. Highly Polar Molecules Consisting of a Copper or Silver Atom Interacting with an Alkali-Metal or Alkaline-Earth-Metal Atom. *Phys. Rev. A* **2021**, *103*, 022802.
- (16) Gregoire, M. D.; Hromada, I.; Holmgren, W. F.; Trubko, R.; Cronin, A. D. Measurements of the Ground-State Polarizabilities of Cs, Rb, and K Using Atom Interferometry. *Phys. Rev. A* **2015**, *92*, 052513.
- (17) Gregoire, M. D.; Brooks, N.; Trubko, R.; Cronin, A. D. Analysis of Polarizability Measurements Made with Atom Interferometry. *Atoms* **2016**, *4*, 21.

- (18) Derevianko, A.; Johnson, W. R.; Safronova, M. S.; Babb, J. F. High-Precision Calculations of Dispersion Coefficients, Static Dipole Polarizabilities, and Atom-Wall Interaction Constants for Alkali-Metal Atoms. *Phys. Rev. Lett.* **1999**, *82*, 3589–3592.
- (19) Badhan, V.; Kaur, S.; Arora, B.; Sahoo, B. K. Assessing Slowdown Times Due to Blackbody Friction Forces for High-Precision Experiments. *Eur. Phys. J. D* **2022**, *76*, 252.
- (20) Lim, I. S.; Schwerdtfeger, P.; Metz, B.; Stoll, H. All-Electron and Relativistic Pseudopotential Studies for the Group 1 Element Polarizabilities from K to Element 119. *J. Chem. Phys.* **2005**, *122*, 104103.
- (21) Kaur, S.; Arora, B.; Sahoo, B. K. Roles of Blackbody Friction Forces in the Rb and Cs Atom Interferometers. 2022.
- (22) Hamilton, R.; Roberts, B. M.; Scholten, S. K.; Locke, C.; Luiten, A. N.; Ginges, J. S.; Perrella, C. Experimental and Theoretical Study of Dynamic Polarizabilities in the  $S_{1/2}$ – $D_{5/2}$  Clock Transition in Rubidium-87 and Determination of Electric Dipole Matrix Elements. *Phys. Rev. Appl.* **2023**, *19*, 054059.
- (23) Borschevsky, A.; Pershina, V.; Eliav, E.; Kaldor, U. Ab Initio Studies of Atomic Properties and Experimental Behavior of Element 119 and Its Lighter Homologs. *J. Chem. Phys.* **2013**, *138*, 124302.
- (24) Faegri Jr, K. Relativistic Gaussian basis sets for the elements K – Uuo. *Theor. Chem. Acc.* **2001**, *105*, 252–258.
- (25) Aoki, T.; Sreekantham, R.; Sahoo, B. K.; Arora, B.; Kastberg, A.; Sato, T.; Ikeda, H.; Okamoto, N.; Torii, Y.; Hayamizu, T.; Nakamura, K.; Nagase, S.; Ohtsuka, M.; Nagahama, H.; Ozawa, N.; Sato, M.; Nakashita, T.; Yamane, K.; Tanaka, K. S.; Harada, K.; Kawamura, H.; Inoue, T.; Uchiyama, A.; Hatakeyama, A.; Takamine, A.; Ueno, H.;

- Ichikawa, Y.; Matsuda, Y.; Haba, H.; Sakemi, Y. Quantum Sensing of the Electron Electric Dipole Moment Using Ultracold Entangled Fr Atoms. *Quantum Sci. Technol.* **2021**, *6*, 044008.
- (26) Kaur, H.; Badhan, V.; Arora, B.; Sahoo, B. K. Determination of Quadrupolar Dispersion Coefficients of the Alkali-Metal Atoms Interacting with Different Material Media. *Phys. Rev. A* **2022**, *106*, 042813.
- (27) Komasa, J. Dipole and Quadrupole Polarizabilities and Shielding Factors of Beryllium from Exponentially Correlated Gaussian Functions. *Phys. Rev. A* **2001**, *65*, 012506.
- (28) Singer, K.; Wilkes, M. V. The Use of Gaussian (Exponential Quadratic) Wave Functions in Molecular Problems - I. General Formulae for the Evaluation of Integrals. *Proc. R. Soc. Lond. Ser. Math. Phys. Sci.* **1997**, *258*, 412–420.
- (29) Zhang, J.-Y.; Mitroy, J.; Bromley, M. W. J. Dispersion Coefficients of the Excited States of Lithium Atoms. *Phys. Rev. A* **2007**, *75*, 042509.
- (30) Johnson, W. R.; Safronova, U. I.; Derevianko, A.; Safronova, M. S. Relativistic Many-Body Calculation of Energies, Lifetimes, Hyperfine Constants, and Polarizabilities in  $^7\text{Li}$ . *Phys. Rev. A* **2008**, *77*, 022510.
- (31) Li, X.; Qian, Y.; Chen, J. Electric Polarization from a Many-Body Neural Network Ansatz. *Phys. Rev. Lett.* **2024**, *132*, 176401.
- (32) Mitroy, J.; Bromley, M. W. J. Semiempirical Calculation of van Der Waals Coefficients for Alkali-Metal and Alkaline-Earth-Metal Atoms. *Phys. Rev. A* **2003**, *68*, 052714.
- (33) Derevianko, A.; Porsev, S. G.; Babb, J. F. Electric dipole polarizabilities at imaginary frequencies for hydrogen, the alkali-metal, alkaline-earth, and noble gas atoms. *Atomic Data and Nuclear Data Tables* **2010**, *96*, 323–331.

- (34) Jiang, J.; Mitroy, J. Hyperfine Effects on Potassium Tune-out Wavelengths and Polarizabilities. *Phys. Rev. A* **2013**, *88*, 032505.
- (35) Jiang, J.; Mitroy, J.; Cheng, Y.; Bromley, M. W. J. Effective Oscillator Strength Distributions of Spherically Symmetric Atoms for Calculating Polarizabilities and Long-Range Atom–Atom Interactions. *At. Data Nucl. Data Tables* **2015**, *101*, 158–186.
- (36) Amini, J. M.; Gould, H. High Precision Measurement of the Static Dipole Polarizability of Cesium. *Phys. Rev. Lett.* **2003**, *91*, 153001.
- (37) Safronova, M. S.; Clark, C. W. Inconsistencies between Lifetime and Polarizability Measurements in  $\text{Cs}$ . *Phys. Rev. A* **2004**, *69*, 040501.
- (38) Iskrenova-Tchoukova, E.; Safronova, M. S.; Safronova, U. I. High-Precision Study of Cs Polarizabilities. *J. Comput. Methods Sci. Eng.* **2007**, *7*, 521–540.
- (39) Singh, S.; Kaur, K.; Sahoo, B. K.; Arora, B. Comparing Magic Wavelengths for the Transitions of Cs Using Circularly and Linearly Polarized Light. *J. Phys. B At. Mol. Opt. Phys.* **2016**, *49*, 145005.
- (40) Safronova, U. I.; Johnson, W. R.; Safronova, M. S. Excitation Energies, Polarizabilities, Multipole Transition Rates, and Lifetimes of Ions along the Francium Isoelectronic Sequence. *Phys. Rev. A* **2007**, *76*, 042504.
- (41) Gobre, V. V. *Efficient Modelling of Linear Electronic Polarization in Materials Using Atomic Response Functions*; Technische Universitaet Berlin (Germany), 2016.
- (42) Singh, S.; Sahoo, B. K.; Arora, B. Determination of Magic Wavelengths for the  $7s^2S_{1/2} \rightarrow 7p^2P_{3/2,1/2}$  Transitions in Fr. *Phys. Rev. A* **2016**, *94*, 023418.
- (43) Cheng, Y.; Jiang, J.; Mitroy, J. Tune-out Wavelengths for the Alkaline-Earth-Metal Atoms. *Phys. Rev. A* **2013**, *88*, 022511.

- (44) Wu, L.; Wang, X.; Wang, T.; Jiang, J.; Dong, C. Be Optical Lattice Clocks with the Fractional Stark Shift up to the Level of  $10^{-19}$ . *New J. Phys.* **2023**, *25*, 043011.
- (45) Porsev, S. G.; Derevianko, A. High-Accuracy Calculations of Dipole, Quadrupole, and Octupole Electric Dynamic Polarizabilities and van Der Waals Coefficients C6, C8, and C10 for Alkaline-Earth Dimers. *J. Exp. Theor. Phys.* **2006**, *102*, 195–205.
- (46) Sahoo, B. K.; Das, B. P. Relativistic Coupled-Cluster Studies of Dipole Polarizabilities in Closed-Shell Atoms. *Phys. Rev. A* **2008**, *77*, 062516.
- (47) Singh, Y.; Sahoo, B. K.; Das, B. P. Correlation Trends in the Ground-State Static Electric Dipole Polarizabilities of Closed-Shell Atoms and Ions. *Phys. Rev. A* **2013**, *88*, 062504.
- (48) A. Manz, T.; Chen, T.; J. Cole, D.; Gabaldon Limas, N.; Fiszbein, B. New Scaling Relations to Compute Atom-in-Material Polarizabilities and Dispersion Coefficients: Part 1. Theory and Accuracy. *RSC Adv.* **2019**, *9*, 19297–19324.
- (49) Visentin, G.; Buchachenko, A. A. Polarizabilities, Dispersion Coefficients, and Retardation Functions at the Complete Basis Set CCSD Limit: From Be to Ba plus Yb. *The Journal of Chemical Physics* **2019**, *151*, 214302.
- (50) Lim, I. S.; Schwerdtfeger, P. Four-Component and Scalar Relativistic Douglas-Kroll Calculations for Static Dipole Polarizabilities of the Alkaline-Earth-Metal Elements and Their Ions from  $\{\mathrm{Ca}\}^n$  to  $\{\mathrm{Ra}\}^n$  ( $n=0, +1, +2$ ). *Phys. Rev. A* **2004**, *70*, 062501.
- (51) Borschevsky, A.; Pershina, V.; Eliav, E.; Kaldor, U. Ab Initio Predictions of Atomic Properties of Element 120 and Its Lighter Group-2 Homologues. *Phys. Rev. A* **2013**, *87*, 022502.

- (52) Dutta, N. N. Trend of Gaunt interaction contributions to the electric dipole polarizabilities of noble gas, alkaline-earth, and a few group-12 atoms. *Chem. Phys. Lett.* **2020**, *758*, 137911.
- (53) Müller, W.; Flesch, J.; Meyer, W. Treatment of Intershell Correlation Effects in Ab Initio Calculations by Use of Core Polarization Potentials. Method and Application to Alkali and Alkaline Earth Atoms. *J. Chem. Phys.* **1984**, *80*, 3297–3310.
- (54) Tunega, D.; Noga, J.; Klopper, W. Basis Set Limit Value for the Static Dipole Polarizability of Beryllium. *Chem. Phys. Lett.* **1997**, *269*, 435–440.
- (55) Patil, S. A Simple Model Potential Description of the Alkaline Earth Isoelectronic Sequences. *Eur. Phys. J. D* **2000**, *10*, 341–347.
- (56) Bendazzoli, G. L.; Monari, A. A Davidson Technique for the Computation of Dispersion Constants: Full CI Results for Be and LiH. *Chem. Phys.* **2004**, *306*, 153–161.
- (57) Dong, H.; Jiang, J.; Wu, Z.; Dong, C.; Gaigalas, G. Calculations of Atomic Polarizability for Beryllium Using MCDHF Method\*. *Chinese Phys. B* **2021**, *30*, 043103.
- (58) Lundin, L.; Engman, B.; Hilke, J.; Martinson, I. Lifetime Measurements in Mg I-Mg IV. *Phys. Scr.* **1973**, *8*, 274.
- (59) Reinsch, E.-A.; Meyer, W. Finite Perturbation Calculation for the Static Dipole Polarizabilities of the Atoms Na through Ca. *Phys. Rev. A* **1976**, *14*, 915–918.
- (60) Maeder, F.; Kutzelnigg, W. Natural States of Interacting Systems and Their Use for the Calculation of Intermolecular Forces: IV. Calculation of van Der Waals Coefficients between One- and Two-Valence-Electron Atoms in Their Ground States, as Well as of Polarizabilities, Oscillator Strength Sums and Related Quantities, Including Correlation Effects. *Chemical Physics* **1979**, *42*, 95–112.

- (61) Archibong, E. F.; Thakkar, A. J. Finite-Field Many-Body-Perturbation-Theory Calculation of the Static Hyperpolarizabilities and Polarizabilities of Mg,  $\{\mathrm{Al}\}^{\{+\}}$ , and Ca. *Phys. Rev. A* **1991**, *44*, 5478–5484.
- (62) Sadlej, A. J.; Urban, M. Medium-Size Polarized Basis Sets for High-Level-Correlated Calculations of Molecular Electric Properties: III. Alkali (Li, Na, K, Rb) and Alkaline-Earth (Be, Mg, Ca, Sr) Atoms. *Journal of Molecular Structure: THEOCHEM* **1991**, *234*, 147–171.
- (63) Stwalley, W. C. Polarizability and Long-Range Interactions of Magnesium Atoms. *The Journal of Chemical Physics* **1971**, *54*, 4517–4518.
- (64) Stiehler, J.; Hinze, J. Calculation of Static Polarizabilities and Hyperpolarizabilities for the Atoms He through Kr with a Numerical RHF Method. *J. Phys. B: At. Mol. Opt. Phys.* **1995**, *28*, 4055.
- (65) Bromley, M. W. J.; Mitroy, J. Configuration-Interaction Calculations of Positron Binding to Group-II Elements. *Phys. Rev. A* **2002**, *65*, 062505.
- (66) Roos, B. O.; Veryazov, V.; Widmark, P.-O. Relativistic Atomic Natural Orbital Type Basis Sets for the Alkaline and Alkaline-Earth Atoms Applied to the Ground-State Potentials for the Corresponding Dimers. *Theor. Chem. Acc.* **2004**, *111*, 345–351.
- (67) Porsev, S. G.; Derevianko, A. Multipolar Theory of Blackbody Radiation Shift of Atomic Energy Levels and Its Implications for Optical Lattice Clocks. *Phys. Rev. A* **2006**, *74*, 020502.
- (68) Hohm, U.; Thakkar, A. J. New Relationships Connecting the Dipole Polarizability, Radius, and Second Ionization Potential for Atoms. *J. Phys. Chem. A* **2012**, *116*, 697–703.

- (69) Chattopadhyay, S.; Mani, B. K.; Angom, D. Electric Dipole Polarizability of Alkaline-Earth-Metal Atoms from Perturbed Relativistic Coupled-Cluster Theory with Triples. *Phys. Rev. A* **2014**, *89*, 022506.
- (70) Bala, R.; Nataraj, H. S.; Nayak, M. K. Ab Initio Calculations of Permanent Dipole Moments and Dipole Polarizabilities of Alkaline-Earth Monofluorides. *J. Phys. B: At. Mol. Opt. Phys.* **2019**, *52*, 085101.
- (71) Shukla, N.; Arora, B.; Sharma, L.; Srivastava, R. Two-Dipole and Three-Dipole Dispersion Coefficients for Interaction of Alkaline-Earth-Metal Atoms with Alkaline-Earth-Metal Atoms and Alkaline-Earth-Metal Ions. *Phys. Rev. A* **2020**, *102*, 022817.
- (72) Canal Neto, A.; Ferreira, I. B.; Jorge, F. E.; de Oliveira, A. Z. All-Electron Triple Zeta Basis Sets for ZORA Calculations: Application in Studies of Atoms and Molecules. *Chemical Physics Letters* **2021**, *771*, 138548.
- (73) Neto, A. C.; de Oliveira, A. Z.; Jorge, F. E.; Camiletti, G. G. ZORA All-Electron Double Zeta Basis Sets for the Elements from H to Xe: Application in Atomic and Molecular Property Calculations. *J Mol Model* **2021**, *27*, 1–9.
- (74) Sarkisov, G. S. Laser Measurements of Static and Dynamic Dipole Polarizability for 11 Metal Atoms Using Fast Exploding Wires in Vacuum and Integrated-Phase Technique. *Physics of Plasmas* **2022**, *29*, 073502.
- (75) Sadlej, A. J.; Urban, M.; Gropen, O. Relativistic and Electron-Correlation Contributions to the Dipole Polarizability of the Alkaline-Earth-Metal Atoms Ca, Sr, and Ba. *Phys. Rev. A* **1991**, *44*, 5547–5557.
- (76) Porsev, S. G.; Derevianko, A. High-Accuracy Relativistic Many-Body Calculations of van Der Waals Coefficients  $\{C_6\}$  for Alkaline-Earth-Metal Atoms. *Phys. Rev. A* **2002**, *65*, 020701.



- (77) Moszynski, R.; Łach, G.; Jaszuński, M.; Bussery-Honvault, B. Long-Range Relativistic Interactions in the Cowan-Griffin Approximation and Their QED Retardation: Application to Helium, Calcium, and Cadmium Dimers. *Phys. Rev. A* **2003**, *68*, 052706.
- (78) Lide, D. R. *CRC Handbook of Chemistry and Physics*; CRC press, 2004; Vol. 85.
- (79) Schwartz, H. L.; Miller, T. M.; Bederson, B. Measurement of the Static Electric Dipole Polarizabilities of Barium and Strontium. *Phys. Rev. A* **1974**, *10*, 1924–1926.
- (80) Mitroy, J.; Zhang, J.-Y. Properties and Long Range Interactions of the Calcium Atom. *The Journal of Chemical Physics* **2008**, *128*, 134305.
- (81) Zhang, R.-K.; Jiang, J.; Dong, C.-Z.; Tang, Y.-B. Magic-Zero and Magic Wavelengths of the Ca Atom. *Phys. Rev. A* **2023**, *108*, 012803.
- (82) Porsev, S. G.; Ludlow, A. D.; Boyd, M. M.; Ye, J. Determination of Sr Properties for a High-Accuracy Optical Clock. *Phys. Rev. A* **2008**, *78*, 032508.
- (83) Mitroy, J.; Zhang, J. Dispersion and Polarization Interactions of the Strontium Atom. *Mol. Phys.* **2010**, *108*, 1999–2006.
- (84) Safronova, M. S.; Porsev, S. G.; Safronova, U. I.; Kozlov, M. G.; Clark, C. W. Blackbody-Radiation Shift in the Sr Optical Atomic Clock. *Phys. Rev. A* **2013**, *87*, 012509.
- (85) Schäfer, S.; Mehring, M.; Schäfer, R.; Schwerdtfeger, P. Polarizabilities of Ba and  $\text{Ba}_2$ : Comparison of Molecular Beam Experiments with Relativistic Quantum Chemistry. *Phys. Rev. A* **2007**, *76*, 052515.
- (86) Dzuba, V. A. Ionization Potentials and Polarizabilities of Superheavy Elements from Db to Cn ( $Z=105\text{--}112$ ). *Phys. Rev. A* **2016**, *93*, 032519.

- (87) Buchachenko, A. A.; Viehland, L. A. Interaction Potentials and Transport Properties of Ba, Ba<sup>+</sup>, and Ba<sup>2+</sup> in Rare Gases from He to Xe. *The Journal of Chemical Physics* **2018**, *148*, 154304.
- (88) Sahoo, B. K.; Das, B. P. The Role of Relativistic Many-Body Theory in Probing New Physics beyond the Standard Model via the Electric Dipole Moments of Diamagnetic Atoms. *J. Phys. Conf. Ser.* **2018**, *1041*, 012014.
- (89) Flambaum, V. V.; Dzuba, V. A. Electric Dipole Moments of Atoms and Molecules Produced by Enhanced Nuclear Schiff Moments. *Phys. Rev. A* **2020**, *101*, 042504.
- (90) Werner, H.-J.; Meyer, W. Finite Perturbation Calculations for the Static Dipole Polarizabilities of the First-Row Atoms. *Phys. Rev. A* **1976**, *13*, 13–16.
- (91) Éhn, L.; Černušák, I. Atomic and Ionic Polarizabilities of B, C, N, O, and F. *Int. J. Quantum Chem.* **2021**, *121*, e26467.
- (92) Wang, K.; Wang, X.; Fan, Z.; Zhao, H.-Y.; Miao, L.; Yin, G.-J.; Moro, R.; Ma, L. Static Dipole Polarizabilities of Atoms and Ions from  $Z = 1$  to 20 Calculated within a Single Theoretical Scheme. *Eur. Phys. J. D* **2021**, *75*, 1–11.
- (93) Fleig, T. Spin-Orbit-Resolved Static Polarizabilities of Group-13 Atoms: Four-component Relativistic Configuration Interaction and Coupled Cluster Calculations. *Phys. Rev. A* **2005**, *72*, 052506.
- (94) Kumar, R.; Angom, D.; Mani, B. K. Fock-Space Perturbed Relativistic Coupled-Cluster Theory for Electric Dipole Polarizability of One-Valence Atomic Systems: Application to Al and In. *Phys. Rev. A* **2022**, *106*, 032801.
- (95) Sarkisov, G. S.; Beigman, I. L.; Shevelko, V. P.; Struve, K. W. Interferometric Measurements of Dynamic Polarizabilities for Metal Atoms Using Electrically Exploding Wires in Vacuum. *Phys. Rev. A* **2006**, *73*, 042501.

- (96) Chen, Z.; Wu, J.; Lu, Y.; Jiang, Z.; Zhang, C.; Wang, Z.; Shi, H.; Li, X.; Zhou, L. Measurement of Dynamic Atomic Polarizabilities of Al at 19 Wavelengths from 420 Nm to 680 Nm in Electrical Exploding Wire Experiments. *Opt. Express, OE* **2022**, *30*, 26102–26110.
- (97) Buchachenko, A. A. State-Interacting Spin-Orbit Configuration Interaction Method for J-resolved Anisotropic Static Dipole Polarizabilities: Application to Al, Ga, In, and Tl Atoms. *Russ. J. Phys. Chem.* **2010**, *84*, 2325–2333.
- (98) Lupinetti, C.; Thakkar, A. J. Polarizabilities and Hyperpolarizabilities for the Atoms Al, Si, P, S, Cl, and Ar: Coupled Cluster Calculations. *The Journal of Chemical Physics* **2005**, *122*, 044301.
- (99) Borschevsky, A.; Zelovich, T.; Eliav, E.; Kaldor, U. Precision of Calculated Static Polarizabilities: Ga, In and Tl Atoms. *Chem. Phys.* **2012**, *395*, 104–107.
- (100) Černušák, I.; Kellö, V.; Sadlej, A. J. Standardized Medium-Size Basis Sets for Calculations of Molecular Electric Properties: Group IIIA. *Collect. Czech. Chem. Commun.* **2003**, *68*, 211–239.
- (101) Pershina, V.; Borschevsky, A.; Eliav, E.; Kaldor, U. Adsorption of Inert Gases Including Element 118 on Noble Metal and Inert Surfaces from Ab Initio Dirac–Coulomb Atomic Calculations. *J. Chem. Phys.* **2008**, *129*, 144106.
- (102) Dzuba, V. A.; Flambaum, V. V. Electron Structure of Superheavy Elements Uut, Fl and Uup (Z=113 to 115). *Hyperfine Interact.* **2016**, *237*, 160.
- (103) Hibbert, A. Atomic Polarisabilities and Polarised Pseudostates in the Multiconfigurational Approach. III. Second-row Atoms and Ions. *J. Phys. B At. Mol. Phys.* **1980**, *13*, 3725.

- (104) Milani, P.; Moullet, I.; de Heer, W. A. Experimental and Theoretical Electric Dipole Polarizabilities of Al and  $\{\mathrm{Al}\}_2$ . *Phys. Rev. A* **1990**, *42*, 5150–5154.
- (105) Chu, X.; Dalgarno, A. Linear Response Time-Dependent Density Functional Theory for van Der Waals Coefficients. *J. Chem. Phys.* **2004**, *121*, 4083–4088.
- (106) Fuentealba, P. The Static Dipole Polarizability of Aluminium Atom: Discrepancy between Theory and Experiment. *Chem. Phys. Lett.* **2004**, *397*, 459–461.
- (107) Gould, T. How Polarizabilities and C6 Coefficients Actually Vary with Atomic Volume. *The Journal of Chemical Physics* **2016**, *145*, 084308.
- (108) Wang, K.; Fang, S.-Z.; Fan, Z.; Zhao, H.-Y.; Miao, L.; Yin, G.-J.; Moro, R.; Ma, L. Reconciliation of the Theoretical and Experimental Value of the Static Electric Polarizability of the Aluminum Atom. *J. Clust. Sci.* **2023**, *34*, 2147–2151.
- (109) Gould, T.; Bučko, T. C6 Coefficients and Dipole Polarizabilities for All Atoms and Many Ions in Rows 1–6 of the Periodic Table. *J. Chem. Theory Comput.* **2016**, *12*, 3603–3613.
- (110) Guella, T. P.; Miller, T. M.; Bederson, B.; Stockdale, J. A. D.; Jaduszliwer, B. Polarizability of  $5s^25p(^2P_{1/2})$  Atomic Indium. *Phys. Rev. A* **1984**, *29*, 2977–2980.
- (111) Safronova, M. S.; Safronova, U. I.; Porsev, S. G. Polarizabilities, Stark Shifts, and Lifetimes of the In Atom. *Phys. Rev. A* **2013**, *87*, 032513.
- (112) Safronova, M. S.; Johnson, W. R.; Safronova, U. I.; Cowan, T. E. Relativistic Many-Body Calculations of the Stark-induced Amplitude of the  $6P_{1/2} \rightarrow 7P_{1/2}$  Transition in Thallium. *Phys. Rev. A* **2006**, *74*, 022504.

- (113) Pershina, V.; Borschevsky, A.; Eliav, E.; Kaldor, U. Atomic Properties of Element 113 and Its Adsorption on Inert Surfaces from Ab Initio Dirac-Coulomb Calculations. *J. Phys. Chem. A* **2008**, *112*, 13712–13716.
- (114) Dzuba, V. A.; Flambaum, V. V. Calculation of the  $(T,P)$ -Odd Electric Dipole Moment of Thallium and Cesium. *Phys. Rev. A* **2009**, *80*, 062509.
- (115) Mitroy, J.; Safronova, M. S.; Clark, C. W. Theory and Applications of Atomic and Ionic Polarizabilities. *J. Phys. B: At. Mol. Opt. Phys.* **2010**, *43*, 202001.
- (116) Kozlov, M. G.; Porsev, S. G.; Johnson, W. R. Parity Nonconservation in Thallium. *Phys. Rev. A* **2001**, *64*, 052107.
- (117) Safronova, M. S.; Majumder, P. K. Thallium  $7s$  Lifetimes Derived from Experimental Data and Ab Initio Calculations of Scalar Polarizabilities. *Phys. Rev. A* **2013**, *87*, 042502.
- (118) Borschevsky, A.; Yakobi, H.; Eliav, E.; Kaldor, U. High-Accuracy Coupled Cluster Calculations of Atomic Properties. *AIP Conference Proceedings* **2015**, *1642*, 209–212.
- (119) Tang, Y.-B.; Gao, N.-N.; Lou, B.-Q.; Shi, T.-Y. Relativistic Coupled-Cluster Calculations of the Polarizabilities of Atomic Thallium. *Phys. Rev. A* **2018**, *98*, 062511.
- (120) Thierfelder, C.; Assadollahzadeh, B.; Schwerdtfeger, P.; Schäfer, S.; Schäfer, R. Relativistic and Electron Correlation Effects in Static Dipole Polarizabilities for the Group-14 Elements from Carbon to Element  $Z = 114$ : Theory and Experiment. *Phys. Rev. A* **2008**, *78*, 052506.
- (121) Maroulis, G.; Pouchan, C. Static Dipole (Hyper)Polarizability of the Silicon Atom. *J. Phys. B: At. Mol. Opt. Phys.* **2003**, *36*, 2011.
- (122) Andersson, K.; Sadlej, A. J. Electric Dipole Polarizabilities of Atomic Valence States. *Phys. Rev. A* **1992**, *46*, 2356–2362.

- (123) Mori, N. A.; Scarlett, L. H.; Bray, I.; Fursa, D. V. Convergent Close-Coupling Calculations of Positron Scattering from Atomic Carbon. *Phys. Rev. A* **2023**, *107*, 032817.
- (124) Doolen, G.; Liberman, D. A. Calculations of Photoabsorption by Atoms Using a Linear Response Method. *Phys. Scr.* **1987**, *36*, 77.
- (125) Assadollahzadeh, B.; Schäfer, S.; Schwerdtfeger, P. Electronic properties for small tin clusters  $S_{nn}$  ( $n \leq 20$ ) from density functional theory and the convergence toward the solid state. *J. Comput. Chem.* **2010**, *31*, 929–937.
- (126) Nash, C. S. Atomic and Molecular Properties of Elements 112, 114, and 118. *J. Phys. Chem. A* **2005**, *109*, 3493–3500.
- (127) Pershina, V.; Borschevsky, A.; Eliav, E.; Kaldor, U. Prediction of the Adsorption Behavior of Elements 112 and 114 on Inert Surfaces from Ab Initio Dirac-Coulomb Atomic Calculations. *The Journal of Chemical Physics* **2008**, *128*, 024707.
- (128) Zalialiutdinov, T.; Solovyev, D.; Labzowsky, L.; Plunien, G. Spin-Statistic Selection Rules for Multiphoton Transitions: Application to Helium Atoms. *Phys. Rev. A* **2016**, *93*, 012510.
- (129) Oleynichenko, A. V.; Zaitsevskii, A.; Skripnikov, L. V.; Eliav, E. Relativistic Fock Space Coupled Cluster Method for Many-Electron Systems: Non-Perturbative Account for Connected Triple Excitations. *Symmetry* **2020**, *12*, 1101.
- (130) Neto, A. C.; Jorge, F. E.; da Cruz, H. R. C. All-Electron ZORA Triple Zeta Basis Sets for the Elements Cs–La and Hf–Rn. *Chinese Phys. B* **2023**, *32*, 093101.
- (131) Alpher, R. A.; White, D. R. Optical Refractivity of High-Temperature Gases. I. Effects Resulting from Dissociation of Diatomic Gases. *Phys. Fluids* **1959**, *2*, 153.
- (132) Zeiss, G.; Meath, W. J. Dispersion Energy Constants  $C_6(A, B)$ , Dipole Oscillator

- Strength Sums and Refractivities for Li, N, O, H<sub>2</sub>, N<sub>2</sub>, O<sub>2</sub>, NH<sub>3</sub>, H<sub>2</sub>O, NO and N<sub>2</sub>O. *Mol. Phys.* **1977**, *33*, 1155–1176.
- (133) Buchachenko, A. A. Anisotropy of the Static Dipole Polarizability Induced by the Spin–Orbit Interaction: The S-state Atoms N–Bi, Cr, Mo and Re. *Proc. R. Soc. Math. Phys. Eng. Sci.* **2010**, *467*, 1310–1328.
- (134) Visentin, G.; Kalinina, I. S.; Buchachenko, A. A. Extended Combination Rule for Like-Atom Dipole Dispersion Coefficients. *The Journal of Chemical Physics* **2020**, *153*, 064110.
- (135) Maroulis, G. Cluster Size Effect on the Electric Polarizability and Hyperpolarizability in Small Antimony Clusters Sbn, N=1,2 and 4. *Chem. Phys. Lett.* **2007**, *444*, 44–47.
- (136) Roos, B. O.; Lindh, R.; Malmqvist, P.-Å.; Veryazov, V.; Widmark, P.-O. Main Group Atoms and Dimers Studied with a New Relativistic ANO Basis Set. *J. Phys. Chem. A* **2004**, *108*, 2851–2858.
- (137) Kellö, V.; Sadlej, A. J. Medium-Size Polarized Basis Sets for High-Level-Correlated Calculations of Molecular Electric Properties. *Theoret. Chim. Acta* **1992**, *83*, 351–366.
- (138) Centoducatte, R.; de Oliveira, A. Z.; Jorge, F. E.; Camiletti, G. G. ZORA Double Zeta Basis Sets for Fifth Row Elements: Application in Studies of Electronic Structures of Atoms and Molecules. *Computational and Theoretical Chemistry* **2022**, *1207*, 113511.
- (139) Pershina, V. In *The Chemistry of Superheavy Elements*; Schädel, M., Shaughnessy, D., Eds.; Springer: Berlin, Heidelberg, 2014; pp 135–239.
- (140) Cuthbertson, C.; Metcalfe, E. P.; Trouton, F. T. On the Dispersion of Gaseous Mercury, Sulphur, Phosphorous, and Helium. *Proc. R. Soc. Lond. Ser. Contain. Pap. Math. Phys. Character* **1997**, *80*, 411–419.

- (141) MEDVEDĚ, M.; FOWLER, P. W.; HUTSON, J. M. Anisotropic Dipole Polarizabilities and Quadrupole Moments of Open-Shell Atoms and Ions: O, F, S, Cl, Se, Br and Isoelectronic Systems. *Mol. Phys.* **2000**, *98*, 453–463.
- (142) Sadlej, A. J. Medium-Size Polarized Basis Sets for High-Level-Correlated Calculations of Molecular Electric Properties. *Theoret. Chim. Acta* **1992**, *81*, 339–354.
- (143) Allehabi, S. O.; Brewer, S. M.; Dzuba, V. A.; Flambaum, V. V.; Beloy, K. High-Accuracy Optical Clocks Based on Group-16-like Highly Charged Ions. *Phys. Rev. A* **2022**, *106*, 043101.
- (144) Fleig, T.; Sadlej, A. J. Electric dipole polarizabilities of the halogen atoms in  $^2P_{1/2}$  and  $^2P_{3/2}$  states: Scalar relativistic and two-component configuration-interaction calculations. *Phys. Rev. A* **2002**, *65*, 032506.
- (145) de Farias, R. F. Estimation of Some Physical Properties for Tennessine and Tennessine Hydride (TsH). *Chem. Phys. Lett.* **2017**, *667*, 1–3.
- (146) Maroulis, G.; Makris, C.; Hohm, U.; Goebel, D. Electrooptical Properties and Molecular Polarization of Iodine, I<sub>2</sub>. *J. Phys. Chem. A* **1997**, *101*, 953–956.
- (147) Newell, A. C.; Baird, R. C. Absolute Determination of Refractive Indices of Gases at 47.7 Gigahertz. *Journal of Applied Physics* **1965**, *36*, 3751–3759.
- (148) Schooley, J. F. *Temperature: Its Measurement and Control in Science and Industry*; American Institute of Physics: New York, 1992; Vol. 1269.
- (149) Schmidt, J. W.; Gavioso, R. M.; May, E. F.; Moldover, M. R. Polarizability of Helium and Gas Metrology. *Phys. Rev. Lett.* **2007**, *98*, 254504.
- (150) Gaiser, C.; Fellmuth, B. Polarizability of Helium, Neon, and Argon: New Perspectives for Gas Metrology. *Phys. Rev. Lett.* **2018**, *120*, 123203.



- (151) Pachucki, K.; Sapirstein, J. Relativistic and QED Corrections to the Polarizability of Helium. *Phys. Rev. A* **2000**, *63*, 012504.
- (152) Łach, G.; Jeziorski, B.; Szalewicz, K. Radiative Corrections to the Polarizability of Helium. *Phys. Rev. Lett.* **2004**, *92*, 233001.
- (153) Puchalski, M.; Szalewicz, K.; Lesiuk, M.; Jeziorski, B. QED Calculation of the Dipole Polarizability of Helium Atom. *Phys. Rev. A* **2020**, *101*, 022505.
- (154) Orcutt, R. H.; Cole, R. H. Dielectric Constants of Imperfect Gases. III. Atomic Gases, Hydrogen, and Nitrogen. *The Journal of Chemical Physics* **1967**, *46*, 697–702.
- (155) Huot, J.; Bose, T. K. Experimental Determination of the Dielectric Virial Coefficients of Atomic Gases as a Function of Temperature. *The Journal of Chemical Physics* **1991**, *95*, 2683–2687.
- (156) Dalgarno, A.; Kingston, A. E.; Bates, D. R. The Refractive Indices and Verdet Constants of the Inert Gases. *Proc. R. Soc. Lond. Ser. Math. Phys. Sci.* **1997**, *259*, 424–431.
- (157) Hohm, U.; Kerl, K. Interferometric Measurements of the Dipole Polarizability  $\alpha$  of Molecules between 300 K and 1100 K. *Mol. Phys.* **1990**, *69*, 803–817.
- (158) Chattopadhyay, S.; Mani, B. K.; Angom, D. Perturbed Coupled-Cluster Theory to Calculate Dipole Polarizabilities of Closed-Shell Systems: Application to Ar, Kr, Xe, and Rn. *Phys. Rev. A* **2012**, *86*, 062508.
- (159) Langhoff, P. W.; Karplus, M. Padé Summation of the Cauchy Dispersion Equation\*. *J. Opt. Soc. Am., JOSA* **1969**, *59*, 863–871.
- (160) Nakajima, T.; Hirao, K. Relativistic Effects for Polarizabilities and Hyperpolarizabilities of Rare Gas Atoms. *Chem. Lett.* **2001**, *30*, 766–767.

- (161) Soldán, P.; Lee, E. P. F.; Wright, T. G. Static Dipole Polarizabilities ( $\alpha$ ) and Static Second Hyperpolarizabilities ( $\gamma$ ) of the Rare Gas Atoms (He–Rn). *Phys. Chem. Chem. Phys.* **2001**, *3*, 4661–4666.
- (162) Bezchastnov, V. G.; Pernpointner, M.; Schmelcher, P.; Cederbaum, L. S. Nonadditivity and anisotropy of the polarizability of clusters: Relativistic finite-field calculations for the Xe dimer. *Phys. Rev. A* **2010**, *81*, 062507.
- (163) Sakurai, A.; Sahoo, B. K.; Das, B. P. Electric Dipole Polarizability of  $^{129}\text{Xe}$  Using the Relativistic Coupled-Cluster and the Normal Coupled-Cluster Methods. *Phys. Rev. A* **2018**, *97*, 062510.
- (164) Smits, O. R.; Jerabek, P.; Pahl, E.; Schwerdtfeger, P. A Hundred-year-old Experiment Re-evaluated: Accurate Ab Initio Monte Carlo Simulations of the Melting of Radon. *Angew. Chem. Int. Ed.* **2018**, *57*, 9961–9964.
- (165) Kumar, R.; Chattopadhyay, S.; Angom, D.; Mani, B. K. Relativistic Coupled-Cluster Calculation of the Electric Dipole Polarizability and Correlation Energy of Cn,  $\text{Nh}^+$ , and Og: Correlation Effects from Lighter to Superheavy Elements. *Phys. Rev. A* **2021**, *103*, 062803.
- (166) Jerabek, P.; Schuetrumpf, B.; Schwerdtfeger, P.; Nazarewicz, W. Electron and Nucleon Localization Functions of Oganesson: Approaching the Thomas-Fermi Limit. *Phys. Rev. Lett.* **2018**, *120*, 053001.
- (167) Puchalski, M.; Piszczatowski, K.; Komasa, J.; Jeziorski, B.; Szalewicz, K. Theoretical Determination of the Polarizability Dispersion and the Refractive Index of Helium. *Phys. Rev. A* **2016**, *93*, 032515.
- (168) Rice, J. E.; Scuseria, G. E.; Lee, T. J.; Taylor, P. R.; Almlöf, J. Connected Triple Excitations in Coupled-Cluster Calculations of Hyperpolarizabilities: Neon. *Chem. Phys. Lett.* **1992**, *191*, 23–28.

- (169) Hald, K.; Pawłowski, F.; Jørgensen, P.; Hättig, C. Calculation of Frequency-Dependent Polarizabilities Using the Approximate Coupled-Cluster Triples Model CC3. *The Journal of Chemical Physics* **2003**, *118*, 1292–1300.
- (170) Larsen, H.; Olsen, J.; Hättig, C.; Jørgensen, P.; Christiansen, O.; Gauss, J. Polarizabilities and First Hyperpolarizabilities of HF, Ne, and BH from Full Configuration Interaction and Coupled Cluster Calculations. *The Journal of Chemical Physics* **1999**, *111*, 1917–1925.
- (171) Gaiser, C.; Fellmuth, B. Experimental Benchmark Value for the Molar Polarizability of Neon. *Europhys. Lett.* **2010**, *90*, 63002.
- (172) Chattopadhyay, S.; Mani, B. K.; Angom, D. Electric Dipole Polarizability from Perturbed Relativistic Coupled-Cluster Theory: Application to Neon. *Phys. Rev. A* **2012**, *86*, 022522.
- (173) Lesiuk, M.; Przybytek, M.; Jeziorski, B. Theoretical Determination of Polarizability and Magnetic Susceptibility of Neon. *Phys. Rev. A* **2020**, *102*, 052816.
- (174) Hellmann, R. Determination of the Polarizability of Neon. *Phys. Rev. A* **2022**, *105*, 022809.
- (175) Johnston, D. R.; Oudemans, G. J.; Cole, R. H. Dielectric Constants of Imperfect Gases. I. Helium, Argon, Nitrogen, and Methane. *The Journal of Chemical Physics* **1960**, *33*, 1310–1317.
- (176) Lesiuk, M.; Jeziorski, B. First-Principles Calculation of the Frequency-Dependent Dipole Polarizability of Argon. *Phys. Rev. A* **2023**, *107*, 042805.
- (177) Thakkar, A. J.; Hettema, H.; Wormer, P. E. S. Ab Initio Dispersion Coefficients for Interactions Involving Rare-gas Atoms. *The Journal of Chemical Physics* **1992**, *97*, 3252–3257.

- (178) Mani, B. K.; Latha, K. V. P.; Angom, D. Relativistic Coupled-Cluster Calculations of  $^{20}\text{N}$ ,  $^{40}\text{Ar}$ ,  $^{84}\text{Kr}$ , and  $^{129}\text{Xe}$ : Correlation Energies and Dipole Polarizabilities. *Phys. Rev. A* **2009**, *80*, 062505.
- (179) Runeberg, N.; Pyykkö, P. Relativistic pseudopotential calculations on  $\text{Xe}_2$ ,  $\text{RnXe}$ , and  $\text{Rn}_2$ : The van der Waals properties of radon. *Int. J. Quantum Chem.* **1998**, *66*, 131–140.
- (180) Sahoo, B. K.; Yamanaka, N.; Yanase, K. Revisiting Theoretical Analysis of the Electric Dipole Moment of  $^{129}\text{Xe}$ . *Phys. Rev. A* **2023**, *108*, 042811.
- (181) Wesendrup, R.; Schwerdtfeger, P. Extremely Strong  $\text{S}_2 - \text{S}_2$  Closed-Shell Interactions. *Angew. Chem. Int. Ed.* **2000**, *39*, 907–910.
- (182) Labello, N. P.; Ferreira, A. M.; Kurtz, H. A. An augmented effective core potential basis set for the calculation of molecular polarizabilities. *J. Comput. Chem.* **2005**, *26*, 1464–1471.
- (183) Sulzer, D.; Norman, P.; Saue, T. Atomic  $\text{C}_6$  Dispersion Coefficients: A Four-Component Relativistic Kohn–Sham Study. *Mol. Phys.* **2012**, *110*, 2535–2541.
- (184) Pantazis, D. A.; Neese, F. All-Electron Scalar Relativistic Basis Sets for the 6p Elements. *Theor Chem Acc* **2012**, *131*, 1292.
- (185) Dzuba, V. A.; Berengut, J. C.; Ginges, J. S. M.; Flambaum, V. V. Screening of an Oscillating External Electric Field in Atoms. *Phys. Rev. A* **2018**, *98*, 043411.
- (186) McNeill, A. S.; Peterson, K. A.; Dixon, D. A. Polarizabilities of neutral atoms and atomic ions with a noble gas electron configuration. *J. Chem. Phys.* **2020**, *153*, 174304.
